# Supplementary material for: Integrable systems in 4D associated with sixfolds in Gr(4,6)
Source: arXiv:1705.06999 ancillary file (2017-05-18)
Supplement: Supplementary file 1 [file DFKN-2017-Integrability-Ex.pdf]

This worksheet accompanies the paper B.Doubrov, E.Ferapontov, B.Kruglikov, V.Novikov "Integrable systems in 4D associated with sixfolds in Gr(4,6)".

The file ran on **Maple** version 17, the package **DifferentialGeometry** was used.

In this worksheet we check that all equations from the Tables classifying linearly degenerate systems posses the property of self-duality of the conformal structures on every solution. We omit 4 cases of Monge-Ampere types as obvious, concentrating only on the general linearly degenerate 2x2 systems.

We do not compute for Segre types [1] and [0] but integrability of the geometry (self-duality) in the presence of Lax pair follows in any case from the work D.Calderbank, B.Kruglikov "Integrability via geometry: dispresionless differential equations in three and four dimensions" (arXiv:1612.02753).

The computations below therefore are only independent verifications for Segre types [1,1,1,1]-...-[2].

```
>
> with(DifferentialGeometry):with(Tensor):with(Tools):with(JetCalculus):with(LinearAlgebra):
  with(PDEtools, D_Dx, declare, ToJet, FromJet): with(DEtools):DepVars := [u(x1, x2, x3, x4),v(x1,
  x2, x3, x4)]:
```

```
> Preferences("ShowFramePrompt",'false'):
```

```
> DGsetup([x1, x2, x3, x4], M, quiet) :
```

```
>
```

Type [1,1,1,1]

```
> F := u1·v2 - α·u2·v1 : H := u1·v3 - u4·v1 :
```

```
> DR := (diff(F, u1)·ξ1 + diff(F, u2)·ξ2 + diff(F, u3)·ξ3 + diff(F, u4)·ξ4)·(diff(H, v1)·ξ1
  + diff(H, v2)·ξ2 + diff(H, v3)·ξ3 + diff(H, v4)·ξ4) - (diff(F, v1)·ξ1 + diff(F, v2)·ξ2
  + diff(F, v3)·ξ3 + diff(F, v4)·ξ4)·(diff(H, u1)·ξ1 + diff(H, u2)·ξ2 + diff(H, u3)·ξ3
  + diff(H, u4)·ξ4) :
```

```
GA := Matrix([ [diff(DR, ξ1, ξ1), diff(DR, ξ1, ξ2), diff(DR, ξ1, ξ3), diff(DR, ξ1, ξ4)],
  [diff(DR, ξ1, ξ2), diff(DR, ξ2, ξ2), diff(DR, ξ2, ξ3), diff(DR, ξ2, ξ4)], [diff(DR, ξ1,
  ξ3), diff(DR, ξ2, ξ3), diff(DR, ξ3, ξ3), diff(DR, ξ3, ξ4)], [diff(DR, ξ1, ξ4), diff(DR, ξ2,
  ξ4), diff(DR, ξ3, ξ4), diff(DR, ξ4, ξ4)] ] ) :
```

```
AA := FromJet(GA, DepVars) : Ai := MatrixInverse(AA) :
```

```
g := evalDG(add(add(Ai[i, j]·dx||i &t dx||j, i = 1..4), j = 1..4)) : gInv
  := evalDG(add(add(AA[i, j]·D_x||i &t D_x||j, i = 1..4), j = 1..4)) :
```

```
> DGsetup([x1, x2, x3, x4], [u, v], E, 3) :
  unkn0 := {u1, v3} : contr0 := {F, H} : unkn := unkn0 : contr := contr0 :for i to 4 do unkn
  := {op(unkn), TotalDiff(unkn0[1], i), TotalDiff(unkn0[2], i)} : contr := {op(contr),
  TotalDiff(contr0[1], i), TotalDiff(contr0[2], i)} : for j to i do unkn := {op(unkn),
  TotalDiff(unkn0[1], [i, j]), TotalDiff(unkn0[2], [i, j])} : contr := {op(contr),
  TotalDiff(contr0[1], [i, j]), TotalDiff(contr0[2], [i, j])} :od:od: SS := solve(contr,
  unkn) :
```

```
> ChangeFrame(M) :
  W := simplify(WeylTensor(g)) : gI2 := evalDG(gInv &t gInv) : tmp := ContractIndices(gI2,
  W, [[1, 1], [3, 2]]) :
```

$$\begin{aligned}
& \triangleright \text{densV} := \text{simplify}(\text{sqrt}(\text{Determinant}(A_i))) \text{ assuming } \frac{\partial}{\partial x1} u(x1, x2, x3, x4) > 0, \frac{\partial}{\partial x1} v(x1, \\
& \quad x2, x3, x4) > 0, \left( \frac{\partial}{\partial x1} u(x1, x2, x3, x4) \right) \left( \frac{\partial}{\partial x2} v(x1, x2, x3, x4) \right) > \left( \frac{\partial}{\partial x2} u(x1, x2, \right. \\
& \quad \left. x3, x4) \right) \left( \frac{\partial}{\partial x1} v(x1, x2, x3, x4) \right) \alpha^2, \alpha > 0; \\
& \text{densV} := 1 / \left( \left( - \left( \frac{\partial}{\partial x2} u(x1, x2, x3, x4) \right) \left( \frac{\partial}{\partial x1} v(x1, x2, x3, x4) \right) \alpha^2 + \left( \frac{\partial}{\partial x1} u(x1, x2, \right. \right. \quad (1) \\
& \quad \left. \left. x3, x4) \right) \left( \frac{\partial}{\partial x2} v(x1, x2, x3, x4) \right) \right) \left( \frac{\partial}{\partial x1} v(x1, x2, x3, x4) \right) \left( \frac{\partial}{\partial x1} u(x1, x2, x3, x4) \right) \right)
\end{aligned}$$

$$\begin{aligned}
& \triangleright V := \text{evalDG}(\text{densV} \cdot dx1 \text{ \&w } dx2 \text{ \&w } dx3 \text{ \&w } dx4) : \\
& \# VV := \text{convert}(V, \text{DGtensor}) :
\end{aligned}$$

$$\begin{aligned}
& \triangleright Wst := \text{evalDG} \left( \frac{1}{2} \cdot \text{ContractIndices}(V, \text{tmp}, [[3, 1], [4, 2]]) \right) : \\
& A := \text{simplify}(\text{subs}(SS, \text{ToJet}(\text{ContractIndices}(W, \text{evalDG}(D\_x1 \text{ \&t } D\_x2 \text{ \&t } D\_x3 \text{ \&t } D\_x4), \\
& \quad [[1, 1], [2, 2], [3, 3], [4, 4]]), \text{DepVars}, \text{notation} = \text{jetnumbers}))) ; \\
& B := \text{simplify}(\text{subs}(SS, \text{ToJet}(\text{ContractIndices}(Wst, \text{evalDG}(D\_x1 \text{ \&t } D\_x2 \text{ \&t } D\_x3 \text{ \&t } D\_x4), \\
& \quad [[1, 1], [2, 2], [3, 3], [4, 4]]), \text{DepVars}, \text{notation} = \text{jetnumbers}))) ; \\
& \text{simplify}(A - B)
\end{aligned}$$

$$\begin{aligned}
A := & \frac{1}{4} \frac{1}{v_2^2 v_1^4 u_2^4 \alpha^2} \left( 2 \alpha u_2^3 v_1^3 v_2 v_{2,2,4} - 2 \alpha u_2^3 v_1^3 v_{2,2} v_{2,4} - 2 \alpha u_2^3 v_1^2 v_2^2 v_{1,2,4} + 2 \alpha \right. \\
& u_2^3 v_1 v_2^2 v_{1,2} v_{1,4} - 2 \alpha u_2^2 u_4 v_1^3 v_2 v_{2,2,2} + 2 \alpha u_2^2 u_4 v_1^3 v_{2,2}^2 + 2 \alpha u_2^2 u_4 v_1^2 v_2^2 v_{1,2,2} \\
& - 2 \alpha u_2^2 u_4 v_1 v_2^2 v_{1,2}^2 - 2 \alpha u_2^2 u_{2,4} v_1^3 v_2 v_{2,2} + 2 \alpha u_2^2 u_{2,4} v_1^2 v_2^2 v_{1,2} - 2 \alpha u_2^2 u_{2,2,4} \\
& v_1^3 v_2^2 + 2 \alpha u_2 u_4 u_{2,2} v_1^3 v_2 v_{2,2} - 2 \alpha u_2 u_4 u_{2,2} v_1^2 v_2^2 v_{1,2} + 2 \alpha u_2 u_4 u_{2,2,2} v_1^3 v_2^2 \\
& + 4 \alpha u_2 u_{2,2} u_{2,4} v_1^3 v_2^2 - 4 \alpha u_4 u_{2,2}^2 v_1^3 v_2^2 - u_2^2 u_4 v_1^2 v_2^2 v_{1,2,2} + u_2^2 u_4 v_1^2 v_2 v_{1,2} v_{2,2} \\
& \left. + u_2^2 u_4 v_1 v_2^3 v_{1,1,2} - u_2^2 u_4 v_2^3 v_{1,1} v_{1,2} \right)
\end{aligned}$$

$$\begin{aligned}
B := & \frac{1}{4} \frac{1}{v_2^2 v_1^4 u_2^4 \alpha^2} \left( 2 \alpha u_2^3 v_1^3 v_2 v_{2,2,4} - 2 \alpha u_2^3 v_1^3 v_{2,2} v_{2,4} - 2 \alpha u_2^3 v_1^2 v_2^2 v_{1,2,4} + 2 \alpha \right. \\
& u_2^3 v_1 v_2^2 v_{1,2} v_{1,4} - 2 \alpha u_2^2 u_4 v_1^3 v_2 v_{2,2,2} + 2 \alpha u_2^2 u_4 v_1^3 v_{2,2}^2 + 2 \alpha u_2^2 u_4 v_1^2 v_2^2 v_{1,2,2} \\
& - 2 \alpha u_2^2 u_4 v_1 v_2^2 v_{1,2}^2 - 2 \alpha u_2^2 u_{2,4} v_1^3 v_2 v_{2,2} + 2 \alpha u_2^2 u_{2,4} v_1^2 v_2^2 v_{1,2} - 2 \alpha u_2^2 u_{2,2,4} \\
& v_1^3 v_2^2 + 2 \alpha u_2 u_4 u_{2,2} v_1^3 v_2 v_{2,2} - 2 \alpha u_2 u_4 u_{2,2} v_1^2 v_2^2 v_{1,2} + 2 \alpha u_2 u_4 u_{2,2,2} v_1^3 v_2^2 \\
& + 4 \alpha u_2 u_{2,2} u_{2,4} v_1^3 v_2^2 - 4 \alpha u_4 u_{2,2}^2 v_1^3 v_2^2 - u_2^2 u_4 v_1^2 v_2^2 v_{1,2,2} + u_2^2 u_4 v_1^2 v_2 v_{1,2} v_{2,2} \\
& \left. + u_2^2 u_4 v_1 v_2^3 v_{1,1,2} - u_2^2 u_4 v_2^3 v_{1,1} v_{1,2} \right)
\end{aligned}$$

0

(2)

$$\begin{aligned}
& \triangleright \text{ANS} := \text{simplify}(\text{expand}(\text{subs}(SS, \text{ToJet}(\text{DGinfo}(\text{evalDG}(W - Wst), \text{"CoefficientSet"}), \\
& \quad \text{DepVars}, \text{notation} = \text{jetnumbers}))))
\end{aligned}$$

$$\text{ANS} := \{0\}$$

(3)

```

> fvec2 := { } :for i to 4 do for j from (i + 1) to 4 do fvec2 := {op(fvec2), evalDG(D_x||i
    &t D_x||j)} :od:od:
fvec4 := { } :for i to nops(fvec2) do for j from i to nops(fvec2) do fvec4 := {op(fvec4),
    evalDG(fvec2[i] &t fvec2[j])} :od:od:
for i to nops(fvec4) do:
A||i := simplify(subs(SS, ToJet(ContractIndices(W, fvec4[i], [[1, 1], [2, 2], [3, 3], [4, 4]]),
    DepVars, notation = jetnumbers))) :
B||i := simplify(subs(SS, ToJet(ContractIndices(Wst, fvec4[i], [[1, 1], [2, 2], [3, 3], [4, 4]]),
    DepVars, notation = jetnumbers))) :
ANS||i := simplify(factor(A||i) - factor(B||i)) :od:
ANS := {seq(ANS||i, i = 1..nops(fvec4))}
ANS := {0}

```

(4)

>

Type [2,1,1]

```

> F := u1 v2 - u2 v1 + v1 v2 : H := u1 v4 - u4 v1 + v1 v3 :
> DR := (diff(F, u1)·ξ1 + diff(F, u2)·ξ2 + diff(F, u3)·ξ3 + diff(F, u4)·ξ4)·(diff(H, v1)·ξ1
    + diff(H, v2)·ξ2 + diff(H, v3)·ξ3 + diff(H, v4)·ξ4) - (diff(F, v1)·ξ1 + diff(F, v2)·ξ2
    + diff(F, v3)·ξ3 + diff(F, v4)·ξ4)·(diff(H, u1)·ξ1 + diff(H, u2)·ξ2 + diff(H, u3)·ξ3
    + diff(H, u4)·ξ4) :
GA := Matrix([ [diff(DR, ξ1, ξ1), diff(DR, ξ1, ξ2), diff(DR, ξ1, ξ3), diff(DR, ξ1, ξ4)],
    [diff(DR, ξ1, ξ2), diff(DR, ξ2, ξ2), diff(DR, ξ2, ξ3), diff(DR, ξ2, ξ4)], [diff(DR, ξ1,
    ξ3), diff(DR, ξ2, ξ3), diff(DR, ξ3, ξ3), diff(DR, ξ3, ξ4)], [diff(DR, ξ1, ξ4), diff(DR, ξ2,
    ξ4), diff(DR, ξ3, ξ4), diff(DR, ξ4, ξ4)]) :
AA := FromJet(GA, DepVars) : Ai := MatrixInverse(AA) :
g := evalDG(add(add(Ai[i, j]·dx||i &t dx||j, i = 1..4), j = 1..4)) : gInv
    := evalDG(add(add(AA[i, j]·D_x||i &t D_x||j, i = 1..4), j = 1..4)) :
> DGsetup([x1, x2, x3, x4], [u, v], E, 3) :
unkn0 := {u1, v3} : contr0 := {F, H} : unkn := unkn0 : contr := contr0 :for i to 4 do unkn
    := {op(unkn), TotalDiff(unkn0[1], i), TotalDiff(unkn0[2], i)} : contr := {op(contr),
    TotalDiff(contr0[1], i), TotalDiff(contr0[2], i)} :for j to i do unkn := {op(unkn),
    TotalDiff(unkn0[1], [i, j]), TotalDiff(unkn0[2], [i, j])} : contr := {op(contr),
    TotalDiff(contr0[1], [i, j]), TotalDiff(contr0[2], [i, j])} :od:od: SS := solve(contr,
    unkn) :
> ChangeFrame(M) :
W := simplify(WeylTensor(g)) : gI2 := evalDG(gInv &t gInv) : tmp := ContractIndices(gI2,
    W, [[1, 1], [3, 2]]) :
> densV := simplify(sqrt(Determinant(Ai))) assuming ∂/∂x1 u(x1, x2, x3, x4) > 0, ∂/∂x1 v(x1,
    x2, x3, x4) > 0, 2 (∂/∂x2 v(x1, x2, x3, x4)) (∂/∂x1 v(x1, x2, x3, x4)) + (∂/∂x2 v(x1, x2,
    x3, x4)) (∂/∂x1 u(x1, x2, x3, x4)) - (∂/∂x1 v(x1, x2, x3, x4)) (∂/∂x2 u(x1, x2, x3, x4))
    > 0;

```

$$densV := 1 / \left( \left( 2 \left( \frac{\partial}{\partial x1} v(x1, x2, x3, x4) \right) \left( \frac{\partial}{\partial x2} v(x1, x2, x3, x4) \right) + \left( \frac{\partial}{\partial x1} u(x1, x2, x3, x4) \right) \left( \frac{\partial}{\partial x2} v(x1, x2, x3, x4) \right) - \left( \frac{\partial}{\partial x1} v(x1, x2, x3, x4) \right) \left( \frac{\partial}{\partial x2} u(x1, x2, x3, x4) \right) \right) \left( \frac{\partial}{\partial x1} v(x1, x2, x3, x4) \right)^2 \right) \quad (5)$$

>  $V := evalDG(densV \cdot dx1 \&w dx2 \&w dx3 \&w dx4) :$

>  $Wst := evalDG\left(\frac{1}{2} \cdot ContractIndices(W, tmp, [[3, 1], [4, 2]])\right) :$

$A := simplify(subs(SS, ToJet(ContractIndices(W, evalDG(D\_x1 \&t D\_x2 \&t D\_x3 \&t D\_x4), [[1, 1], [2, 2], [3, 3], [4, 4]]), DepVars, notation = jetnumbers))) ;$

$B := simplify(subs(SS, ToJet(ContractIndices(Wst, evalDG(D\_x1 \&t D\_x2 \&t D\_x3 \&t D\_x4), [[1, 1], [2, 2], [3, 3], [4, 4]]), DepVars, notation = jetnumbers))) ;$

$simplify(A - B)$

$$A := -\frac{1}{4} \frac{1}{v_1^4 v_2^3} \left( 2 v_1^2 v_2^2 v_{1,2,4} - v_1^2 v_2 v_4 v_{1,2,2} - 2 v_1^2 v_2 v_{1,2} v_{2,4} + v_1^2 v_4 v_{1,2} v_{2,2} - v_1 v_2^2 v_4 v_{1,1,2} - 2 v_1 v_2^2 v_{1,2} v_{1,4} + 2 v_1 v_2 v_4 v_{1,2}^2 + v_2^2 v_4 v_{1,1} v_{1,2} \right)$$

$$B := -\frac{1}{4} \frac{1}{v_1^4 v_2^3} \left( 2 v_1^2 v_2^2 v_{1,2,4} - v_1^2 v_2 v_4 v_{1,2,2} - 2 v_1^2 v_2 v_{1,2} v_{2,4} + v_1^2 v_4 v_{1,2} v_{2,2} - v_1 v_2^2 v_4 v_{1,1,2} - 2 v_1 v_2^2 v_{1,2} v_{1,4} + 2 v_1 v_2 v_4 v_{1,2}^2 + v_2^2 v_4 v_{1,1} v_{1,2} \right)$$

0

(6)

> #  $ANS := simplify(expand(subs(SS, ToJet(DGinfo(evalDG(W - Wst), "CoefficientSet"), DepVars, notation = jetnumbers))))$

>  $fvec2 := \{ \} : \text{for } i \text{ to } 4 \text{ do for } j \text{ from } (i + 1) \text{ to } 4 \text{ do } fvec2 := \{ op(fvec2), evalDG(D\_x || i \&t D\_x || j) \} : \text{od:od:}$

$fvec4 := \{ \} : \text{for } i \text{ to } nops(fvec2) \text{ do for } j \text{ from } i \text{ to } nops(fvec2) \text{ do } fvec4 := \{ op(fvec4), evalDG(fvec2[i] \&t fvec2[j]) \} : \text{od:od:}$

**for**  $i$  **to**  $nops(fvec4)$  **do:**

$A || i := simplify(subs(SS, ToJet(ContractIndices(W, fvec4[i], [[1, 1], [2, 2], [3, 3], [4, 4]]), DepVars, notation = jetnumbers))) :$

$B || i := simplify(subs(SS, ToJet(ContractIndices(Wst, fvec4[i], [[1, 1], [2, 2], [3, 3], [4, 4]]), DepVars, notation = jetnumbers))) :$

$ANS || i := simplify(factor(A || i) - factor(B || i)) : \text{od:}$

$ANS := \{ seq(ANS || i, i = 1 .. nops(fvec4)) \}$

$ANS := \{ 0 \}$

(7)

>

Type [2,2]

>  $F := u_1 v_2 - u_2 v_1 + v_1^2 : H := u_1 v_4 - u_4 v_1 + v_1 v_3 :$

>  $DR := (diff(F, u_1) \cdot \xi_1 + diff(F, u_2) \cdot \xi_2 + diff(F, u_3) \cdot \xi_3 + diff(F, u_4) \cdot \xi_4) \cdot (diff(H, v_1) \cdot \xi_1 + diff(H, v_2) \cdot \xi_2 + diff(H, v_3) \cdot \xi_3 + diff(H, v_4) \cdot \xi_4) - (diff(F, v_1) \cdot \xi_1 + diff(F, v_2) \cdot \xi_2$

$$+ \text{diff}(F, v_3) \cdot \xi_3 + \text{diff}(F, v_4) \cdot \xi_4) \cdot (\text{diff}(H, u_1) \cdot \xi_1 + \text{diff}(H, u_2) \cdot \xi_2 + \text{diff}(H, u_3) \cdot \xi_3 + \text{diff}(H, u_4) \cdot \xi_4) :$$

$$GA := \text{Matrix}([[\text{diff}(DR, \xi_1, \xi_1), \text{diff}(DR, \xi_1, \xi_2), \text{diff}(DR, \xi_1, \xi_3), \text{diff}(DR, \xi_1, \xi_4)], [\text{diff}(DR, \xi_1, \xi_2), \text{diff}(DR, \xi_2, \xi_2), \text{diff}(DR, \xi_2, \xi_3), \text{diff}(DR, \xi_2, \xi_4)], [\text{diff}(DR, \xi_1, \xi_3), \text{diff}(DR, \xi_2, \xi_3), \text{diff}(DR, \xi_3, \xi_3), \text{diff}(DR, \xi_3, \xi_4)], [\text{diff}(DR, \xi_1, \xi_4), \text{diff}(DR, \xi_2, \xi_4), \text{diff}(DR, \xi_3, \xi_4), \text{diff}(DR, \xi_4, \xi_4)]]]) :$$

$$AA := \text{FromJet}(GA, \text{DepVars}) : Ai := \text{MatrixInverse}(AA) :$$

$$g := \text{evalDG}(\text{add}(\text{add}(Ai[i, j] \cdot dx || i \& t \, dx || j, i = 1..4), j = 1..4)) : gInv := \text{evalDG}(\text{add}(\text{add}(AA[i, j] \cdot D\_x || i \& t \, D\_x || j, i = 1..4), j = 1..4)) :$$

$$> \text{DGsetup}([x1, x2, x3, x4], [u, v], E, 3) :$$

$$\text{unkn0} := \{u_1, v_3\} : \text{contr0} := \{F, H\} : \text{unkn} := \text{unkn0} : \text{contr} := \text{contr0} : \text{for } i \text{ to } 4 \text{ do } \text{unkn} := \{\text{op}(\text{unkn}), \text{TotalDiff}(\text{unkn0}[1], i), \text{TotalDiff}(\text{unkn0}[2], i)\} : \text{contr} := \{\text{op}(\text{contr}), \text{TotalDiff}(\text{contr0}[1], i), \text{TotalDiff}(\text{contr0}[2], i)\} : \text{for } j \text{ to } i \text{ do } \text{unkn} := \{\text{op}(\text{unkn}), \text{TotalDiff}(\text{unkn0}[1], [i, j]), \text{TotalDiff}(\text{unkn0}[2], [i, j])\} : \text{contr} := \{\text{op}(\text{contr}), \text{TotalDiff}(\text{contr0}[1], [i, j]), \text{TotalDiff}(\text{contr0}[2], [i, j])\} : \text{od} : \text{od} : SS := \text{solve}(\text{contr}, \text{unkn}) :$$

$$> \text{ChangeFrame}(M) :$$

$$W := \text{simplify}(\text{WeylTensor}(g)) : gI2 := \text{evalDG}(gInv \& t \, gInv) : tmp := \text{ContractIndices}(gI2, W, [[1, 1], [3, 2]]) :$$

$$> \text{densV} := \text{simplify}(\text{sqrt}(\text{Determinant}(Ai))) \text{ assuming } \frac{\partial}{\partial x1} u(x1, x2, x3, x4) > 0, \frac{\partial}{\partial x1} v(x1, x2, x3, x4) > 0, \left( \frac{\partial}{\partial x2} v(x1, x2, x3, x4) \right) \left( \frac{\partial}{\partial x1} u(x1, x2, x3, x4) \right) + 2 \left( \frac{\partial}{\partial x1} v(x1, x2, x3, x4) \right)^2 - \left( \frac{\partial}{\partial x1} v(x1, x2, x3, x4) \right) \left( \frac{\partial}{\partial x2} u(x1, x2, x3, x4) \right) > 0;$$

$$\text{densV} := 1 / \left( \left( \left( \frac{\partial}{\partial x1} u(x1, x2, x3, x4) \right) \left( \frac{\partial}{\partial x2} v(x1, x2, x3, x4) \right) - \left( \frac{\partial}{\partial x1} v(x1, x2, x3, x4) \right) \left( \frac{\partial}{\partial x2} u(x1, x2, x3, x4) \right) + 2 \left( \frac{\partial}{\partial x1} v(x1, x2, x3, x4) \right)^2 \right) \left( \frac{\partial}{\partial x1} v(x1, x2, x3, x4) \right)^2 \right) \quad (8)$$

$$> V := \text{evalDG}(\text{densV} \cdot dx1 \& w \, dx2 \& w \, dx3 \& w \, dx4) :$$

$$> Wst := \text{evalDG} \left( \frac{1}{2} \cdot \text{ContractIndices}(V, tmp, [[3, 1], [4, 2]]) \right) :$$

$$A := \text{simplify}(\text{subs}(SS, \text{ToJet}(\text{ContractIndices}(W, \text{evalDG}(D\_x1 \& t \, D\_x2 \& t \, D\_x3 \& t \, D\_x4), [[1, 1], [2, 2], [3, 3], [4, 4]]), \text{DepVars}, \text{notation} = \text{jetnumbers}))) :$$

$$B := \text{simplify}(\text{subs}(SS, \text{ToJet}(\text{ContractIndices}(Wst, \text{evalDG}(D\_x1 \& t \, D\_x2 \& t \, D\_x3 \& t \, D\_x4), [[1, 1], [2, 2], [3, 3], [4, 4]]), \text{DepVars}, \text{notation} = \text{jetnumbers}))) :$$

$$\text{simplify}(A - B)$$

$$A := -\frac{1}{2} \frac{v_1^2 v_{1,1,4} - v_1 v_4 v_{1,1,1} - 2 v_1 v_{1,1} v_{1,4} + 2 v_4 v_{1,1}^2}{v_1^5}$$

$$B := -\frac{1}{2} \frac{v_1^2 v_{1,1,4} - v_1 v_4 v_{1,1,1} - 2 v_1 v_{1,1} v_{1,4} + 2 v_4 v_{1,1}^2}{v_1^5}$$

0

(9)

```

> fvec2 := { } :for i to 4 do for j from (i + 1) to 4 do fvec2 := {op(fvec2), evalDG(D_x||i
    &t D_x||j)} :od:od:
fvec4 := { } :for i to nops(fvec2) do for j from i to nops(fvec2) do fvec4 := {op(fvec4),
    evalDG(fvec2[i] &t fvec2[j])} :od:od:
for i to nops(fvec4) do:
A||i := simplify(subs(SS, ToJet(ContractIndices(W, fvec4[i], [[1, 1], [2, 2], [3, 3], [4, 4]]),
    DepVars, notation = jetnumbers))) :
B||i := simplify(subs(SS, ToJet(ContractIndices(Wst, fvec4[i], [[1, 1], [2, 2], [3, 3], [4, 4]]),
    DepVars, notation = jetnumbers))) :
ANS||i := simplify(factor(A||i) - factor(B||i)) :od:
ANS := {seq(ANS||i, i = 1..nops(fvec4))}
ANS := {0}

```

(10)

>

Type [3,1]

```

> F := u_2 + v_1 v_2 : H := u_4 - v_3 + v_1 v_4 :
> DR := (diff(F, u_1)·ξ_1 + diff(F, u_2)·ξ_2 + diff(F, u_3)·ξ_3 + diff(F, u_4)·ξ_4)·(diff(H, v_1)·ξ_1
    + diff(H, v_2)·ξ_2 + diff(H, v_3)·ξ_3 + diff(H, v_4)·ξ_4) - (diff(F, v_1)·ξ_1 + diff(F, v_2)·ξ_2
    + diff(F, v_3)·ξ_3 + diff(F, v_4)·ξ_4)·(diff(H, u_1)·ξ_1 + diff(H, u_2)·ξ_2 + diff(H, u_3)·ξ_3
    + diff(H, u_4)·ξ_4) :
GA := Matrix([ [diff(DR, ξ_1, ξ_1), diff(DR, ξ_1, ξ_2), diff(DR, ξ_1, ξ_3), diff(DR, ξ_1, ξ_4)],
    [diff(DR, ξ_1, ξ_2), diff(DR, ξ_2, ξ_2), diff(DR, ξ_2, ξ_3), diff(DR, ξ_2, ξ_4)], [diff(DR, ξ_1,
    ξ_3), diff(DR, ξ_2, ξ_3), diff(DR, ξ_3, ξ_3), diff(DR, ξ_3, ξ_4)], [diff(DR, ξ_1, ξ_4), diff(DR, ξ_2,
    ξ_4), diff(DR, ξ_3, ξ_4), diff(DR, ξ_4, ξ_4)] ] ) :
AA := FromJet(GA, DepVars) : Ai := MatrixInverse(AA) :
g := evalDG(add(add(Ai[i, j]·dx||i &t dx||j, i = 1..4), j = 1..4)) : gInv
    := evalDG(add(add(AA[i, j]·D_x||i &t D_x||j, i = 1..4), j = 1..4)) :
> DGsetup([x1, x2, x3, x4], [u, v], E, 3) :
unkn0 := {u_2, v_3} : contr0 := {F, H} : unkn := unkn0 : contr := contr0 :for i to 4 do unkn
    := {op(unkn), TotalDiff(unkn0[1], i), TotalDiff(unkn0[2], i)} : contr := {op(contr),
    TotalDiff(contr0[1], i), TotalDiff(contr0[2], i)} :for j to i do unkn := {op(unkn),
    TotalDiff(unkn0[1], [i, j]), TotalDiff(unkn0[2], [i, j])} : contr := {op(contr),
    TotalDiff(contr0[1], [i, j]), TotalDiff(contr0[2], [i, j])} :od:od: SS := solve(contr,
    unkn) :
> ChangeFrame(M) :
W := simplify(WeylTensor(g)) : gI2 := evalDG(gInv &t gInv) : tmp := ContractIndices(gI2,
    W, [[1, 1], [3, 2]]) :

```

```

> densV := simplify(sqrt(Determinant(Ai))) assuming ∂/∂x2 v(x1, x2, x3, x4) < 0;

```

$$densV := - \frac{1}{\frac{\partial}{\partial x_2} v(x_1, x_2, x_3, x_4)} \quad (11)$$

```

> V := evalDG(densV·dx1 &w dx2 &w dx3 &w dx4) :
> Wst := evalDG( (1/2)·ContractIndices(V, tmp, [[3, 1], [4, 2]]) ) :
A := simplify(subs(SS, ToJet(ContractIndices(W, evalDG(D_x1 &t D_x2 &t D_x3 &t D_x4),
  [[1, 1], [2, 2], [3, 3], [4, 4]]), DepVars, notation = jetnumbers))) ;
B := simplify(subs(SS, ToJet(ContractIndices(Wst, evalDG(D_x1 &t D_x2 &t D_x3 &t D_x4),
  [[1, 1], [2, 2], [3, 3], [4, 4]]), DepVars, notation = jetnumbers))) ;
simplify(A - B)

```

$$A := -\frac{1}{4} \frac{2 v_2^2 v_{1,2,4} - v_2 v_4 v_{1,2,2} - 2 v_2 v_{1,2} v_{2,4} + v_4 v_{1,2} v_{2,2}}{v_2^3}$$

$$B := -\frac{1}{4} \frac{2 v_2^2 v_{1,2,4} - v_2 v_4 v_{1,2,2} - 2 v_2 v_{1,2} v_{2,4} + v_4 v_{1,2} v_{2,2}}{v_2^3}$$

0 (12)

```

> fvec2 := { } :for i to 4 do for j from (i + 1) to 4 do fvec2 := {op(fvec2), evalDG(D_x||i
  &t D_x||j)} :od:od:
fvec4 := { } : for i to nops(fvec2) do for j from i to nops(fvec2) do fvec4 := {op(fvec4),
  evalDG(fvec2[i] &t fvec2[j])} :od:od:
for i to nops(fvec4) do:
A||i := simplify(subs(SS, ToJet(ContractIndices(W, fvec4[i], [[1, 1], [2, 2], [3, 3], [4, 4]]),
  DepVars, notation = jetnumbers))) :
B||i := simplify(subs(SS, ToJet(ContractIndices(Wst, fvec4[i], [[1, 1], [2, 2], [3, 3], [4, 4]]),
  DepVars, notation = jetnumbers))) :
ANS||i := simplify(factor(A||i) - factor(B||i)) :od:
ANS := {seq(ANS||i, i = 1..nops(fvec4))}

```

ANS := {0} (13)

>  
Type [4]

```

> F := u1 - v2 + v12 : H := u4 - v3 + v1·v4 :
> DR := (diff(F, u1)·ξ1 + diff(F, u2)·ξ2 + diff(F, u3)·ξ3 + diff(F, u4)·ξ4)·(diff(H, v1)·ξ1
  + diff(H, v2)·ξ2 + diff(H, v3)·ξ3 + diff(H, v4)·ξ4) - (diff(F, v1)·ξ1 + diff(F, v2)·ξ2
  + diff(F, v3)·ξ3 + diff(F, v4)·ξ4)·(diff(H, u1)·ξ1 + diff(H, u2)·ξ2 + diff(H, u3)·ξ3
  + diff(H, u4)·ξ4) :
GA := Matrix( [ [diff(DR, ξ1, ξ1), diff(DR, ξ1, ξ2), diff(DR, ξ1, ξ3), diff(DR, ξ1, ξ4)],
  [diff(DR, ξ1, ξ2), diff(DR, ξ2, ξ2), diff(DR, ξ2, ξ3), diff(DR, ξ2, ξ4)], [diff(DR, ξ1,
  ξ3), diff(DR, ξ2, ξ3), diff(DR, ξ3, ξ3), diff(DR, ξ3, ξ4)], [diff(DR, ξ1, ξ4), diff(DR, ξ2,
  ξ4), diff(DR, ξ3, ξ4), diff(DR, ξ4, ξ4) ] ] ) :

```

```

AA := FromJet(GA, DepVars) : Ai := MatrixInverse(AA) :
g := evalDG(add(add(Ai[i,j]·dx||i &t dx||j, i = 1..4), j = 1..4)) : gInv
:= evalDG(add(add(AA[i,j]·D_x||i &t D_x||j, i = 1..4), j = 1..4)) :
> DGsetup([x1, x2, x3, x4], [u, v], E, 3) :
unkn0 := {u1, v3} : contr0 := {F, H} : unkn := unkn0 : contr := contr0 :for i to 4 do unkn
:= {op(unkn), TotalDiff(unkn0[1], i), TotalDiff(unkn0[2], i)} : contr := {op(contr),
TotalDiff(contr0[1], i), TotalDiff(contr0[2], i)} :for j to i do unkn := {op(unkn),
TotalDiff(unkn0[1], [i, j]), TotalDiff(unkn0[2], [i, j])} : contr := {op(contr),
TotalDiff(contr0[1], [i, j]), TotalDiff(contr0[2], [i, j])} :od:od: SS := solve(contr,
unkn) :
> ChangeFrame(M) :
W := simplify(WeylTensor(g)) : gI2 := evalDG(gInv &t gInv) : tmp := ContractIndices(gI2,
W, [[1, 1], [3, 2]]) :
> densV := simplify(sqrt(Determinant(Ai))) assuming  $\frac{\partial}{\partial x1} u(x1, x2, x3, x4) > 0$ ;
densV := 1
(14)

```

```

> V := evalDG(densV·dx1 &w dx2 &w dx3 &w dx4) :
> Wst := evalDG( $\frac{1}{2}$ ·ContractIndices(V, tmp, [[3, 1], [4, 2]])) :
A := simplify(subs(SS, ToJet(ContractIndices(W, evalDG(D_x1 &t D_x2 &t D_x3 &t D_x4),
[[1, 1], [2, 2], [3, 3], [4, 4]]), DepVars, notation = jetnumbers))) :
B := simplify(subs(SS, ToJet(ContractIndices(Wst, evalDG(D_x1 &t D_x2 &t D_x3 &t D_x4),
[[1, 1], [2, 2], [3, 3], [4, 4]]), DepVars, notation = jetnumbers))) :
simplify(A + B)
A := - $\frac{1}{2} v_{1,1,4}$ 
B :=  $\frac{1}{2} v_{1,1,4}$ 
0
(15)

```

```

> fvec2 := {} :for i to 4 do for j from (i + 1) to 4 do fvec2 := {op(fvec2), evalDG(D_x||i
&t D_x||j)} :od:od:
fvec4 := {} :for i to nops(fvec2) do for j from i to nops(fvec2) do fvec4 := {op(fvec4),
evalDG(fvec2[i] &t fvec2[j])} :od:od:
for i to nops(fvec4) do:
A||i := simplify(subs(SS, ToJet(ContractIndices(W, fvec4[i], [[1, 1], [2, 2], [3, 3], [4, 4]]),
DepVars, notation = jetnumbers)))) :
B||i := simplify(subs(SS, ToJet(ContractIndices(Wst, fvec4[i], [[1, 1], [2, 2], [3, 3], [4, 4]]),
DepVars, notation = jetnumbers)))) :
ANS||i := simplify(factor(A||i) + factor(B||i)) :od:
ANS := {seq(ANS||i, i = 1..nops(fvec4))}
ANS := {0}
(16)

```

```

>
Type [1,1,1]

```

```

> F :=  $u_3 v_1 - \alpha \cdot (v_2 - v_3) \cdot u_1$  : H :=  $u_4 v_1 - \alpha \cdot (v_3 - v_4) \cdot u_1$  :

```



>  $DR := (diff(F, u_1) \cdot \xi_1 + diff(F, u_2) \cdot \xi_2 + diff(F, u_3) \cdot \xi_3 + diff(F, u_4) \cdot \xi_4) \cdot (diff(H, v_1) \cdot \xi_1 + diff(H, v_2) \cdot \xi_2 + diff(H, v_3) \cdot \xi_3 + diff(H, v_4) \cdot \xi_4) - (diff(F, v_1) \cdot \xi_1 + diff(F, v_2) \cdot \xi_2 + diff(F, v_3) \cdot \xi_3 + diff(F, v_4) \cdot \xi_4) \cdot (diff(H, u_1) \cdot \xi_1 + diff(H, u_2) \cdot \xi_2 + diff(H, u_3) \cdot \xi_3 + diff(H, u_4) \cdot \xi_4) :$

$GA := Matrix([ [diff(DR, \xi_1, \xi_1), diff(DR, \xi_1, \xi_2), diff(DR, \xi_1, \xi_3), diff(DR, \xi_1, \xi_4)], [diff(DR, \xi_1, \xi_2), diff(DR, \xi_2, \xi_2), diff(DR, \xi_2, \xi_3), diff(DR, \xi_2, \xi_4)], [diff(DR, \xi_1, \xi_3), diff(DR, \xi_2, \xi_3), diff(DR, \xi_3, \xi_3), diff(DR, \xi_3, \xi_4)], [diff(DR, \xi_1, \xi_4), diff(DR, \xi_2, \xi_4), diff(DR, \xi_3, \xi_4), diff(DR, \xi_4, \xi_4)] ] ) :$

$AA := FromJet(GA, DepVars) : Ai := simplify(Determinant(AA) \cdot MatrixInverse(AA)) :$

$g := evalDG(add(add(Ai[i, j] \cdot dx || i \&t dx || j, i = 1..4), j = 1..4)) : gInv := simplify(evalDG( \frac{1}{Determinant(AA)} add(add(AA[i, j] \cdot D_x || i \&t D_x || j, i = 1..4), j = 1..4) )) :$

>  $DGsetup([x1, x2, x3, x4], [u, v], E, 3) :$   
 $unkn0 := \{u_3, v_3\} : contr0 := \{F, H\} : unkn := unkn0 : contr := contr0 : \text{for } i \text{ to } 4 \text{ do } unkn := \{op(unkn), TotalDiff(unkn0[1], i), TotalDiff(unkn0[2], i)\} : contr := \{op(contr), TotalDiff(contr0[1], i), TotalDiff(contr0[2], i)\} : \text{for } j \text{ to } i \text{ do } unkn := \{op(unkn), TotalDiff(unkn0[1], [i, j]), TotalDiff(unkn0[2], [i, j])\} : contr := \{op(contr), TotalDiff(contr0[1], [i, j]), TotalDiff(contr0[2], [i, j])\} : \text{od} : SS := solve(contr, unkn) :$

>  $ChangeFrame(M) :$   
 $W := simplify(WeylTensor(g)) : gI2 := evalDG(gInv \&t gInv) : tmp := ContractIndices(gI2, W, [[1, 1], [3, 2]]) :$

>  $densV := simplify(sqrt(Determinant(Ai))) \text{ assuming } \frac{\partial}{\partial x1} u(x1, x2, x3, x4) > 0, \frac{\partial}{\partial x1} v(x1, x2, x3, x4) > 0, 2 \alpha^2 \left( \frac{\partial}{\partial x1} u(x1, x2, x3, x4) \right) \left( \frac{\partial}{\partial x3} v(x1, x2, x3, x4) \right) - \alpha^2 \left( \frac{\partial}{\partial x1} u(x1, x2, x3, x4) \right) \left( \frac{\partial}{\partial x2} v(x1, x2, x3, x4) \right) - \alpha^2 \left( \frac{\partial}{\partial x1} u(x1, x2, x3, x4) \right) \left( \frac{\partial}{\partial x4} v(x1, x2, x3, x4) \right) + \left( \frac{\partial}{\partial x1} v(x1, x2, x3, x4) \right) \left( \frac{\partial}{\partial x4} u(x1, x2, x3, x4) \right) > 0, \alpha > 0;$

$densV := \alpha^3 \left( \frac{\partial}{\partial x1} v(x1, x2, x3, x4) \right)^3 \left( \frac{\partial}{\partial x1} u(x1, x2, x3, x4) \right)^3 \left( 2 \alpha^2 \left( \frac{\partial}{\partial x1} u(x1, x2, x3, x4) \right) \left( \frac{\partial}{\partial x3} v(x1, x2, x3, x4) \right) - \alpha^2 \left( \frac{\partial}{\partial x1} u(x1, x2, x3, x4) \right) \left( \frac{\partial}{\partial x4} v(x1, x2, x3, x4) \right) - \alpha^2 \left( \frac{\partial}{\partial x1} u(x1, x2, x3, x4) \right) \left( \frac{\partial}{\partial x2} v(x1, x2, x3, x4) \right) + \left( \frac{\partial}{\partial x1} v(x1, x2, x3, x4) \right) \left( \frac{\partial}{\partial x4} u(x1, x2, x3, x4) \right) \right)^3 \quad (17)$

>  $V := evalDG(densV \cdot dx1 \&w dx2 \&w dx3 \&w dx4) :$

>  $Wst := evalDG\left(\frac{1}{2} \cdot ContractIndices(W, tmp, [[3, 1], [4, 2]])\right) :$   
 $A := simplify(subs(SS, ToJet(ContractIndices(W, evalDG(D_{x1} \& D_{x2} \& D_{x3} \& D_{x4}),$   
 $[[1, 1], [2, 2], [3, 3], [4, 4]]), DepVars, notation = jetnumbers))) :$   
 $B := simplify(subs(SS, ToJet(ContractIndices(Wst, evalDG(D_{x1} \& D_{x2} \& D_{x3} \& D_{x4}),$   
 $[[1, 1], [2, 2], [3, 3], [4, 4]]), DepVars, notation = jetnumbers))) :$   
 $simplify(A + B)$

0

(18)

>  $fvec2 := \{ \} : \text{for } i \text{ to } 4 \text{ do for } j \text{ from } (i + 1) \text{ to } 4 \text{ do } fvec2 := \{ op(fvec2), evalDG(D_{x||i}$   
 $\& D_{x||j}) \} : \text{od:od:}$   
 $fvec4 := \{ \} : \text{for } i \text{ to } nops(fvec2) \text{ do for } j \text{ from } i \text{ to } nops(fvec2) \text{ do } fvec4 := \{ op(fvec4),$   
 $evalDG(fvec2[i] \& fvec2[j]) \} : \text{od:od:}$   
 $\text{for } i \text{ to } nops(fvec4) \text{ do:}$   
 $A||i := simplify(subs(SS, ToJet(ContractIndices(W, fvec4[i], [[1, 1], [2, 2], [3, 3], [4, 4]]),$   
 $DepVars, notation = jetnumbers))) :$   
 $B||i := simplify(subs(SS, ToJet(ContractIndices(Wst, fvec4[i], [[1, 1], [2, 2], [3, 3], [4, 4]]),$   
 $DepVars, notation = jetnumbers))) :$   
 $ANS||i := simplify(factor(A||i) + factor(B||i)) : \text{od:}$   
 $ANS := \{ seq(ANS||i, i = 1 .. nops(fvec4)) \}$   
 $ANS := \{ 0 \}$

(19)

>  
Type [2,1]

>  $F := u_3 v_1 - u_1 v_3 - (v_2 - \alpha \cdot v_3) v_1 : H := u_4 v_1 - u_1 v_4 - (v_3 - \alpha \cdot v_4) v_1 :$   
>  $DR := (diff(F, u_1) \cdot \xi_1 + diff(F, u_2) \cdot \xi_2 + diff(F, u_3) \cdot \xi_3 + diff(F, u_4) \cdot \xi_4) \cdot (diff(H, v_1) \cdot \xi_1$   
 $+ diff(H, v_2) \cdot \xi_2 + diff(H, v_3) \cdot \xi_3 + diff(H, v_4) \cdot \xi_4) - (diff(F, v_1) \cdot \xi_1 + diff(F, v_2) \cdot \xi_2$   
 $+ diff(F, v_3) \cdot \xi_3 + diff(F, v_4) \cdot \xi_4) \cdot (diff(H, u_1) \cdot \xi_1 + diff(H, u_2) \cdot \xi_2 + diff(H, u_3) \cdot \xi_3$   
 $+ diff(H, u_4) \cdot \xi_4) :$   
 $GA := Matrix\left(\left[\left[diff(DR, \xi_1, \xi_1), diff(DR, \xi_1, \xi_2), diff(DR, \xi_1, \xi_3), diff(DR, \xi_1, \xi_4)\right],\right.\right.$   
 $\left.\left[diff(DR, \xi_2, \xi_1), diff(DR, \xi_2, \xi_2), diff(DR, \xi_2, \xi_3), diff(DR, \xi_2, \xi_4)\right], \left[diff(DR, \xi_3,\right.\right.$   
 $\left.\xi_1), diff(DR, \xi_3, \xi_2), diff(DR, \xi_3, \xi_3), diff(DR, \xi_3, \xi_4)\right], \left[diff(DR, \xi_4, \xi_1),\right.$   
 $\left.\xi_2), diff(DR, \xi_4, \xi_3), diff(DR, \xi_4, \xi_4)\right]\right) :$   
 $AA := FromJet(GA, DepVars) : Ai := simplify(Determinant(AA) \cdot MatrixInverse(AA)) :$   
 $g := evalDG(add(add(Ai[i, j] \cdot dx||i \& dx||j, i = 1 .. 4), j = 1 .. 4)) : gInv$   
 $:= simplify\left(evalDG\left(\frac{1}{Determinant(AA)} add(add(AA[i, j] \cdot D_{x||i} \& D_{x||j}, i = 1 .. 4), j\right.\right.$   
 $\left.\left.= 1 .. 4)\right)\right) :$

>  $DGsetup([x1, x2, x3, x4], [u, v], E, 3) :$   
 $unkn0 := \{u_3, v_3\} : contr0 := \{F, H\} : unkn := unkn0 : contr := contr0 : \text{for } i \text{ to } 4 \text{ do } unkn$   
 $:= \{ op(unkn), TotalDiff(unkn0[1], i), TotalDiff(unkn0[2], i) \} : contr := \{ op(contr),$   
 $TotalDiff(contr0[1], i), TotalDiff(contr0[2], i) \} : \text{for } j \text{ to } i \text{ do } unkn := \{ op(unkn),$   
 $TotalDiff(unkn0[1], [i, j]), TotalDiff(unkn0[2], [i, j]) \} : contr := \{ op(contr),$

$TotalDiff(contr0[1], [i, j]), TotalDiff(contr0[2], [i, j])\} : \mathbf{od} : \mathbf{od} : SS := solve(contr, unkn) :$

>  $ChangeFrame(M) :$

$W := simplify(WeylTensor(g)) : gI2 := evalDG(gInv \& t gInv) : tmp := ContractIndices(gI2, W, [[1, 1], [3, 2]]) :$

>  $densV := simplify(sqrt(Determinant(Ai)))$  assuming  $\frac{\partial}{\partial x1} u(x1, x2, x3, x4) > 0, \frac{\partial}{\partial x1} v(x1, x2, x3, x4) > 0, \left(-2 \left(\frac{\partial}{\partial x1} v(x1, x2, x3, x4)\right) \left(\frac{\partial}{\partial x4} v(x1, x2, x3, x4)\right) \alpha + 2 \left(\frac{\partial}{\partial x1} v(x1, x2, x3, x4)\right) \left(\frac{\partial}{\partial x3} v(x1, x2, x3, x4)\right) - \left(\frac{\partial}{\partial x1} v(x1, x2, x3, x4)\right) \left(\frac{\partial}{\partial x4} u(x1, x2, x3, x4)\right) + \left(\frac{\partial}{\partial x4} v(x1, x2, x3, x4)\right) \left(\frac{\partial}{\partial x1} u(x1, x2, x3, x4)\right)\right) > 0;$

$$densV := \left(\frac{\partial}{\partial x1} v(x1, x2, x3, x4)\right)^6 \left(-2 \left(\frac{\partial}{\partial x4} v(x1, x2, x3, x4)\right) \left(\frac{\partial}{\partial x1} v(x1, x2, x3, x4)\right) \alpha + 2 \left(\frac{\partial}{\partial x1} v(x1, x2, x3, x4)\right) \left(\frac{\partial}{\partial x3} v(x1, x2, x3, x4)\right) - \left(\frac{\partial}{\partial x1} v(x1, x2, x3, x4)\right) \left(\frac{\partial}{\partial x4} u(x1, x2, x3, x4)\right) + \left(\frac{\partial}{\partial x4} v(x1, x2, x3, x4)\right) \left(\frac{\partial}{\partial x1} u(x1, x2, x3, x4)\right)\right)^3 \quad (20)$$

>  $V := evalDG(densV \cdot dx1 \& w dx2 \& w dx3 \& w dx4) :$

>  $Wst := evalDG\left(\frac{1}{2} \cdot ContractIndices(V, tmp, [[3, 1], [4, 2]])\right) :$

$A := simplify(subs(SS, ToJet(ContractIndices(W, evalDG(D_x1 \& t D_x2 \& t D_x3 \& t D_x4), [[1, 1], [2, 2], [3, 3], [4, 4]]), DepVars, notation = jetnumbers))) :$

$B := simplify(subs(SS, ToJet(ContractIndices(Wst, evalDG(D_x1 \& t D_x2 \& t D_x3 \& t D_x4), [[1, 1], [2, 2], [3, 3], [4, 4]]), DepVars, notation = jetnumbers))) :$

$simplify(A - B)$

0

(21)

>  $fvec2 := \{ \} : \mathbf{for} \ i \ \mathbf{to} \ 4 \ \mathbf{do} \ \mathbf{for} \ j \ \mathbf{from} \ (i + 1) \ \mathbf{to} \ 4 \ \mathbf{do} \ fvec2 := \{op(fvec2), evalDG(D_x || i \& t D_x || j)\} : \mathbf{od} : \mathbf{od} :$

$fvec4 := \{ \} : \mathbf{for} \ i \ \mathbf{to} \ nops(fvec2) \ \mathbf{do} \ \mathbf{for} \ j \ \mathbf{from} \ i \ \mathbf{to} \ nops(fvec2) \ \mathbf{do} \ fvec4 := \{op(fvec4), evalDG(fvec2[i] \& t fvec2[j])\} : \mathbf{od} : \mathbf{od} :$

$\mathbf{for} \ i \ \mathbf{to} \ nops(fvec4) \ \mathbf{do} :$

$A || i := simplify(subs(SS, ToJet(ContractIndices(W, fvec4[i], [[1, 1], [2, 2], [3, 3], [4, 4]]), DepVars, notation = jetnumbers))) :$

$B || i := simplify(subs(SS, ToJet(ContractIndices(Wst, fvec4[i], [[1, 1], [2, 2], [3, 3], [4, 4]]), DepVars, notation = jetnumbers))) :$

$ANS || i := simplify(factor(A || i) - factor(B || i)) : \mathbf{od} :$

$ANS := \{seq(ANS || i, i = 1 .. nops(fvec4))\}$

$ANS := \{0\}$

(22)

>

Type [3]

>  $F := u_3 - v_2 + v_1 v_3 : H := u_4 - v_3 + v_1 v_4 :$

>  $DR := (diff(F, u_1) \cdot \xi_1 + diff(F, u_2) \cdot \xi_2 + diff(F, u_3) \cdot \xi_3 + diff(F, u_4) \cdot \xi_4) \cdot (diff(H, v_1) \cdot \xi_1 + diff(H, v_2) \cdot \xi_2 + diff(H, v_3) \cdot \xi_3 + diff(H, v_4) \cdot \xi_4) - (diff(F, v_1) \cdot \xi_1 + diff(F, v_2) \cdot \xi_2 + diff(F, v_3) \cdot \xi_3 + diff(F, v_4) \cdot \xi_4) \cdot (diff(H, u_1) \cdot \xi_1 + diff(H, u_2) \cdot \xi_2 + diff(H, u_3) \cdot \xi_3 + diff(H, u_4) \cdot \xi_4) :$

$GA := Matrix([ [diff(DR, \xi_1, \xi_1), diff(DR, \xi_1, \xi_2), diff(DR, \xi_1, \xi_3), diff(DR, \xi_1, \xi_4)], [diff(DR, \xi_1, \xi_2), diff(DR, \xi_2, \xi_2), diff(DR, \xi_2, \xi_3), diff(DR, \xi_2, \xi_4)], [diff(DR, \xi_1, \xi_3), diff(DR, \xi_2, \xi_3), diff(DR, \xi_3, \xi_3), diff(DR, \xi_3, \xi_4)], [diff(DR, \xi_1, \xi_4), diff(DR, \xi_2, \xi_4), diff(DR, \xi_3, \xi_4), diff(DR, \xi_4, \xi_4)] ] ) :$

$AA := FromJet(GA, DepVars) : Ai := simplify(Determinant(AA) \cdot MatrixInverse(AA)) :$

$g := evalDG(add(add(Ai[i, j] \cdot dx || i \&t dx || j, i = 1..4), j = 1..4)) : gInv$

$:= simplify\left( evalDG\left( \frac{1}{Determinant(AA)} add(add(AA[i, j] \cdot D\_x || i \&t D\_x || j, i = 1..4), j = 1..4) \right) \right) :$

>  $DGsetup([x1, x2, x3, x4], [u, v], E, 3) :$

$unkn0 := \{u_3, v_3\} : contr0 := \{F, H\} : unkn := unkn0 : contr := contr0 : \text{for } i \text{ to } 4 \text{ do } unkn := \{op(unkn), TotalDiff(unkn0[1], i), TotalDiff(unkn0[2], i)\} : contr := \{op(contr), TotalDiff(contr0[1], i), TotalDiff(contr0[2], i)\} : \text{for } j \text{ to } i \text{ do } unkn := \{op(unkn), TotalDiff(unkn0[1], [i, j]), TotalDiff(unkn0[2], [i, j])\} : contr := \{op(contr), TotalDiff(contr0[1], [i, j]), TotalDiff(contr0[2], [i, j])\} : \text{od} : SS := solve(contr, unkn) :$

>  $ChangeFrame(M) :$

$W := simplify(WeylTensor(g)) : gI2 := evalDG(gInv \&t gInv) : tmp := ContractIndices(gI2, W, [[1, 1], [3, 2]]) :$

>  $densV := simplify(sqrt(Determinant(Ai))) \text{ assuming } \frac{\partial}{\partial x1} u(x1, x2, x3, x4) > 0, \frac{\partial}{\partial x1} v(x1, x2, x3, x4) > 0, \frac{\partial}{\partial x4} v(x1, x2, x3, x4) > 0 ;$

$$densV := \left( \frac{\partial}{\partial x4} v(x1, x2, x3, x4) \right)^3 \quad (23)$$

>  $V := evalDG(densV \cdot dx1 \&w dx2 \&w dx3 \&w dx4) :$

>  $Wst := evalDG\left( \frac{1}{2} \cdot ContractIndices(V, tmp, [[3, 1], [4, 2]]) \right) :$

$A := simplify(subs(SS, ToJet(ContractIndices(W, evalDG(D\_x1 \&t D\_x2 \&t D\_x3 \&t D\_x4), [[1, 1], [2, 2], [3, 3], [4, 4]]), DepVars, notation = jetnumbers))) :$

$B := simplify(subs(SS, ToJet(ContractIndices(Wst, evalDG(D\_x1 \&t D\_x2 \&t D\_x3 \&t D\_x4), [[1, 1], [2, 2], [3, 3], [4, 4]]), DepVars, notation = jetnumbers))) : simplify(A + B)$

0

(24)

>  $fvec2 := \{ \} : \text{for } i \text{ to } 4 \text{ do for } j \text{ from } (i + 1) \text{ to } 4 \text{ do } fvec2 := \{op(fvec2), evalDG(D\_x || i \&t D\_x || j)\} : \text{od} : \text{od} : fvec4 := \{ \} : \text{for } i \text{ to } nops(fvec2) \text{ do for } j \text{ from } i \text{ to } nops(fvec2) \text{ do } fvec4 := \{op(fvec4),$

```

    evalDG(fvec2[i] &t fvec2[j])) :od:od:
for i to nops(fvec4) do:
A||i := simplify(subs(SS, ToJet(ContractIndices(W, fvec4[i], [[1, 1], [2, 2], [3, 3], [4, 4]]),
    DepVars, notation = jetnumbers))) :
B||i := simplify(subs(SS, ToJet(ContractIndices(Wst, fvec4[i], [[1, 1], [2, 2], [3, 3], [4, 4]]),
    DepVars, notation = jetnumbers))) :
ANS||i := simplify(factor(A||i) + factor(B||i)) :od:
ANS := {seq(ANS||i, i = 1..nops(fvec4))}
ANS := {0}

```

(25)

>

Type [1,1]

```

> F := u2 v3 - u3 v2 - u2 v2 + u3 v1 : H := u2 v4 - u4 v2 - u2 v3 + u4 v1 :
> DR := (diff(F, u1)·ξ1 + diff(F, u2)·ξ2 + diff(F, u3)·ξ3 + diff(F, u4)·ξ4)·(diff(H, v1)·ξ1
+ diff(H, v2)·ξ2 + diff(H, v3)·ξ3 + diff(H, v4)·ξ4) - (diff(F, v1)·ξ1 + diff(F, v2)·ξ2
+ diff(F, v3)·ξ3 + diff(F, v4)·ξ4)·(diff(H, u1)·ξ1 + diff(H, u2)·ξ2 + diff(H, u3)·ξ3
+ diff(H, u4)·ξ4) :
GA := Matrix([ [diff(DR, ξ1, ξ1), diff(DR, ξ1, ξ2), diff(DR, ξ1, ξ3), diff(DR, ξ1, ξ4)],
[diff(DR, ξ1, ξ2), diff(DR, ξ2, ξ2), diff(DR, ξ2, ξ3), diff(DR, ξ2, ξ4)], [diff(DR, ξ1,
ξ3), diff(DR, ξ2, ξ3), diff(DR, ξ3, ξ3), diff(DR, ξ3, ξ4)], [diff(DR, ξ1, ξ4), diff(DR, ξ2,
ξ4), diff(DR, ξ3, ξ4), diff(DR, ξ4, ξ4)] ] ) :
Ga := factor(simplify( (u2 (v1 - v2) / Determinant(GA)) · GA )) : Gi := factor(simplify( (Determinant(GA) /
u2 (v1 - v2) )
· MatrixInverse(GA) )) :
Aa := FromJet(Ga, DepVars) : Ai := FromJet(Gi, DepVars) :
g := evalDG(add(add(Ai[i, j]·dx||i &t dx||j, i = 1..4), j = 1..4)) : gInv
:= simplify(evalDG(add(add(Aa[i, j]·D_x||i &t D_x||j, i = 1..4), j = 1..4))) :
> DGsetup([x1, x2, x3, x4], [u, v], E, 3) :
unkn0 := {u3, v3} : contr0 := {F, H} : unkn := unkn0 : contr := contr0 : for i to 4 do unkn
:= {op(unkn), TotalDiff(unkn0[1], i), TotalDiff(unkn0[2], i)} : contr := {op(contr),
TotalDiff(contr0[1], i), TotalDiff(contr0[2], i)} : for j to i do unkn := {op(unkn),
TotalDiff(unkn0[1], [i, j]), TotalDiff(unkn0[2], [i, j])} : contr := {op(contr),
TotalDiff(contr0[1], [i, j]), TotalDiff(contr0[2], [i, j])} :od:od: SS := solve(contr,
unkn) :
> ChangeFrame(M) :
W := WeylTensor(g) :
Error, (in PDEtools/NumerDenom) too many levels of recursion
> gI2 := evalDG(gInv &t gInv) : tmp := ContractIndices(gI2, W, [[1, 1], [3, 2]]) :
> densV := simplify(sqrt(Determinant(Ai))) assuming ∂/∂x1 u(x1, x2, x3, x4) > 0, ∂/∂x1 v(x1,
x2, x3, x4) > 0, ∂/∂x4 v(x1, x2, x3, x4) > 0;

```

```

> V := evalDG(densV·dx1 &w dx2 &w dx3 &w dx4) :
> Wst := evalDG( (1/2 · ContractIndices(V, tmp, [[3, 1], [4, 2]])) :
A := simplify(subs(SS, ToJet(ContractIndices(W, evalDG(D_x1 &t D_x2 &t D_x3 &t D_x4),
  [[1, 1], [2, 2], [3, 3], [4, 4]]), DepVars, notation = jetnumbers))) :
B := simplify(subs(SS, ToJet(ContractIndices(Wst, evalDG(D_x1 &t D_x2 &t D_x3 &t D_x4),
  [[1, 1], [2, 2], [3, 3], [4, 4]]), DepVars, notation = jetnumbers))) :
simplify(A + B)
> fvec2 := { } :for i to 4 do for j from (i + 1) to 4 do fvec2 := {op(fvec2), evalDG(D_x||i
  &t D_x||j)} :od:od:
fvec4 := { } :for i to nops(fvec2) do for j from i to nops(fvec2) do fvec4 := {op(fvec4),
  evalDG(fvec2[i] &t fvec2[j])} :od:od:
for i to nops(fvec4) do:
A||i := simplify(subs(SS, ToJet(ContractIndices(W, fvec4[i], [[1, 1], [2, 2], [3, 3], [4, 4]]),
  DepVars, notation = jetnumbers))) :
B||i := simplify(subs(SS, ToJet(ContractIndices(Wst, fvec4[i], [[1, 1], [2, 2], [3, 3], [4, 4]]),
  DepVars, notation = jetnumbers))) :
ANS||i := simplify(factor(A||i) + factor(B||i)) :od:
ANS := {seq(ANS||i, i = 1 ..nops(fvec4))}
... shall do this differently below ...
>
Type [2]
> F := u3 v2 - v2^2 - u2 v3 + v1 v3 : H := u4 v2 - v2 v3 - u2 v4 + v1 v4 :
> DR := (diff(F, u1)·ξ1 + diff(F, u2)·ξ2 + diff(F, u3)·ξ3 + diff(F, u4)·ξ4) · (diff(H, v1)·ξ1
  + diff(H, v2)·ξ2 + diff(H, v3)·ξ3 + diff(H, v4)·ξ4) - (diff(F, v1)·ξ1 + diff(F, v2)·ξ2
  + diff(F, v3)·ξ3 + diff(F, v4)·ξ4) · (diff(H, u1)·ξ1 + diff(H, u2)·ξ2 + diff(H, u3)·ξ3
  + diff(H, u4)·ξ4) :
GA := Matrix( [ [diff(DR, ξ1, ξ1), diff(DR, ξ1, ξ2), diff(DR, ξ1, ξ3), diff(DR, ξ1, ξ4)],
  [diff(DR, ξ1, ξ2), diff(DR, ξ2, ξ2), diff(DR, ξ2, ξ3), diff(DR, ξ2, ξ4)], [diff(DR, ξ1,
  ξ3), diff(DR, ξ2, ξ3), diff(DR, ξ3, ξ3), diff(DR, ξ3, ξ4)], [diff(DR, ξ1, ξ4), diff(DR, ξ2,
  ξ4), diff(DR, ξ3, ξ4), diff(DR, ξ4, ξ4)] ] ) :
Ga := factor( simplify( (v2^2 / Determinant(GA)) · GA ) ) : Gi := factor( simplify( (Determinant(GA) /
  v2^2)
  · MatrixInverse(GA) ) ) :
Aa := FromJet(Ga, DepVars) : Ai := FromJet(Gi, DepVars) :
g := evalDG(add(add(Ai[i, j]·dx||i &t dx||j, i = 1 ..4), j = 1 ..4)) : gInv
  := simplify(evalDG(add(add(Aa[i, j]·D_x||i &t D_x||j, i = 1 ..4), j = 1 ..4))) :
> DGsetup([x1, x2, x3, x4], [u, v], E, 3) :
unkn0 := {u3, v3} : contr0 := {F, H} : unkn := unkn0 : contr := contr0 :for i to 4 do unkn
  := {op(unkn), TotalDiff(unkn0[1], i), TotalDiff(unkn0[2], i)} : contr := {op(contr),

```

$TotalDiff(contr0[1], i), TotalDiff(contr0[2], i) \} : \text{for } j \text{ to } i \text{ do } unkn := \{op(unkn),$   
 $TotalDiff(unkn0[1], [i, j]), TotalDiff(unkn0[2], [i, j]) \} : contr := \{op(contr),$   
 $TotalDiff(contr0[1], [i, j]), TotalDiff(contr0[2], [i, j]) \} : \text{od:od: } SS := solve(contr,$   
 $unkn) :$

>  $ChangeFrame(M) :$

$W := WeylTensor(g) :$

>  $gl2 := evalDG(gInv \&t gInv) : tmp := ContractIndices(gl2, W, [[1, 1], [3, 2]]) :$

>  $densV := simplify(sqrt(Determinant(Ai)))$  assuming  $\frac{\partial}{\partial x_2} v(x1, x2, x3, x4) > 0, \frac{\partial}{\partial x_2} u(x1,$

$$x2, x3, x4) > 0, \frac{\partial}{\partial x_2} v(x1, x2, x3, x4) > \frac{\partial}{\partial x_1} v(x1, x2, x3, x4), \left( \frac{\partial}{\partial x_3} u(x1, x2, x3, x4) \right) \left( \frac{\partial}{\partial x_4} v(x1, x2, x3, x4) \right) + 2 \left( \frac{\partial}{\partial x_3} v(x1, x2, x3, x4) \right)^2 - \left( \frac{\partial}{\partial x_3} v(x1, x2, x3, x4) \right) \left( \frac{\partial}{\partial x_4} u(x1, x2, x3, x4) \right) - 2 \left( \frac{\partial}{\partial x_4} v(x1, x2, x3, x4) \right) \left( \frac{\partial}{\partial x_2} v(x1, x2, x3, x4) \right) < 0, \text{csgn} \left( \left( \left( \frac{\partial}{\partial x_3} u(x1, x2, x3, x4) \right) \left( \frac{\partial}{\partial x_4} v(x1, x2, x3, x4) \right) + 2 \left( \frac{\partial}{\partial x_3} v(x1, x2, x3, x4) \right)^2 - \left( \frac{\partial}{\partial x_3} v(x1, x2, x3, x4) \right) \left( \frac{\partial}{\partial x_4} u(x1, x2, x3, x4) \right) - 2 \left( \frac{\partial}{\partial x_4} v(x1, x2, x3, x4) \right) \left( \frac{\partial}{\partial x_2} v(x1, x2, x3, x4) \right) \right)^3 \right) = -1;$$

$$densV := \left( \frac{\partial}{\partial x_2} v(x1, x2, x3, x4) \right)^2 \left( 2 \left( \frac{\partial}{\partial x_2} v(x1, x2, x3, x4) \right) \left( \frac{\partial}{\partial x_4} v(x1, x2, x3, x4) \right) - \left( \frac{\partial}{\partial x_3} u(x1, x2, x3, x4) \right) \left( \frac{\partial}{\partial x_4} v(x1, x2, x3, x4) \right) + \left( \frac{\partial}{\partial x_4} u(x1, x2, x3, x4) \right) \left( \frac{\partial}{\partial x_3} v(x1, x2, x3, x4) \right) - 2 \left( \frac{\partial}{\partial x_3} v(x1, x2, x3, x4) \right)^2 \right)^3 \quad (26)$$

>  $V := evalDG(densV \cdot dx1 \&w dx2 \&w dx3 \&w dx4) :$

>  $Wst := evalDG \left( \frac{1}{2} \cdot ContractIndices(V, tmp, [[3, 1], [4, 2]]) \right) :$

$A := simplify(subs(SS, ToJet(ContractIndices(W, evalDG(D_x1 \&t D_x2 \&t D_x3 \&t D_x4),$   
 $[[1, 1], [2, 2], [3, 3], [4, 4]]), DepVars, notation = jetnumbers))) :$

$B := simplify(subs(SS, ToJet(ContractIndices(Wst, evalDG(D_x1 \&t D_x2 \&t D_x3 \&t D_x4),$   
 $[[1, 1], [2, 2], [3, 3], [4, 4]]), DepVars, notation = jetnumbers))) :$

$simplify(A + B);$

$\# simplify(A - B);$

0

(27)

>  $fvec2 := \{ \} : \text{for } i \text{ to } 4 \text{ do for } j \text{ from } (i + 1) \text{ to } 4 \text{ do } fvec2 := \{op(fvec2), evalDG(D_x||i$   
 $\&t D_x||j) \} : \text{od:od:}$

$fvec4 := \{ \} : \text{for } i \text{ to } nops(fvec2) \text{ do for } j \text{ from } i \text{ to } nops(fvec2) \text{ do } fvec4 := \{op(fvec4),$   
 $evalDG(fvec2[i] \&t fvec2[j]) \} : \text{od:od:}$

**for**  $i$  **to**  $nops(fvec4)$  **do:**

$A||i := simplify(subs(SS, ToJet(ContractIndices(W, fvec4[i], [[1, 1], [2, 2], [3, 3], [4, 4]]),$



```

    DepVars, notation = jetnumbers))) :
B||i := simplify(subs(SS, ToJet(ContractIndices(Wst,fvec4[i], [[1, 1], [2, 2], [3, 3], [4, 4]]),
    DepVars, notation = jetnumbers))) :
ANS||i := simplify(factor(A||i) + factor(B||i)) :od:
ANS := {seq(ANS||i, i = 1 ..nops(fvec4))}
ANS := {0}

```

(28)

>

In case [1,1] Maple does not want to compute due to some internal error (in PDEtools/NumerDenom) too many levels of recursion, so we re-wrote the program to make it more effective (now it does not use existing internal DG commands).

>

```

> WeylplusComp := proc(A, dens, i1, i2, i3, i4)
local Ai, R, Gam, Riem, Ric, Sc, W, e, vol, Wstar, Wplus, a, b, i, j, k, l, s, t, tmp;
Ai := MatrixInverse(A) :
for i to 4 do for j to 4 do for k to 4 do Gam[i, j, k] := 1/2 add(Ai[k, l]·(TotalDiff(A[i, l], j)
+ TotalDiff(A[j, l], i) - TotalDiff(A[i, j], l)), l = 1 ..4) :od:od:od:
for i to 4 do for j to 4 do for k to 4 do for l to 4 do R[i, j, k, l] := TotalDiff(Gam[i, k, l], j)
- TotalDiff(Gam[j, k, l], i) + add(Gam[i, k, s]·Gam[j, s, l] - Gam[j, k, s]·Gam[i, s,
l], s = 1 ..4) :od:od:od:od:
for i to 4 do for j to 4 do Ric[i, j] := add(R[i, s, j, s], s = 1 ..4) :od:od:
Sc := add(add(Ai[i, j]·Ric[i, j], j = 1 ..4), i = 1 ..4) :
for i to 4 do for j to 4 do for k to 4 do for l to 4 do W[i, j, k, l] := add(A[l, s]·R[i, j, k, s], s = 1
..4) + 1/2·(Ric[i, l]·A[j, k] - Ric[i, k]·A[j, l] + Ric[j, k]·A[i, l] - Ric[j, l]·A[i, k])
+ 1/6·Sc·(A[i, k]·A[j, l] - A[i, l]·A[j, k]) :od:od:od:od:
for i to 4 do for j to 4 do for k to 4 do for l to 4 do e[i, j, k, l] := 0 :od:od:od:od:
e[1, 2, 3, 4] := 1 : e[1, 2, 4, 3] := -1 : e[1, 3, 2, 4] := -1 : e[1, 3, 4, 2] := 1 : e[1, 4, 2, 3] :=
1 : e[1, 4, 3, 2] := -1 :
e[2, 1, 3, 4] := -1 : e[2, 1, 4, 3] := 1 : e[3, 1, 2, 4] := 1 : e[3, 1, 4, 2] := -1 : e[4, 1, 2, 3] :=
-1 : e[4, 1, 3, 2] := 1 :
e[2, 3, 1, 4] := 1 : e[2, 3, 4, 1] := -1 : e[2, 4, 1, 3] := -1 : e[2, 4, 3, 1] := 1 : e[3, 4, 1, 2] :=
1 : e[3, 4, 2, 1] := -1 :
e[3, 2, 1, 4] := -1 : e[3, 2, 4, 1] := 1 : e[4, 2, 1, 3] := 1 : e[4, 2, 3, 1] := -1 : e[4, 3, 1, 2] :=
-1 : e[4, 3, 2, 1] := 1 :
for i to 4 do for j to 4 do for k to 4 do for l to 4 do vol[i, j, k, l] := dens·e[i, j, k, l] :od:od:od:od:
od:
for i to 4 do for j to 4 do for k to 4 do for l to 4 do Wstar[i, j, k, l] := 1/2
·add(add(add(add(vol[i, j, s, t]·Ai[s, a]·Ai[t, b]·W[a, b, k, l], a = 1 ..4), b = 1 ..4), s = 1
..4), t = 1 ..4) :od:od:od:od:
for i to 4 do for j to 4 do for k to 4 do for l to 4 do Wplus[i, j, k, l] := 1/2·(W[i, j, k, l]
+ Wstar[i, j, k, l]) :od:od:od:od:
simplify(subs(SS, Wplus[i1, i2, i3, i4]))
end proc:

```



```

> Weylplus := proc(A, dens)
local Ai, R, Gam, Riem, Ric, Sc, W, e, vol, Wstar, Wplus, out, a, b, i, j, k, l, s, t, tmp;
Ai := MatrixInverse(A) :

for i to 4 do for j to 4 do for k to 4 do Gam[i, j, k] :=  $\frac{1}{2}$  add(Ai[k, l] · (TotalDiff(A[i, l], j)
+ TotalDiff(A[j, l], i) - TotalDiff(A[i, j], l)), l = 1..4) : od: od: od:
for i to 4 do for j to 4 do for k to 4 do for l to 4 do R[i, j, k, l] := TotalDiff(Gam[i, k, l], j)
- TotalDiff(Gam[j, k, l], i) + add(Gam[i, k, s] · Gam[j, s, l] - Gam[j, k, s] · Gam[i, s,
l], s = 1..4) : od: od: od: od:
for i to 4 do for j to 4 do Ric[i, j] := add(R[i, s, j, s], s = 1..4) : od: od:
Sc := add(add(Ai[i, j] · Ric[i, j], j = 1..4), i = 1..4) :
for i to 4 do for j to 4 do for k to 4 do for l to 4 do W[i, j, k, l] := add(A[l, s] · R[i, j, k, s], s = 1
..4) +  $\frac{1}{2}$  · (Ric[i, l] · A[j, k] - Ric[i, k] · A[j, l] + Ric[j, k] · A[i, l] - Ric[j, l] · A[i, k])
+  $\frac{1}{6}$  · Sc · (A[i, k] · A[j, l] - A[i, l] · A[j, k]) : od: od: od: od:
for i to 4 do for j to 4 do for k to 4 do for l to 4 do e[i, j, k, l] := 0 : od: od: od: od:
e[1, 2, 3, 4] := 1 : e[1, 2, 4, 3] := -1 : e[1, 3, 2, 4] := -1 : e[1, 3, 4, 2] := 1 : e[1, 4, 2, 3] :=
1 : e[1, 4, 3, 2] := -1 :
e[2, 1, 3, 4] := -1 : e[2, 1, 4, 3] := 1 : e[3, 1, 2, 4] := 1 : e[3, 1, 4, 2] := -1 : e[4, 1, 2, 3] :=
-1 : e[4, 1, 3, 2] := 1 :
e[2, 3, 1, 4] := 1 : e[2, 3, 4, 1] := -1 : e[2, 4, 1, 3] := -1 : e[2, 4, 3, 1] := 1 : e[3, 4, 1, 2] :=
1 : e[3, 4, 2, 1] := -1 :
e[3, 2, 1, 4] := -1 : e[3, 2, 4, 1] := 1 : e[4, 2, 1, 3] := 1 : e[4, 2, 3, 1] := -1 : e[4, 3, 1, 2] :=
-1 : e[4, 3, 2, 1] := 1 :
for i to 4 do for j to 4 do for k to 4 do for l to 4 do vol[i, j, k, l] := dens · e[i, j, k, l] : od: od: od:
od:
for i to 4 do for j to 4 do for k to 4 do for l to 4 do Wstar[i, j, k, l] :=  $\frac{1}{2}$ 
· add(add(add(add(vol[i, j, s, t] · Ai[s, a] · Ai[t, b] · W[a, b, k, l], a = 1..4), b = 1..4), s = 1
..4), t = 1..4) : od: od: od: od:
for i to 4 do for j to 4 do for k to 4 do for l to 4 do Wplus[i, j, k, l] :=  $\frac{1}{2}$  · (W[i, j, k, l]
+ Wstar[i, j, k, l]) : od: od: od: od:
out := { } : for i to 4 do for j from (i + 1) to 4 do for k from i to 4 do for l from  $\left( (k + 1) \right.$ 
 $\left. \cdot \frac{\text{sign}(k - i - 1) + 1}{2} + j \cdot \frac{1 - \text{sign}(k - i - 1)}{2} \right)$  to 4 do out := {op(out),
simplify(subs(SS, Wplus[i, j, k, l]))} : od: od: od: od:
out
end proc:

```

>

Type [2]

>  $F := u_3 v_2 - v_2^2 - u_2 v_3 + v_1 v_3 : H := u_4 v_2 - v_2 v_3 - u_2 v_4 + v_1 v_4 :$

>  $DR := \left( \text{diff}(F, u_1) \cdot \xi_1 + \text{diff}(F, u_2) \cdot \xi_2 + \text{diff}(F, u_3) \cdot \xi_3 + \text{diff}(F, u_4) \cdot \xi_4 \right) \cdot \left( \text{diff}(H, v_1) \cdot \xi_1 \right.$

$$+ \text{diff}(H, v_2) \cdot \xi_2 + \text{diff}(H, v_3) \cdot \xi_3 + \text{diff}(H, v_4) \cdot \xi_4 - (\text{diff}(F, v_1) \cdot \xi_1 + \text{diff}(F, v_2) \cdot \xi_2 \\ + \text{diff}(F, v_3) \cdot \xi_3 + \text{diff}(F, v_4) \cdot \xi_4) \cdot (\text{diff}(H, u_1) \cdot \xi_1 + \text{diff}(H, u_2) \cdot \xi_2 + \text{diff}(H, u_3) \cdot \xi_3 \\ + \text{diff}(H, u_4) \cdot \xi_4) :$$

$$GA := \text{Matrix} \left( \left[ \left[ \text{diff}(DR, \xi_1, \xi_1), \text{diff}(DR, \xi_1, \xi_2), \text{diff}(DR, \xi_1, \xi_3), \text{diff}(DR, \xi_1, \xi_4) \right], \right. \right. \\ \left. \left[ \text{diff}(DR, \xi_1, \xi_2), \text{diff}(DR, \xi_2, \xi_2), \text{diff}(DR, \xi_2, \xi_3), \text{diff}(DR, \xi_2, \xi_4) \right], \left[ \text{diff}(DR, \xi_1, \right. \right. \\ \left. \left. \xi_3), \text{diff}(DR, \xi_2, \xi_3), \text{diff}(DR, \xi_3, \xi_3), \text{diff}(DR, \xi_3, \xi_4) \right], \left[ \text{diff}(DR, \xi_1, \xi_4), \text{diff}(DR, \xi_2, \right. \right. \\ \left. \left. \xi_4), \text{diff}(DR, \xi_3, \xi_4), \text{diff}(DR, \xi_4, \xi_4) \right] \right] \right) :$$

$$A := \text{factor} \left( \text{simplify} \left( \frac{\text{Determinant}(GA)}{v_2^2} \cdot \text{MatrixInverse}(GA) \right) \right) :$$

$$\text{dens} := \text{simplify}(\text{sqrt}(\text{Determinant}(A))) \text{ assuming } v_2 > 0$$

$$\text{dens} := v_2^2 \text{ csgn} \left( (u_3 v_4 - u_4 v_3 - 2 v_2 v_4 + 2 v_3^2)^3 \right) (u_3 v_4 - u_4 v_3 - 2 v_2 v_4 + 2 v_3^2)^3 \quad (29)$$

$$> \text{dens} := \text{factor}(\text{dens}) \text{ assuming } (u_3 v_4 - u_4 v_3 - 2 v_2 v_4 + 2 v_3^2) < 0, \text{ csgn} \left( (u_3 v_4 - u_4 v_3 \right. \\ \left. - 2 v_2 v_4 + 2 v_3^2)^3 \right) = -1$$

$$\text{dens} := -v_2^2 (u_3 v_4 - u_4 v_3 - 2 v_2 v_4 + 2 v_3^2)^3 \quad (30)$$

$$> \text{DGsetup}([x1, x2, x3, x4], [u, v], E, 3) :$$

$$\text{unkn0} := \{u_3, v_3\} : \text{contr0} := \{F, H\} : \text{unkn} := \text{unkn0} : \text{contr} := \text{contr0} : \text{for } i \text{ to } 4 \text{ do } \text{unkn} \\ := \{\text{op}(\text{unkn}), \text{TotalDiff}(\text{unkn0}[1], i), \text{TotalDiff}(\text{unkn0}[2], i)\} : \text{contr} := \{\text{op}(\text{contr}), \\ \text{TotalDiff}(\text{contr0}[1], i), \text{TotalDiff}(\text{contr0}[2], i)\} : \text{for } j \text{ to } i \text{ do } \text{unkn} := \{\text{op}(\text{unkn}), \\ \text{TotalDiff}(\text{unkn0}[1], [i, j]), \text{TotalDiff}(\text{unkn0}[2], [i, j])\} : \text{contr} := \{\text{op}(\text{contr}), \\ \text{TotalDiff}(\text{contr0}[1], [i, j]), \text{TotalDiff}(\text{contr0}[2], [i, j])\} : \text{od:od: SS} := \text{solve}(\text{contr}, \\ \text{unkn}) :$$

$$> \text{WeylplusComp}(A, \text{dens}, 1, 2, 3, 4)$$

$$0$$

$$(31)$$

$$> \text{Weylplus}(A, \text{dens})$$

$$\{0\}$$

$$(32)$$

>

Type [1,1]

$$> F := u_2 v_3 - u_3 v_2 - u_2 v_2 + u_3 v_1 : H := u_2 v_4 - u_4 v_2 - u_2 v_3 + u_4 v_1 :$$

$$> DR := (\text{diff}(F, u_1) \cdot \xi_1 + \text{diff}(F, u_2) \cdot \xi_2 + \text{diff}(F, u_3) \cdot \xi_3 + \text{diff}(F, u_4) \cdot \xi_4) \cdot (\text{diff}(H, v_1) \cdot \xi_1 \\ + \text{diff}(H, v_2) \cdot \xi_2 + \text{diff}(H, v_3) \cdot \xi_3 + \text{diff}(H, v_4) \cdot \xi_4) - (\text{diff}(F, v_1) \cdot \xi_1 + \text{diff}(F, v_2) \cdot \xi_2 \\ + \text{diff}(F, v_3) \cdot \xi_3 + \text{diff}(F, v_4) \cdot \xi_4) \cdot (\text{diff}(H, u_1) \cdot \xi_1 + \text{diff}(H, u_2) \cdot \xi_2 + \text{diff}(H, u_3) \cdot \xi_3 \\ + \text{diff}(H, u_4) \cdot \xi_4) :$$

$$GA := \text{Matrix} \left( \left[ \left[ \text{diff}(DR, \xi_1, \xi_1), \text{diff}(DR, \xi_1, \xi_2), \text{diff}(DR, \xi_1, \xi_3), \text{diff}(DR, \xi_1, \xi_4) \right], \right. \right. \\ \left. \left[ \text{diff}(DR, \xi_1, \xi_2), \text{diff}(DR, \xi_2, \xi_2), \text{diff}(DR, \xi_2, \xi_3), \text{diff}(DR, \xi_2, \xi_4) \right], \left[ \text{diff}(DR, \xi_1, \right. \right. \\ \left. \left. \xi_3), \text{diff}(DR, \xi_2, \xi_3), \text{diff}(DR, \xi_3, \xi_3), \text{diff}(DR, \xi_3, \xi_4) \right], \left[ \text{diff}(DR, \xi_1, \xi_4), \text{diff}(DR, \xi_2, \right. \right. \\ \left. \left. \xi_4), \text{diff}(DR, \xi_3, \xi_4), \text{diff}(DR, \xi_4, \xi_4) \right] \right] \right)$$

$$\begin{aligned}
& \xi_4), \text{diff}(DR, \xi_3, \xi_4), \text{diff}(DR, \xi_4, \xi_4) ] ] ) : \\
A &:= \text{factor} \left( \text{simplify} \left( \frac{\text{Determinant}(GA)}{u_2 (v_1 - v_2)} \cdot \text{MatrixInverse}(GA) \right) \right) : \\
dens &:= \text{simplify}(\text{sqrt}(\text{Determinant}(A))) \text{ assuming } u_2 > 0, v_1 > v_2 \\
dens &:= u_2 (v_1 - v_2) \text{csgn} \left( (u_3 v_2 - 2 u_3 v_3 + u_3 v_4 - u_4 v_1 + 2 u_4 v_2 - u_4 v_3)^3 \right) (u_3 v_2 \\
& \quad - 2 u_3 v_3 + u_3 v_4 - u_4 v_1 + 2 u_4 v_2 - u_4 v_3)^3 \tag{33}
\end{aligned}$$

$$\begin{aligned}
> dens &:= \text{simplify}(dens) \text{ assuming } (u_3 v_2 - 2 u_3 v_3 + u_3 v_4 - u_4 v_1 + 2 u_4 v_2 - u_4 v_3) < 0, \\
& \text{csgn} \left( (u_3 v_2 - 2 u_3 v_3 + u_3 v_4 - u_4 v_1 + 2 u_4 v_2 - u_4 v_3)^3 \right) = -1 \\
dens &:= -u_2 (v_1 - v_2) (u_3 v_2 - 2 u_3 v_3 + u_3 v_4 - u_4 v_1 + 2 u_4 v_2 - u_4 v_3)^3 \tag{34}
\end{aligned}$$

$$\begin{aligned}
> DGsetup &([x1, x2, x3, x4], [u, v], E, 3) : \\
unkn0 &:= \{u_3, v_3\} : contr0 := \{F, H\} : unkn := unkn0 : contr := contr0 : \text{for } i \text{ to } 4 \text{ do } unkn \\
&:= \{op(unkn), \text{TotalDiff}(unkn0[1], i), \text{TotalDiff}(unkn0[2], i)\} : contr := \{op(contr), \\
&\text{TotalDiff}(contr0[1], i), \text{TotalDiff}(contr0[2], i)\} : \text{for } j \text{ to } i \text{ do } unkn := \{op(unkn), \\
&\text{TotalDiff}(unkn0[1], [i, j]), \text{TotalDiff}(unkn0[2], [i, j])\} : contr := \{op(contr), \\
&\text{TotalDiff}(contr0[1], [i, j]), \text{TotalDiff}(contr0[2], [i, j])\} : \text{od:od: } SS := \text{solve}(contr, \\
&unkn) :
\end{aligned}$$

$$\begin{aligned}
> WeylplusComp(A, dens, 1, 2, 3, 4) \\
& \quad 0 \tag{35}
\end{aligned}$$

$$\begin{aligned}
> Weylplus(A, dens) \\
& \quad \{0\} \tag{36}
\end{aligned}$$

>
