# Supplementary material for: Integrable systems in 4D associated with sixfolds in Gr(4,6)
Source: arXiv:1705.06999 ancillary file (2017-05-18)
Supplement: Supplementary file 2 [file DFKN-2017-Integrability_conditions.pdf]

This notebook accompanies the paper B.Doubrov, E.Ferapontov, B.Kruglikov, V.Novikov "Integrable systems in 4D associated with sixfolds in  $Gr(4,6)$ ".

We compute integrability conditions for the 2x2 system:  $ut=f[ux,uy,uz,vx,vy,vz]$ ,  $vt=g[ux,uy,uz,vx,vy,vz]$  by the method of hydrodynamic reductions.

Notations:  $R1[0]$ ,  $R2[0]$ ,  $R3[0]$  - Riemann invariants satisfying

$R1_t=\lambda_1 R1_x$ ,  $R2_t=\lambda_2 R2_x$ ,  $R3_t=\lambda_3 R3_x$ ,  
 $R1_y=\mu_1 R1_x$ ,  $R2_y=\mu_2 R2_x$ ,  $R3_y=\mu_3 R3_x$ ,  
 $R1_z=\nu_1 R1_x$ ,  $R2_z=\nu_2 R2_x$ ,  $R3_z=\nu_3 R3_x$ .

$R1[n]$ ,  $R2[n]$ ,  $R3[n]$  denote n-th derivatives of  $R1, R2, R3$  with respect to  $x$ .  $DX, Dy, DT, Dz$  - operator of derivatives.

```
imax = 20;
DX[exp_] := Block[{i, res}, res = 0;
  Do[res = res + R1[i + 1] D[exp, R1[i]] + R2[i + 1] D[exp, R2[i]] + R3[i + 1] D[exp, R3[i]];
    res = res /. {u[imax + 1] -> 0}, {i, 0, imax}]; res];
DXN[exp_, n_] := Block[{i, res}, res = exp;
  If[n > 0, Do[res = DX[res], {i, 1, n}], None]; res];
Off[General::spell1]; Off[General::spell];
Dy[exp_] := Block[{i, res = 0},
  Do[If[ToString[D[exp, R1[i]]] != "0" || ToString[D[exp, R2[i]]] != "0" ||
    ToString[D[exp, R3[i]]] != "0", res = res + D[exp, R1[i]] DXN[R1y, i] +
    D[exp, R2[i]] DXN[R2y, i] + D[exp, R3[i]] DXN[R3y, i], None], {i, 0, imax}];
  res];
DT[exp_] := Block[{i, res = 0}, Do[If[ToString[D[exp, R1[i]]] != "0" ||
  ToString[D[exp, R2[i]]] != "0" || ToString[D[exp, R3[i]]] != "0",
  res = res + D[exp, R1[i]] DXN[R1t, i] + D[exp, R2[i]] DXN[R2t, i] +
  D[exp, R3[i]] DXN[R3t, i], None], {i, 0, imax}];
  res];
Dz[exp_] := Block[{i, res = 0}, Do[If[ToString[D[exp, R1[i]]] != "0" ||
  ToString[D[exp, R2[i]]] != "0" || ToString[D[exp, R3[i]]] != "0",
  res = res + D[exp, R1[i]] DXN[R1z, i] + D[exp, R2[i]] DXN[R2z, i] +
  D[exp, R3[i]] DXN[R3z, i], None], {i, 0, imax}];
  res];
SetAttributes[killfactor, Listable];
killfactor[a_^_] := a;
killfactor[a_^_] := 1 /; MemberQ[factorlist, a];
killfactor[a_] := 1 /; MemberQ[factorlist, a];
killfactor[a_] := a;
killfactor[a_] := 0 /; MemberQ[factorlistzero, a];
killfactor[a_b_] := killfactor[a] killfactor[b];
killfactor[a_] := 1 /; IntegerQ[a];
killfactor[0] := 0;
factorlist = {};
der[exp_, var_] := Block[{jj, num, den, numd, dend}, num = Numerator[exp];
  den = Denominator[exp];
```

```

numd = Factor[D[num, var]];
dend = Factor[D[den, var]];
jj = Factor[numd den - dend num] / den^2; jj];

(*=====*)
(*Definitions*)

r1 = R1[0];
r2 = R2[0];
r3 = R3[0];

R1y =  $\mu_1[r1, r2, r3]$  R1[1];
R2y =  $\mu_2[r1, r2, r3]$  R2[1];
R3y =  $\mu_3[r1, r2, r3]$  R3[1];

R1t =  $\lambda_1[r1, r2, r3]$  R1[1];
R2t =  $\lambda_2[r1, r2, r3]$  R2[1];
R3t =  $\lambda_3[r1, r2, r3]$  R3[1];

R1z =  $\nu_1[r1, r2, r3]$  R1[1];
R2z =  $\nu_2[r1, r2, r3]$  R2[1];
R3z =  $\nu_3[r1, r2, r3]$  R3[1];

f = F[a, b, c, p, q, r];
g = G[a, b, c, p, q, r];

fa = D[f, a];
fb = D[f, b];
fc = D[f, c];
fp = D[f, p];
fq = D[f, q];
fr = D[f, r];

ga = D[g, a];
gb = D[g, b];
gc = D[g, c];
gp = D[g, p];
gq = D[g, q];
gr = D[g, r];

(*=====*)
(*We rewrite
   ut=f[ux,uy,uz,vx,vy,vz];
   vt=g[ux,uy,uz,vx,vy,vz];
in the first order quasilinear form

```

\*)

(\*a=ux, b=uy, c=uz, p=vx, q=vy, r=vz\*)\_

(\* ay=bx, az=cx, bz=cy, ... \*)\_

```
a = A[r1, r2, r3];
b = B[r1, r2, r3];
c = Cc[r1, r2, r3];
p = P[r1, r2, r3];
q = Q[r1, r2, r3];
r = R[r1, r2, r3];
```

```
ax = DX[a];
ay = Dy[a];
at = DT[a];
az = Dz[a];
```

```
bx = DX[b];
by = Dy[b];
bt = DT[b];
bz = Dz[b];
```

```
cx = DX[c];
cy = Dy[c];
ct = DT[c];
cz = Dz[c];
```

```
px = DX[p];
py = Dy[p];
pt = DT[p];
pz = Dz[p];
```

```
qx = DX[q];
qy = Dy[q];
qt = DT[q];
qz = Dz[q];
```

```
rx = DX[r];
ry = Dy[r];
rt = DT[r];
rz = Dz[r];
```

(\*relations on first derivative of b,c,q,r,  
p as well as the explicit expressions for  $\lambda_i$  and  $\mu_i$  due to  $ay=bx$ ,

az=cx, bz=cy, ...\*)

$$\begin{aligned}
S = & \{ B^{(1,0,0)}[x_-, y_-, z_-] \Rightarrow \mu 1[x, y, z] A^{(1,0,0)}[x, y, z], \\
& B^{(0,1,0)}[x_-, y_-, z_-] \Rightarrow \mu 2[x, y, z] A^{(0,1,0)}[x, y, z], \\
& B^{(0,0,1)}[x_-, y_-, z_-] \Rightarrow \mu 3[x, y, z] A^{(0,0,1)}[x, y, z], Cc^{(1,0,0)}[x_-, y_-, z_-] \Rightarrow \\
& \quad \nu 1[x, y, z] A^{(1,0,0)}[x, y, z], Cc^{(0,1,0)}[x_-, y_-, z_-] \Rightarrow \nu 2[x, y, z] A^{(0,1,0)}[x, y, z], \\
& Cc^{(0,0,1)}[x_-, y_-, z_-] \Rightarrow \nu 3[x, y, z] A^{(0,0,1)}[x, y, z], \\
& Q^{(1,0,0)}[x_-, y_-, z_-] \Rightarrow \mu 1[x, y, z] \phi 1[x, y, z] A^{(1,0,0)}[x, y, z], \\
& Q^{(0,1,0)}[x_-, y_-, z_-] \Rightarrow \mu 2[x, y, z] \phi 2[x, y, z] A^{(0,1,0)}[x, y, z], \\
& Q^{(0,0,1)}[x_-, y_-, z_-] \Rightarrow \mu 3[x, y, z] \phi 3[x, y, z] A^{(0,0,1)}[x, y, z], \\
& R^{(1,0,0)}[x_-, y_-, z_-] \Rightarrow \nu 1[x, y, z] \phi 1[x, y, z] A^{(1,0,0)}[x, y, z], \\
& R^{(0,1,0)}[x_-, y_-, z_-] \Rightarrow \nu 2[x, y, z] \phi 2[x, y, z] A^{(0,1,0)}[x, y, z], \\
& R^{(0,0,1)}[x_-, y_-, z_-] \Rightarrow \nu 3[x, y, z] \phi 3[x, y, z] A^{(0,0,1)}[x, y, z], \\
& P^{(1,0,0)}[x_-, y_-, z_-] \Rightarrow \phi 1[x, y, z] A^{(1,0,0)}[x, y, z], \\
& P^{(0,1,0)}[x_-, y_-, z_-] \Rightarrow \phi 2[x, y, z] A^{(0,1,0)}[x, y, z], \\
& P^{(0,0,1)}[x_-, y_-, z_-] \Rightarrow \phi 3[x, y, z] A^{(0,0,1)}[x, y, z] \}; \\
\lambda 1[x_-, y_-, z_-] := & \nu 1[x, y, z] \phi 1[x, y, z] F^{(0,0,0,0,0,1)}[A[x, y, z], B[x, y, z], \\
& Cc[x, y, z], P[x, y, z], Q[x, y, z], R[x, y, z]] + \mu 1[x, y, z] \phi 1[x, y, z] \\
& F^{(0,0,0,0,1,0)}[A[x, y, z], B[x, y, z], Cc[x, y, z], P[x, y, z], Q[x, y, z], R[x, y, z]] + \\
& \phi 1[x, y, z] F^{(0,0,0,1,0,0)}[A[x, y, z], B[x, y, z], Cc[x, y, z], P[x, y, z], \\
& Q[x, y, z], R[x, y, z]] + \nu 1[x, y, z] F^{(0,0,1,0,0,0)}[A[x, y, z], B[x, y, z], \\
& Cc[x, y, z], P[x, y, z], Q[x, y, z], R[x, y, z]] + \mu 1[x, y, z] \\
& F^{(0,1,0,0,0,0)}[A[x, y, z], B[x, y, z], Cc[x, y, z], P[x, y, z], Q[x, y, z], R[x, y, z]] + \\
& F^{(1,0,0,0,0,0)}[A[x, y, z], B[x, y, z], Cc[x, y, z], P[x, y, z], Q[x, y, z], R[x, y, z]]; \\
\lambda 2[x_-, y_-, z_-] := & \nu 2[x, y, z] \phi 2[x, y, z] F^{(0,0,0,0,0,1)}[A[x, y, z], B[x, y, z], \\
& Cc[x, y, z], P[x, y, z], Q[x, y, z], R[x, y, z]] + \mu 2[x, y, z] \phi 2[x, y, z] \\
& F^{(0,0,0,0,1,0)}[A[x, y, z], B[x, y, z], Cc[x, y, z], P[x, y, z], Q[x, y, z], R[x, y, z]] + \\
& \phi 2[x, y, z] F^{(0,0,0,1,0,0)}[A[x, y, z], B[x, y, z], Cc[x, y, z], P[x, y, z], \\
& Q[x, y, z], R[x, y, z]] + \nu 2[x, y, z] F^{(0,0,1,0,0,0)}[A[x, y, z], B[x, y, z], \\
& Cc[x, y, z], P[x, y, z], Q[x, y, z], R[x, y, z]] + \mu 2[x, y, z] \\
& F^{(0,1,0,0,0,0)}[A[x, y, z], B[x, y, z], Cc[x, y, z], P[x, y, z], Q[x, y, z], R[x, y, z]] + \\
& F^{(1,0,0,0,0,0)}[A[x, y, z], B[x, y, z], Cc[x, y, z], P[x, y, z], Q[x, y, z], R[x, y, z]]; \\
\lambda 3[x_-, y_-, z_-] := & \nu 3[x, y, z] \phi 3[x, y, z] F^{(0,0,0,0,0,1)}[A[x, y, z], B[x, y, z], \\
& Cc[x, y, z], P[x, y, z], Q[x, y, z], R[x, y, z]] + \mu 3[x, y, z] \phi 3[x, y, z] \\
& F^{(0,0,0,0,1,0)}[A[x, y, z], B[x, y, z], Cc[x, y, z], P[x, y, z], Q[x, y, z], R[x, y, z]] + \\
& \phi 3[x, y, z] F^{(0,0,0,1,0,0)}[A[x, y, z], B[x, y, z], Cc[x, y, z], P[x, y, z], \\
& Q[x, y, z], R[x, y, z]] + \nu 3[x, y, z] F^{(0,0,1,0,0,0)}[A[x, y, z], B[x, y, z], \\
& Cc[x, y, z], P[x, y, z], Q[x, y, z], R[x, y, z]] + \mu 3[x, y, z] \\
& F^{(0,1,0,0,0,0)}[A[x, y, z], B[x, y, z], Cc[x, y, z], P[x, y, z], Q[x, y, z], R[x, y, z]] + \\
& F^{(1,0,0,0,0,0)}[A[x, y, z], B[x, y, z], Cc[x, y, z], P[x, y, z], Q[x, y, z], R[x, y, z]]; \\
\mu 1[x_-, y_-, z_-] := & -(\nu 1[x, y, z] \phi 1[x, y, z]^2 F^{(0,0,0,0,0,1)}[A[x, y, z], B[x, y, z], \\
& Cc[x, y, z], P[x, y, z], Q[x, y, z], R[x, y, z]] - \nu 1[x, y, z] \phi 1[x, y, z] \\
& G^{(0,0,0,0,0,1)}[A[x, y, z], B[x, y, z], Cc[x, y, z], P[x, y, z], Q[x, y, z], R[x, y, z]] + \\
& \phi 1[x, y, z]^2 F^{(0,0,0,1,0,0)}[A[x, y, z], B[x, y, z], Cc[x, y, z],
\end{aligned}$$

[illegible]

```

eq1 = (ay - bx) /. S;
eq2 = (az - cx) /. S;
eq3 = (cy - bz) /. S;
eq4 = (py - qx) /. S;
eq5 = (pz - rx) /. S;
eq6 = (qz - ry) /. S;
eq7 = (at - DX[f]) /. S;
eq8 = (bt - Dy[f]) /. S;
eq9 = (ct - Dz[f]) /. S;
eq10 = (pt - DX[g]) /. S;
eq11 = (qt - Dy[g]) /. S;
eq12 = (rt - Dz[g]) /. S;

```

(\*Verifying equations \*)

```

Factor[eq1]
Factor[eq2]
Factor[eq3]
Factor[eq4]
Factor[eq5]
Factor[eq6]
Factor[eq7]
Factor[eq8]
Factor[eq9]
Factor[eq10]
Factor[eq11]
Factor[eq12]

```

0

```

factorlist = {};
denfactor := Block[{i}, Do[
  AppendTo[factorlist, FactorList[Denominator[listderfin[[i]][[1]] /. listderfin]]];
  factorlist = Union[Flatten[factorlist], {i, 1, Length[listderfin]}]];
denfactor;

```

```

S1 = {B(1,0,0)[x, y, z] ⇒ μ1[x, y, z] A(1,0,0)[x, y, z],
  B(0,1,0)[x, y, z] ⇒ μ2[x, y, z] A(0,1,0)[x, y, z], B(0,0,1)[x, y, z] ⇒
  μ3[x, y, z] A(0,0,1)[x, y, z], Cc(1,0,0)[x, y, z] ⇒ ν1[x, y, z] A(1,0,0)[x, y, z],
  Cc(0,1,0)[x, y, z] ⇒ ν2[x, y, z] A(0,1,0)[x, y, z], Cc(0,0,1)[x, y, z] ⇒
  ν3[x, y, z] A(0,0,1)[x, y, z], Q(1,0,0)[x, y, z] ⇒ μ1[x, y, z] ϕ1[x, y, z] A(1,0,0)[x, y, z],
  Q(0,1,0)[x, y, z] ⇒ μ2[x, y, z] ϕ2[x, y, z] A(0,1,0)[x, y, z],
  Q(0,0,1)[x, y, z] ⇒ μ3[x, y, z] ϕ3[x, y, z] A(0,0,1)[x, y, z],
  R(1,0,0)[x, y, z] ⇒ ν1[x, y, z] ϕ1[x, y, z] A(1,0,0)[x, y, z],
  R(0,1,0)[x, y, z] ⇒ ν2[x, y, z] ϕ2[x, y, z] A(0,1,0)[x, y, z],
  R(0,0,1)[x, y, z] ⇒ ν3[x, y, z] ϕ3[x, y, z] A(0,0,1)[x, y, z],

```

$$\begin{aligned}
& P^{(1,0,0)}[x, y, z] \Rightarrow \phi 1[x, y, z] A^{(1,0,0)}[x, y, z], \\
& P^{(0,1,0)}[x, y, z] \Rightarrow \phi 2[x, y, z] A^{(0,1,0)}[x, y, z], \\
& P^{(0,0,1)}[x, y, z] \Rightarrow \phi 3[x, y, z] A^{(0,0,1)}[x, y, z]; \\
SS = & \{A[x, y, z] \rightarrow Af, B[x, y, z] \rightarrow Bf, Cc[x, y, z] \rightarrow Cf, P[x, y, z] \rightarrow Pf, Q[x, y, z] \rightarrow Qf, \\
& R[x, y, z] \rightarrow Rf, \phi 1[x, y, z] \rightarrow \phi 1, \phi 2[x, y, z] \rightarrow \phi 2, \phi 3[x, y, z] \rightarrow \phi 3, \nu 1[x, y, z] \rightarrow \nu 1, \\
& \nu 2[x, y, z] \rightarrow \nu 2, \nu 3[x, y, z] \rightarrow \nu 3, A^{(1,0,0)}[x, y, z] \rightarrow a1, A^{(0,1,0)}[x, y, z] \rightarrow a2, \\
& A^{(0,0,1)}[x, y, z] \rightarrow a3, B^{(1,0,0)}[x, y, z] \rightarrow b1, B^{(0,1,0)}[x, y, z] \rightarrow b2, \\
& B^{(0,0,1)}[x, y, z] \rightarrow b3, Cc^{(1,0,0)}[x, y, z] \rightarrow c1, Cc^{(0,1,0)}[x, y, z] \rightarrow c2, \\
& Cc^{(0,0,1)}[x, y, z] \rightarrow c3, D[P[x, y, z], x] \rightarrow p1, D[P[x, y, z], y] \rightarrow p2, \\
& D[P[x, y, z], z] \rightarrow p3, Q^{(1,0,0)}[x, y, z] \rightarrow q1, Q^{(0,1,0)}[x, y, z] \rightarrow q2, Q^{(0,0,1)}[x, y, z] \rightarrow q3, \\
& R^{(1,0,0)}[x, y, z] \rightarrow rr1, R^{(0,1,0)}[x, y, z] \rightarrow rr2, R^{(0,0,1)}[x, y, z] \rightarrow rr3, \\
& D[\phi 1[x, y, z], y] \rightarrow \phi 12, D[\phi 1[x, y, z], z] \rightarrow \phi 13, D[\phi 2[x, y, z], x] \rightarrow \phi 21, \\
& D[\phi 2[x, y, z], z] \rightarrow \phi 23, D[\phi 3[x, y, z], x] \rightarrow \phi 31, D[\phi 3[x, y, z], y] \rightarrow \phi 32, \\
& D[\nu 1[x, y, z], y] \rightarrow \nu 12, D[\nu 1[x, y, z], z] \rightarrow \nu 13, D[\nu 2[x, y, z], x] \rightarrow \nu 21, \\
& D[\nu 2[x, y, z], z] \rightarrow \nu 23, D[\nu 3[x, y, z], x] \rightarrow \nu 31, D[\nu 3[x, y, z], y] \rightarrow \nu 32, \\
& D[A[x, y, z], x, y] \rightarrow a12, D[A[x, y, z], x, z] \rightarrow a13, D[A[x, y, z], y, z] \rightarrow a23\}; \\
SS1 = & \{F^{(1,0,0,0,0,0,0,0)}[Af, Bf, Cf, Pf, Qf, Rf] \rightarrow Fa, F^{(0,1,0,0,0,0,0,0)}[Af, Bf, Cf, Pf, Qf, Rf] \rightarrow Fb, \\
& F^{(0,0,1,0,0,0,0,0)}[Af, Bf, Cf, Pf, Qf, Rf] \rightarrow Fc, F^{(0,0,0,1,0,0,0,0)}[Af, Bf, Cf, Pf, Qf, Rf] \rightarrow Fp, \\
& F^{(0,0,0,0,1,0,0,0)}[Af, Bf, Cf, Pf, Qf, Rf] \rightarrow Fq, F^{(0,0,0,0,0,1,0,0)}[Af, Bf, Cf, Pf, Qf, Rf] \rightarrow Fr, \\
& G^{(1,0,0,0,0,0,0,0)}[Af, Bf, Cf, Pf, Qf, Rf] \rightarrow Ga, G^{(0,1,0,0,0,0,0,0)}[Af, Bf, Cf, Pf, Qf, Rf] \rightarrow Gb, \\
& G^{(0,0,1,0,0,0,0,0)}[Af, Bf, Cf, Pf, Qf, Rf] \rightarrow Gc, G^{(0,0,0,1,0,0,0,0)}[Af, Bf, Cf, Pf, Qf, Rf] \rightarrow Gp, \\
& G^{(0,0,0,0,1,0,0,0)}[Af, Bf, Cf, Pf, Qf, Rf] \rightarrow Gq, G^{(0,0,0,0,0,1,0,0)}[Af, Bf, Cf, Pf, Qf, Rf] \rightarrow Gr, \\
& F^{(2,0,0,0,0,0,0,0)}[Af, Bf, Cf, Pf, Qf, Rf] \rightarrow Faa, F^{(1,1,0,0,0,0,0,0)}[Af, Bf, Cf, Pf, Qf, Rf] \rightarrow Fab, \\
& F^{(1,0,1,0,0,0,0,0)}[Af, Bf, Cf, Pf, Qf, Rf] \rightarrow Fac, F^{(1,0,0,1,0,0,0,0)}[Af, Bf, Cf, Pf, Qf, Rf] \rightarrow Fap, \\
& F^{(1,0,0,0,1,0,0,0)}[Af, Bf, Cf, Pf, Qf, Rf] \rightarrow Faq, F^{(1,0,0,0,0,1,0,0)}[Af, Bf, Cf, Pf, Qf, Rf] \rightarrow Far, \\
& F^{(0,2,0,0,0,0,0,0)}[Af, Bf, Cf, Pf, Qf, Rf] \rightarrow Fbb, F^{(0,1,1,0,0,0,0,0)}[Af, Bf, Cf, Pf, Qf, Rf] \rightarrow Fbc, \\
& F^{(0,1,0,1,0,0,0,0)}[Af, Bf, Cf, Pf, Qf, Rf] \rightarrow Fbp, F^{(0,1,0,0,1,0,0,0)}[Af, Bf, Cf, Pf, Qf, Rf] \rightarrow Fbq, \\
& F^{(0,1,0,0,0,1,0,0)}[Af, Bf, Cf, Pf, Qf, Rf] \rightarrow Fbr, F^{(0,0,2,0,0,0,0,0)}[Af, Bf, Cf, Pf, Qf, Rf] \rightarrow Fcc, \\
& F^{(0,0,1,1,0,0,0,0)}[Af, Bf, Cf, Pf, Qf, Rf] \rightarrow Fcp, F^{(0,0,1,0,1,0,0,0)}[Af, Bf, Cf, Pf, Qf, Rf] \rightarrow Fcq, \\
& F^{(0,0,1,0,0,1,0,0)}[Af, Bf, Cf, Pf, Qf, Rf] \rightarrow Fcr, F^{(0,0,0,2,0,0,0,0)}[Af, Bf, Cf, Pf, Qf, Rf] \rightarrow Fpp, \\
& F^{(0,0,0,1,1,0,0,0)}[Af, Bf, Cf, Pf, Qf, Rf] \rightarrow Fpq, F^{(0,0,0,1,0,1,0,0)}[Af, Bf, Cf, Pf, Qf, Rf] \rightarrow Fpr, \\
& F^{(0,0,0,0,2,0,0,0)}[Af, Bf, Cf, Pf, Qf, Rf] \rightarrow Fqq, F^{(0,0,0,0,1,1,0,0)}[Af, Bf, Cf, Pf, Qf, Rf] \rightarrow Fqr, \\
& F^{(0,0,0,0,0,2,0,0)}[Af, Bf, Cf, Pf, Qf, Rf] \rightarrow Frr, G^{(2,0,0,0,0,0,0,0)}[Af, Bf, Cf, Pf, Qf, Rf] \rightarrow Gaa, \\
& G^{(1,1,0,0,0,0,0,0)}[Af, Bf, Cf, Pf, Qf, Rf] \rightarrow Gab, G^{(1,0,1,0,0,0,0,0)}[Af, Bf, Cf, Pf, Qf, Rf] \rightarrow Gac, \\
& G^{(1,0,0,1,0,0,0,0)}[Af, Bf, Cf, Pf, Qf, Rf] \rightarrow Gap, G^{(1,0,0,0,1,0,0,0)}[Af, Bf, Cf, Pf, Qf, Rf] \rightarrow Gaq, \\
& G^{(1,0,0,0,0,1,0,0)}[Af, Bf, Cf, Pf, Qf, Rf] \rightarrow Gar, G^{(0,2,0,0,0,0,0,0)}[Af, Bf, Cf, Pf, Qf, Rf] \rightarrow Gbb, \\
& G^{(0,1,1,0,0,0,0,0)}[Af, Bf, Cf, Pf, Qf, Rf] \rightarrow Gbc, G^{(0,1,0,1,0,0,0,0)}[Af, Bf, Cf, Pf, Qf, Rf] \rightarrow Gbp, \\
& G^{(0,1,0,0,1,0,0,0)}[Af, Bf, Cf, Pf, Qf, Rf] \rightarrow Gbq, G^{(0,1,0,0,0,1,0,0)}[Af, Bf, Cf, Pf, Qf, Rf] \rightarrow Gbr, \\
& G^{(0,0,2,0,0,0,0,0)}[Af, Bf, Cf, Pf, Qf, Rf] \rightarrow Gcc, G^{(0,0,1,1,0,0,0,0)}[Af, Bf, Cf, Pf, Qf, Rf] \rightarrow Gcp, \\
& G^{(0,0,1,0,1,0,0,0)}[Af, Bf, Cf, Pf, Qf, Rf] \rightarrow Gcq, G^{(0,0,1,0,0,1,0,0)}[Af, Bf, Cf, Pf, Qf, Rf] \rightarrow Gcr, \\
& G^{(0,0,0,2,0,0,0,0)}[Af, Bf, Cf, Pf, Qf, Rf] \rightarrow Gpp, G^{(0,0,0,1,1,0,0,0)}[Af, Bf, Cf, Pf, Qf, Rf] \rightarrow Gpq, \\
& G^{(0,0,0,1,0,1,0,0)}[Af, Bf, Cf, Pf, Qf, Rf] \rightarrow Gpr, G^{(0,0,0,0,2,0,0,0)}[Af, Bf, Cf, Pf, Qf, Rf] \rightarrow Gqq, \\
& G^{(0,0,0,0,1,1,0,0)}[Af, Bf, Cf, Pf, Qf, Rf] \rightarrow Gqr, G^{(0,0,0,0,0,2,0,0)}[Af, Bf, Cf, Pf, Qf, Rf] \rightarrow Grr\}; \\
Sf = & \{b1 \rightarrow (a1 (Ga + Gc \nu 1 - Fa \phi 1 + Gp \phi 1 - Fc \nu 1 \phi 1 + Gr \nu 1 \phi 1 - Fp \phi 1^2 - Fr \nu 1 \phi 1^2)) /
\end{aligned}$$

```

      (-Gb + Fb ϕ1 - Gq ϕ1 + Fq ϕ12),
b2 → (a2 (Ga + Gc v2 - Fa ϕ2 + Gp ϕ2 - Fc v2 ϕ2 + Gr v2 ϕ2 - Fp ϕ22 - Fr v2 ϕ22)) /
      (-Gb + Fb ϕ2 - Gq ϕ2 + Fq ϕ22),
b3 → (a3 (Ga + Gc v3 - Fa ϕ3 + Gp ϕ3 - Fc v3 ϕ3 + Gr v3 ϕ3 - Fp ϕ32 - Fr v3 ϕ32)) /
      (-Gb + Fb ϕ3 - Gq ϕ3 + Fq ϕ32), c1 → a1 v1, c2 → a2 v2, c3 → a3 v3,
q1 → (a1 ϕ1 (Ga + Gc v1 - Fa ϕ1 + Gp ϕ1 - Fc v1 ϕ1 + Gr v1 ϕ1 - Fp ϕ12 - Fr v1 ϕ12)) /
      (-Gb + Fb ϕ1 - Gq ϕ1 + Fq ϕ12),
q2 → (a2 ϕ2 (Ga + Gc v2 - Fa ϕ2 + Gp ϕ2 - Fc v2 ϕ2 + Gr v2 ϕ2 - Fp ϕ22 - Fr v2 ϕ22)) /
      (-Gb + Fb ϕ2 - Gq ϕ2 + Fq ϕ22),
q3 → (a3 ϕ3 (Ga + Gc v3 - Fa ϕ3 + Gp ϕ3 - Fc v3 ϕ3 + Gr v3 ϕ3 - Fp ϕ32 - Fr v3 ϕ32)) /
      (-Gb + Fb ϕ3 - Gq ϕ3 + Fq ϕ32), rr1 → a1 v1 ϕ1,
rr2 → a2 v2 ϕ2, rr3 → a3 v3 ϕ3, p1 → a1 ϕ1, p2 → a2 ϕ2, p3 → a3 ϕ3};

sub[exp_, list_] :=
Block[{el, n = Length[list], i, cf, elem, exp1, num, den, cf1, add1, add2}, exp1 = exp;
Do[el = list[[i]][[1]];
If[FreeQ[exp, el], None, elem = list[[i]][[2]];
Print["Considering ", el];
num = Numerator[elem];
den = Denominator[elem];
cf = Factor[Coefficient[exp1, el]];
cf1 = Factor[cf/den];
add1 = Numerator[cf1] num;
add2 = Denominator[cf1] (exp1 /. el → 0);
exp1 = Numerator[Factor[add1 + add2]]], {i, 1, n}]; exp1];
subf[exp_, list_] := Block[{el, n = Length[list], i, cf, elem, exp1}, exp1 = exp;
Do[el = list[[i]][[1]];
If[FreeQ[exp1, el], None, elem = list[[i]][[2]];
Print["Considering ", el];
exp1 = Factor[Collect[exp1, el] /. list[[i]]], {i, 1, n}]; exp1];
der[exp_, var_] := Block[{jj, num, den, numd, dend}, num = Numerator[exp];
den = Denominator[exp];
numd = Factor[D[num, var]];
dend = Factor[D[den, var]];
jj = Factor[numd den - dend num] / den^2;
jj];

```

(\*Computing the compatibility of relations in the list S1\*)



```

eq1 = Numerator[Factor[Factor[D[(D[B[x, y, z], x] /. S), y] /. S] -
  Factor[D[(D[B[x, y, z], y] /. S), x] /. S]] /. SS /. SS1;
eq2 = Numerator[Factor[Factor[D[(D[B[x, y, z], x] /. S), z] /. S] -
  Factor[D[(D[B[x, y, z], z] /. S), x] /. S]] /. SS /. SS1;
eq3 = Numerator[Factor[Factor[D[(D[B[x, y, z], y] /. S), z] /. S] -
  Factor[D[(D[B[x, y, z], z] /. S), y] /. S]] /. SS /. SS1;
eq4 = Numerator[Factor[Factor[D[(D[Cc[x, y, z], x] /. S), y] /. S] -
  Factor[D[(D[Cc[x, y, z], y] /. S), x] /. S]] /. SS /. SS1;
eq5 = Numerator[Factor[Factor[D[(D[Cc[x, y, z], x] /. S), z] /. S] -
  Factor[D[(D[Cc[x, y, z], z] /. S), x] /. S]] /. SS /. SS1;
eq6 = Numerator[Factor[Factor[D[(D[Cc[x, y, z], y] /. S), z] /. S] -
  Factor[D[(D[Cc[x, y, z], z] /. S), y] /. S]] /. SS /. SS1;
eq7 = Numerator[Factor[Factor[D[(D[P[x, y, z], x] /. S), y] /. S] -
  Factor[D[(D[P[x, y, z], y] /. S), x] /. S]] /. SS /. SS1;
eq8 = Numerator[Factor[Factor[D[(D[P[x, y, z], x] /. S), z] /. S] -
  Factor[D[(D[P[x, y, z], z] /. S), x] /. S]] /. SS /. SS1;
eq9 = Numerator[Factor[Factor[D[(D[P[x, y, z], y] /. S), z] /. S] -
  Factor[D[(D[P[x, y, z], z] /. S), y] /. S]] /. SS /. SS1;
eq10 = Numerator[Factor[Factor[D[(D[Q[x, y, z], x] /. S), y] /. S] -
  Factor[D[(D[Q[x, y, z], y] /. S), x] /. S]] /. SS /. SS1;
eq11 = Numerator[Factor[Factor[D[(D[Q[x, y, z], x] /. S), z] /. S] -
  Factor[D[(D[Q[x, y, z], z] /. S), x] /. S]] /. SS /. SS1;
eq12 = Numerator[Factor[Factor[D[(D[Q[x, y, z], y] /. S), z] /. S] -
  Factor[D[(D[Q[x, y, z], z] /. S), y] /. S]] /. SS /. SS1;
eq13 = Numerator[Factor[Factor[D[(D[R[x, y, z], x] /. S), y] /. S] -
  Factor[D[(D[R[x, y, z], y] /. S), x] /. S]] /. SS /. SS1;
eq14 = Numerator[Factor[Factor[D[(D[R[x, y, z], x] /. S), z] /. S] -
  Factor[D[(D[R[x, y, z], z] /. S), x] /. S]] /. SS /. SS1;
eq15 = Numerator[Factor[Factor[D[(D[R[x, y, z], y] /. S), z] /. S] -
  Factor[D[(D[R[x, y, z], z] /. S), y] /. S]] /. SS /. SS1;

deplist = {D[v1[x, y, z], y], D[v1[x, y, z], z], D[v2[x, y, z], x], D[v2[x, y, z], z],
  D[v3[x, y, z], x], D[v3[x, y, z], y], D[phi1[x, y, z], y], D[phi1[x, y, z], z],
  D[phi2[x, y, z], x], D[phi2[x, y, z], z], D[phi3[x, y, z], x], D[phi3[x, y, z], y],
  D[A[x, y, z], x, y], D[A[x, y, z], x, z], D[A[x, y, z], y, z]} /. SS /. SS1;
dep[exp_] := Block[{i}, Do[If[FreeQ[exp, deplist[[i]]], None,
  Print["Depends on ", deplist[[i]]], {i, 1, Length[deplist]}]]
solver[exp_, var_] := Block[{cf}, cf = Factor[Coefficient[exp, var]];
  -Factor[(exp /. var -> 0) / cf]];
listder = {};
listderfin = {};
sys = {eq1, eq2, eq3, eq4, eq5, eq6, eq7, eq8, eq9, eq10, eq11, eq12, eq13, eq14, eq15};

```

```

sys = Complement[sys, {0}];
sys = Sort[sys, LeafCount[#1] < LeafCount[#2] &];
Length[sys]
15

```

```

(*Solving system sys with respect to v1y,v1z,v2x,
v2z,v3x,v3y,φ1y,φ1z,φ2x,φ2z,φ3x,φ3y,axy,axz,ayz*)

```

```

dep[sys[[1]]]

var = φ23;
elem = solver[sys[[1]], var];
rule = var → elem;
AppendTo[listder, rule];

sys1 = {};
Do[AppendTo[sys1, sub[sys[[i]], listder]];
  Print[i], {i, 2, Length[sys]}]

sys1 = Complement[sys1, {0}];
sys1 = Sort[sys1, LeafCount[#1] < LeafCount[#2] &];
Length[sys1]
14

```

```

dep[sys1[[1]]]

var = φ13;
elem = solver[sys1[[1]], var];
rule = var → elem;
AppendTo[listder, rule];

sys2 = {};
Do[AppendTo[sys2, sub[sys1[[i]], listder]];
  Print[i], {i, 2, Length[sys1]}]

sys2 = Complement[sys2, {0}];
sys2 = Sort[sys2, LeafCount[#1] < LeafCount[#2] &];
Length[sys2]
13

```

```

dep[sys2[[1]]]

var = φ12;
elem = solver[sys2[[1]], var];
rule = var → elem;
AppendTo[listder, rule];

```

```

sys3 = {};
Do[AppendTo[sys3, sub[sys2[[i]], listder]];
  Print[i], {i, 2, Length[sys2]}]

sys3 = Complement[sys3, {0}];
sys3 = Sort[sys3, LeafCount[#1] < LeafCount[#2] &];
Length[sys3]
12

dep[sys3[[1]]]

var = v23;
elem = solver[sys3[[1]], var];
rule = var → elem;
AppendTo[listder, rule];

sys4 = {};
Do[AppendTo[sys4, sub[sys3[[i]], listder]];
  Print[i], {i, 2, Length[sys3]}]

sys4 = Complement[sys4, {0}];
sys4 = Sort[sys4, LeafCount[#1] < LeafCount[#2] &];
Length[sys4]
11

dep[sys4[[1]]]

var = v13;
elem = solver[sys4[[1]], var];
rule = var → elem;
AppendTo[listder, rule];

sys5 = {};
Do[AppendTo[sys5, sub[sys4[[i]], listder]];
  Print[i], {i, 2, Length[sys4]}]

sys5 = Complement[sys5, {0}];
sys5 = Sort[sys5, LeafCount[#1] < LeafCount[#2] &];
Length[sys5]
10

dep[sys5[[1]]]

var = v12;
elem = solver[sys5[[1]], var];
rule = var → elem;
AppendTo[listder, rule];

```

```

sys6 = {};
Do[AppendTo[sys6, sub[sys5[[i]], listder]];
  Print[i], {i, 2, Length[sys5]}]

sys6 = Complement[sys6, {0}];
sys6 = Sort[sys6, LeafCount[#1] < LeafCount[#2] &];
Length[sys6]
9

dep[sys6[[1]]]

var = v32;
elem = solver[sys6[[1]], var];
rule = var → elem;
AppendTo[listder, rule];

sys7 = {};
Do[AppendTo[sys7, sub[sys6[[i]], listder]];
  Print[i], {i, 2, Length[sys6]}]

sys7 = Complement[sys7, {0}];
sys7 = Sort[sys7, LeafCount[#1] < LeafCount[#2] &];
Length[sys7]
8

dep[sys7[[1]]]

var = v31;
elem = solver[sys7[[1]], var];
rule = var → elem;
AppendTo[listder, rule];

sys8 = {};
Do[AppendTo[sys8, sub[sys7[[i]], listder]];
  Print[i], {i, 2, Length[sys7]}]

sys8 = Complement[sys8, {0}];
sys8 = Sort[sys8, LeafCount[#1] < LeafCount[#2] &];
Length[sys8]
7

dep[sys8[[1]]]

var = v21;
elem = solver[sys8[[1]], var];
rule = var → elem;
AppendTo[listder, rule];

```

```

sys9 = {};
Do[AppendTo[sys9, sub[sys8[[i]], listder]];
Print[i], {i, 2, Length[sys8]}]

sys9 = Complement[sys9, {0}];
sys9 = Sort[sys9, LeafCount[#1] < LeafCount[#2] &];
Length[sys9]
6

dep[sys9[[1]]]

var =  $\phi_{32}$ ;
elem = solver[sys9[[1]], var];
rule = var  $\rightarrow$  elem;
AppendTo[listder, rule];

sys10 = {};
Do[AppendTo[sys10, sub[sys9[[i]], listder]];
Print[i], {i, 2, Length[sys9]}]

sys10 = Complement[sys10, {0}];
sys10 = Sort[sys10, LeafCount[#1] < LeafCount[#2] &];
Length[sys10]
5

dep[sys10[[1]]]

var =  $\phi_{31}$ ;
elem = solver[sys10[[1]], var];
rule = var  $\rightarrow$  elem;
AppendTo[listder, rule];

sys11 = {};
Do[AppendTo[sys11, sub[sys10[[i]], listder]];
Print[i], {i, 2, Length[sys10]}]

sys11 = Complement[sys11, {0}];
sys11 = Sort[sys11, LeafCount[#1] < LeafCount[#2] &];
Length[sys11]
4

dep[sys11[[1]]]

var =  $\phi_{21}$ ;
elem = solver[sys11[[1]], var];
rule = var  $\rightarrow$  elem;
AppendTo[listder, rule];

```

```

sys12 = {};
Do[AppendTo[sys12, sub[sys11[[i]], listder]];
Print[i], {i, 2, Length[sys11]}]

sys12 = Complement[sys12, {0}];
sys12 = Sort[sys12, LeafCount[#1] < LeafCount[#2] &];
Length[sys12]
3

dep[sys12[[1]]]

factorlist = {-Gb + Fb  $\phi$ 2 - Gq  $\phi$ 2 + Fq  $\phi$ 22, -(-Gb + Fb  $\phi$ 2 - Gq  $\phi$ 2 + Fq  $\phi$ 22),
  -Gb + Fb  $\phi$ 3 - Gq  $\phi$ 3 + Fq  $\phi$ 32, -(-Gb + Fb  $\phi$ 3 - Gq  $\phi$ 3 + Fq  $\phi$ 32), ( $\phi$ 2 -  $\phi$ 3)};

killfactor[sys12[[1]]]

var = a23;
elem = solver[killfactor[sys12[[1]]], var];
rule = var → elem;
AppendTo[listder, rule];
AppendTo[listderfin, rule];

killfactor[sys12[[2]]]

AppendTo[factorlist,  $\phi$ 1 -  $\phi$ 3];
AppendTo[factorlist, (-Gb + Fb  $\phi$ 1 - Gq  $\phi$ 1 + Fq  $\phi$ 12)];

killfactor[sys12[[2]]]

dep[sys12[[2]]]

var = a13;
elem = solver[killfactor[sys12[[2]]], var];
rule = var → elem;
AppendTo[listder, rule];
AppendTo[listderfin, rule];

killfactor[sys12[[3]]]

AppendTo[factorlist, ( $\phi$ 1 -  $\phi$ 2)];

killfactor[sys12[[3]]]

var = a12;
elem = solver[killfactor[sys12[[3]]], var];
rule = var → elem;
AppendTo[listder, rule];
AppendTo[listderfin, rule];

Length[listderfin]
3

```

```

dep[sys11[[1]]]
jj = sub[sys11[[1]], listderfin];
dep[jj]

var =  $\phi_{21}$ ;
elem = solver[killfactor[jj], var];
rule = var  $\rightarrow$  elem;
AppendTo[listder, rule];
AppendTo[listderfin, rule];

jj = sub[sys10[[1]], listderfin];
dep[jj]

var =  $\phi_{31}$ ;
elem = solver[killfactor[jj], var];
rule = var  $\rightarrow$  elem;
AppendTo[listder, rule];
AppendTo[listderfin, rule];

jj = sub[sys9[[1]], listderfin];
dep[jj]

var =  $\phi_{32}$ ;
elem = solver[killfactor[jj], var];
rule = var  $\rightarrow$  elem;
AppendTo[listder, rule];
AppendTo[listderfin, rule];

jj = sub[sys8[[1]], listderfin];
dep[jj]

var =  $v_{21}$ ;
elem = solver[killfactor[jj], var];
rule = var  $\rightarrow$  elem;
AppendTo[listder, rule];
AppendTo[listderfin, rule];

jj = sub[sys7[[1]], listderfin];
dep[jj]

var =  $v_{31}$ ;
elem = solver[killfactor[jj], var];
rule = var  $\rightarrow$  elem;
AppendTo[listder, rule];
AppendTo[listderfin, rule];

jj = sub[sys6[[1]], listderfin];
dep[jj]

```

```

var = v32;
elem = solver[killfactor[jj], var];
rule = var → elem;
AppendTo[listder, rule];
AppendTo[listderfin, rule];

jj = sub[sys5[[1]], listderfin];
dep[jj]

var = v12;
elem = solver[killfactor[jj], var];
rule = var → elem;
AppendTo[listder, rule];
AppendTo[listderfin, rule];

jj = sub[sys4[[1]], listderfin];
dep[jj]

var = v13;
elem = solver[killfactor[jj], var];
rule = var → elem;
AppendTo[listder, rule];
AppendTo[listderfin, rule];

jj = sub[sys3[[1]], listderfin];
dep[jj]

var = v23;
elem = solver[killfactor[jj], var];
rule = var → elem;
AppendTo[listder, rule];
AppendTo[listderfin, rule];

jj = sub[sys2[[1]], listderfin];
dep[jj]

var = ϕ12;
elem = solver[killfactor[jj], var];
rule = var → elem;
AppendTo[listder, rule];
AppendTo[listderfin, rule];

jj = sub[sys1[[1]], listderfin];
dep[jj]

```



```

var =  $\phi$ 13;
elem = solver[killfactor[jj], var];
rule = var  $\rightarrow$  elem;
AppendTo[listder, rule];
AppendTo[listderfin, rule];

jj = sub[sys[[1]], listderfin];
dep[jj]

var =  $\phi$ 23;
elem = solver[killfactor[jj], var];
rule = var  $\rightarrow$  elem;
AppendTo[listder, rule];
AppendTo[listderfin, rule];

listderfinsim = listderfin;

```

(\*Computing the compatibility conditions v123=v132\*)

```

inca[exp_] :=
Block[{}, exp /. {Fa  $\rightarrow$  Faa, Fb  $\rightarrow$  Fab, Fc  $\rightarrow$  Fac, Fp  $\rightarrow$  Fap, Fq  $\rightarrow$  Faq, Fr  $\rightarrow$  Far, Ga  $\rightarrow$  Gaa,
Gb  $\rightarrow$  Gab, Gc  $\rightarrow$  Gac, Gp  $\rightarrow$  Gap, Gq  $\rightarrow$  Gaq, Gr  $\rightarrow$  Gar, Faa  $\rightarrow$  Faaa, Fab  $\rightarrow$  Faab,
Fac  $\rightarrow$  Faac, Fap  $\rightarrow$  Faap, Faq  $\rightarrow$  Faaq, Far  $\rightarrow$  Faar, Fbb  $\rightarrow$  Fabb, Fbc  $\rightarrow$  Fabc, Fbp  $\rightarrow$  Fabp,
Fbq  $\rightarrow$  Fabq, Fbr  $\rightarrow$  Fabr, Fcc  $\rightarrow$  Facc, Fcp  $\rightarrow$  Facp, Fcq  $\rightarrow$  Facq, Fcr  $\rightarrow$  Facr, Fpp  $\rightarrow$  Fapp,
Fpq  $\rightarrow$  Fapq, Fpr  $\rightarrow$  Fapr, Fqq  $\rightarrow$  Faqq, Fqr  $\rightarrow$  Faqr, Frr  $\rightarrow$  Farr, Gaa  $\rightarrow$  Gaaa, Gab  $\rightarrow$  Gaab,
Gac  $\rightarrow$  Gaac, Gap  $\rightarrow$  Gaap, Gaq  $\rightarrow$  Gaaq, Gar  $\rightarrow$  Gaar, Gbb  $\rightarrow$  Gabb, Gbc  $\rightarrow$  Gabc, Gbp  $\rightarrow$  Gabp,
Gbq  $\rightarrow$  Gabq, Gbr  $\rightarrow$  Gabr, Gcc  $\rightarrow$  Gacc, Gcp  $\rightarrow$  Gacp, Gcq  $\rightarrow$  Gacq, Gcr  $\rightarrow$  Gacr,
Gpp  $\rightarrow$  Gapp, Gpq  $\rightarrow$  Gapq, Gpr  $\rightarrow$  Gapr, Gqq  $\rightarrow$  Gaqq, Gqr  $\rightarrow$  Gaqr, Grr  $\rightarrow$  Garr}]]

incb[exp_] := Block[{}, exp /. {Fa  $\rightarrow$  Fab, Fb  $\rightarrow$  Fbb, Fc  $\rightarrow$  Fbc, Fp  $\rightarrow$  Fbp, Fq  $\rightarrow$  Fbq,
Fr  $\rightarrow$  Fbr, Ga  $\rightarrow$  Gab, Gb  $\rightarrow$  Gbb, Gc  $\rightarrow$  Gbc, Gp  $\rightarrow$  Gbp, Gq  $\rightarrow$  Gbq, Gr  $\rightarrow$  Gbr, Faa  $\rightarrow$  Faab,
Fab  $\rightarrow$  Fabb, Fac  $\rightarrow$  Fabc, Fap  $\rightarrow$  Fabp, Faq  $\rightarrow$  Fabq, Far  $\rightarrow$  Fabr, Fbb  $\rightarrow$  Fbbb, Fbc  $\rightarrow$  Fbbc,
Fbp  $\rightarrow$  Fbbp, Fbq  $\rightarrow$  Fbbq, Fbr  $\rightarrow$  Fbbr, Fcc  $\rightarrow$  Fbcc, Fcp  $\rightarrow$  Fbc p, Fcq  $\rightarrow$  Fbcq, Fcr  $\rightarrow$  Fbcr,
Fpp  $\rightarrow$  Fbpp, Fpq  $\rightarrow$  Fbpq, Fpr  $\rightarrow$  Fbpr, Fqq  $\rightarrow$  Fbqq, Fqr  $\rightarrow$  Fbqr, Frr  $\rightarrow$  Fbrr, Gaa  $\rightarrow$  Gaab,
Gab  $\rightarrow$  Gabb, Gac  $\rightarrow$  Gabc, Gap  $\rightarrow$  Gabp, Gaq  $\rightarrow$  Gabq, Gar  $\rightarrow$  Gabr, Gbb  $\rightarrow$  Gbbb, Gbc  $\rightarrow$  Gbbc,
Gbp  $\rightarrow$  Gbbp, Gbq  $\rightarrow$  Gbbq, Gbr  $\rightarrow$  Gbbr, Gcc  $\rightarrow$  Gbcc, Gcp  $\rightarrow$  Gbc p, Gcq  $\rightarrow$  Gbcq, Gcr  $\rightarrow$  Gbcr,
Gpp  $\rightarrow$  Gbpp, Gpq  $\rightarrow$  Gbpq, Gpr  $\rightarrow$  Gbpr, Gqq  $\rightarrow$  Gbqq, Gqr  $\rightarrow$  Gbqr, Grr  $\rightarrow$  Gbrr}]]

incc[exp_] := Block[{}, exp /. {Fa  $\rightarrow$  Fac, Fb  $\rightarrow$  Fbc, Fc  $\rightarrow$  Fcc, Fp  $\rightarrow$  Fcp, Fq  $\rightarrow$  Fcq,
Fr  $\rightarrow$  Fcr, Ga  $\rightarrow$  Gac, Gb  $\rightarrow$  Gbc, Gc  $\rightarrow$  Gcc, Gp  $\rightarrow$  Gcp, Gq  $\rightarrow$  Gcq, Gr  $\rightarrow$  Gcr, Faa  $\rightarrow$  Faac,
Fab  $\rightarrow$  Fabc, Fac  $\rightarrow$  Facc, Fap  $\rightarrow$  Facp, Faq  $\rightarrow$  Facq, Far  $\rightarrow$  Facr, Fbb  $\rightarrow$  Fbbc, Fbc  $\rightarrow$  Fbcc,
Fbp  $\rightarrow$  Fbc p, Fbq  $\rightarrow$  Fbcq, Fbr  $\rightarrow$  Fbcr, Fcc  $\rightarrow$  Fccc, Fcp  $\rightarrow$  Fcc p, Fcq  $\rightarrow$  Fccq, Fcr  $\rightarrow$  Fccr,
Fpp  $\rightarrow$  Fcpp, Fpq  $\rightarrow$  Fcpq, Fpr  $\rightarrow$  Fcpr, Fqq  $\rightarrow$  Fcqq, Fqr  $\rightarrow$  Fcqr, Frr  $\rightarrow$  Fcrr, Gaa  $\rightarrow$  Gaac,
Gab  $\rightarrow$  Gabc, Gac  $\rightarrow$  Gacc, Gap  $\rightarrow$  Gacp, Gaq  $\rightarrow$  Gacq, Gar  $\rightarrow$  Gacr, Gbb  $\rightarrow$  Gbbc, Gbc  $\rightarrow$  Gbcc,
Gbp  $\rightarrow$  Gbc p, Gbq  $\rightarrow$  Gbcq, Gbr  $\rightarrow$  Gbcr, Gcc  $\rightarrow$  Gccc, Gcp  $\rightarrow$  Gcc p, Gcq  $\rightarrow$  Gccq, Gcr  $\rightarrow$  Gccr,
Gpp  $\rightarrow$  Gcpp, Gpq  $\rightarrow$  Gcpq, Gpr  $\rightarrow$  Gcpr, Gqq  $\rightarrow$  Gcqq, Gqr  $\rightarrow$  Gcqr, Grr  $\rightarrow$  Gcrr}]]

incp[exp_] := Block[{}, exp /. {Fa  $\rightarrow$  Fap, Fb  $\rightarrow$  Fbp, Fc  $\rightarrow$  Fcp, Fp  $\rightarrow$  Fpp, Fq  $\rightarrow$  Fpq,
Fr  $\rightarrow$  Fpr, Ga  $\rightarrow$  Gap, Gb  $\rightarrow$  Gbp, Gc  $\rightarrow$  Gcp, Gp  $\rightarrow$  Gpp, Gq  $\rightarrow$  Gpq, Gr  $\rightarrow$  Gpr, Faa  $\rightarrow$  Faap,

```

```

Fab → Fabp, Fac → Facp, Fap → Fapp, Faq → Fapq, Far → Fapr, Fbb → Fbbp, Fbc → Fbcp,
Fbp → Fbpp, Fbq → Fbpq, Fbr → Fbpr, Fcc → Fccp, Fcp → Fcpp, Fcq → Fcpq, Fcr → Fcpr,
Fpp → Fppp, Fpq → Fppq, Fpr → Fppr, Fqq → Fpqq, Fqr → Fpqr, Frr → Fprr, Gaa → Gaap,
Gab → Gabp, Gac → Gacp, Gap → Gapp, Gaq → Gapq, Gar → Gapr, Gbb → Gbbp, Gbc → Gbcp,
Gbp → Gbpp, Gbq → Gbpq, Gbr → Gbpr, Gcc → Gccp, Gcp → Gcpp, Gcq → Gcpq, Gcr → Gcpr,
Gpp → Gppp, Gpq → Gppq, Gpr → Gppr, Gqq → Gpqq, Gqr → Gpqr, Grr → Gprr}]
incq[exp_] := Block[{ }, exp /. {Fa → Faq, Fb → Fbq, Fc → Fcq, Fp → Fpq, Fq → Fqq,
Fr → Fqr, Ga → Gaq, Gb → Gbq, Gc → Gcq, Gp → Gpq, Gq → Gqq, Gr → Gqr, Faa → Faaq,
Fab → Fabq, Fac → Facq, Fap → Fapq, Faq → Faqq, Far → Faqr, Fbb → Fbbq, Fbc → Fbcq,
Fbp → Fbpq, Fbq → Fbqq, Fbr → Fbqr, Fcc → Fccq, Fcp → Fcpq, Fcq → Fcqq, Fcr → Fcqr,
Fpp → Fppq, Fpq → Fpqq, Fpr → Fpqr, Fqq → Fqqq, Fqr → Fqqr, Frr → Fqrr, Gaa → Gaaq,
Gab → Gabq, Gac → Gacq, Gap → Gapq, Gaq → Gaqq, Gar → Gaqr, Gbb → Gbbq, Gbc → Gbcq,
Gbp → Gbpq, Gbq → Gbqq, Gbr → Gbqr, Gcc → Gccq, Gcp → Gcpq, Gcq → Gcqq, Gcr → Gcqr,
Gpp → Gppq, Gpq → Gpqq, Gpr → Gpqr, Gqq → Gqqq, Gqr → Gqqr, Grr → Gqrr}]
incr[exp_] := Block[{ }, exp /. {Fa → Far, Fb → Fbr, Fc → Fcr, Fp → Fpr, Fq → Fqr,
Fr → Frr, Ga → Gar, Gb → Gbr, Gc → Gcr, Gp → Gpr, Gq → Gqr, Gr → Grr, Faa → Faar,
Fab → Fabr, Fac → Facr, Fap → Fapr, Faq → Faqr, Far → Farr, Fbb → Fbbr, Fbc → Fbcr,
Fbp → Fbpr, Fbq → Fbqr, Fbr → Fbrr, Fcc → Fccr, Fcp → Fcpr, Fcq → Fcqr, Fcr → Fcrr,
Fpp → Fppr, Fpq → Fpqr, Fpr → Fprr, Fqq → Fqqr, Fqr → Fqrr, Frr → Frrr, Gaa → Gaar,
Gab → Gabr, Gac → Gacr, Gap → Gapr, Gaq → Gaqr, Gar → Garr, Gbb → Gbbr, Gbc → Gbcr,
Gbp → Gbpr, Gbq → Gbqr, Gbr → Gbrr, Gcc → Gccr, Gcp → Gcpr, Gcq → Gcqr, Gcr → Gcrr,
Gpp → Gppr, Gpq → Gpqr, Gpr → Gprr, Gqq → Gqqr, Gqr → Gqrr, Grr → Grrr}]
D1fg[exp_] := Block[{res}, res = Factor[inca[exp] (a1 /. Sf) +
incb[exp] (b1 /. Sf) + incc[exp] (c1 /. Sf) + incp[exp] (p1 /. Sf) +
incq[exp] (q1 /. Sf) + incr[exp] (rr1 /. Sf)];
res];
D2fg[exp_] := Block[{res}, res = Factor[
inca[exp] (a2 /. Sf) + incb[exp] (b2 /. Sf) + incc[exp] (c2 /. Sf) +
incp[exp] (p2 /. Sf) + incq[exp] (q2 /. Sf) + incr[exp] (rr2 /. Sf)];
res];
D3fg[exp_] := Block[{res}, res = Factor[
inca[exp] (a3 /. Sf) + incb[exp] (b3 /. Sf) + incc[exp] (c3 /. Sf) +
incp[exp] (p3 /. Sf) + incq[exp] (q3 /. Sf) + incr[exp] (rr3 /. Sf)];
res];
together[e1_, e2_] := Block[{n1 = Numerator[e1], n2 = Numerator[e2], d1 = Denominator[e1],
d2 = Denominator[e2], gcd, dd1, dd2}, gcd = PolynomialGCD[d1, d2];
dd1 = Factor[d1/gcd];
dd2 = Factor[d2/gcd];
(n1 dd2 + n2 dd1) / dd1 / dd2 / gcd];
together1[e1_, e2_] :=
Block[{n1 = Numerator[e1], n2 = Numerator[e2], d1 = Denominator[e1],
d2 = Denominator[e2], gcd, dd1, dd2}, gcd = PolynomialGCD[d1, d2];
dd1 = Factor[d1/gcd];
dd2 = Factor[d2/gcd];
Factor[(n1 dd2 + n2 dd1) / dd1 / dd2 / gcd]].

```

```

(*v123=v132*)

var1 = v12 /. listderfinsim;
var2 = v13 /. listderfinsim;

expf = 0;

varsfg = {Fa, Fb, Fc};

Do[v1 = varsfg[[i]];
  exp1 = der[var1, v1] D3fg[v1];
  Print["Part 1 of variable ", v1, " is done"];
  exp2 = -der[var2, v1] D2fg[v1];
  Print["Part 2 of variable ", v1, " is done"];
  exp3 = together1[exp1, exp2];
  Print["Part 3 of variable ", v1, " is done"];
  expf = together[expf, exp3];
  Print["===== Variable ", v1, " is done ====="],
  {i, 1, Length[varsfg]}]

varsfg = {Fp, Fq, Fr};

Do[v1 = varsfg[[i]];
  exp1 = der[var1, v1] D3fg[v1];
  Print["Part 1 of variable ", v1, " is done"];
  exp2 = -der[var2, v1] D2fg[v1];
  Print["Part 2 of variable ", v1, " is done"];
  exp3 = together1[exp1, exp2];
  Print["Part 3 of variable ", v1, " is done"];
  expf = together[expf, exp3];
  Print["===== Variable ", v1, " is done ====="],
  {i, 1, Length[varsfg]}]

varsfg = {Ga, Gb, Gc};

Do[v1 = varsfg[[i]];
  exp1 = der[var1, v1] D3fg[v1];
  Print["Part 1 of variable ", v1, " is done"];
  exp2 = -der[var2, v1] D2fg[v1];
  Print["Part 2 of variable ", v1, " is done"];
  exp3 = together1[exp1, exp2];
  Print["Part 3 of variable ", v1, " is done"];
  expf = together[expf, exp3];
  Print["===== Variable ", v1, " is done ====="],
  {i, 1, Length[varsfg]}]

```

```
varsfg = {Gp, Gq, Gr, Faa, Fab, Fac, Fap, Faq, Far, Fbb, Fbc, Fbp, Fbq, Fbr, Fcc,
  Fcp, Fcq, Fcr, Fpp, Fpq, Fpr, Fqq, Fqr, Frr, Gaa, Gab, Gac, Gap, Gaq, Gar,
  Gbb, Gbc, Gbp, Gbq, Gbr, Gcc, Gcp, Gcq, Gcr, Gpp, Gpq, Gpr, Gqq, Gqr, Grr};
```

```
Do[v1 = varsfg[[i]];
  exp1 = der[var1, v1] D3fg[v1];
  Print["Part 1 of variable ", v1, " is done"];
  exp2 = -der[var2, v1] D2fg[v1];
  Print["Part 2 of variable ", v1, " is done"];
  exp3 = together1[exp1, exp2];
  Print["Part 3 of variable ", v1, " is done"];
  expf = together[expf, exp3];
  Print["===== Variable ", v1, " is done ====="],
  {i, 1, Length[varsfg]}]
```

```
exp1 = der[var1,  $\phi_1$ ] ( $\phi_{13}$  /. listderfinsim);
Print["Part 1 of  $\phi_1$  is done"];
exp2 = -der[var2,  $\phi_1$ ] ( $\phi_{12}$  /. listderfinsim);
Print["Part 2 of  $\phi_1$  is done"];
exp3 = together1[exp1, exp2];
Print["Part 3 of  $\phi_1$  is done"];
expf = together[expf, exp3];
Print[" $\phi_1$  is done"];
```

```
exp1 = der[var1,  $\phi_2$ ] ( $\phi_{23}$  /. listderfinsim);
Print["Part 1 of  $\phi_2$  is done"];
exp2 = -der[var2,  $\phi_2$ ] ( $\phi_{22}$  /. listderfinsim);
Print["Part 2 of  $\phi_2$  is done"];
exp3 = together1[exp1, exp2];
Print["Part 3 of  $\phi_2$  is done"];
expf = together[expf, exp3];
Print[" $\phi_2$  is done"];
```

```
exp1 = der[var1,  $\phi_3$ ] ( $\phi_{33}$  /. listderfinsim);
Print["Part 1 of  $\phi_3$  is done"];
exp2 = -der[var2,  $\phi_3$ ] ( $\phi_{32}$  /. listderfinsim);
Print["Part 2 of  $\phi_3$  is done"];
exp3 = together1[exp1, exp2];
Print["Part 3 of  $\phi_3$  is done"];
expf = together[expf, exp3];
Print[" $\phi_3$  is done"];
```

```
exp1 = der[var1, v1] ( $v_{13}$  /. listderfinsim);
Print["Part 1 of v1 is done"];
```

```

exp2 = -der[var2, v1] (v12 /. listderfinsim);
Print["Part 2 of v1 is done"];
exp3 = together1[exp1, exp2];
Print["Part 3 of v1 is done"];
expf = together[expf, exp3];
Print["v1 is done"];

```

```

exp1 = der[var1, v2] (v23 /. listderfinsim);
Print["Part 1 of v2 is done"];
exp2 = -der[var2, v2] (v22 /. listderfinsim);
Print["Part 2 of v2 is done"];
exp3 = together1[exp1, exp2];
Print["Part 3 of v2 is done"];
expf = together[expf, exp3];
Print["v2 is done"];

```

```

exp1 = der[var1, v3] (v33 /. listderfinsim);
Print["Part 1 of v3 is done"];
exp2 = -der[var2, v3] (v32 /. listderfinsim);
Print["Part 2 of v3 is done"];
exp3 = together1[exp1, exp2];
Print["Part 3 of v3 is done"];
expf = together[expf, exp3];
Print["v3 is done"];

```

```

exp1 = der[var1, a1] (a13 /. listderfinsim);
Print["Part 1 of a1 is done"];
exp2 = -der[var2, a1] (a12 /. listderfinsim);
Print["Part 2 of a1 is done"];
exp3 = together1[exp1, exp2];
Print["Part 3 of a1 is done"];
expf = together[expf, exp3];
Print["a1 is done"];

```

```

exp1 = der[var1, a2] (a23 /. listderfinsim);
Print["Part 1 of a2 is done"];
exp2 = -der[var2, a2] (a22 /. listderfinsim);
Print["Part 2 of a2 is done"];
exp3 = together1[exp1, exp2];
Print["Part 3 of a2 is done"];
expf = together[expf, exp3];
Print["a2 is done"];

```

```

exp1 = der[var1, a3] (a33 /. listderfinsim);

```

```

Print["Part 1 of a3 is done"];
exp2 = -der[var2, a3] (a23 /. listderfinsim);
Print["Part 2 of a3 is done"];
exp3 = together1[exp1, exp2];
Print["Part 3 of a3 is done"];
expf = together[expf, exp3];
Print["a3 is done"];

cond = expf;

```

(\*cond is a polynomial in a1, a2, a3,  $\phi_1$ ,  $\phi_2$ ,  $\phi_3$ ,  $v_1$ ,  $v_2$ ,  $v_3$ .  
 If the system is integrable then cond=0. All coefficients of cond at a1,  
 a2, a3,  $\phi_1$ ,  $\phi_2$ ,  $\phi_3$ ,  $v_1$ ,  $v_2$ ,  $v_3$  must vanish. Setting a1=  
 a2=a3=1 and taking the coefficient at  $\phi_1^{12} \phi_2^9 \phi_3^6 v_1^6 v_2 v_3^3$  we obtain:  
 \*)

```

jj1 = Coefficient[cond,  $\phi_1$ , 12];
jj2 = Coefficient[jj1,  $\phi_2$ , 9];
jj3 = Coefficient[jj2,  $\phi_3$ , 6];
jj4 = Coefficient[jj3,  $v_1$ , 6];
jj5 = Coefficient[jj4,  $v_2$ , 1];
jj6 = Coefficient[jj5,  $v_3$ , 3];
jj = Factor[jj6];

jj

```

$$\begin{aligned}
& -Fq^5 (Fc Fq Ga - Fb Fr Ga - Fc Fp Gb + Fa Fr Gb + Fb Fp Gc - \\
& Fa Fq Gc - Fr Gb Gp + Fq Gc Gp + Fr Ga Gq - Fp Gc Gq - Fq Ga Gr + Fp Gb Gr)^3 \\
& (-2 Fq Fqr Fr^2 Gb + Fqq Fr^3 Gb + Fq^2 Fr Frr Gb + 2 Fq^2 Fqr Fr Gc - Fq Fqq Fr^2 Gc - Fq^3 Frr Gc + \\
& Fc Fq Fr^2 Gqq - Fb Fr^3 Gqq + Fr^3 Gq Gqq - 2 Fc Fq^2 Fr Gqr + 2 Fb Fq Fr^2 Gqr - 2 Fq Fr^2 Gq Gqr - \\
& Fq Fr^2 Gqq Gr + 2 Fq^2 Fr Gqr Gr + Fc Fq^3 Grr - Fb Fq^2 Fr Grr + Fq^2 Fr Gq Grr - Fq^3 Gr Grr)^2
\end{aligned}$$

```

cond1 =
(-2 Fq Fqr Fr^2 Gb + Fqq Fr^3 Gb + Fq^2 Fr Frr Gb + 2 Fq^2 Fqr Fr Gc - Fq Fqq Fr^2 Gc - Fq^3 Frr Gc +
Fc Fq Fr^2 Gqq - Fb Fr^3 Gqq + Fr^3 Gq Gqq - 2 Fc Fq^2 Fr Gqr + 2 Fb Fq Fr^2 Gqr - 2 Fq Fr^2 Gq Gqr -
Fq Fr^2 Gqq Gr + 2 Fq^2 Fr Gqr Gr + Fc Fq^3 Grr - Fb Fq^2 Fr Grr + Fq^2 Fr Gq Grr - Fq^3 Gr Grr);

```

This cond1 is equivalent to one of the equations of the system of linear degeneracy. In the file SL6-action it is shown that the equivalence group acts transitively on the system, and we deduce there that given only one this equation and SL6-invariance (known apriori for both the integrability property and the system of linear degeneracy). Thus integrability of the 2x2 system describing sixfolds  $X \subset Gr(4,6)$  implies linear degeneracy.
