# Supplementary material for: Integrable systems in 4D associated with sixfolds in Gr(4,6)
Source: arXiv:1705.06999 ancillary file (2017-05-18)
Supplement: Supplementary file 3 [file DFKN-2017-Involution.pdf]

This worksheet accompanies the paper B.Doubrov, E.Ferapontov, B.Kruglikov, V.Novikov "Integrable systems in 4D associated with sixfolds in Gr(4,6)".

The file ran on **Maple** version 17, the package **DifferentialGeometry** was used.

In this worksheet we perform the prolongation-projection analysis of the system of linear degeneracy of 2x2 systems. In other words we complete the system to formally integrable (bring to involution) by adding all compatibility conditions. The computations are excessive, so to simplify them we substitute a nondegenerate 1-jet, which does not restricts the generality due to almost transitivity of the symmetry group action.

```
>
> restart : with (DifferentialGeometry) : with (JetCalculus) : with (PolynomialIdeals) :
  Preferences ("ShowFramePrompt", false) :
> DGsetup([u1, u2, u3, v1, v2, v3], [f, g], J, 3) :
> Ef := (i, j, k) -> (TotalDiff(f[ ], u || k) - TotalDiff(g[ ], v || k)) * TotalDiff(TotalDiff(f[ ], u
  || i), u || j) + TotalDiff(g[ ], u || k) * (TotalDiff(TotalDiff(f[ ], u || i), v || j)
  + TotalDiff(TotalDiff(f[ ], u || j), v || i)) + TotalDiff(f[ ], v || k) * TotalDiff(TotalDiff
  (g[ ], u || i), u || j) + TotalDiff(g[ ], u || k) * TotalDiff(TotalDiff(g[ ], v || i), v || j):
EF := (i, j, k) -> Ef(i, j, k) + Ef(j, k, i) + Ef(k, i, j) :
Eg := (i, j, k) -> (TotalDiff(g[ ], v || k) - TotalDiff(f[ ], u || k)) * TotalDiff(TotalDiff(g[ ], v || i),
  v || j) + TotalDiff(f[ ], v || k) * (TotalDiff(TotalDiff(g[ ], u || i), v || j)
  + TotalDiff(TotalDiff(g[ ], u || j), v || i)) + TotalDiff(g[ ], u || k) * TotalDiff(TotalDiff
  (f[ ], v || i), v || j) + TotalDiff(f[ ], v || k) * TotalDiff(TotalDiff(f[ ], u || i), u || j):
EG := (i, j, k) -> Eg(i, j, k) + Eg(j, k, i) + Eg(k, i, j) :
EQ := {seq(seq(seq(EF(i, j, k), k = j .. 3), j = i .. 3), i = 1 .. 3), seq(seq(seq(EG(i, j, k), k = j
  .. 3), j = i .. 3), i = 1 .. 3)} : nops(EQ)
```

20

(1)

These EQ are the equations of linear degeneracy in 4D: they are 20 in number. We are going to compute differential closure of this second order system.

Below is the nondegenerate 1-jet (called pt) that we are going to substitute throughout our computations (after the proper prolongation is being made) to simplify and compare the output.

```
> pt := {f[1] = 0, f[2] = 1, f[3] = 0, f[4] = 1, f[5] = 0, f[6] = 0, g[1] = 0, g[2] = 0, g[3] = 1,
  g[4] = 0, g[5] = 0, g[6] = 0} :
spt := solve(subs(pt, EQ)); nops(spt)
spt := {f1,1 = -2 g1,4, f1,2 = -f1,4 - g1,3 - g1,5 - g2,4, f1,3 = -f1,5 - f2,4 - g4,5 - g2,3,
  f1,4 = f1,4, f1,5 = f1,5, f1,6 = f1,6, f2,2 = 0, f2,3 = -f4,5 - g2,6 - g3,5 + g4,6, f2,4 = f2,4,
  f2,5 = f4,5 + g2,6 + g3,5 - g4,6, f2,6 = -f3,5 - g5,6 + f4,6 + g3,6, f3,3 = -2 f4,6
  - 2 g3,6, f3,4 = f3,4, f3,5 = f3,5, f3,6 = -f5,6, f4,4 = -2 g1,6 - 2 g3,4 + 2 f1,5 + 2 f2,4
  + 2 g4,5 + 2 g2,3, f4,5 = f4,5, f4,6 = f4,6, f5,5 = 2 g5,6, f5,6 = f5,6, f6,6 = 0, g1,1 = 0, g1,2
  = g1,4, g1,3 = g1,3, g1,4 = g1,4, g1,5 = g1,5, g1,6 = g1,6, g2,2 = 2 f1,4 + 2 g1,3 + 2 g1,5
  + 2 g2,4, g2,3 = g2,3, g2,4 = g2,4, g2,5 = g4,5, g2,6 = g2,6, g3,3 = -2 f1,6 - 2 f3,4
  - 2 g4,6, g3,4 = g3,4, g3,5 = g3,5, g3,6 = g3,6, g4,4 = -2 f1,4 - 2 g1,3, g4,5 = g4,5, g4,6
  = g4,6, g5,5 = 0, g5,6 = g5,6, g6,6 = 2 f5,6}
```

$$\begin{aligned} &> nops(\{f_{1,1} = -2g_{1,4}, f_{1,2} = -f_{1,4} - g_{1,3} - g_{1,5} - g_{2,4}, f_{1,3} = -f_{1,5} - f_{2,4} - g_{4,5} - g_{2,3}, f_{2,2} \\ &= 0, f_{2,3} = -f_{4,5} - g_{2,6} - g_{3,5} + g_{4,6}, f_{2,5} = f_{4,5} + g_{2,6} + g_{3,5} - g_{4,6}, f_{2,6} = -f_{3,5} \\ &- g_{5,6} + f_{4,6} + g_{3,6}, f_{3,3} = -2f_{4,6} - 2g_{3,6}, f_{3,6} = -f_{5,6}, f_{4,4} = -2g_{1,6} - 2g_{3,4} + 2f_{1,5} \\ &+ 2f_{2,4} + 2g_{4,5} + 2g_{2,3}, f_{5,5} = 2g_{5,6}, f_{6,6} = 0, g_{1,1} = 0, g_{1,2} = g_{1,4}, g_{2,2} = 2f_{1,4} \\ &+ 2g_{1,3} + 2g_{1,5} + 2g_{2,4}, g_{2,5} = g_{4,5}, g_{3,3} = -2f_{1,6} - 2f_{3,4} - 2g_{4,6}, g_{4,4} = -2f_{1,4} \\ &- 2g_{1,3}, g_{5,5} = 0, g_{6,6} = 2f_{5,6}\}) \end{aligned}$$

20

(3)

$$\begin{aligned} &> tmp := \{ \} : \text{for } i \text{ to } 42 \text{ do if } lhs(spt[i]) = rhs(spt[i]) \text{ then } tmp := tmp \text{ union } \{lhs(spt[i])\} : \text{fi} \\ &\text{od: } nops(tmp); \\ &simplify(subs(spt, subs(pt, EQ))) \end{aligned}$$

22

{0}

(4)

$$\begin{aligned} &> EQ3 := \{seq(seq(TotalDiff(EQ[i], j), j = 1..6), i = 1..20)\} : nops(EQ3); \\ &EQ3s := simplify(subs(spt, subs(pt, EQ3))) : \\ &jt3 := \{seq(seq(seq(f[i, j, k], k = j..6), j = i..6), i = 1..6), seq(seq(seq(g[i, j, k], k = j..6), j = i \\ &..6), i = 1..6)\} : nops(jt3) \end{aligned}$$

120

112

(5)

EQ3 is the system obtained by 1-prolongation from EQ. The number of equations is  $6 \cdot 20 = 120$ . The number of 3-jet variables is 112, so some combinations of these 3rd order (quasilinear) equations shall give (new? we will see) 2nd order equations.

$$\begin{aligned} &> SI3 := eliminate(EQ3s, jt3) : nops(SI3[1]); \\ &fv3 := \{ \} : \text{for } i \text{ to } nops(SI3[1]) \text{ do if } lhs(SI3[1][i]) = rhs(SI3[1][i]) \text{ then } fv3 := fv3 \\ &\text{union } \{lhs(SI3[1][i])\} : \text{fi:od: } nops(fv3) \end{aligned}$$

112

17

(6)

&gt; fv3

$$\begin{aligned} &\{g_{1,4,6}, g_{2,3,3}, g_{2,3,4}, g_{2,4,4}, g_{2,4,6}, g_{3,3,3}, g_{3,3,4}, g_{3,3,5}, g_{3,4,4}, g_{3,4,5}, g_{3,4,6}, g_{3,5,6}, \\ &g_{4,4,4}, g_{4,4,5}, g_{4,4,6}, g_{4,5,6}, g_{4,6,6}\} \end{aligned}$$

(7)

So there are  $112 - 17 = 95$  equations with independent 3-symbol among 120 third order equations in EQ3. The free jets are fv3 (in totality 17). SI3[2] gives the equations of the 2nd order (pt substituted) that are obtained by the projection (these are differential syzygies from EQ3). We see it is the quadratic ideal by the 2-jet variables (dependence on 1-jet is more complicated, but it is of no importance for this computation).

&gt; SI3[2]

$$\begin{aligned} &\{f_{5,6}(f_{3,5} - f_{4,6} - g_{3,6} + g_{5,6}), g_{1,4}g_{1,5}, g_{1,5}(g_{2,6} + g_{3,5} - g_{4,6}), g_{1,5}(g_{1,6} - g_{2,3} \\ &+ g_{3,4} - g_{4,5}), g_{5,6}g_{1,5}, f_{1,4}g_{1,5} - f_{1,5}g_{1,4} + g_{1,4}g_{1,6} - g_{1,4}g_{4,5}, f_{1,5}g_{5,6} \\ &- f_{5,6}g_{1,5} - g_{1,6}g_{5,6} + g_{4,5}g_{5,6}, 3f_{1,4}g_{1,5} - f_{1,5}g_{1,4} + g_{1,3}g_{1,5} + g_{1,4}g_{1,6} \end{aligned}$$

(8)

$$\begin{aligned}
& -g_{1,4}g_{4,5} + g_{1,5}^2 + g_{1,5}g_{2,4}f_{1,5}f_{5,6} + f_{1,6}g_{5,6} - f_{4,5}g_{5,6} - f_{5,6}g_{1,6} + f_{5,6}g_{4,5} \\
& -g_{3,5}g_{5,6} + g_{4,6}g_{5,6}f_{3,5}g_{2,3} + f_{3,5}g_{4,5} - f_{4,6}g_{2,3} - f_{4,6}g_{4,5} - g_{2,3}g_{3,6} \\
& + g_{2,3}g_{5,6} - g_{3,6}g_{4,5} + g_{4,5}g_{5,6}f_{1,4}f_{1,5} - f_{1,4}g_{1,6} + f_{1,4}g_{4,5} + f_{1,6}g_{1,4} \\
& -f_{4,5}g_{1,4} - g_{1,4}g_{3,5} + g_{1,4}g_{4,6} - g_{1,5}g_{1,6} - g_{1,5}g_{3,4}f_{1,6}f_{5,6} - 2f_{3,5}g_{3,6} \\
& -f_{3,5}g_{5,6} - f_{4,5}f_{5,6} + 2f_{4,6}g_{3,6} + f_{4,6}g_{5,6} - f_{5,6}g_{3,5} + f_{5,6}g_{4,6} + 2g_{3,6}^2 \\
& -g_{3,6}g_{5,6} - g_{5,6}^2, 2f_{1,6}f_{5,6} - f_{3,5}g_{3,6} + f_{3,5}g_{5,6} - 2f_{4,5}f_{5,6} + f_{4,6}g_{3,6} \\
& -f_{4,6}g_{5,6} - 2f_{5,6}g_{3,5} + 2f_{5,6}g_{4,6} + g_{3,6}^2 - 2g_{3,6}g_{5,6} + g_{5,6}^2, 3f_{1,5}g_{1,3} \\
& + 3f_{1,5}g_{1,5} + 3f_{1,5}g_{2,4} - 6f_{1,6}g_{1,4} + 6f_{4,5}g_{1,4} - 3g_{1,3}g_{1,6} + 3g_{1,3}g_{4,5} \\
& + 6g_{1,4}g_{3,5} - 6g_{1,4}g_{4,6} - 2g_{1,5}g_{1,6} + 2g_{1,5}g_{2,3} + g_{1,5}g_{3,4} + 5g_{1,5}g_{4,5} \\
& - 3g_{1,6}g_{2,4} + 3g_{2,4}g_{4,5}f_{1,4}f_{3,5} - f_{1,4}f_{4,6} - f_{1,4}g_{3,6} + f_{1,4}g_{5,6} + f_{3,5}g_{1,3} \\
& + f_{3,5}g_{1,5} + f_{3,5}g_{2,4} - f_{4,6}g_{1,3} - f_{4,6}g_{1,5} - f_{4,6}g_{2,4} - g_{1,3}g_{3,6} + g_{1,3}g_{5,6} \\
& - g_{1,5}g_{3,6} + g_{1,5}g_{5,6} - g_{2,4}g_{3,6} + g_{2,4}g_{5,6}f_{1,5}g_{1,6} - f_{1,5}g_{2,3} + f_{1,5}g_{3,4} \\
& - f_{1,5}g_{4,5} - f_{1,6}g_{1,5} - f_{3,4}g_{1,5} - 2g_{1,5}g_{2,6} - 2g_{1,5}g_{3,5} + 2g_{1,5}g_{4,6} - g_{1,6}^2 \\
& + g_{1,6}g_{2,3} - g_{1,6}g_{3,4} + 2g_{1,6}g_{4,5} - g_{2,3}g_{4,5} + g_{3,4}g_{4,5} - g_{4,5}^2, f_{1,4}f_{3,5} \\
& - f_{1,4}f_{4,6} - f_{1,4}g_{3,6} + f_{1,4}g_{5,6} + f_{1,5}f_{1,6} + f_{1,5}f_{3,4} + f_{1,6}g_{3,4} + f_{1,6}g_{4,5} \\
& - f_{3,4}g_{1,6} + f_{3,4}g_{4,5} - f_{4,5}g_{1,6} - f_{4,5}g_{3,4} - g_{1,5}g_{3,6} - g_{1,6}g_{3,5} + g_{1,6}g_{4,6} \\
& - g_{3,4}g_{3,5} + g_{3,4}g_{4,6}f_{1,4}f_{1,6} - f_{1,4}f_{4,5} - f_{1,4}g_{3,5} + f_{1,4}g_{4,6} + f_{1,6}g_{1,3} \\
& + f_{1,6}g_{1,5} + f_{1,6}g_{2,4} - f_{3,5}g_{1,4} - f_{4,5}g_{1,3} - f_{4,5}g_{1,5} - f_{4,5}g_{2,4} + f_{4,6}g_{1,4} \\
& - g_{1,3}g_{3,5} + g_{1,3}g_{4,6} + g_{1,4}g_{3,6} - g_{1,4}g_{5,6} + g_{1,5}g_{2,6} - g_{2,4}g_{3,5} + g_{2,4}g_{4,6}, \\
& f_{1,6}f_{3,5} - f_{1,6}f_{4,6} - f_{1,6}g_{3,6} + f_{1,6}g_{5,6} + f_{3,4}f_{3,5} - f_{3,4}f_{4,6} - f_{3,4}g_{3,6} + f_{3,4}g_{5,6} \\
& - f_{3,5}g_{2,6} - f_{3,5}g_{3,5} + f_{3,5}g_{4,6} + f_{4,6}g_{2,6} + f_{4,6}g_{3,5} - f_{4,6}g_{4,6} + g_{2,6}g_{3,6} \\
& - g_{2,6}g_{5,6} + g_{3,5}g_{3,6} - g_{3,5}g_{5,6} - g_{3,6}g_{4,6} + g_{4,6}g_{5,6}, 3f_{1,5}f_{5,6} - f_{1,6}f_{3,5} \\
& + f_{1,6}f_{4,6} - 2f_{1,6}g_{3,6} - f_{1,6}g_{5,6} - f_{3,4}f_{3,5} + f_{3,4}f_{4,6} + f_{3,4}g_{3,6} - f_{3,4}g_{5,6} \\
& - 2f_{3,5}g_{2,6} - 2f_{3,5}g_{3,5} + 2f_{3,5}g_{4,6} + 3f_{4,5}g_{3,6} + 2f_{4,6}g_{2,6} + 2f_{4,6}g_{3,5} \\
& - 2f_{4,6}g_{4,6} - 3f_{5,6}g_{1,6} + 3f_{5,6}g_{4,5} + 2g_{2,6}g_{3,6} - 2g_{2,6}g_{5,6} + 5g_{3,5}g_{3,6} \\
& - 2g_{3,5}g_{5,6} - 5g_{3,6}g_{4,6} + 2g_{4,6}g_{5,6}, 3f_{1,4}f_{1,6} - 3f_{1,4}f_{4,5} - 3f_{1,4}g_{3,5} \\
& + 3f_{1,4}g_{4,6} + 2f_{1,5}g_{1,6} + f_{1,5}g_{2,3} + 2f_{1,5}g_{3,4} + f_{1,5}g_{4,5} - 2f_{1,6}g_{1,5}
\end{aligned}$$

$$\begin{aligned}
& -2f_{3,4}g_{1,5} + 3f_{3,5}g_{1,4} - 3f_{4,6}g_{1,4} - 3g_{1,4}g_{3,6} + 3g_{1,4}g_{5,6} + 2g_{1,5}g_{2,6} \\
& + 2g_{1,5}g_{3,5} - 2g_{1,5}g_{4,6} - 2g_{1,6}^2 - g_{1,6}g_{2,3} - 2g_{1,6}g_{3,4} + g_{1,6}g_{4,5} + g_{2,3}g_{4,5} \\
& + 2g_{3,4}g_{4,5} + g_{4,5}^2 f_{1,5}f_{1,6} + f_{1,5}f_{3,4} + 2f_{1,5}g_{2,6} + 2f_{1,5}g_{3,5} - 2f_{1,5}g_{4,6} \\
& - f_{1,6}g_{2,3} + f_{1,6}g_{3,4} - f_{3,4}g_{1,6} + f_{3,4}g_{4,5} - f_{4,5}g_{1,6} + f_{4,5}g_{2,3} - f_{4,5}g_{3,4} \\
& + f_{4,5}g_{4,5} - 3g_{1,5}g_{3,6} + 3g_{1,5}g_{5,6} - 2g_{1,6}g_{2,6} - 3g_{1,6}g_{3,5} + 3g_{1,6}g_{4,6} \\
& + g_{2,3}g_{3,5} - g_{2,3}g_{4,6} + 2g_{2,6}g_{4,5} - g_{3,4}g_{3,5} + g_{3,4}g_{4,6} + 3g_{3,5}g_{4,5} \\
& - 3g_{4,5}g_{4,6} + 2f_{1,6}^2 + 2f_{1,6}f_{3,4} - 2f_{1,6}f_{4,5} - 2f_{1,6}g_{2,6} - 4f_{1,6}g_{3,5} + 4f_{1,6}g_{4,6} \\
& - 2f_{3,4}f_{4,5} - 2f_{3,4}g_{3,5} + 2f_{3,4}g_{4,6} + 2f_{3,5}g_{1,6} + f_{3,5}g_{2,3} + 2f_{3,5}g_{3,4} \\
& + f_{3,5}g_{4,5} + 2f_{4,5}g_{2,6} + 2f_{4,5}g_{3,5} - 2f_{4,5}g_{4,6} - 2f_{4,6}g_{1,6} - f_{4,6}g_{2,3} \\
& - 2f_{4,6}g_{3,4} - f_{4,6}g_{4,5} - 2g_{1,6}g_{3,6} + 2g_{1,6}g_{5,6} - g_{2,3}g_{3,6} + g_{2,3}g_{5,6} \\
& + 2g_{2,6}g_{3,5} - 2g_{2,6}g_{4,6} - 2g_{3,4}g_{3,6} + 2g_{3,4}g_{5,6} + 2g_{3,5}^2 - 4g_{3,5}g_{4,6} \\
& - g_{3,6}g_{4,5} + g_{4,5}g_{5,6} + 2g_{4,6}^2 + 3f_{1,5}g_{3,6} + f_{1,6}^2 + f_{1,6}f_{3,4} - f_{1,6}f_{4,5} + 2f_{1,6}g_{2,6} \\
& + f_{1,6}g_{3,5} - f_{1,6}g_{4,6} - f_{3,4}f_{4,5} - f_{3,4}g_{3,5} + f_{3,4}g_{4,6} + f_{3,5}g_{1,6} - f_{3,5}g_{2,3} \\
& + f_{3,5}g_{3,4} - f_{3,5}g_{4,5} - 2f_{4,5}g_{2,6} - 2f_{4,5}g_{3,5} + 2f_{4,5}g_{4,6} - f_{4,6}g_{1,6} + f_{4,6}g_{2,3} \\
& - f_{4,6}g_{3,4} + f_{4,6}g_{4,5} + 3f_{5,6}g_{1,5} - 4g_{1,6}g_{3,6} + g_{1,6}g_{5,6} + g_{2,3}g_{3,6} - g_{2,3}g_{5,6} \\
& - 2g_{2,6}g_{3,5} + 2g_{2,6}g_{4,6} - g_{3,4}g_{3,6} + g_{3,4}g_{5,6} - 2g_{3,5}^2 + 4g_{3,5}g_{4,6} \\
& + 4g_{3,6}g_{4,5} - g_{4,5}g_{5,6} - 2g_{4,6}^2 + 3f_{1,4}f_{3,5} - 3f_{1,4}f_{4,6} - 3f_{1,4}g_{3,6} + 3f_{1,4}g_{5,6} \\
& + 2f_{1,5}f_{1,6} + 2f_{1,5}f_{3,4} + f_{1,5}g_{2,6} + f_{1,5}g_{3,5} - f_{1,5}g_{4,6} - 2f_{1,6}g_{2,3} + 2f_{1,6}g_{3,4} \\
& - 2f_{3,4}g_{1,6} + 2f_{3,4}g_{4,5} + 3f_{3,5}g_{1,3} + 3f_{3,5}g_{1,5} + 3f_{3,5}g_{2,4} - 2f_{4,5}g_{1,6} \\
& + 2f_{4,5}g_{2,3} - 2f_{4,5}g_{3,4} + 2f_{4,5}g_{4,5} - 3f_{4,6}g_{1,3} - 3f_{4,6}g_{1,5} - 3f_{4,6}g_{2,4} \\
& - 3g_{1,3}g_{3,6} + 3g_{1,3}g_{5,6} - 6g_{1,5}g_{3,6} + 3g_{1,5}g_{5,6} - g_{1,6}g_{2,6} - 3g_{1,6}g_{3,5} \\
& + 3g_{1,6}g_{4,6} + 2g_{2,3}g_{3,5} - 2g_{2,3}g_{4,6} - 3g_{2,4}g_{3,6} + 3g_{2,4}g_{5,6} + g_{2,6}g_{4,5} \\
& - 2g_{3,4}g_{3,5} + 2g_{3,4}g_{4,6} + 3g_{3,5}g_{4,5} - 3g_{4,5}g_{4,6} \}
\end{aligned}$$

Let us solve this system, this is possible because some generators are visually products and this allow to branch the solution space. We get 4 branches.

$\triangleright$  `sl32 := solve(Sl3[2]); nops({sl32})`

$$\begin{aligned}
sl32 &:= \{f_{1,4}=f_{1,4}, f_{1,5}=g_{1,6}-g_{4,5}, f_{1,6}=f_{1,6}, f_{3,4}=f_{3,4}, f_{3,5}=f_{4,6}+g_{3,6}-g_{5,6}, f_{4,5} \\
&= f_{1,6}-g_{3,5}+g_{4,6}, f_{4,6}=f_{4,6}, f_{5,6}=f_{5,6}, g_{1,3}=g_{1,3}, g_{1,4}=g_{1,4}, g_{1,5}=0, g_{1,6} \\
&= g_{1,6}, g_{2,3}=g_{2,3}, g_{2,4}=g_{2,4}, g_{2,6}=g_{2,6}, g_{3,4}=g_{3,4}, g_{3,5}=g_{3,5}, g_{3,6}=g_{3,6}, g_{4,5}
\end{aligned}$$

$$\begin{aligned}
&= g_{4,5}, g_{4,6} = g_{4,6}, g_{5,6} = g_{5,6}, \{f_{1,4} = 0, f_{1,5} = -g_{3,4} - g_{4,5}, f_{1,6} = -f_{3,4}, f_{3,4} = f_{3,4}, \\
&f_{3,5} = f_{4,6}, f_{4,5} = f_{4,5}, f_{4,6} = f_{4,6}, f_{5,6} = 0, g_{1,3} = -g_{2,4}, g_{1,4} = 0, g_{1,5} = 0, g_{1,6} = -g_{3,4}, \\
&g_{2,3} = -g_{4,5}, g_{2,4} = g_{2,4}, g_{2,6} = -g_{3,5} + g_{4,6}, g_{3,4} = g_{3,4}, g_{3,5} = g_{3,5}, g_{3,6} = 0, g_{4,5} \\
&= g_{4,5}, g_{4,6} = g_{4,6}, g_{5,6} = 0\}, \{f_{1,4} = 0, f_{1,5} = f_{1,5}, f_{1,6} = f_{1,6}, f_{3,4} = -f_{1,6}, f_{3,5} = f_{3,5}, \\
&f_{4,5} = f_{4,5}, f_{4,6} = f_{4,6}, f_{5,6} = 0, g_{1,3} = -g_{2,4}, g_{1,4} = 0, g_{1,5} = 0, g_{1,6} = -g_{3,4}, g_{2,3} = \\
&-g_{4,5}, g_{2,4} = g_{2,4}, g_{2,6} = -g_{3,5} + g_{4,6}, g_{3,4} = g_{3,4}, g_{3,5} = g_{3,5}, g_{3,6} = 0, g_{4,5} = g_{4,5}, \\
&g_{4,6} = g_{4,6}, g_{5,6} = 0\}, \{f_{1,4} = 0, f_{1,5} = f_{1,5}, f_{1,6} = f_{1,6}, f_{3,4} = -f_{1,6}, f_{3,5} = f_{3,5}, f_{4,5} \\
&= f_{4,5}, f_{4,6} = f_{4,6}, f_{5,6} = 0, g_{1,3} = -g_{1,5} - g_{2,4}, g_{1,4} = 0, g_{1,5} = g_{1,5}, g_{1,6} = g_{1,6}, g_{2,3} = \\
&-g_{4,5}, g_{2,4} = g_{2,4}, g_{2,6} = -g_{3,5} + g_{4,6}, g_{3,4} = -g_{1,6}, g_{3,5} = g_{3,5}, g_{3,6} = 0, g_{4,5} = g_{4,5}, \\
&g_{4,6} = g_{4,6}, g_{5,6} = 0\}
\end{aligned}$$

4

(9)

> for  $i$  to 4 do  $tmp \parallel i := \{ \}$  :for  $j$  to  $nops(sl32[i])$  do if  $lhs(sl32[i][j]) = rhs(sl32[i][j])$   
then  $tmp \parallel i := tmp \parallel i \cup \{lhs(sl32[i][j])\}$  :fi:od: od:  $seq(nops(sl32[i]) - nops(tmp \parallel i), i = 1..4)$

4, 13, 11, 10

(10)

The most general branch is the one that contains the minimum equations: 4 relations s22. Below we confirm this with PrimeDecomposition (instead of less reliable solve). We get the same number of equations 4, but in addition we find another stratum of the locus of this quadratic ideal.

>  $s22 := eliminate(Sl3[2], \{f_{1,5}, f_{3,5}, f_{4,5}, g_{1,5}\})$   
 $s22 := [\{f_{1,5} = g_{1,6} - g_{4,5}, f_{3,5} = f_{4,6} + g_{3,6} - g_{5,6}, f_{4,5} = f_{1,6} - g_{3,5} + g_{4,6}, g_{1,5} = 0\}, \{ \}]$  (11)

>  $Sl3[2] :$

>  $nops(IdealInfo:-Variables(\langle op(Sl3[2]) \rangle)), nops(MaximalIndependentSet(\langle op(Sl3[2]) \rangle)),$   
 $nops(IdealInfo:-Variables(\langle op(Sl3[2]) \rangle)) - HilbertDimension(\langle op(Sl3[2]) \rangle)$   
21, 17, 4 (12)

>  $PS3 := PrimeDecomposition(\langle op(Sl3[2]) \rangle)$   
 $PS3 := \langle g_{1,5}, f_{1,5} - g_{1,6} + g_{4,5}, -f_{1,6} + f_{4,5} + g_{3,5} - g_{4,6}, -f_{3,5} - g_{5,6} + f_{4,6} + g_{3,6} \rangle,$  (13)  
 $\langle f_{5,6}, g_{1,5}, f_{1,5} - g_{1,6} + g_{4,5}, -f_{1,6} + f_{4,5} + g_{3,5} - g_{4,6}, f_{3,5} - f_{4,6} - g_{3,6} + g_{5,6} \rangle,$   
 $\langle g_{1,4}, g_{1,5}, f_{1,5} - g_{1,6} + g_{4,5}, -f_{1,6} + f_{4,5} + g_{3,5} - g_{4,6}, f_{3,5} - f_{4,6} - g_{3,6} + g_{5,6} \rangle,$   
 $\langle g_{1,5}, g_{3,6}, f_{1,5} - g_{1,6} + g_{4,5}, -g_{5,6} - f_{3,5} + f_{4,6}, -f_{1,6} + f_{4,5} + g_{3,5} - g_{4,6} \rangle, \langle g_{1,5},$   
 $g_{5,6}, f_{1,5} - g_{1,6} + g_{4,5}, -f_{3,5} + f_{4,6} + g_{3,6}, -f_{1,6} + f_{4,5} + g_{3,5} - g_{4,6} \rangle, \langle g_{1,5}, g_{3,6},$   
 $g_{5,6}, -f_{3,5} + f_{4,6}, f_{1,5} - g_{1,6} + g_{4,5}, -f_{1,6} + f_{4,5} + g_{3,5} - g_{4,6} \rangle, \langle f_{5,6}, g_{1,4}, g_{1,5}, g_{5,6},$   
 $f_{1,5} - g_{1,6} + g_{4,5}, f_{3,5} - f_{4,6} - g_{3,6}, -f_{1,6} + f_{4,5} + g_{3,5} - g_{4,6} \rangle, \langle g_{1,4}, g_{1,5}, g_{3,6}, f_{1,4}$   
 $+ g_{1,3} + g_{2,4}, f_{1,5} - g_{1,6} + g_{4,5}, g_{5,6} + f_{3,5} - f_{4,6}, -f_{1,6} + f_{4,5} + g_{3,5} - g_{4,6} \rangle,$   
 $\langle g_{1,4}, g_{1,5}, g_{5,6}, f_{1,4} + g_{1,3} + g_{2,4}, f_{1,5} - g_{1,6} + g_{4,5}, -f_{3,5} + f_{4,6} + g_{3,6}, -f_{1,6} + f_{4,5}$

$$\begin{aligned}
& + g_{3,5} - g_{4,6} \rangle \langle g_{1,4}, g_{1,5}, g_{5,6}, f_{1,4} + g_{1,3} + g_{2,4}, f_{1,5} - g_{1,6} + g_{4,5}, f_{3,5} - f_{4,6} \\
& - g_{3,6}, -f_{1,6} + f_{4,5} + g_{3,5} - g_{4,6} \rangle \langle f_{1,4}, g_{1,4}, g_{1,5}, g_{3,6}, g_{1,3} + g_{2,4}, f_{1,5} - g_{1,6} \\
& + g_{4,5}, g_{5,6} + f_{3,5} - f_{4,6}, -f_{1,6} + f_{4,5} + g_{3,5} - g_{4,6} \rangle \langle f_{1,4}, g_{1,4}, g_{1,5}, g_{5,6}, g_{1,3} \\
& + g_{2,4}, f_{1,5} - g_{1,6} + g_{4,5}, f_{3,5} - f_{4,6} - g_{3,6}, -f_{1,6} + f_{4,5} + g_{3,5} - g_{4,6} \rangle \langle f_{5,6}, g_{1,4}, \\
& g_{1,5}, g_{3,6}, g_{5,6}, f_{3,5} - f_{4,6}, f_{1,5} - g_{1,6} + g_{4,5}, -f_{1,6} + f_{4,5} + g_{3,5} - g_{4,6} \rangle \langle g_{1,4}, g_{1,5}, \\
& g_{3,6}, g_{5,6}, -f_{3,5} + f_{4,6}, f_{1,4} + g_{1,3} + g_{2,4}, f_{1,5} - g_{1,6} + g_{4,5}, -f_{1,6} + f_{4,5} + g_{3,5} \\
& - g_{4,6} \rangle \langle g_{1,4}, g_{1,5}, g_{3,6}, g_{5,6}, f_{3,5} - f_{4,6}, f_{1,4} + g_{1,3} + g_{2,4}, f_{1,5} - g_{1,6} + g_{4,5}, -f_{1,6} \\
& + f_{4,5} + g_{3,5} - g_{4,6} \rangle \langle f_{1,4}, g_{1,4}, g_{1,5}, g_{3,6}, g_{5,6}, f_{3,5} - f_{4,6}, g_{1,3} + g_{2,4}, f_{1,5} - g_{1,6} \\
& + g_{4,5}, -f_{1,6} + f_{4,5} + g_{3,5} - g_{4,6} \rangle \langle f_{1,4}, f_{5,6}, g_{1,4}, g_{3,6}, g_{5,6}, f_{1,6} + f_{3,4}, g_{1,6} + g_{3,4}, \\
& g_{2,3} + g_{4,5}, g_{1,3} + g_{1,5} + g_{2,4}, g_{2,6} + g_{3,5} - g_{4,6} \rangle \langle f_{1,4}, f_{5,6}, g_{1,4}, g_{1,5}, g_{3,6}, g_{5,6}, \\
& f_{1,6} + f_{3,4}, g_{1,3} + g_{2,4}, g_{1,6} + g_{3,4}, g_{2,3} + g_{4,5}, g_{2,6} + g_{3,5} - g_{4,6} \rangle
\end{aligned}$$

> seq([nops(IdealInfo:-Variables(PS3[i])) - HilbertDimension(PS3[i]), i], i = 1  
..nops({PS3}))

[4, 1], [5, 2], [5, 3], [5, 4], [5, 5], [6, 6], [7, 7], [7, 8], [7, 9], [7, 10], [8, 11], [8, 12], [8, 13], [8, 14], [8, 15], [9, 16], [10, 17], [11, 18] (14)

> PS3 :=  $\langle g_{1,5}, f_{1,5} - g_{1,6} + g_{4,5}, -f_{1,6} + f_{4,5} + g_{3,5} - g_{4,6}, -f_{3,5} - g_{5,6} + f_{4,6} + g_{3,6} \rangle,$   
 $\langle f_{5,6}, g_{1,5}, f_{1,5} - g_{1,6} + g_{4,5}, -f_{1,6} + f_{4,5} + g_{3,5} - g_{4,6}, f_{3,5} - f_{4,6} - g_{3,6} + g_{5,6} \rangle,$   
 $\langle g_{1,4}, g_{1,5}, f_{1,5} - g_{1,6} + g_{4,5}, -f_{1,6} + f_{4,5} + g_{3,5} - g_{4,6}, f_{3,5} - f_{4,6} - g_{3,6} + g_{5,6} \rangle,$   
 $\langle g_{1,5}, g_{3,6}, f_{1,5} - g_{1,6} + g_{4,5}, -g_{5,6} - f_{3,5} + f_{4,6}, -f_{1,6} + f_{4,5} + g_{3,5} - g_{4,6} \rangle \langle g_{1,5},$   
 $g_{5,6}, f_{1,5} - g_{1,6} + g_{4,5}, -f_{3,5} + f_{4,6} + g_{3,6}, -f_{1,6} + f_{4,5} + g_{3,5} - g_{4,6} \rangle \langle g_{1,5}, g_{3,6},$   
 $g_{5,6}, -f_{3,5} + f_{4,6}, f_{1,5} - g_{1,6} + g_{4,5}, -f_{1,6} + f_{4,5} + g_{3,5} - g_{4,6} \rangle \langle f_{5,6}, g_{1,4}, g_{1,5}, g_{5,6},$   
 $f_{1,5} - g_{1,6} + g_{4,5}, f_{3,5} - f_{4,6} - g_{3,6}, -f_{1,6} + f_{4,5} + g_{3,5} - g_{4,6} \rangle \langle g_{1,4}, g_{1,5}, g_{3,6}, f_{1,4}$   
 $+ g_{1,3} + g_{2,4}, f_{1,5} - g_{1,6} + g_{4,5}, g_{5,6} + f_{3,5} - f_{4,6}, -f_{1,6} + f_{4,5} + g_{3,5} - g_{4,6} \rangle \langle g_{1,4},$   
 $g_{1,5}, g_{5,6}, f_{1,4} + g_{1,3} + g_{2,4}, f_{1,5} - g_{1,6} + g_{4,5}, -f_{3,5} + f_{4,6} + g_{3,6}, -f_{1,6} + f_{4,5} + g_{3,5}$   
 $- g_{4,6} \rangle \langle g_{1,4}, g_{1,5}, g_{5,6}, f_{1,4} + g_{1,3} + g_{2,4}, f_{1,5} - g_{1,6} + g_{4,5}, f_{3,5} - f_{4,6} - g_{3,6}, -f_{1,6}$   
 $+ f_{4,5} + g_{3,5} - g_{4,6} \rangle \langle f_{1,4}, g_{1,4}, g_{1,5}, g_{3,6}, g_{1,3} + g_{2,4}, f_{1,5} - g_{1,6} + g_{4,5}, g_{5,6} + f_{3,5}$   
 $- f_{4,6}, -f_{1,6} + f_{4,5} + g_{3,5} - g_{4,6} \rangle \langle f_{1,4}, g_{1,4}, g_{1,5}, g_{5,6}, g_{1,3} + g_{2,4}, f_{1,5} - g_{1,6}$   
 $+ g_{4,5}, f_{3,5} - f_{4,6} - g_{3,6}, -f_{1,6} + f_{4,5} + g_{3,5} - g_{4,6} \rangle \langle f_{5,6}, g_{1,4}, g_{1,5}, g_{3,6}, g_{5,6}, f_{3,5}$   
 $- f_{4,6}, f_{1,5} - g_{1,6} + g_{4,5}, -f_{1,6} + f_{4,5} + g_{3,5} - g_{4,6} \rangle \langle g_{1,4}, g_{1,5}, g_{3,6}, g_{5,6}, -f_{3,5}$   
 $+ f_{4,6}, f_{1,4} + g_{1,3} + g_{2,4}, f_{1,5} - g_{1,6} + g_{4,5}, -f_{1,6} + f_{4,5} + g_{3,5} - g_{4,6} \rangle \langle g_{1,4}, g_{1,5},$   
 $g_{3,6}, g_{5,6}, f_{3,5} - f_{4,6}, f_{1,4} + g_{1,3} + g_{2,4}, f_{1,5} - g_{1,6} + g_{4,5}, -f_{1,6} + f_{4,5} + g_{3,5} - g_{4,6} \rangle$   
 $\cdot \langle f_{1,4}, g_{1,4}, g_{1,5}, g_{3,6}, g_{5,6}, f_{3,5} - f_{4,6}, g_{1,3} + g_{2,4}, f_{1,5} - g_{1,6} + g_{4,5}, -f_{1,6} + f_{4,5}$   
 $+ g_{3,5} - g_{4,6} \rangle \langle f_{1,4}, f_{5,6}, g_{1,4}, g_{3,6}, g_{5,6}, f_{1,6} + f_{3,4}, g_{1,6} + g_{3,4}, g_{2,3} + g_{4,5}, g_{1,3}$   
 $+ g_{1,5} + g_{2,4}, g_{2,6} + g_{3,5} - g_{4,6} \rangle \langle f_{1,4}, f_{5,6}, g_{1,4}, g_{1,5}, g_{3,6}, g_{5,6}, f_{1,6} + f_{3,4}, g_{1,3}$   
 $+ g_{2,4}, g_{1,6} + g_{3,4}, g_{2,3} + g_{4,5}, g_{2,6} + g_{3,5} - g_{4,6} \rangle :$

```

> ps3 := i → convert(PS3[i], 'list') :
> seq(subs(solve(ps3(i)), ps3(1)), i = 2..18)
[0, 0, 0, 0], [0, 0, 0, 0], [0, 0, 0, 0], [0, 0, 0, 0], [0, 0, 0, 0], [0, 0, 0, 0], [0, 0, 0, 0], [0, 0, 0, 0],
[0, 0, 0, 0], [0, 0, 0, 0], [0, 0, 0, 0], [0, 0, 0, 0], [0, 0, 0, 0], [0, 0, 0, 0], [0, 0, 0, 0], [0, 0, 0, 0],
[ $g_{1,5}f_{1,5} + g_{3,4} + g_{4,5}f_{3,4} + f_{4,5} + g_{3,5} - g_{4,6}$ ,  $-f_{3,5} + f_{4,6}$ ], [ $0, f_{1,5} + g_{3,4}$ 
+  $g_{4,5}f_{3,4} + f_{4,5} + g_{3,5} - g_{4,6}$ ,  $-f_{3,5} + f_{4,6}$ ]

```

(15)

```

> subs(solve(ps3(18)), ps3(17))
[0, 0, 0, 0, 0, 0, 0, 0, 0, 0]

```

(16)

```

> < $g_{1,5}f_{1,5} - g_{1,6} + g_{4,5}$ ,  $-f_{1,6} + f_{4,5} + g_{3,5} - g_{4,6}$ ,  $-f_{3,5} - g_{5,6} + f_{4,6} + g_{3,6}$ > :
< $f_{1,4}f_{5,6}g_{1,4}g_{3,6}g_{5,6}f_{1,6} + f_{3,4}g_{1,6} + g_{3,4}g_{2,3} + g_{4,5}g_{1,3} + g_{1,5} + g_{2,4}g_{2,6}$ 
+  $g_{3,5} - g_{4,6}$ > :

```

The output of the above investigations is the following: most of the branches of the quadratic ideal (the first 16 of the total 18) are sub-branches of the main branch consisting of 4 equations (that are linear in 2-jets), except for two (numbers 17,18) that form a different branch of 10 equations (that are linear in 2-jets). Thus the locus of the ideal is a reducible variety with the components of codimensions 4 and 10 respectively (they are linear subspaces in the projective spaces that are projectivizations of the fibers  $J^2 \rightarrow J^1$ ).

Recall that these 4 and 10 equations are additional equations that we obtained after substitution spt, so uniting these with 20 equations EQ we obtain the components given by 24 and 30 equations respectively. These can be identified (see Mathematica computations) with the conditions describing general linearly degenerate equations ( $W_+ = 0$ ) and Monge-Ampere 2x2 systems ( $W_- = 0$ ).

```

> Intsc := solve({op(ps3(1)), op(ps3(17))}); tmp := 0 :for i to nops(Intsc) do if lhs(Intsc[i])
≠ rhs(Intsc[i]) then tmp := tmp + 1 :fi:od: tmp
Intsc := { $f_{1,4} = 0, f_{1,5} = -g_{3,4} - g_{4,5}f_{1,6} = f_{4,5} + g_{3,5} - g_{4,6}$ ,  $f_{3,4} = -f_{4,5} - g_{3,5}$ 
+  $g_{4,6}$ ,  $f_{3,5} = f_{4,6}f_{4,5} = f_{4,5}f_{4,6} = f_{4,6}f_{5,6} = 0$ ,  $g_{1,3} = -g_{2,4}$ ,  $g_{1,4} = 0$ ,  $g_{1,5} = 0$ ,  $g_{1,6}$ 
=  $-g_{3,4}$ ,  $g_{2,3} = -g_{4,5}$ ,  $g_{2,4} = g_{2,4}$ ,  $g_{2,6} = -g_{3,5} + g_{4,6}$ ,  $g_{3,4} = g_{3,4}$ ,  $g_{3,5} = g_{3,5}$ ,  $g_{3,6}$ 
=  $0$ ,  $g_{4,5} = g_{4,5}$ ,  $g_{4,6} = g_{4,6}$ ,  $g_{5,6} = 0$ }

```

14

(17)

Here we unite 4 and 10 equations to see the intersection of components. We get 14 equations, or counted together with 20 equations EQ we get 34 equations. These can be identified (see Mathematica computations) with the conditions of linearizability ( $W_+ = W_- = 0$ , or equivalently  $W = 0$ ).

```

> EQ4 := {seq(seq(seq(TotalDiff(TotalDiff(EQ[i], j), k), k = j..6), j = 1..6), i = 1..20)} :
nops(EQ4);
EQ4s := simplify(subs(spt, subs(pt, EQ4))) :
jt4 := {seq(seq(seq(seq(f[i, j, k, l], l = k..6), k = j..6), j = i..6), i = 1..6),
seq(seq(seq(seq(g[i, j, k, l], l = k..6), k = j..6), j = i..6), i = 1..6)} : nops(jt4)

```

420

252

(18)

```

> sl4 := eliminate(EQ4s, jt4) :
tmp4 := {} :for i to nops(sl4[1]) do if lhs(sl4[1][i]) = rhs(sl4[1][i]) then tmp4 := tmp4

```

```

union {lhs(sl4[1][i])} :fi:od: tmp4;
nops(sl4[1]), nops(sl4[2])

```

{ }  
252, 168

(19)

Above EQ4 are 2-prolonged equations from the system EQ. They contain  $20 \cdot \frac{6 \cdot 7}{2} = 420$  fourth order equations, while the number of 4-jet variables is 252. Now this system can already be resolved with respect to all 4-jet variables, so it closes on 4-jet level. Yet it is not involutive.

First of all notice that prolongation of the prolongation-projection system on 2-jets (the largest stratum consisting of 24 equations) does not give a Frobenius system after prolongation to 3-jets (see sls3 below) : the number of free 3-jet variables is 8. Even the projection of EQ4 to 3-jet (that adds up more third order equations) is still not closed (see tmp3 below): the number of free 3-jet variables is 3. No new equations of the 2nd order are however added.

```

> E3n := simplify(subs(s22[1], sl4[2])) : nops(%)
168

```

(20)

```

> spt1 := { } :for i to nops(spt) do if lhs(spt[i])  $\neq$  rhs(spt[i]) then spt1 := spt1
union {spt[i]} :fi:od:
eq2 := spt1 union s22[1] : nops(eq2)
24

```

(21)

```

> eq3 := { } :for i to nops(eq2) do for j to 6 do eq3 := eq3 union {TotalDiff(eq2[i], j)} :od:
od: nops(eq3)
141

```

(22)

```

> nops(jt3)
112

```

(23)

```

> sls3 := solve(eq3, jt3)
sls3 := {f1,1,1 = 0, f1,1,2 = 0, f1,1,3 = -2f1,2,4, f1,1,4 = 0, f1,1,5 = 0, f1,1,6 = 2f1,4,5, f1,2,2
= 0, f1,2,3 = -f1,4,5, f1,2,4 = f1,2,4, f1,2,5 = f1,4,5, f1,2,6 = 0, f1,3,3 = -2f1,4,6
- 2g1,3,6, f1,3,4 = -3f1,4,5 + g2,3,4, f1,3,5 = f1,4,6 + g1,3,6, f1,3,6 = -g4,5,6, f1,4,4
= 2f1,2,4, f1,4,5 = f1,4,5, f1,4,6 = f1,4,6, f1,5,5 = 0, f1,5,6 = g4,5,6, f1,6,6 = 0, f2,2,2 = 0,
f2,2,3 = 0, f2,2,4 = 0, f2,2,5 = 0, f2,2,6 = 0, f2,3,3 = 2g4,5,6, f2,3,4 = g1,3,6, f2,3,5 =
-2g4,5,6, f2,3,6 = 0, f2,4,4 = -2g2,3,4 + 4f1,4,5, f2,4,5 = -g1,3,6, f2,4,6 = 0, f2,5,5
= 2g4,5,6, f2,5,6 = 0, f2,6,6 = 0, f3,3,3 = 6g3,5,6, f3,3,4 = -2g4,5,6 - 2f3,4,5, f3,3,5 =
-4g3,5,6, f3,3,6 = 0, f3,4,4 = 2g1,3,6, f3,4,5 = f3,4,5, f3,4,6 = -g3,5,6, f3,5,5 = 2g3,5,6,
f3,5,6 = 0, f3,6,6 = 0, f4,4,4 = 12f1,4,5 - 6g2,3,4, f4,4,5 = -2g1,3,6, f4,4,6 = 4g4,5,6
+ 2f3,4,5, f4,5,5 = 2g4,5,6, f4,5,6 = g3,5,6, f4,6,6 = 0, f5,5,5 = 0, f5,5,6 = 0, f5,6,6 = 0,
f6,6,6 = 0, g1,1,1 = 0, g1,1,2 = 0, g1,1,3 = 0, g1,1,4 = 0, g1,1,5 = 0, g1,1,6 = 0, g1,2,2
= 0, g1,2,3 = f1,2,4, g1,2,4 = 0, g1,2,5 = 0, g1,2,6 = -f1,4,5, g1,3,3 = -2g2,3,4
+ 4f1,4,5, g1,3,4 = f1,2,4, g1,3,5 = 0, g1,3,6 = g1,3,6, g1,4,4 = 0, g1,4,5 = 0, g1,4,6 =

```

(24)



$$\begin{aligned}
& -f_{1,4,5}, g_{1,5,5} = 0, g_{1,5,6} = 0, g_{1,6,6} = 2g_{4,5,6}, g_{2,2,2} = 0, g_{2,2,3} = 2f_{1,4,5}, g_{2,2,4} = \\
& -2f_{1,2,4}, g_{2,2,5} = -2f_{1,4,5}, g_{2,2,6} = 0, g_{2,3,3} = 2f_{1,4,6}, g_{2,3,4} = g_{2,3,4}, g_{2,3,5} = \\
& -f_{1,4,6}, g_{2,3,6} = -g_{4,5,6}, g_{2,4,4} = -4f_{1,2,4}, g_{2,4,5} = -2f_{1,4,5}, g_{2,4,6} = -f_{1,4,6} \\
& -g_{1,3,6}, g_{2,5,5} = 0, g_{2,5,6} = g_{4,5,6}, g_{2,6,6} = 0, g_{3,3,3} = 12g_{4,5,6} + 6f_{3,4,5}, g_{3,3,4} = \\
& 2f_{1,4,6}, g_{3,3,5} = -4g_{4,5,6} - 2f_{3,4,5}, g_{3,3,6} = -2g_{3,5,6}, g_{3,4,4} = 2g_{2,3,4} \\
& -2f_{1,4,5}, g_{3,4,5} = -f_{1,4,6}, g_{3,4,6} = -3g_{4,5,6} - f_{3,4,5}, g_{3,5,5} = 0, g_{3,5,6} = g_{3,5,6}, \\
& g_{3,6,6} = 0, g_{4,4,4} = -6f_{1,2,4}, g_{4,4,5} = -2f_{1,4,5}, g_{4,4,6} = -2f_{1,4,6} - 2g_{1,3,6}, g_{4,5,5} \\
& = 0, g_{4,5,6} = g_{4,5,6}, g_{4,6,6} = 2g_{3,5,6}, g_{5,5,5} = 0, g_{5,5,6} = 0, g_{5,6,6} = 0, g_{6,6,6} = 0\}
\end{aligned}$$

> nops(sls3)

112

(25)

> tmp := { } :for i to nops(sls3) do if lhs(sls3[i]) = rhs(sls3[i]) then tmp := tmp  
union {lhs(sls3[i])} :fi:od: tmp, nops(%)

{f<sub>1,2,4</sub>, f<sub>1,4,5</sub>, f<sub>1,4,6</sub>, f<sub>3,4,5</sub>, g<sub>1,3,6</sub>, g<sub>2,3,4</sub>, g<sub>3,5,6</sub>, g<sub>4,5,6</sub>}, 8

(26)

> # nops(IdealInfo:-Variables(⟨op(E3n)⟩)), nops(MaximalIndependentSet(⟨op(E3n)⟩)),  
nops(IdealInfo:-Variables(⟨op(E3n)⟩)) - HilbertDimension(⟨op(E3n)⟩)

> E3p := subs(s22[1], subs(Sl3[1], E3n)) :

> s3p := eliminate(E3p, fv3) :

> nops(%)

2

(27)

> nops(s3p[2])

0

(28)

> s3p[1]

{g<sub>1,4,6</sub> = -2f<sub>1,4</sub>f<sub>1,6</sub> + g<sub>4,6</sub>f<sub>1,4</sub> - g<sub>1,3</sub>f<sub>1,6</sub> + g<sub>1,6</sub><sup>2</sup> + g<sub>1,6</sub>g<sub>3,4</sub> - f<sub>1,4</sub>g<sub>3,5</sub> - f<sub>1,6</sub>g<sub>2,4</sub>

(29)

- g<sub>4,5</sub>f<sub>2,4</sub> - g<sub>1,3</sub>g<sub>3,5</sub> + g<sub>1,3</sub>g<sub>4,6</sub> - g<sub>5,6</sub>g<sub>1,4</sub> - g<sub>2,3</sub>g<sub>4,5</sub> - g<sub>4,6</sub>g<sub>2,4</sub> + g<sub>4,5</sub>g<sub>3,4</sub>

+  $\frac{1}{2}$ g<sub>4,4,5</sub>g<sub>2,3,3</sub> = - $\frac{1}{2}$ g<sub>4,4,6</sub> - 2f<sub>2,4</sub>g<sub>2,6</sub> + 2f<sub>2,4</sub>f<sub>3,4</sub> - 2f<sub>2,4</sub>g<sub>3,5</sub> - 2g<sub>2,4</sub>g<sub>3,6</sub>

- 2g<sub>1,3</sub>g<sub>3,6</sub> - f<sub>4,6</sub>f<sub>1,4</sub> + 2f<sub>1,6</sub>f<sub>2,4</sub> + f<sub>1,6</sub>g<sub>1,6</sub> + f<sub>1,6</sub>g<sub>3,4</sub> - g<sub>2,3</sub>g<sub>4,6</sub> + 3g<sub>4,6</sub>f<sub>2,4</sub>

+ f<sub>5,6</sub>g<sub>1,4</sub> - 2g<sub>2,3</sub>f<sub>3,4</sub> + g<sub>4,6</sub>g<sub>1,6</sub> - 2g<sub>2,3</sub>f<sub>1,6</sub> - g<sub>1,3</sub>f<sub>4,6</sub> - 2f<sub>1,4</sub>g<sub>3,6</sub>

- 2g<sub>2,3</sub>g<sub>2,6</sub> - 2g<sub>2,3</sub>g<sub>3,5</sub>g<sub>2,3,4</sub> = f<sub>1,4</sub>g<sub>2,6</sub> + f<sub>1,4</sub>g<sub>3,5</sub> - f<sub>1,4</sub>g<sub>4,6</sub> + f<sub>1,6</sub>g<sub>1,3</sub>

- f<sub>2,4</sub>g<sub>2,3</sub> - f<sub>2,4</sub>g<sub>4,5</sub> + f<sub>4,6</sub>g<sub>1,4</sub> + 2g<sub>1,3</sub>g<sub>2,6</sub> + g<sub>1,3</sub>g<sub>3,5</sub> - g<sub>1,3</sub>g<sub>4,6</sub> + g<sub>1,4</sub>g<sub>3,6</sub> -

g<sub>2,3</sub><sup>2</sup> + g<sub>2,3</sub>g<sub>3,4</sub> - g<sub>2,3</sub>g<sub>4,5</sub> - g<sub>2,4</sub>g<sub>4,6</sub>g<sub>2,4,4</sub> = -2f<sub>1,4</sub>f<sub>2,4</sub> + 2f<sub>1,4</sub>g<sub>4,5</sub> + 4f<sub>1,6</sub>g<sub>1,4</sub>

$$\begin{aligned}
& -2f_{2,4}g_{1,3} + 2g_{1,3}g_{4,5} + 2g_{1,4}g_{2,6} + 2g_{1,4}g_{4,6}g_{2,4,6} = f_{4,6}f_{1,4} + g_{5,6}f_{1,4} \\
& + g_{2,3}f_{1,6} + g_{4,5}f_{1,6} + g_{1,3}f_{4,6} + g_{5,6}g_{1,3} + g_{1,6}g_{2,6} - g_{4,6}g_{1,6} + g_{2,6}g_{3,4} \\
& + \frac{1}{2}g_{4,4,6}g_{3,3,3} = 6f_{1,6}^2 + 12f_{1,6}f_{3,4} - 12f_{1,6}g_{2,6} - 12f_{1,6}g_{3,5} + 12f_{1,6}g_{4,6} \\
& - 6f_{2,4}g_{3,6} - 12f_{2,4}g_{5,6} + 6f_{3,4}^2 + 12f_{3,4}g_{4,6} - 12f_{4,6}g_{4,5} - 12f_{5,6}g_{2,4} \\
& - 12g_{1,6}g_{5,6} - 6g_{2,3}g_{3,6} - 12g_{2,3}g_{5,6} - 12g_{2,6}g_{4,6} + 6g_{4,6}^2 + 12g_{4,5,6}g_{3,3,4} \\
& = -f_{4,6}f_{1,4} + 2f_{1,4}g_{3,6} + 2f_{1,6}f_{2,4} + f_{1,6}g_{1,6} + 2g_{2,3}f_{1,6} - f_{1,6}g_{3,4} + 2f_{2,4}f_{3,4} \\
& + g_{4,6}f_{2,4} + 2g_{2,3}f_{3,4} - 2f_{3,4}g_{3,4} + g_{1,3}f_{4,6} + f_{5,6}g_{1,4} + 4g_{1,3}g_{3,6} + g_{4,6}g_{1,6} \\
& + g_{2,3}g_{4,6} - 2g_{4,6}g_{3,4} - \frac{1}{2}g_{4,4,6}g_{3,3,5} = 4f_{1,6}g_{2,6} + 2f_{1,6}g_{3,5} + 2f_{2,4}g_{5,6} \\
& - 2f_{3,4}g_{3,5} + 2f_{4,6}g_{2,3} + 4f_{4,6}g_{4,5} + 4f_{5,6}g_{2,4} + 4g_{1,6}g_{5,6} + 2g_{2,3}g_{3,6} \\
& + 2g_{2,3}g_{5,6} + 4g_{2,6}g_{4,6} - 2g_{3,5}g_{4,6} - 2g_{3,6}g_{4,5} - 4g_{4,5,6}g_{3,4,4} = -2f_{1,4}f_{1,6} \\
& - 2f_{1,4}f_{3,4} - 2f_{1,4}g_{3,5} - 2f_{1,6}g_{2,4} - 2f_{2,4}g_{4,5} - 2f_{3,4}g_{1,3} + 2f_{4,6}g_{1,4} \\
& - 2g_{1,3}g_{3,5} + 2g_{1,3}g_{4,6} + 2g_{1,4}g_{3,6} - 2g_{1,4}g_{5,6} - 2g_{2,3}g_{4,5} - 2g_{2,4}g_{4,6} \\
& + 2g_{3,4}g_{4,5} + g_{4,4,5}g_{3,4,5} = \frac{1}{2}f_{4,6}f_{1,4} + g_{5,6}f_{1,4} - \frac{1}{2}f_{1,6}g_{1,6} + g_{2,3}f_{1,6} \\
& - \frac{1}{2}f_{1,6}g_{3,4} + g_{4,5}f_{1,6} - \frac{1}{2}g_{4,6}f_{2,4} + g_{4,5}f_{3,4} + \frac{1}{2}g_{1,3}f_{4,6} + f_{4,6}g_{2,4} \\
& - \frac{1}{2}f_{5,6}g_{1,4} + 2g_{5,6}g_{1,3} - \frac{1}{2}g_{4,6}g_{1,6} + \frac{1}{2}g_{2,3}g_{4,6} + g_{2,4}g_{3,6} + \frac{1}{4}g_{4,4,6}g_{3,4,6} \\
& = 2f_{1,4}f_{5,6} - 2f_{1,6}^2 - 2f_{1,6}f_{3,4} + 3f_{1,6}g_{2,6} + 3f_{1,6}g_{3,5} - 2f_{1,6}g_{4,6} \\
& + 3f_{2,4}g_{5,6} - f_{3,4}g_{4,6} + f_{4,6}g_{1,6} + f_{4,6}g_{3,4} + 3f_{4,6}g_{4,5} + 3f_{5,6}g_{1,3} + 3f_{5,6}g_{2,4} \\
& + g_{1,6}g_{3,6} + 3g_{1,6}g_{5,6} + 3g_{2,3}g_{5,6} + 3g_{2,6}g_{4,6} + g_{3,4}g_{3,6} - g_{4,6}^2 - 3g_{4,5,6}g_{3,5,6} \\
& = -f_{3,4}g_{5,6} + f_{4,6}g_{2,6} + f_{4,6}g_{3,5} + f_{5,6}g_{2,3} - 2f_{5,6}g_{4,5} + g_{2,6}g_{3,6} \\
& + g_{3,5}g_{3,6} - g_{4,6}g_{5,6}g_{4,4,4} = -6f_{1,4}f_{2,4} - 6f_{1,4}g_{2,3} + 6f_{1,4}g_{3,4} + 6f_{1,6}g_{1,4} \\
& - 6f_{2,4}g_{1,3} - 6g_{1,3}g_{2,3} + 6g_{1,3}g_{3,4} + 6g_{1,4}g_{4,6}g_{4,4,5} = g_{4,4,5}g_{4,4,6} \\
& = g_{4,4,6}g_{4,5,6} = g_{4,5,6}g_{4,6,6} = 2f_{1,6}g_{3,6} + 2f_{2,4}f_{5,6} + 2f_{4,6}g_{4,6} + 2f_{5,6}g_{1,6}
\end{aligned}$$

$$+ 2f_{5,6}g_{2,3} + 2g_{3,6}g_{4,6}\}$$

$$\begin{aligned} &> \text{IdeallInfo:-Variables}(\langle \text{op}(E3p) \rangle), \text{nops}(\text{IdeallInfo:-Variables}(\langle \text{op}(E3p) \rangle)) \\ &\{f_{1,4}, f_{1,6}, f_{2,4}, f_{3,4}, f_{4,6}, f_{5,6}, g_{1,3}, g_{1,4}, g_{1,6}, g_{2,3}, g_{2,4}, g_{2,6}, g_{3,4}, g_{3,5}, g_{3,6}, g_{4,5}, g_{4,6}, \\ &g_{5,6}, g_{1,4,6}, g_{2,3,3}, g_{2,3,4}, g_{2,4,4}, g_{2,4,6}, g_{3,3,3}, g_{3,3,4}, g_{3,3,5}, g_{3,4,4}, g_{3,4,5}, g_{3,4,6}, \\ &g_{3,5,6}, g_{4,4,4}, g_{4,4,5}, g_{4,4,6}, g_{4,5,6}, g_{4,6,6}\}, 35 \end{aligned} \quad (30)$$

$$\begin{aligned} &> \text{tmp3} := \{ \} : \text{for } i \text{ to } \text{nops}(s3p[1]) \text{ do if } \text{lhs}(s3p[1][i]) = \text{rhs}(s3p[1][i]) \text{ then } \text{tmp3} := \text{tmp3} \\ &\quad \text{union } \{ \text{lhs}(s3p[1][i]) \} : \text{fi:od: tmp3, nops}(\%) \\ &\quad \{g_{4,4,5}, g_{4,4,6}, g_{4,5,6}\}, 3 \end{aligned} \quad (31)$$

Ok, so the system is not yet involutive (formally integrable). We have to do one more prolongation (to 5-jets): this is the system EQ5. It consists of 1120 equations, and indeed can be resolved with respect to all 504 jets of order 5.

$$\begin{aligned} &> \text{EQ5} := \{ \text{seq}(\text{seq}(\text{seq}(\text{seq}(\text{TotalDiff}(\text{TotalDiff}(\text{TotalDiff}(\text{EQ}[i], j), k), l), l = k..6), k = j..6), j \\ &\quad = 1..6), i = 1..20) \} : \text{nops}(\text{EQ5}); \\ &\text{EQ5s} := \text{simplify}(\text{subs}(spt, \text{subs}(pt, \text{EQ5}))) : \\ &\text{jt5} := \{ \text{seq}(\text{seq}(\text{seq}(\text{seq}(\text{seq}(f[i, j, k, l, m], m = l..6), l = k..6), k = j..6), j = i..6), i = 1..6), \\ &\quad \text{seq}(\text{seq}(\text{seq}(\text{seq}(\text{seq}(g[i, j, k, l, m], m = l..6), l = k..6), k = j..6), j = i..6), i = 1..6) \} : \\ &\quad \text{nops}(\text{jt5}) \end{aligned} \quad \begin{array}{l} 1120 \\ 504 \end{array} \quad (32)$$

$$\begin{aligned} &> \text{sl5} := \text{eliminate}(\text{EQ5s}, \text{jt5}) : \\ &\text{tmp5} := \{ \} : \text{for } i \text{ to } \text{nops}(\text{sl5}[1]) \text{ do if } \text{lhs}(\text{sl5}[1][i]) = \text{rhs}(\text{sl5}[1][i]) \text{ then } \text{tmp5} := \text{tmp5} \\ &\quad \text{union } \{ \text{lhs}(\text{sl5}[1][i]) \} : \text{fi:od: tmp5}; \\ &\text{nops}(\text{sl5}[1]), \text{nops}(\text{sl5}[2]) \\ &\quad \{ \} \\ &\quad 504, 616 \end{aligned} \quad (33)$$

$$\begin{aligned} &> \text{Eq4q} := \text{subs}(\text{sl4}[1], \text{sl5}[2]) : \\ &> \text{Eq3q} := \text{subs}(\text{s22}[1], \text{subs}(spt, \text{subs}(s3p[1], \text{subs}(\text{sl3}[1], \text{Eq4q})))) : \\ &> \text{length}(\text{Eq3q}) \\ &\quad 1770630336 \end{aligned} \quad (34)$$

Now the system is projected down (by substituting the expressed all 5-jets to the remaining equations, then by substituting the expressed all 4-jets to the remaining equations, then by substituting 112-3=109 jets of order 3 that are already expressed to the remaining equations; everything is done at pt, but the substitution of this 1-jet is made only after the equations have been computed in full generality). As follows from SnS2 computation below we can express the remaining 3-jets, and now we close the system: it has a reduced variety on the level of 2-jets (24 or 30 equations), then all 3- and 4- and 5- etc jets are expressed by free 2-jets (and 1-jets indeed, but these are frozen in our latest computation). The dimensional count implies that this system is in involution.

$$\begin{aligned} &> \text{SnS2} := \text{eliminate}(\text{Eq3q}, \{g_{4,4,5}, g_{4,4,6}, g_{4,5,6}\}) : \\ &> \text{nops}(\text{SnS2}[1]), \text{nops}(\text{SnS2}[2]) \\ &\quad 3, 0 \end{aligned} \quad (35)$$

$$> \text{SnS2}$$

$$\begin{aligned}
& \left[ \{ g_{4,4,5} = 2f_{1,4}g_{3,5} + 2f_{1,6}g_{2,4} + 2f_{2,4}g_{4,5} + 2g_{1,3}g_{3,5} + 2g_{1,4}g_{5,6} + 2g_{2,3}g_{4,5} \right. \\
& \quad + 2g_{2,4}g_{4,6} - 2g_{3,4}g_{4,5}, g_{4,4,6} = -2f_{1,4}f_{4,6} + 2f_{1,6}g_{1,6} + 2f_{1,6}g_{3,4} \\
& \quad + 2f_{2,4}g_{4,6} - 2f_{4,6}g_{1,3} + 2f_{5,6}g_{1,4} + 2g_{1,6}g_{4,6} + 2g_{2,3}g_{4,6}, g_{4,5,6} = f_{1,6}g_{2,6} \\
& \quad + f_{1,6}g_{3,5} + f_{2,4}g_{5,6} + f_{4,6}g_{4,5} + f_{5,6}g_{2,4} + g_{1,6}g_{5,6} + g_{2,3}g_{5,6} + g_{2,6}g_{4,6} \}, \\
& \quad \left. \{ \} \right]
\end{aligned}
\tag{36}$$

$\left[ \begin{array}{l} \text{ } \\ \text{ } \end{array} \right] >$
