# Supplementary material for: Integrable systems in 4D associated with sixfolds in Gr(4,6)
Source: arXiv:1705.06999 ancillary file (2017-05-18)
Supplement: Supplementary file 4 [file DFKN-2017-LaxPairsTables.pdf]

This worksheet accompanies the paper B.Doubrov, E.Ferapontov, B.Kruglikov, V.Novikov "Integrable systems in 4D associated with sixfolds in Gr(4,6)".

The file ran on **Maple** version 17, the package **DifferentialGeometry** was used.

Here we verify the Lax pairs for general linearly degenerate systems. Segre type numeration follows the one in the paper.

```

>
> with(DifferentialGeometry) : with(JetCalculus) : with(Tools) : with(PDETools) :
  Preferences("ShowFramePrompt",false) :
>
> uv := {u(x1, x2, x3, x4), v(x1, x2, x3, x4)} :
>
> DGsetup([x1, x2, x3, x4], [u, v], J, 2) :
> F0 := (u2 - u1 v1) · (v3 - u2 - v1 v2) - (v2 - u1 - v1^2) · (u3 - u1 v2) :
  G0 := (u2 - u1 v1) · (v4 - u3 - v1 v3) - (v2 - u1 - v1^2) · (u4 - u1 v3) :
> S0 := solve({F0, G0, TotalDiff(F0, 1), TotalDiff(F0, 2), TotalDiff(F0, 3), TotalDiff(F0, 4),
  TotalDiff(G0, 1), TotalDiff(G0, 2), TotalDiff(G0, 3), TotalDiff(G0, 4)}, {u3, v4, u1,3,
  u2,3, u3,3, u3,4, v1,4, v2,4, v3,3, v4,4}) :
> DGsetup([x1, x2, x3, x4], R4) :
> m0 := (u1 v2 - u3) / (u1 v1 - u2) : n0 := (u1 v3 - u4) / (u1 v1 - u2) : a0 := - (u2 v2 - u3 v1) / (u1 v1 - u2) : b0 := - (u2 v3 - u4 v1) / (u1 v1 - u2) :
  M0 := FromJet(m0, uv) : N0 := FromJet(n0, uv) : A0 := FromJet(a0, uv) : B0
  := FromJet(b0, uv) :
> X0 := evalDG(D_x3 - (q + M0) D_x2 + (q M0 - A0) D_x1) :
  Y0 := evalDG(D_x4 - (q^2 + q M0 + N0) D_x2 + (q^2 M0 + q N0 - q A0 - B0) D_x1) :
> simplify(subs(S0, ToJet(LieDerivative(X0, Y0), uv, notation = jetnumbers)))
      0 D_x1 + 0 D_x2
(1)
>
> DGsetup([x1, x2, x3, x4], [u, v], J, 2) :
> F1 := (u2 - u1 v1) · (v3 - v1 v2) - (v2 - v1^2) · (u3 - u1 v2) :
  G1 := (u2 - u1 v1) · (v4 - v1 v3) - (v2 - v1^2) · (u4 - u1 v3) :
> S1 := solve({F1, G1, TotalDiff(F1, 1), TotalDiff(F1, 2), TotalDiff(F1, 3), TotalDiff(F1, 4),
  TotalDiff(G1, 1), TotalDiff(G1, 2), TotalDiff(G1, 3), TotalDiff(G1, 4)}, {u3, v4, u1,3,
  u2,3, u3,3, u3,4, v1,4, v2,4, v3,3, v4,4}) :
> DGsetup([x1, x2, x3, x4], R4) :
> m1 := (v3 - v1 v2) / (v2 - v1^2) : n1 := (v4 - v1 v3) / (v2 - v1^2) : a1 := (v2^2 - v1 v3) / (v2 - v1^2) : b1 := (v2 v3 - v1 v4) / (v2 - v1^2) :
  M1 := FromJet(m1, uv) : N1 := FromJet(n1, uv) : A1 := FromJet(a1, uv) : B1
  := FromJet(b1, uv) :

```

```

> X1 := evalDG(D_x3 - (q + M1)·D_x2 + (q M1 - A1)·D_x1) :
Y1 := evalDG(D_x4 - (q^2 + q M1 + N1)·D_x2 + (q^2 M1 + q N1 - q A1 - B1)·D_x1) :
> simplify(subs(S1, ToJet(LieDerivative(X1, Y1), uv, notation = jetnumbers)))
0 D_x1 + 0 D_x2
(2)

```

```

>
> DGsetup([x1, x2, x3, x4], [u, v], J, 2) :
> F11 := u3·(v2 - v1) - u2·(v3 - v2) :
G11 := u4·(v2 - v1) - u2·(v4 - v3) :
> S11 := solve({F11, G11, TotalDiff(F11, 1), TotalDiff(F11, 2), TotalDiff(F11, 3),
TotalDiff(F11, 4), TotalDiff(G11, 1), TotalDiff(G11, 2), TotalDiff(G11, 3),
TotalDiff(G11, 4)}, {u3, v4, u1, 3, u2, 3, u3, 3, v1, 4, v2, 4, v3, 3, v3, 4, v4, 4}) :
> DGsetup([x1, x2, x3, x4], R4) :
> m11 := (v3 - v2) / (v2 - v1) : n11 := (v4 - v3) / (v2 - v1) :
M11 := FromJet(m11, uv) : N11 := FromJet(n11, uv) :
> X11 := evalDG(D_x3 - (q + M11)·D_x2 + q M11·D_x1) :
Y11 := evalDG(D_x4 - (q^2 + q M11 + N11)·D_x2 + (q^2 M11 + q N11)·D_x1) :
> simplify(subs(S11, ToJet(LieDerivative(X11, Y11), uv, notation = jetnumbers)))
0 D_x1 + 0 D_x2
(3)

```

```

>
> DGsetup([x1, x2, x3, x4], [u, v], J, 2) :
> F2 := (u2 v3 - u3 v2) - (v1 v3 - v2^2) :
G2 := (u2 v4 - u4 v2) - (v1 v4 - v2 v3) :
> S2 := solve({F2, G2, TotalDiff(F2, 1), TotalDiff(F2, 2), TotalDiff(F2, 3), TotalDiff(F2, 4),
TotalDiff(G2, 1), TotalDiff(G2, 2), TotalDiff(G2, 3), TotalDiff(G2, 4)}, {u3, v4, u1, 3,
u2, 3, u3, 3, v1, 4, v2, 4, v3, 3, v3, 4, v4, 4}) :
> DGsetup([x1, x2, x3, x4], R4) :
> m2 := v3 / v2 : n2 := v4 / v2 :
M2 := FromJet(m2, uv) : N2 := FromJet(n2, uv) :
> X2 := evalDG(D_x3 - (q + M2)·D_x2 + q M2·D_x1) :
Y2 := evalDG(D_x4 - (q^2 + q M2 + N2)·D_x2 + (q^2 M2 + q N2)·D_x1) :
> simplify(subs(S2, ToJet(LieDerivative(X2, Y2), uv, notation = jetnumbers)))
0 D_x1 + 0 D_x2
(4)

```

```

>
> DGsetup([x1, x2, x3, x4], [u, v], J, 2) :
> F111 := u3 v1 - α u1·(v2 - v3) :
G111 := u4 v1 - α u1·(v3 - v4) :

```

```

> S111 := solve( {F111, G111, TotalDiff(F111, 1), TotalDiff(F111, 2), TotalDiff(F111, 3),
  TotalDiff(F111, 4), TotalDiff(G111, 1), TotalDiff(G111, 2), TotalDiff(G111, 3),
  TotalDiff(G111, 4)}, {u3, v4, u1,3, u2,3, u3,3, v1,4, v2,4, v3,3, v3,4, v4,4} ) :
> DGsetup([x1, x2, x3, x4], R4) :
> m111 := (v2 - v3) / v1 : n111 := (v3 - v4) / v1 :
  M111 := FromJet(m111, uv) : N111 := FromJet(n111, uv) :
> X111 := evalDG(D_x2 - (1 + α - q α) · (M111 + q N111) · D_x1 - q^2 · D_x4) :
  Y111 := evalDG(D_x3 - (1 + α - q α) · N111 · D_x1 - q · D_x4) :
> simplify(subs(S111, ToJet(LieDerivative(X111, Y111), uv, notation = jetnumbers)))
0 D_x1
(5)

```

```

>
> DGsetup([x1, x2, x3, x4], [u, v], J, 2) :
> F21 := (u3 v1 - u1 v3) - v1 · (v2 - α · v3) :
  G21 := (u4 v1 - u1 v4) - v1 · (v3 - α · v4) :
> S21 := solve( {F21, G21, TotalDiff(F21, 1), TotalDiff(F21, 2), TotalDiff(F21, 3),
  TotalDiff(F21, 4), TotalDiff(G21, 1), TotalDiff(G21, 2), TotalDiff(G21, 3),
  TotalDiff(G21, 4)}, {u3, v4, u1,3, u2,3, u3,3, v1,4, v2,4, v3,3, v3,4, v4,4} ) :
> DGsetup([x1, x2, x3, x4], R4) :
> m21 := (q v4 + v3) / v1 : n21 := v4 / v1 :
  M21 := FromJet(m21, uv) : N21 := FromJet(n21, uv) :
> X21 := evalDG(D_x2 + (q - α) · M21 · D_x1 - q^2 · D_x4) :
  Y21 := evalDG(D_x3 + (q - α) · N21 · D_x1 - q · D_x4) :
> simplify(subs(S21, ToJet(LieDerivative(X21, Y21), uv, notation = jetnumbers)))
0 D_x1
(6)

```

```

>
> DGsetup([x1, x2, x3, x4], [u, v], J, 2) :
> F3 := u3 - (v2 - v1 v3) :
  G3 := u4 - (v3 - v1 v4) :
> S3 := solve( {F3, G3, TotalDiff(F3, 1), TotalDiff(F3, 2), TotalDiff(F3, 3), TotalDiff(F3, 4),
  TotalDiff(G3, 1), TotalDiff(G3, 2), TotalDiff(G3, 3), TotalDiff(G3, 4)}, {u3, v4, u1,3,
  u2,3, u3,3, v1,4, v2,4, v3,3, v3,4, v4,4} ) :
> DGsetup([x1, x2, x3, x4], R4) :
> m3 := q v4 + v3 : n3 := v4 :
  M3 := FromJet(m3, uv) : N3 := FromJet(n3, uv) :
> X3 := evalDG(D_x2 - M3 · D_x1 - q^2 · D_x4) :
  Y3 := evalDG(D_x3 - N3 · D_x1 - q · D_x4) :

```

> simplify(subs(S3, ToJet(LieDerivative(X3, Y3), uv, notation = jetnumbers)))  
0 D\_x1 (7)

>  
> DGsetup([x1, x2, x3, x4], [u, v], J, 2) :  
> F1111 :=  $\alpha \cdot u_2 v_1 - u_1 v_2$  :  
G1111 :=  $u_4 v_1 - u_1 v_3$  :  
> S1111 := solve({F1111, G1111, TotalDiff(F1111, 1), TotalDiff(F1111, 2), TotalDiff(F1111, 3), TotalDiff(F1111, 4), TotalDiff(G1111, 1), TotalDiff(G1111, 2), TotalDiff(G1111, 3), TotalDiff(G1111, 4)}, {u<sub>2</sub>, v<sub>3</sub>, u<sub>1,2</sub>, u<sub>2,2</sub>, u<sub>2,3</sub>, u<sub>2,4</sub>, v<sub>1,3</sub>, v<sub>2,3</sub>, v<sub>3,3</sub>, v<sub>3,4</sub>}) :  
> DGsetup([x1, x2, x3, x4], R4) :  
> m1111 :=  $\frac{v_1}{v_2}$  : n1111 :=  $\frac{v_3}{v_2}$  :  
M1111 := FromJet(m1111, uv) : N1111 := FromJet(n1111, uv) :  
> X1111 := evalDG( $D_{x1} + \frac{q - \alpha}{1 - q} \cdot M1111 \cdot D_{x2}$ ) :  
Y1111 := evalDG( $D_{x4} - q \cdot D_{x3} + (q - \alpha) \cdot N1111 \cdot D_{x2}$ ) :  
> simplify(subs(S1111, ToJet(LieDerivative(X1111, Y1111), uv, notation = jetnumbers)))  
0 D\_x2 (8)

>  
> DGsetup([x1, x2, x3, x4], [u, v], J, 2) :  
> F211 :=  $(u_2 v_1 - u_1 v_2) - v_1 v_2$  :  
G211 :=  $(u_4 v_1 - u_1 v_4) - v_1 v_3$  :  
> S211 := solve({F211, G211, TotalDiff(F211, 1), TotalDiff(F211, 2), TotalDiff(F211, 3), TotalDiff(F211, 4), TotalDiff(G211, 1), TotalDiff(G211, 2), TotalDiff(G211, 3), TotalDiff(G211, 4)}, {u<sub>2</sub>, v<sub>3</sub>, u<sub>1,2</sub>, u<sub>2,2</sub>, u<sub>2,3</sub>, u<sub>2,4</sub>, v<sub>1,3</sub>, v<sub>2,3</sub>, v<sub>3,3</sub>, v<sub>3,4</sub>}) :  
> DGsetup([x1, x2, x3, x4], R4) :  
> m211 :=  $\frac{v_1}{v_2}$  : n211 :=  $\frac{v_4}{v_2}$  :  
M211 := FromJet(m211, uv) : N211 := FromJet(n211, uv) :  
> X211 := evalDG( $D_{x1} + (q - 1) \cdot M211 \cdot D_{x2}$ ) :  
Y211 := evalDG( $D_{x4} - q \cdot D_{x3} + (q - 1) \cdot N211 \cdot D_{x2}$ ) :  
> simplify(subs(S211, ToJet(LieDerivative(X211, Y211), uv, notation = jetnumbers)))  
0 D\_x2 (9)

>  
> DGsetup([x1, x2, x3, x4], [u, v], J, 2) :  
> F22 :=  $(u_2 v_1 - u_1 v_2) - v_1^2$  :  
G22 :=  $(u_4 v_1 - u_1 v_4) - v_1 v_3$  :  
> S22 := solve({F22, G22, TotalDiff(F22, 1), TotalDiff(F22, 2), TotalDiff(F22, 3),

```

    TotalDiff(F22, 4), TotalDiff(G22, 1), TotalDiff(G22, 2), TotalDiff(G22, 3),
    TotalDiff(G22, 4)}, {u2, v3, u1, 2, u2, 2, u2, 3, u2, 4, v1, 3, v2, 3, v3, 3, v3, 4}) :
> DGsetup([x1, x2, x3, x4], R4) :
> m22 :=  $\frac{v_2}{v_1}$  : n22 :=  $\frac{v_4}{v_1}$  :
    M22 := FromJet(m22, uv) : N22 := FromJet(n22, uv) :
> X22 := evalDG(D_x2 - (q + M22)·D_x1) :
    Y22 := evalDG(D_x4 - q·D_x3 - N22·D_x1) :
> simplify(subs(S22, ToJet(LieDerivative(X22, Y22), uv, notation = jetnumbers)))
0 D_x1
(10)

```

```

>
> DGsetup([x1, x2, x3, x4], [u, v], J, 2) :
> F31 := u2 + v1 v2 :
    G31 := u4 - v3 + v1 v4 :
> S31 := solve({F31, G31, TotalDiff(F31, 1), TotalDiff(F31, 2), TotalDiff(F31, 3),
    TotalDiff(F31, 4), TotalDiff(G31, 1), TotalDiff(G31, 2), TotalDiff(G31, 3),
    TotalDiff(G31, 4)}, {u2, v3, u1, 2, u2, 2, u2, 3, u2, 4, v1, 3, v2, 3, v3, 3, v3, 4}) :
> DGsetup([x1, x2, x3, x4], R4) :
> m31 := v2 : n31 := v4 :
    M31 := FromJet(m31, uv) : N31 := FromJet(n31, uv) :
> X31 := evalDG(D_x2 + q·M31·D_x1) :
    Y31 := evalDG(D_x4 - q·D_x3 + q·N31·D_x1) :
> simplify(subs(S31, ToJet(LieDerivative(X31, Y31), uv, notation = jetnumbers)))
0 D_x1
(11)

```

```

>
> DGsetup([x1, x2, x3, x4], [u, v], J, 2) :
> F4 := u1 - v2 + v12 :
    G4 := u4 - v3 + v1 v4 :
> S4 := solve({F4, G4, TotalDiff(F4, 1), TotalDiff(F4, 2), TotalDiff(F4, 3), TotalDiff(F4, 4),
    TotalDiff(G4, 1), TotalDiff(G4, 2), TotalDiff(G4, 3), TotalDiff(G4, 4)}, {u4, v2, u1, 4,
    u2, 4, u3, 4, u4, 4, v1, 2, v2, 2, v2, 3, v2, 4}) :
> DGsetup([x1, x2, x3, x4], R4) :
> m4 := v1 : n4 := v4 :
    M4 := FromJet(m4, uv) : N4 := FromJet(n4, uv) :
> X4 := evalDG(D_x2 - (q + M4)·D_x1) :
    Y4 := evalDG(D_x3 - q·D_x4 - N4·D_x1) :
> simplify(subs(S4, ToJet(LieDerivative(X4, Y4), uv, notation = jetnumbers)))
0 D_x1
(12)

```
