# Supplementary material for: Integrable systems in 4D associated with sixfolds in Gr(4,6)
Source: arXiv:1705.06999 ancillary file (2017-05-18)
Supplement: Supplementary file 5 [file DFKN-2017-Linearization.pdf]

This worksheet accompanies the paper B.Doubrov, E.Ferapontov, B.Kruglikov, V.Novikov "Integrable systems in 4D associated with sixfolds in  $\text{Gr}(4,6)$ ".

The file ran on **Maple** version 17, the package **DifferentialGeometry** was used.

Here we deduce 34 conditions of linearizability of a Monge-Ampere 2x2 system. Then we check that the additional 4=34-30 equations coincide with the 4 additional equations obtained by prolongation-projection for the (non-involutive) system of linear degeneracy.

```
> restart : with (LinearAlgebra) : with (PDETools) :
```

**3D: warm-up**

```
> var := u1, u2, v1, v2 : F := f(var) : G := g(var) :
```

```
> r := subs( {u3 = F, v3 = G}, [1, u1, v1, u2, v2, u1 v2 - v1 u2, u1 v3 - v1 u3, u2 v3 - v2 u3, u3, v3] ) :
```

```
> EQ1 := { } :for i in var do EQ1 := EQ1 union {r || i = diff(r, i)} :od: nops(EQ1)
```

4

(1)

```
> EQ2 := { } :for i to 4 do for j from i to 4 do EQ2 := EQ2 union {r || (var[i]) || (var[j]) = diff(r, var[i], var[j])} :od:od: nops(EQ2)
```

10

(2)

```
> Mr := Matrix( [r, seq(subs(EQ1, r || (var[i])), i = 1..4), seq(seq(subs(EQ2, r || (var[i]) || (var[j])), j = i..4), i = 1..4)] ) :
```

```
> interface(rtablesize = 15) :
```

```
> Mr[1..15, 1..5]
```

$$\begin{bmatrix} 1 & u1 & v1 & u2 & v2 \\ 0 & 1 & 0 & 0 & 0 \\ 0 & 0 & 0 & 1 & 0 \\ 0 & 0 & 1 & 0 & 0 \\ 0 & 0 & 0 & 0 & 1 \\ 0 & 0 & 0 & 0 & 0 \\ 0 & 0 & 0 & 0 & 0 \\ 0 & 0 & 0 & 0 & 0 \\ 0 & 0 & 0 & 0 & 0 \\ 0 & 0 & 0 & 0 & 0 \\ 0 & 0 & 0 & 0 & 0 \\ 0 & 0 & 0 & 0 & 0 \\ 0 & 0 & 0 & 0 & 0 \\ 0 & 0 & 0 & 0 & 0 \\ 0 & 0 & 0 & 0 & 0 \end{bmatrix}$$

(3)

So r is the position vector of the Plucker embedding of  $\text{Gr}(3,5)$  into  $P^9$ , Mr its 2-jet matrix (10x15). Its rank is equal to the rank of its minor obtained by removing first 5 rows and columns. The Monge-Ampere

equations are codimension 2 plane sections, so the condition is that  $\text{rank}(\text{Mr2})=3$ , i.e. all 4x4 minors of Mr2 vanish.

>  $\text{Mr2} := \text{eval}(\text{ToJet}(\text{Mr}[6..15, 6..10], \{F, G\}, \text{notation} = \text{jetnumbers}), \{u1 = 0, v1 = 0, u2 = 0, v2 = 0\})$

$$\text{Mr2} := \begin{bmatrix} 0 & 2g_1 & 0 & f_{1,1} & g_{1,1} \\ 0 & g_2 & g_1 & f_{1,2} & g_{1,2} \\ 0 & -f_1 + g_3 & 0 & f_{1,3} & g_{1,3} \\ 1 & g_4 & -f_1 & f_{1,4} & g_{1,4} \\ 0 & 0 & 2g_2 & f_{2,2} & g_{2,2} \\ -1 & -f_2 & g_3 & f_{2,3} & g_{2,3} \\ 0 & 0 & -f_2 + g_4 & f_{2,4} & g_{2,4} \\ 0 & -2f_3 & 0 & f_{3,3} & g_{3,3} \\ 0 & -f_4 & -f_3 & f_{3,4} & g_{3,4} \\ 0 & 0 & -2f_4 & f_{4,4} & g_{4,4} \end{bmatrix} \quad (4)$$

>  $\text{sbM} := (i, j) \rightarrow \text{factor}(\text{Determinant}(\text{Mr2}[[1, 2, 4, i], [1..3, j]])) :$

>  $\text{SEQ} := \{\text{sbM}(3, 4), \text{sbM}(3, 5), \text{seq}(\text{sbM}(i, 4), i = 5..10), \text{seq}(\text{sbM}(i, 5), i = 5..10)\}$

$$\text{SEQ} := \{g_1(f_1 f_{1,1} - f_{1,1} g_3 + 2f_{1,3} g_1), g_1(f_1 g_{1,1} + 2g_1 g_{1,3} - g_3 g_{1,1}), 2g_1(f_3 f_{1,1} + f_{3,3} g_1), 2g_1(f_3 g_{1,1} + g_1 g_{3,3}), 2f_{1,1} g_2^2 - 4f_{1,2} g_1 g_2 + 2f_{2,2} g_1^2, 2g_1^2 g_{2,2} - 4g_1 g_2 g_{1,2} + 2g_2^2 g_{1,1}, -2f_4 f_{1,1} g_2 + 4f_4 f_{1,2} g_1 + 2f_{4,4} g_1^2, 4f_4 g_1 g_{1,2} - 2f_4 g_2 g_{1,1} + 2g_1^2 g_{4,4}, -f_3 f_{1,1} g_2 + 2f_3 f_{1,2} g_1 + f_4 f_{1,1} g_1 + 2f_{3,4} g_1^2, 2f_3 g_1 g_{1,2} - f_3 g_2 g_{1,1} + f_4 g_1 g_{1,1} + 2g_1^2 g_{3,4}, -f_2 f_{1,1} g_2 + 2f_2 f_{1,2} g_1 + f_{1,1} g_2 g_4 - 2f_{1,2} g_1 g_4 + 2f_{2,4} g_1^2, 2f_2 g_1 g_{1,2} - f_2 g_2 g_{1,1} + 2g_1^2 g_{2,4} - 2g_1 g_4 g_{1,2} + g_2 g_4 g_{1,1}, -f_1 f_{1,1} g_2 + 2f_1 f_{1,2} g_1 + f_2 f_{1,1} g_1 - f_{1,1} g_1 g_4 + f_{1,1} g_2 g_3 - 2f_{1,2} g_1 g_3 + 2f_{1,4} g_1^2 + 2f_{2,3} g_1^2, 2f_1 g_1 g_{1,2} - f_1 g_2 g_{1,1} + f_2 g_1 g_{1,1} + 2g_1^2 g_{1,4} + 2g_1^2 g_{2,3} - 2g_1 g_3 g_{1,2} - g_1 g_4 g_{1,1} + g_2 g_3 g_{1,1}\} \quad (5)$$

>  $\text{sfg} := \text{solve}(\text{SEQ}, \{\text{seq}(\text{seq}(f_{i,j}, j = i..4), i = 1..4), \text{seq}(\text{seq}(g_{i,j}, j = i..4), i = 1..4)\}) :$

>  $\text{sfg} := \text{simplify}(\text{solve}(\text{SEQ}, \{f_{1,1}, f_{1,2}, f_{2,2}, f_{1,4}, f_{3,3}, f_{3,4}, f_{4,4}, g_{1,1}, g_{1,2}, g_{2,2}, g_{2,3}, g_{3,3}, g_{3,4}, g_{4,4}\}))$

$$\text{sfg} := \left\{ f_{1,1} = -\frac{2f_{1,3} g_1}{f_1 - g_3}, f_{1,2} = \frac{-g_2 (f_2 - g_4) f_{1,3} - g_1 f_{2,4} (f_1 - g_3)}{(f_2 - g_4) (f_1 - g_3)}, f_{1,4} \right\} \quad (6)$$

$$\begin{aligned}
&= \frac{1}{(f_2 - g_4)(f_1 - g_3)} (f_1^2 f_{2,4} + (-f_2 f_{2,3} + f_{2,3} g_4 - 2f_{2,4} g_3) f_1 + f_2^2 f_{1,3} + (-2f_{1,3} g_4 + f_{2,3} g_3) f_2 + f_{2,4} g_3^2 - f_{2,3} g_3 g_4 + f_{1,3} g_4^2) f_{2,2} = -\frac{2f_{2,4} g_2}{f_2 - g_4} f_{3,3} \\
&= \frac{2f_3 f_{1,3}}{f_1 - g_3} f_{3,4} = \frac{f_4 (f_2 - g_4) f_{1,3} + f_3 f_{2,4} (f_1 - g_3)}{(f_2 - g_4)(f_1 - g_3)} f_{4,4} = \frac{2f_4 f_{2,4}}{f_2 - g_4} g_{1,1} = \\
&= -\frac{2g_1 g_{1,3}}{f_1 - g_3} g_{1,2} = \frac{-g_2 (f_2 - g_4) g_{1,3} - g_1 g_{2,4} (f_1 - g_3)}{(f_2 - g_4)(f_1 - g_3)} g_{2,2} = -\frac{2g_2 g_{2,4}}{f_2 - g_4} g_{2,3} \\
&= \frac{1}{(f_2 - g_4)(f_1 - g_3)} (f_1^2 g_{2,4} + (-f_2 g_{1,4} - 2g_3 g_{2,4} + g_4 g_{1,4}) f_1 + f_2^2 g_{1,3} + (g_3 g_{1,4} - 2g_4 g_{1,3}) f_2 + g_3^2 g_{2,4} - g_3 g_4 g_{1,4} + g_4^2 g_{1,3}) g_{3,3} = \frac{2f_3 g_{1,3}}{f_1 - g_3} g_{3,4} \\
&= \frac{f_4 (f_2 - g_4) g_{1,3} + f_3 g_{2,4} (f_1 - g_3)}{(f_2 - g_4)(f_1 - g_3)} g_{4,4} = \frac{2f_4 g_{2,4}}{f_2 - g_4} \}
\end{aligned}$$

These are the conditions of Monge-Ampere, but since in 3D all Monge-Ampere 2x2 systems are linearizable [see B.Doubrov, E.Ferapontov, B.Kruglikov, V.Novikov "On a class of integrable systems of Monge-Ampere type"], these are also the linearizability constraints. Next we prove that these coincide with the conditions in parametric form.

>  $MAE := \{ \}$  :for  $i$  to 2 do for  $j$  from  $i$  to 2 do  $MAE := MAE \cup \{f_{i,j} = -p_i g_j - p_j g_i, f_{i+2,j+2} = p_i f_{j+2} + p_j f_{i+2}, g_{i,j} = -q_i g_j - q_j g_i, g_{i+2,j+2} = q_i f_{j+2} + q_j f_{i+2}\}$  :od:  
od:for  $i$  to 2 do for  $j$  to 2 do  $MAE := MAE \cup \{f_{i,j+2} = a_{i,j} + p_j f_i - p_i g_{j+2}, g_{i,j+2} = b_{i,j} + q_j f_i - q_i g_{j+2}\}$  :od:od:  $MAE := subs(\{seq(seq(a_{j,i} = -a_{i,j}, j = i + 1 .. 2), i = 1 .. 2), seq(seq(b_{j,i} = -b_{i,j}, j = i + 1 .. 2), i = 1 .. 2)\}, subs(\{seq(a_{i,i} = 0, i = 1 .. 2), seq(b_{i,i} = 0, i = 1 .. 2)\}, MAE)) :$

>  $MAE$   
 $\{f_{1,1} = -2g_1 p_1, f_{1,2} = -g_1 p_2 - g_2 p_1, f_{1,3} = f_1 p_1 - g_3 p_1, f_{1,4} = f_1 p_2 - g_4 p_1 + a_{1,2}, f_{2,2} = -2g_2 p_2, f_{2,3} = f_2 p_1 - g_3 p_2 - a_{1,2}, f_{2,4} = f_2 p_2 - g_4 p_2, f_{3,3} = 2f_3 p_1, f_{3,4} = f_3 p_2 + f_4 p_1, f_{4,4} = 2f_4 p_2, g_{1,1} = -2g_1 q_1, g_{1,2} = -g_1 q_2 - g_2 q_1, g_{1,3} = f_1 q_1 - g_3 q_1, g_{1,4} = f_1 q_2 - g_4 q_1 + b_{1,2}, g_{2,2} = -2g_2 q_2, g_{2,3} = f_2 q_1 - g_3 q_2 - b_{1,2}, g_{2,4} = f_2 q_2 - g_4 q_2, g_{3,3} = 2f_3 q_1, g_{3,4} = f_3 q_2 + f_4 q_1, g_{4,4} = 2f_4 q_2\}$  (7)

>  $simplify(subs(MAE, SEQ))$   
 $\{0\}$  (8)

>  $sfgmae := simplify(subs(MAE, sfg)) : tmp := 0$  :for  $i$  to  $nops(sfgmae)$  do if  $lhs(sfgmae[i]) \neq rhs(sfgmae[i])$  then  $tmp := tmp + 1$  :fi:od:  $tmp$   
0 (9)

>

4D: now let us turn to our problem

> *interface*(*rtables*size = infinity)

10

(10)

> *var* := *u1*, *u2*, *u3*, *v1*, *v2*, *v3* : *F* := *f*(*var*) : *G* := *g*(*var*) :

> *r* := *subs*( {*u4* = *F*, *v4* = *G*}, [1, *u1*, *v1*, *u2*, *v2*, *u3*, *v3*, *u1* *v2* − *v1* *u2*, *u1* *v3* − *v1* *u3*, *u2* *v3* − *v2* *u3*, *u1* *v4* − *v1* *u4*, *u2* *v4* − *v2* *u4*, *u3* *v4* − *v3* *u4*, *u4*, *v4*] ) :

> *EQ1* := { } :for *i* to 6 do *EQ1* := *EQ1* union {*r* || *i* = *diff*(*r*, *var*[*i*])} :od: *nops*(*EQ1*)

6

(11)

> *EQ2* := { } :for *i* to 6 do for *j* from *i* to 6 do *EQ2* := *EQ2* union {*r* || *i* || *j* = *diff*(*r*, *var*[*i*], *var*[*j*])} :od:od: *nops*(*EQ2*)

21

(12)

> *Mr* := *Matrix*( [*r*, *seq*(*subs*(*EQ1*, *r* || *i*), *i* = 1 ..6), *seq*(*seq*(*subs*(*EQ2*, *r* || *i* || *j*), *j* = *i* ..6), *i* = 1 ..6) ] ) :

> *Mr2* := *eval*(*ToJet*(*Mr*[8..28, 8..15], {*F*, *G*}, *notation* = *jetnumbers*), {*u1* = 0, *v1* = 0, *u2* = 0, *v2* = 0, *u3* = 0, *v3* = 0})

(13)

$$Mr2 := \begin{bmatrix} 0 & 0 & 0 & 2g_1 & 0 & 0 & f_{1,1} & g_{1,1} \\ 0 & 0 & 0 & g_2 & g_1 & 0 & f_{1,2} & g_{1,2} \\ 0 & 0 & 0 & g_3 & 0 & g_1 & f_{1,3} & g_{1,3} \\ 0 & 0 & 0 & -f_1 + g_4 & 0 & 0 & f_{1,4} & g_{1,4} \\ 1 & 0 & 0 & g_5 & -f_1 & 0 & f_{1,5} & g_{1,5} \\ 0 & 1 & 0 & g_6 & 0 & -f_1 & f_{1,6} & g_{1,6} \\ 0 & 0 & 0 & 0 & 2g_2 & 0 & f_{2,2} & g_{2,2} \\ 0 & 0 & 0 & 0 & g_3 & g_2 & f_{2,3} & g_{2,3} \\ -1 & 0 & 0 & -f_2 & g_4 & 0 & f_{2,4} & g_{2,4} \\ 0 & 0 & 0 & 0 & -f_2 + g_5 & 0 & f_{2,5} & g_{2,5} \\ 0 & 0 & 1 & 0 & g_6 & -f_2 & f_{2,6} & g_{2,6} \\ 0 & 0 & 0 & 0 & 0 & 2g_3 & f_{3,3} & g_{3,3} \\ 0 & -1 & 0 & -f_3 & 0 & g_4 & f_{3,4} & g_{3,4} \\ 0 & 0 & -1 & 0 & -f_3 & g_5 & f_{3,5} & g_{3,5} \\ 0 & 0 & 0 & 0 & 0 & -f_3 + g_6 & f_{3,6} & g_{3,6} \\ 0 & 0 & 0 & -2f_4 & 0 & 0 & f_{4,4} & g_{4,4} \\ 0 & 0 & 0 & -f_5 & -f_4 & 0 & f_{4,5} & g_{4,5} \\ 0 & 0 & 0 & -f_6 & 0 & -f_4 & f_{4,6} & g_{4,6} \\ 0 & 0 & 0 & 0 & -2f_5 & 0 & f_{5,5} & g_{5,5} \\ 0 & 0 & 0 & 0 & -f_6 & -f_5 & f_{5,6} & g_{5,6} \\ 0 & 0 & 0 & 0 & 0 & -2f_6 & f_{6,6} & g_{6,6} \end{bmatrix} \quad (13)$$

> Mr2 := Mr2[[5, 6, 11, 1..4, 7..10, 12..21], [1..8]]

$$Mr2 := \begin{bmatrix} 1 & 0 & 0 & g_5 & -f_1 & 0 & f_{1,5} & g_{1,5} \\ 0 & 1 & 0 & g_6 & 0 & -f_1 & f_{1,6} & g_{1,6} \\ 0 & 0 & 1 & 0 & g_6 & -f_2 & f_{2,6} & g_{2,6} \\ 0 & 0 & 0 & 2g_1 & 0 & 0 & f_{1,1} & g_{1,1} \\ 0 & 0 & 0 & g_2 & g_1 & 0 & f_{1,2} & g_{1,2} \\ 0 & 0 & 0 & g_3 & 0 & g_1 & f_{1,3} & g_{1,3} \\ 0 & 0 & 0 & -f_1 + g_4 & 0 & 0 & f_{1,4} & g_{1,4} \\ 0 & 0 & 0 & 0 & 2g_2 & 0 & f_{2,2} & g_{2,2} \\ 0 & 0 & 0 & 0 & g_3 & g_2 & f_{2,3} & g_{2,3} \\ -1 & 0 & 0 & -f_2 & g_4 & 0 & f_{2,4} & g_{2,4} \\ 0 & 0 & 0 & 0 & -f_2 + g_5 & 0 & f_{2,5} & g_{2,5} \\ 0 & 0 & 0 & 0 & 0 & 2g_3 & f_{3,3} & g_{3,3} \\ 0 & -1 & 0 & -f_3 & 0 & g_4 & f_{3,4} & g_{3,4} \\ 0 & 0 & -1 & 0 & -f_3 & g_5 & f_{3,5} & g_{3,5} \\ 0 & 0 & 0 & 0 & 0 & -f_3 + g_6 & f_{3,6} & g_{3,6} \\ 0 & 0 & 0 & -2f_4 & 0 & 0 & f_{4,4} & g_{4,4} \\ 0 & 0 & 0 & -f_5 & -f_4 & 0 & f_{4,5} & g_{4,5} \\ 0 & 0 & 0 & -f_6 & 0 & -f_4 & f_{4,6} & g_{4,6} \\ 0 & 0 & 0 & 0 & -2f_5 & 0 & f_{5,5} & g_{5,5} \\ 0 & 0 & 0 & 0 & -f_6 & -f_5 & f_{5,6} & g_{5,6} \\ 0 & 0 & 0 & 0 & 0 & -2f_6 & f_{6,6} & g_{6,6} \end{bmatrix} \quad (14)$$

$\triangleright sbM := (i1, i2, i3, i4, j) \rightarrow factor(Determinant(Mr2[[1..3, i1, i2, i3, i4], [1..6, j]])) :$   
 $\triangleright SEQ := \{seq(seq(seq(seq(sbM(i1, i2, i3, i4, 7), i4 = (i3 + 1) ..21), i3 = (i2 + 1) ..21), i2 = (i1 + 1) ..21), i1 = 4 ..21), seq(seq(seq(seq(sbM(i1, i2, i3, i4, 8), i4 = (i3 + 1) ..21), i3 = (i2 + 1) ..21), i2 = (i1 + 1) ..21), i1 = 4 ..21)) : nops(\%)$   
5309 (15)

$\triangleright sfg1 := solve(SEQ, \{seq(seq(f_{i,j}, j = i ..6), i = 1 ..6), seq(seq(g_{i,j}, j = i ..6), i = 1 ..6)\}) :$   
 $\triangleright tmp := 0 : \text{for } i \text{ to } nops(sfg1) \text{ do if } lhs(sfg1[i]) = rhs(sfg1[i]) \text{ then } tmp := tmp + 1 : \text{fi. od} :$   
42, 12 (16)

$\triangleright \{seq(seq(f_{i,j}, j = i ..6), i = 1 ..6), seq(seq(g_{i,j}, j = i ..6), i = 1 ..6)\}$   
(17)

$$\{f_{1,1}, f_{1,2}, f_{1,3}, f_{1,4}, f_{1,5}, f_{1,6}, f_{2,2}, f_{2,3}, f_{2,4}, f_{2,5}, f_{2,6}, f_{3,3}, f_{3,4}, f_{3,5}, f_{3,6}, f_{4,4}, f_{4,5}, f_{4,6}, f_{5,5}, f_{5,6}, f_{6,6}, g_{1,1}, g_{1,2}, g_{1,3}, g_{1,4}, g_{1,5}, g_{1,6}, g_{2,2}, g_{2,3}, g_{2,4}, g_{2,5}, g_{2,6}, g_{3,3}, g_{3,4}, g_{3,5}, g_{3,6}, g_{4,4}, g_{4,5}, g_{4,6}, g_{5,5}, g_{5,6}, g_{6,6}\} \quad (17)$$

$$> \text{sfg} := \text{simplify}(\text{solve}(\text{SEQ}, \{f_{1,1}, f_{1,2}, f_{1,3}, f_{2,2}, f_{2,3}, f_{3,3}, f_{1,5}, f_{1,6}, f_{2,6}, f_{4,5}, f_{4,4}, f_{4,6}, f_{5,5}, f_{5,6}, f_{6,6}, g_{1,1}, g_{1,2}, g_{1,3}, g_{2,2}, g_{2,3}, g_{3,3}, g_{1,5}, g_{1,6}, g_{2,6}, g_{4,4}, g_{4,5}, g_{4,6}, g_{5,5}, g_{5,6}, g_{6,6}\}))$$

$$\text{sfg} := \left\{ f_{1,1} = -\frac{2f_{1,4}g_1}{f_1 - g_4}, f_{1,2} = \frac{-g_2(f_2 - g_5)f_{1,4} - g_1f_{2,5}(f_1 - g_4)}{(f_1 - g_4)(f_2 - g_5)}, f_{1,3} \right. \quad (18)$$

$$= \frac{-g_3(f_3 - g_6)f_{1,4} - g_1f_{3,6}(f_1 - g_4)}{(f_1 - g_4)(f_3 - g_6)}, f_{1,5} = \frac{1}{(f_2 - g_5)(f_1 - g_4)}(f_1^2 f_{2,5}$$

$$+ (-f_2 f_{2,4} + f_{2,4} g_5 - 2f_{2,5} g_4)f_1 + f_2^2 f_{1,4} + (-2f_{1,4} g_5 + f_{2,4} g_4)f_2 + f_{2,5} g_4^2$$

$$- f_{2,4} g_4 g_5 + f_{1,4} g_5^2), f_{1,6} = \frac{1}{(f_3 - g_6)(f_1 - g_4)}(f_1^2 f_{3,6} + (-f_3 f_{3,4} + f_{3,4} g_6$$

$$- 2f_{3,6} g_4)f_1 + f_3^2 f_{1,4} + (-2f_{1,4} g_6 + f_{3,4} g_4)f_3 + f_{3,6} g_4^2 - f_{3,4} g_4 g_6 + f_{1,4} g_6^2),$$

$$f_{2,2} = -\frac{2f_{2,5}g_2}{f_2 - g_5}, f_{2,3} = \frac{-g_3(f_3 - g_6)f_{2,5} - g_2f_{3,6}(f_2 - g_5)}{(f_2 - g_5)(f_3 - g_6)}, f_{2,6}$$

$$= \frac{1}{(f_3 - g_6)(f_2 - g_5)}(f_2^2 f_{3,6} + (-f_3 f_{3,5} + f_{3,5} g_6 - 2f_{3,6} g_5)f_2 + f_3^2 f_{2,5} + (-$$

$$- 2f_{2,5} g_6 + f_{3,5} g_5)f_3 + f_{3,6} g_5^2 - f_{3,5} g_5 g_6 + f_{2,5} g_6^2), f_{3,3} = -\frac{2f_{3,6}g_3}{f_3 - g_6}, f_{4,4}$$

$$= \frac{2f_4 f_{1,4}}{f_1 - g_4}, f_{4,5} = \frac{f_5(f_2 - g_5)f_{1,4} + f_4 f_{2,5}(f_1 - g_4)}{(f_1 - g_4)(f_2 - g_5)}, f_{4,6}$$

$$= \frac{f_6(f_3 - g_6)f_{1,4} + f_4 f_{3,6}(f_1 - g_4)}{(f_1 - g_4)(f_3 - g_6)}, f_{5,5} = \frac{2f_5 f_{2,5}}{f_2 - g_5}, f_{5,6}$$

$$= \frac{f_6(f_3 - g_6)f_{2,5} + f_5 f_{3,6}(f_2 - g_5)}{(f_2 - g_5)(f_3 - g_6)}, f_{6,6} = \frac{2f_6 f_{3,6}}{f_3 - g_6}, g_{1,1} = -\frac{2g_1 g_{1,4}}{f_1 - g_4}, g_{1,2}$$

$$= \frac{-g_2(f_2 - g_5)g_{1,4} - g_1 g_{2,5}(f_1 - g_4)}{(f_1 - g_4)(f_2 - g_5)}, g_{1,3}$$

$$\begin{aligned}
&= \frac{-g_3 (f_3 - g_6) g_{1,4} - g_1 g_{3,6} (f_1 - g_4)}{(f_1 - g_4) (f_3 - g_6)}, g_{1,5} = \frac{1}{(f_2 - g_5) (f_1 - g_4)} (f_1^2 g_{2,5} \\
&+ (-f_2 g_{2,4} - 2 g_4 g_{2,5} + g_5 g_{2,4}) f_1 + f_2^2 g_{1,4} + (g_4 g_{2,4} - 2 g_5 g_{1,4}) f_2 + g_4^2 g_{2,5} \\
&- g_4 g_5 g_{2,4} + g_5^2 g_{1,4}), g_{1,6} = \frac{1}{(f_3 - g_6) (f_1 - g_4)} (f_1^2 g_{3,6} + (-f_3 g_{3,4} \\
&- 2 g_4 g_{3,6} + g_6 g_{3,4}) f_1 + f_3^2 g_{1,4} + (g_4 g_{3,4} - 2 g_6 g_{1,4}) f_3 + g_4^2 g_{3,6} - g_4 g_6 g_{3,4} \\
&+ g_6^2 g_{1,4}), g_{2,2} = -\frac{2 g_2 g_{2,5}}{f_2 - g_5}, g_{2,3} = \frac{-g_3 (f_3 - g_6) g_{2,5} - g_2 g_{3,6} (f_2 - g_5)}{(f_2 - g_5) (f_3 - g_6)}, g_{2,6} \\
&= \frac{1}{(f_3 - g_6) (f_2 - g_5)} (f_2^2 g_{3,6} + (-f_3 g_{3,5} - 2 g_5 g_{3,6} + g_6 g_{3,5}) f_2 + f_3^2 g_{2,5} \\
&+ (g_5 g_{3,5} - 2 g_6 g_{2,5}) f_3 + g_5^2 g_{3,6} - g_5 g_6 g_{3,5} + g_6^2 g_{2,5}), g_{3,3} = -\frac{2 g_3 g_{3,6}}{f_3 - g_6}, g_{4,4} \\
&= \frac{2 f_4 g_{1,4}}{f_1 - g_4}, g_{4,5} = \frac{f_5 (f_2 - g_5) g_{1,4} + f_4 g_{2,5} (f_1 - g_4)}{(f_1 - g_4) (f_2 - g_5)}, g_{4,6} \\
&= \frac{f_6 (f_3 - g_6) g_{1,4} + f_4 g_{3,6} (f_1 - g_4)}{(f_1 - g_4) (f_3 - g_6)}, g_{5,5} = \frac{2 f_5 g_{2,5}}{f_2 - g_5}, g_{5,6} \\
&= \frac{f_6 (f_3 - g_6) g_{2,5} + f_5 g_{3,6} (f_2 - g_5)}{(f_2 - g_5) (f_3 - g_6)}, g_{6,6} = \frac{2 f_6 g_{3,6}}{f_3 - g_6} \}
\end{aligned}$$

> nops(sfg)

30

(19)

These are 30 equations that characterize Monge-Ampere equations, obtained similarly to 3D. Let us check that they correspond to the parametric equations (Monge-Ampere constraint for 2x2 systems)

> MAE := { } :for i to 3 do for j from i to 3 do MAE := MAE union {f<sub>i,j</sub> = -p<sub>i</sub> g<sub>j</sub> - p<sub>j</sub> g<sub>i</sub>,  
f<sub>i+3,j+3</sub> = p<sub>i</sub> f<sub>j+3</sub> + p<sub>j</sub> f<sub>i+3</sub>, g<sub>i,j</sub> = -q<sub>i</sub> g<sub>j</sub> - q<sub>j</sub> g<sub>i</sub>, g<sub>i+3,j+3</sub> = q<sub>i</sub> f<sub>j+3</sub> + q<sub>j</sub> f<sub>i+3</sub>} :od:  
od:for i to 3 do for j to 3 do MAE := MAE union {f<sub>i,j+3</sub> = a<sub>i,j</sub> + p<sub>j</sub> f<sub>i</sub> - p<sub>i</sub> g<sub>j+3</sub>, g<sub>i,j+3</sub>  
= b<sub>i,j</sub> + q<sub>j</sub> f<sub>i</sub> - q<sub>i</sub> g<sub>j+3</sub>} :od:od: MAE := subs({seq(seq(a<sub>j,i</sub> = -a<sub>i,j</sub>, j = i + 1 .. 3), i = 1  
.. 3), seq(seq(b<sub>j,i</sub> = -b<sub>i,j</sub>, j = i + 1 .. 3), i = 1 .. 3)}, subs({seq(a<sub>i,i</sub> = 0, i = 1 .. 3), seq(b<sub>i,i</sub>  
= 0, i = 1 .. 3)}), MAE) :

> MAE

$$\begin{aligned}
\{f_{1,1} = -2 g_1 p_1, f_{1,2} = -g_1 p_2 - g_2 p_1, f_{1,3} = -g_1 p_3 - g_3 p_1, f_{1,4} = f_1 p_1 - g_4 p_1, f_{1,5} = f_1 p_2 \\
- g_5 p_1 + a_{1,2}, f_{1,6} = f_1 p_3 - g_6 p_1 + a_{1,3}, f_{2,2} = -2 g_2 p_2, f_{2,3} = -g_2 p_3 - g_3 p_2, f_{2,4}
\end{aligned} \quad (20)$$

$$\begin{aligned}
&= f_2 p_1 - g_4 p_2 - a_{1,2}, f_{2,5} = f_2 p_2 - g_5 p_2, f_{2,6} = f_2 p_3 - g_6 p_2 + a_{2,3}, f_{3,3} = -2 g_3 p_3, \\
&f_{3,4} = f_3 p_1 - g_4 p_3 - a_{1,3}, f_{3,5} = f_3 p_2 - g_5 p_3 - a_{2,3}, f_{3,6} = f_3 p_3 - g_6 p_3, f_{4,4} = 2 f_4 p_1, \\
&f_{4,5} = f_4 p_2 + f_5 p_1, f_{4,6} = f_4 p_3 + f_6 p_1, f_{5,5} = 2 f_5 p_2, f_{5,6} = f_5 p_3 + f_6 p_2, f_{6,6} = 2 f_6 p_3, \\
&g_{1,1} = -2 g_1 q_1, g_{1,2} = -g_1 q_2 - g_2 q_1, g_{1,3} = -g_1 q_3 - g_3 q_1, g_{1,4} = f_1 q_1 - g_4 q_1, g_{1,5} \\
&= f_1 q_2 - g_5 q_1 + b_{1,2}, g_{1,6} = f_1 q_3 - g_6 q_1 + b_{1,3}, g_{2,2} = -2 g_2 q_2, g_{2,3} = -g_2 q_3 \\
&- g_3 q_2, g_{2,4} = f_2 q_1 - g_4 q_2 - b_{1,2}, g_{2,5} = f_2 q_2 - g_5 q_2, g_{2,6} = f_2 q_3 - g_6 q_2 + b_{2,3}, \\
&g_{3,3} = -2 g_3 q_3, g_{3,4} = f_3 q_1 - g_4 q_3 - b_{1,3}, g_{3,5} = f_3 q_2 - g_5 q_3 - b_{2,3}, g_{3,6} = f_3 q_3 \\
&- g_6 q_3, g_{4,4} = 2 f_4 q_1, g_{4,5} = f_4 q_2 + f_5 q_1, g_{4,6} = f_4 q_3 + f_6 q_1, g_{5,5} = 2 f_5 q_2, g_{5,6} = f_5 q_3 \\
&+ f_6 q_2, g_{6,6} = 2 f_6 q_3 \}
\end{aligned}$$

$$\begin{aligned}
&> \text{simplify}(\text{subs}(\text{MAE}, \text{SEQ})) \\
&\quad \{0\} \tag{21}
\end{aligned}$$

$$\begin{aligned}
&> \text{sfgmae} := \text{simplify}(\text{subs}(\text{MAE}, \text{sfg})) : \text{tmp} := 0 : \text{for } i \text{ to } \text{nops}(\text{sfgmae}) \text{ do if } \text{lhs}(\text{sfgmae}[i]) \\
&\quad \neq \text{rhs}(\text{sfgmae}[i]) \text{ then } \text{tmp} := \text{tmp} + 1 : \text{fi} : \text{od} : \text{tmp} \\
&\quad 0 \tag{22}
\end{aligned}$$

Now Plucker embedding  $\text{Gr}(4,6)$  to  $\mathbb{P}^{14}$  can be thought of as representing points in the Grassmanina by  $6 \times 6$  skew-symmetric matrices. This is the matrix  $R_0$  below. Identifying MA 2x2 system with a pencil of 2 skew-symmetric matrices we write the condition of linearizability: every matrix  $A$  in this pencil has zero determinant [see B.Doubrov, E.Ferapontov, B.Kruglikov, V.Novikov "On a class of integrable systems of Monge-Ampere type", proof of Theorem 2: for the normal forms it is straightforward to check that  $\det(A)=0$  or better  $\text{Pf}(A)=0$  holds iff the equation is linear]. This gives linearizability conditions of Monge-Ampere equations, that in addition to the above 30 equations form 4 new equations, denoted I1,I2,I3,I4 below.

$$\begin{aligned}
&> P := \text{subs}(\{u4 = F, v4 = G\}, \text{Matrix}([ [1, 0, u1, u2, u3, u4], [0, 1, v1, v2, v3, v4]])) \\
&\quad P := \begin{bmatrix} 1 & 0 & u1 & u2 & u3 & f(u1, u2, u3, v1, v2, v3) \\ 0 & 1 & v1 & v2 & v3 & g(u1, u2, u3, v1, v2, v3) \end{bmatrix} \tag{23}
\end{aligned}$$

$$> r := (i, j) \rightarrow \text{Determinant}(P[[1, 2], [i, j]]) :$$

$$> R := \text{Matrix}(6, r) :$$

$$> R_0 := \text{ToJet}(R, \{F, G\}, \text{notation} = \text{jetnumbers})$$

$$R_0 := \begin{bmatrix} 0 & 1 & v1 & v2 & v3 & g_{[]} \\ -1 & 0 & -u1 & -u2 & -u3 & -f_{[]} \\ -v1 & u1 & 0 & u1 v2 - u2 v1 & u1 v3 - u3 v1 & u1 g_{[]} - v1 f_{[]} \\ -v2 & u2 & -u1 v2 + u2 v1 & 0 & u2 v3 - u3 v2 & u2 g_{[]} - v2 f_{[]} \\ -v3 & u3 & -u1 v3 + u3 v1 & -u2 v3 + u3 v2 & 0 & u3 g_{[]} - v3 f_{[]} \\ -g_{[]} & f_{[]} & -u1 g_{[]} + v1 f_{[]} & -u2 g_{[]} + v2 f_{[]} & -u3 g_{[]} + v3 f_{[]} & 0 \end{bmatrix} \tag{24}$$

$$> \text{for } i \text{ to } \text{nops}(\{\text{var}\}) \text{ do } r := (a, b) \rightarrow \text{diff}(R[a, b], \text{var}[i]) : R || i := \text{ToJet}(\text{Matrix}(6, r), \{F, G\}, \text{notation} = \text{jetnumbers}) : \text{od} :$$

> **for**  $i$  **to**  $nops(\{var\})$  **do** **for**  $j$  **from**  $i$  **to** 6 **do**  $r := (a, b) \rightarrow diff(R[a, b], var[i], var[j]) : R || i || j$   
 $:= ToJet(Matrix(6, r), \{F, G\}, notation = jetnumbers) : od: od:$

>  $A := Matrix(6, a, shape = antisymmetric)$

$$A := \begin{bmatrix} 0 & a(1, 2) & a(1, 3) & a(1, 4) & a(1, 5) & a(1, 6) \\ -a(1, 2) & 0 & a(2, 3) & a(2, 4) & a(2, 5) & a(2, 6) \\ -a(1, 3) & -a(2, 3) & 0 & a(3, 4) & a(3, 5) & a(3, 6) \\ -a(1, 4) & -a(2, 4) & -a(3, 4) & 0 & a(4, 5) & a(4, 6) \\ -a(1, 5) & -a(2, 5) & -a(3, 5) & -a(4, 5) & 0 & a(5, 6) \\ -a(1, 6) & -a(2, 6) & -a(3, 6) & -a(4, 6) & -a(5, 6) & 0 \end{bmatrix} \quad (25)$$

>  $factor(Determinant(A))$

$$(a(5, 6) a(1, 4) a(2, 3) + a(1, 6) a(4, 5) a(2, 3) - a(1, 5) a(4, 6) a(2, 3) + a(5, 6) a(3, 4) a(1, 2) + a(3, 4) a(1, 6) a(2, 5) - a(3, 4) a(1, 5) a(2, 6) - a(5, 6) a(1, 3) a(2, 4) + a(3, 6) a(4, 5) a(1, 2) - a(4, 5) a(1, 3) a(2, 6) - a(3, 6) a(1, 4) a(2, 5) + a(3, 6) a(1, 5) a(2, 4) - a(3, 5) a(4, 6) a(1, 2) + a(4, 6) a(1, 3) a(2, 5) + a(3, 5) a(1, 4) a(2, 6) - a(3, 5) a(1, 6) a(2, 4))^2 \quad (26)$$

>  $Pf := a \rightarrow a[5, 6] a[1, 2] a[3, 4] + a[3, 4] a[1, 6] a[2, 5] - a[3, 4] a[1, 5] a[2, 6] + a[1, 4] a[5, 6] a[2, 3] - a[5, 6] a[1, 3] a[2, 4] + a[3, 6] a[4, 5] a[1, 2] + a[1, 6] a[4, 5] a[2, 3] - a[4, 5] a[1, 3] a[2, 6] - a[3, 6] a[1, 4] a[2, 5] + a[3, 6] a[1, 5] a[2, 4] - a[3, 5] a[4, 6] a[1, 2] - a[1, 5] a[4, 6] a[2, 3] + a[4, 6] a[1, 3] a[2, 5] + a[3, 5] a[1, 4] a[2, 6] - a[3, 5] a[1, 6] a[2, 4] :$

>  $simplify(Determinant(A) - Pf(A)^2)$   
0 (27)

>  $maeq := subs(MAE, subs(sfg, \{Trace(A.R0), seq(Trace(A.R || i), i = 1..6), seq(seq(Trace(A.R || i || j), j = i..6), i = 1..6)\})):$

>  $sA := solve(maeq, \{seq(seq(a(i, j), j = (i + 1)..6), i = 1..6)\} :$

>  $tmp := \{ \} : \text{for } i \text{ to } nops(sA) \text{ do if } lhs(sA[i]) = rhs(sA[i]) \text{ then } tmp := tmp \cup \{lhs(sA[i])\} : fi: od: tmp$   
 $\{a(4, 6), a(5, 6)\}$  (28)

>  $sA0 := subs(\{a(4, 6) = x, a(5, 6) = y\}, subs(sA, A))$

$$sA0 := \left[ \left[ 0, \frac{1}{p_2 q_3 - p_3 q_2} (u^2 f_2 q_3 x + v^3 g_6 p_2 y - u l f_1 q_2 y + u l f_1 q_3 x + u l g_1 p_2 y \right. \right. \quad (29)$$

$$\left. - u l g_1 p_3 x - v^3 f_6 q_2 y + v^3 f_6 q_3 x - v^3 g_6 p_3 x - v^2 f_5 q_2 y + v^2 f_5 q_3 x + v^2 g_5 p_2 y \right.$$

$$\left. - v^2 g_5 p_3 x - u^3 f_3 q_2 y + u^3 f_3 q_3 x + u^3 g_3 p_2 y - u^3 g_3 p_3 x - u^2 f_2 q_2 y + u^2 g_2 p_2 y \right.$$

$$\left. - u^2 g_2 p_3 x - v l f_4 q_2 y + v l f_4 q_3 x + v l g_4 p_2 y - v l g_4 p_3 x - f_{[]} q_3 x - g_{[]} p_2 y \right]$$

$$\begin{aligned}
& + g_{[]} p_3 x + f_{[]} q_2 y - ul g_{[]} p_1 q_2 y + ul g_{[]} p_1 q_3 x + ul g_{[]} p_2 q_1 y - ul g_{[]} p_3 q_1 x \\
& + ul v_2 a_{1,2} q_2 y - ul v_2 a_{1,2} q_3 x - ul v_2 b_{1,2} p_2 y + ul v_2 b_{1,2} p_3 x - u_2 vl a_{1,2} q_2 y \\
& + u_2 vl a_{1,2} q_3 x + u_2 vl b_{1,2} p_2 y - u_2 vl b_{1,2} p_3 x + ul v_3 a_{1,3} q_2 y - ul v_3 a_{1,3} q_3 x \\
& - ul v_3 b_{1,3} p_2 y + ul v_3 b_{1,3} p_3 x - u_3 vl a_{1,3} q_2 y + u_3 vl a_{1,3} q_3 x + u_3 vl b_{1,3} p_2 y \\
& - u_3 vl b_{1,3} p_3 x + u_2 v_3 a_{2,3} q_2 y - u_2 v_3 a_{2,3} q_3 x - u_2 v_3 b_{2,3} p_2 y + u_2 v_3 b_{2,3} p_3 x \\
& - u_3 v_2 a_{2,3} q_2 y + u_3 v_2 a_{2,3} q_3 x + u_3 v_2 b_{2,3} p_2 y - u_3 v_2 b_{2,3} p_3 x - v_3 f_{[]} p_2 q_3 y \\
& + v_3 f_{[]} p_3 q_2 y - v_2 f_{[]} p_2 q_3 x + v_2 f_{[]} p_3 q_2 x + u_3 g_{[]} p_2 q_3 y - u_3 g_{[]} p_3 q_2 y \\
& + u_2 g_{[]} p_2 q_3 x - u_2 g_{[]} p_3 q_2 x + vl f_{[]} p_1 q_2 y - vl f_{[]} p_1 q_3 x - vl f_{[]} p_2 q_1 y \\
& + vl f_{[]} p_3 q_1 x), \frac{1}{p_2 q_3 - p_3 q_2} (-u_2 x a_{1,2} q_3 + u_2 x b_{1,2} p_3 + u_2 y a_{1,2} q_2 \\
& - u_2 y b_{1,2} p_2 - u_3 x a_{1,3} q_3 + u_3 x b_{1,3} p_3 + u_3 y a_{1,3} q_2 - u_3 y b_{1,3} p_2 + x f_{[]} p_1 q_3 \\
& - x f_{[]} p_3 q_1 - y f_{[]} p_1 q_2 + y f_{[]} p_2 q_1 - x f_4 q_3 + x g_4 p_3 + y f_4 q_2 - y g_4 p_2), \\
& - \frac{1}{p_2 q_3 - p_3 q_2} (-ul x a_{1,2} q_3 + ul x b_{1,2} p_3 + ul y a_{1,2} q_2 - ul y b_{1,2} p_2 \\
& + u_3 x a_{2,3} q_3 - u_3 x b_{2,3} p_3 - u_3 y a_{2,3} q_2 + u_3 y b_{2,3} p_2 - x f_{[]} p_2 q_3 + x f_{[]} p_3 q_2 \\
& + x f_5 q_3 - x g_5 p_3 - y f_5 q_2 + y g_5 p_2), - \frac{1}{p_2 q_3 - p_3 q_2} (-ul x a_{1,3} q_3 \\
& + ul x b_{1,3} p_3 + ul y a_{1,3} q_2 - ul y b_{1,3} p_2 - u_2 x a_{2,3} q_3 + u_2 x b_{2,3} p_3 + u_2 y a_{2,3} q_2 \\
& - u_2 y b_{2,3} p_2 - y f_{[]} p_2 q_3 + y f_{[]} p_3 q_2 + x f_6 q_3 - x g_6 p_3 - y f_6 q_2 + y g_6 p_2),
\end{aligned}$$

$$\begin{aligned}
& \frac{1}{p_2 q_3 - p_3 q_2} \left( -ul x p_1 q_3 + ul x p_3 q_1 + ul y p_1 q_2 - ul y p_2 q_1 - u2 x p_2 q_3 \right. \\
& \left. + u2 x p_3 q_2 - u3 y p_2 q_3 + u3 y p_3 q_2 - x p_3 + y p_2 \right), \\
& \left[ -\frac{1}{p_2 q_3 - p_3 q_2} \left( u2 f_2 q_3 x + v3 g_6 p_2 y - ul f_1 q_2 y + ul f_1 q_3 x + ul g_1 p_2 y \right. \right. \\
& - ul g_1 p_3 x - v3 f_6 q_2 y + v3 f_6 q_3 x - v3 g_6 p_3 x - v2 f_5 q_2 y + v2 f_5 q_3 x + v2 g_5 p_2 y \\
& - v2 g_5 p_3 x - u3 f_3 q_2 y + u3 f_3 q_3 x + u3 g_3 p_2 y - u3 g_3 p_3 x - u2 f_2 q_2 y + u2 g_2 p_2 y \\
& - u2 g_2 p_3 x - vl f_4 q_2 y + vl f_4 q_3 x + vl g_4 p_2 y - vl g_4 p_3 x - f_{[]} q_3 x - g_{[]} p_2 y \\
& + g_{[]} p_3 x + f_{[]} q_2 y - ul g_{[]} p_1 q_2 y + ul g_{[]} p_1 q_3 x + ul g_{[]} p_2 q_1 y - ul g_{[]} p_3 q_1 x \\
& + ul v2 a_{1,2} q_2 y - ul v2 a_{1,2} q_3 x - ul v2 b_{1,2} p_2 y + ul v2 b_{1,2} p_3 x - u2 vl a_{1,2} q_2 y \\
& + u2 vl a_{1,2} q_3 x + u2 vl b_{1,2} p_2 y - u2 vl b_{1,2} p_3 x + ul v3 a_{1,3} q_2 y - ul v3 a_{1,3} q_3 x \\
& - ul v3 b_{1,3} p_2 y + ul v3 b_{1,3} p_3 x - u3 vl a_{1,3} q_2 y + u3 vl a_{1,3} q_3 x + u3 vl b_{1,3} p_2 y \\
& - u3 vl b_{1,3} p_3 x + u2 v3 a_{2,3} q_2 y - u2 v3 a_{2,3} q_3 x - u2 v3 b_{2,3} p_2 y + u2 v3 b_{2,3} p_3 x \\
& - u3 v2 a_{2,3} q_2 y + u3 v2 a_{2,3} q_3 x + u3 v2 b_{2,3} p_2 y - u3 v2 b_{2,3} p_3 x - v3 f_{[]} p_2 q_3 y \\
& + v3 f_{[]} p_3 q_2 y - v2 f_{[]} p_2 q_3 x + v2 f_{[]} p_3 q_2 x + u3 g_{[]} p_2 q_3 y - u3 g_{[]} p_3 q_2 y \\
& + u2 g_{[]} p_2 q_3 x - u2 g_{[]} p_3 q_2 x + vl f_{[]} p_1 q_2 y - vl f_{[]} p_1 q_3 x - vl f_{[]} p_2 q_1 y \\
& + vl f_{[]} p_3 q_1 x), 0, \frac{1}{p_2 q_3 - p_3 q_2} \left( -v2 x a_{1,2} q_3 + v2 x b_{1,2} p_3 + v2 y a_{1,2} q_2 \right. \\
& \left. - v2 y b_{1,2} p_2 - v3 x a_{1,3} q_3 + v3 x b_{1,3} p_3 + v3 y a_{1,3} q_2 - v3 y b_{1,3} p_2 + x g_{[]} p_1 q_3 \right.
\end{aligned}$$

$$\begin{aligned}
& -xg_{[]}p_3q_1 - yg_{[]}p_1q_2 + yg_{[]}p_2q_1 + xf_1q_3 - xg_1p_3 - yf_1q_2 + yg_1p_2), \\
& -\frac{1}{p_2q_3 - p_3q_2} \left( -vlxa_{1,2}q_3 + vlx b_{1,2}p_3 + vly a_{1,2}q_2 - vly b_{1,2}p_2 \right. \\
& + v3xa_{2,3}q_3 - v3xb_{2,3}p_3 - v3ya_{2,3}q_2 + v3yb_{2,3}p_2 - xg_{[]}p_2q_3 + xg_{[]}p_3q_2 \\
& - xf_2q_3 + xg_2p_3 + yf_2q_2 - yg_2p_2), -\frac{1}{p_2q_3 - p_3q_2} \left( -vlix a_{1,3}q_3 \right. \\
& + vlix b_{1,3}p_3 + vly a_{1,3}q_2 - vly b_{1,3}p_2 - v2xa_{2,3}q_3 + v2xb_{2,3}p_3 + v2ya_{2,3}q_2 \\
& - v2yb_{2,3}p_2 - yg_{[]}p_2q_3 + yg_{[]}p_3q_2 - xf_3q_3 + xg_3p_3 + yf_3q_2 - yg_3p_2), \\
& \frac{1}{p_2q_3 - p_3q_2} \left( -vlix p_1q_3 + vlix p_3q_1 + vly p_1q_2 - vly p_2q_1 - v2xp_2q_3 \right. \\
& \left. + v2xp_3q_2 - v3yp_2q_3 + v3yp_3q_2 - xq_3 + yq_2 \right) \Big], \\
& \left[ -\frac{1}{p_2q_3 - p_3q_2} \left( -u2xa_{1,2}q_3 + u2xb_{1,2}p_3 + u2ya_{1,2}q_2 - u2yb_{1,2}p_2 \right. \right. \\
& - u3xa_{1,3}q_3 + u3xb_{1,3}p_3 + u3ya_{1,3}q_2 - u3yb_{1,3}p_2 + xf_{[]}p_1q_3 - xf_{[]}p_3q_1 \\
& - yf_{[]}p_1q_2 + yf_{[]}p_2q_1 - xf_4q_3 + xg_4p_3 + yf_4q_2 - yg_4p_2), -\frac{1}{p_2q_3 - p_3q_2} \left( \right. \\
& -v2xa_{1,2}q_3 + v2xb_{1,2}p_3 + v2ya_{1,2}q_2 - v2yb_{1,2}p_2 - v3xa_{1,3}q_3 + v3xb_{1,3}p_3 \\
& + v3ya_{1,3}q_2 - v3yb_{1,3}p_2 + xg_{[]}p_1q_3 - xg_{[]}p_3q_1 - yg_{[]}p_1q_2 + yg_{[]}p_2q_1 \\
& \left. + xf_1q_3 - xg_1p_3 - yf_1q_2 + yg_1p_2 \right), 0, \\
& \frac{-xa_{1,2}q_3 + xb_{1,2}p_3 + ya_{1,2}q_2 - yb_{1,2}p_2}{p_2q_3 - p_3q_2}, \\
& \frac{-xa_{1,3}q_3 + xb_{1,3}p_3 + ya_{1,3}q_2 - yb_{1,3}p_2}{p_2q_3 - p_3q_2},
\end{aligned}$$

$$\begin{aligned}
& - \frac{-x p_1 q_3 + x p_3 q_1 + y p_1 q_2 - y p_2 q_1}{p_2 q_3 - p_3 q_2} \Bigg], \\
& \left[ \frac{1}{p_2 q_3 - p_3 q_2} \left( -ul x a_{1,2} q_3 + ul x b_{1,2} p_3 + ul y a_{1,2} q_2 - ul y b_{1,2} p_2 \right. \right. \\
& + u^3 x a_{2,3} q_3 - u^3 x b_{2,3} p_3 - u^3 y a_{2,3} q_2 + u^3 y b_{2,3} p_2 - x f_{[]} p_2 q_3 + x f_{[]} p_3 q_2 \\
& + x f_5 q_3 - x g_5 p_3 - y f_5 q_2 + y g_5 p_2 \Big), \frac{1}{p_2 q_3 - p_3 q_2} \left( -vl x a_{1,2} q_3 + vl x b_{1,2} p_3 \right. \\
& + vl y a_{1,2} q_2 - vl y b_{1,2} p_2 + v^3 x a_{2,3} q_3 - v^3 x b_{2,3} p_3 - v^3 y a_{2,3} q_2 + v^3 y b_{2,3} p_2 \\
& - x g_{[]} p_2 q_3 + x g_{[]} p_3 q_2 - x f_2 q_3 + x g_2 p_3 + y f_2 q_2 - y g_2 p_2 \Big), \\
& - \frac{-x a_{1,2} q_3 + x b_{1,2} p_3 + y a_{1,2} q_2 - y b_{1,2} p_2}{p_2 q_3 - p_3 q_2}, 0, \\
& \left. \frac{-x a_{2,3} q_3 + x b_{2,3} p_3 + y a_{2,3} q_2 - y b_{2,3} p_2}{p_2 q_3 - p_3 q_2}, x \right], \\
& \left[ \frac{1}{p_2 q_3 - p_3 q_2} \left( -ul x a_{1,3} q_3 + ul x b_{1,3} p_3 + ul y a_{1,3} q_2 - ul y b_{1,3} p_2 \right. \right. \\
& - u^2 x a_{2,3} q_3 + u^2 x b_{2,3} p_3 + u^2 y a_{2,3} q_2 - u^2 y b_{2,3} p_2 - y f_{[]} p_2 q_3 + y f_{[]} p_3 q_2 \\
& + x f_6 q_3 - x g_6 p_3 - y f_6 q_2 + y g_6 p_2 \Big), \frac{1}{p_2 q_3 - p_3 q_2} \left( -vl x a_{1,3} q_3 + vl x b_{1,3} p_3 \right. \\
& + vl y a_{1,3} q_2 - vl y b_{1,3} p_2 - v^2 x a_{2,3} q_3 + v^2 x b_{2,3} p_3 + v^2 y a_{2,3} q_2 - v^2 y b_{2,3} p_2 \\
& - y g_{[]} p_2 q_3 + y g_{[]} p_3 q_2 - x f_3 q_3 + x g_3 p_3 + y f_3 q_2 - y g_3 p_2 \Big), \\
& - \frac{-x a_{1,3} q_3 + x b_{1,3} p_3 + y a_{1,3} q_2 - y b_{1,3} p_2}{p_2 q_3 - p_3 q_2}, \\
& - \frac{-x a_{2,3} q_3 + x b_{2,3} p_3 + y a_{2,3} q_2 - y b_{2,3} p_2}{p_2 q_3 - p_3 q_2}, 0, y \Big], \\
& \left[ - \frac{1}{p_2 q_3 - p_3 q_2} \left( -ul x p_1 q_3 + ul x p_3 q_1 + ul y p_1 q_2 - ul y p_2 q_1 - u^2 x p_2 q_3 \right. \right.
\end{aligned}$$

$$\begin{aligned}
& + u^2 x p_3 q_2 - u^3 y p_2 q_3 + u^3 y p_3 q_2 - x p_3 + y p_2), - \frac{1}{p_2 q_3 - p_3 q_2} ( -v l x p_1 q_3 \\
& + v l x p_3 q_1 + v l y p_1 q_2 - v l y p_2 q_1 - v^2 x p_2 q_3 + v^2 x p_3 q_2 - v^3 y p_2 q_3 + v^3 y p_3 q_2 \\
& - x q_3 + y q_2), \frac{-x p_1 q_3 + x p_3 q_1 + y p_1 q_2 - y p_2 q_1}{p_2 q_3 - p_3 q_2}, -x, -y, 0 \Big] \Big]
\end{aligned}$$

> Q3 := simplify(Pf(sA0)) :

> I1 := factor  $\left( \frac{1}{6} \text{numer}(\text{diff}(Q3, x, x, x)) \right)$

$$\begin{aligned}
I1 := & f_1 f_6 p_2 q_3^3 - f_1 f_6 p_3 q_2 q_3^2 - f_1 g_6 p_2 p_3 q_3^2 + f_1 g_6 p_3^2 q_2 q_3 - f_2 f_6 p_1 q_3^3 + f_2 f_6 p_3 q_1 q_3^2 \\
& + f_2 g_6 p_1 p_3 q_3^2 - f_2 g_6 p_3^2 q_1 q_3 - f_3 f_4 p_2 q_3^3 + f_3 f_4 p_3 q_2 q_3^2 + f_3 f_5 p_1 q_3^3 - f_3 f_5 p_3 q_1 q_3^2 \\
& + f_3 g_4 p_2 p_3 q_3^2 - f_3 g_4 p_3^2 q_2 q_3 - f_3 g_5 p_1 p_3 q_3^2 + f_3 g_5 p_3^2 q_1 q_3 + f_4 g_3 p_2 p_3 q_3^2 - f_4 g_3 \\
& p_3^2 q_2 q_3 - f_5 g_3 p_1 p_3 q_3^2 + f_5 g_3 p_3^2 q_1 q_3 - f_6 g_1 p_2 p_3 q_3^2 + f_6 g_1 p_3^2 q_2 q_3 + f_6 g_2 p_1 p_3 q_3^2 \\
& - f_6 g_2 p_3^2 q_1 q_3 + g_1 g_6 p_2 p_3^2 q_3 - g_1 g_6 p_3^3 q_2 - g_2 g_6 p_1 p_3^2 q_3 + g_2 g_6 p_3^3 q_1 - g_3 g_4 p_2 \\
& p_3^2 q_3 + g_3 g_4 p_3^3 q_2 + g_3 g_5 p_1 p_3^2 q_3 - g_3 g_5 p_3^3 q_1 + a_{1,2} f_3 p_3 q_3^2 + a_{1,2} f_6 q_3^3 - a_{1,2} g_3 \\
& p_3^2 q_3 - a_{1,2} g_6 p_3 q_3^2 - a_{1,3} f_2 p_3 q_3^2 - a_{1,3} f_5 q_3^3 + a_{1,3} g_2 p_3^2 q_3 + a_{1,3} g_5 p_3 q_3^2 \\
& + a_{2,3} f_1 p_3 q_3^2 + a_{2,3} f_4 q_3^3 - a_{2,3} g_1 p_3^2 q_3 - a_{2,3} g_4 p_3 q_3^2 - b_{1,2} f_3 p_3^2 q_3 - b_{1,2} f_6 p_3 \\
& q_3^2 + b_{1,2} g_3 p_3^3 + b_{1,2} g_6 p_3^2 q_3 + b_{1,3} f_2 p_3^2 q_3 + b_{1,3} f_5 p_3 q_3^2 - b_{1,3} g_2 p_3^3 - b_{1,3} g_5 \\
& p_3^2 q_3 - b_{2,3} f_1 p_3^2 q_3 - b_{2,3} f_4 p_3 q_3^2 + b_{2,3} g_1 p_3^3 + b_{2,3} g_4 p_3^2 q_3
\end{aligned} \tag{30}$$

> I2 := factor  $\left( \frac{1}{2} \text{numer}(\text{diff}(Q3, x, x, y)) \right)$

$$\begin{aligned}
I2 := & -f_1 f_5 p_2 q_3^3 + f_1 f_5 p_3 q_2 q_3^2 - 2 f_1 f_6 p_2 q_2 q_3^2 + 2 f_1 f_6 p_3 q_2^2 q_3 + f_1 g_5 p_2 p_3 q_3^2 - f_1 g_5 \\
& p_3^2 q_2 q_3 + f_1 g_6 p_2^2 q_3^2 - f_1 g_6 p_3^2 q_2^2 + f_2 f_4 p_2 q_3^3 - f_2 f_4 p_3 q_2 q_3^2 + 3 f_2 f_6 p_1 q_2 q_3^2 \\
& - f_2 f_6 p_2 q_1 q_3^2 - 2 f_2 f_6 p_3 q_1 q_2 q_3 - f_2 g_4 p_2 p_3 q_3^2 + f_2 g_4 p_3^2 q_2 q_3 - f_2 g_6 p_1 p_2 q_3^2 \\
& - 2 f_2 g_6 p_1 p_3 q_2 q_3 + 2 f_2 g_6 p_2 p_3 q_1 q_3 + f_2 g_6 p_3^2 q_1 q_2 + 2 f_3 f_4 p_2 q_2 q_3^2 - 2 f_3 f_4 p_3 \\
& q_2^2 q_3 - 3 f_3 f_5 p_1 q_2 q_3^2 + f_3 f_5 p_2 q_1 q_3^2 + 2 f_3 f_5 p_3 q_1 q_2 q_3 - f_3 g_4 p_2^2 q_3^2 + f_3 g_4 p_3^2 q_2^2 \\
& + f_3 g_5 p_1 p_2 q_3^2 + 2 f_3 g_5 p_1 p_3 q_2 q_3 - 2 f_3 g_5 p_2 p_3 q_1 q_3 - f_3 g_5 p_3^2 q_1 q_2 - f_4 g_2 p_2 p_3 \\
& q_3^2 + f_4 g_2 p_3^2 q_2 q_3 - f_4 g_3 p_2^2 q_3^2 + f_4 g_3 p_3^2 q_2^2 + f_5 g_1 p_2 p_3 q_3^2 - f_5 g_1 p_3^2 q_2 q_3 \\
& + f_5 g_3 p_1 p_2 q_3^2 + 2 f_5 g_3 p_1 p_3 q_2 q_3 - 2 f_5 g_3 p_2 p_3 q_1 q_3 - f_5 g_3 p_3^2 q_1 q_2 + f_6 g_1 p_2^2 q_3^2 \\
& - f_6 g_1 p_3^2 q_2^2 - f_6 g_2 p_1 p_2 q_3^2 - 2 f_6 g_2 p_1 p_3 q_2 q_3 + 2 f_6 g_2 p_2 p_3 q_1 q_3 + f_6 g_2 p_3^2 q_1 q_2
\end{aligned} \tag{31}$$

$$\begin{aligned}
& -g_1 g_5 p_2 p_3^2 q_3 + g_1 g_5 p_3^3 q_2 - 2 g_1 g_6 p_2^2 p_3 q_3 + 2 g_1 g_6 p_2 p_3^2 q_2 + g_2 g_4 p_2 p_3^2 q_3 \\
& - g_2 g_4 p_3^3 q_2 + 2 g_2 g_6 p_1 p_2 p_3 q_3 + g_2 g_6 p_1 p_3^2 q_2 - 3 g_2 g_6 p_2 p_3^2 q_1 + 2 g_3 g_4 p_2^2 p_3 q_3 \\
& - 2 g_3 g_4 p_2 p_3^2 q_2 - 2 g_3 g_5 p_1 p_2 p_3 q_3 - g_3 g_5 p_1 p_3^2 q_2 + 3 g_3 g_5 p_2 p_3^2 q_1 - a_{1,2} f_3 p_2 \\
& q_3^2 - 2 a_{1,2} f_3 p_3 q_2 q_3 - 3 a_{1,2} f_6 q_2 q_3^2 + 2 a_{1,2} g_3 p_2 p_3 q_3 + a_{1,2} g_3 p_3^2 q_2 + a_{1,2} g_6 p_2 \\
& q_3^2 + 2 a_{1,2} g_6 p_3 q_2 q_3 + a_{1,3} f_2 p_2 q_3^2 + 2 a_{1,3} f_2 p_3 q_2 q_3 + 3 a_{1,3} f_5 q_2 q_3^2 \\
& - 2 a_{1,3} g_2 p_2 p_3 q_3 - a_{1,3} g_2 p_3^2 q_2 - a_{1,3} g_5 p_2 q_3^2 - 2 a_{1,3} g_5 p_3 q_2 q_3 - a_{2,3} f_1 p_2 q_3^2 \\
& - 2 a_{2,3} f_1 p_3 q_2 q_3 - 3 a_{2,3} f_4 q_2 q_3^2 + 2 a_{2,3} g_1 p_2 p_3 q_3 + a_{2,3} g_1 p_3^2 q_2 + a_{2,3} g_4 p_2 q_3^2 \\
& + 2 a_{2,3} g_4 p_3 q_2 q_3 + 2 b_{1,2} f_3 p_2 p_3 q_3 + b_{1,2} f_3 p_3^2 q_2 + b_{1,2} f_6 p_2 q_3^2 \\
& + 2 b_{1,2} f_6 p_3 q_2 q_3 - 3 b_{1,2} g_3 p_2 p_3^2 - 2 b_{1,2} g_6 p_2 p_3 q_3 - b_{1,2} g_6 p_3^2 q_2 \\
& - 2 b_{1,3} f_2 p_2 p_3 q_3 - b_{1,3} f_2 p_3^2 q_2 - b_{1,3} f_5 p_2 q_3^2 - 2 b_{1,3} f_5 p_3 q_2 q_3 + 3 b_{1,3} g_2 p_2 p_3^2 \\
& + 2 b_{1,3} g_5 p_2 p_3 q_3 + b_{1,3} g_5 p_3^2 q_2 + 2 b_{2,3} f_1 p_2 p_3 q_3 + b_{2,3} f_1 p_3^2 q_2 + b_{2,3} f_4 p_2 q_3^2 \\
& + 2 b_{2,3} f_4 p_3 q_2 q_3 - 3 b_{2,3} g_1 p_2 p_3^2 - 2 b_{2,3} g_4 p_2 p_3 q_3 - b_{2,3} g_4 p_3^2 q_2
\end{aligned}$$

$$\triangleright I3 := \text{factor} \left( \frac{1}{2} \text{numer}(\text{diff}(Q3, x, y, y)) \right)$$

$$\begin{aligned}
I3 := & 2 f_1 f_5 p_2 q_2 q_3^2 - 2 f_1 f_5 p_3 q_2^2 q_3 + f_1 f_6 p_2 q_2^2 q_3 - f_1 f_6 p_3 q_2^3 - f_1 g_5 p_2^2 q_3^2 + f_1 g_5 p_3^2 q_2^2 \quad (32) \\
& - f_1 g_6 p_2^2 q_2 q_3 + f_1 g_6 p_2 p_3 q_2^2 - 2 f_2 f_4 p_2 q_2 q_3^2 + 2 f_2 f_4 p_3 q_2^2 q_3 - 3 f_2 f_6 p_1 q_2^2 q_3 \\
& + 2 f_2 f_6 p_2 q_1 q_2 q_3 + f_2 f_6 p_3 q_1 q_2^2 + f_2 g_4 p_2^2 q_3^2 - f_2 g_4 p_3^2 q_2^2 + 2 f_2 g_6 p_1 p_2 q_2 q_3 \\
& + f_2 g_6 p_1 p_3 q_2^2 - f_2 g_6 p_2^2 q_1 q_3 - 2 f_2 g_6 p_2 p_3 q_1 q_2 - f_3 f_4 p_2 q_2^2 q_3 + f_3 f_4 p_3 q_2^3 \\
& + 3 f_3 f_5 p_1 q_2^2 q_3 - 2 f_3 f_5 p_2 q_1 q_2 q_3 - f_3 f_5 p_3 q_1 q_2^2 + f_3 g_4 p_2^2 q_2 q_3 - f_3 g_4 p_2 p_3 q_2^2 \\
& - 2 f_3 g_5 p_1 p_2 q_2 q_3 - f_3 g_5 p_1 p_3 q_2^2 + f_3 g_5 p_2^2 q_1 q_3 + 2 f_3 g_5 p_2 p_3 q_1 q_2 + f_4 g_2 p_2^2 q_3^2 \\
& - f_4 g_2 p_3^2 q_2^2 + f_4 g_3 p_2^2 q_2 q_3 - f_4 g_3 p_2 p_3 q_2^2 - f_5 g_1 p_2^2 q_3^2 + f_5 g_1 p_3^2 q_2^2 \\
& - 2 f_5 g_3 p_1 p_2 q_2 q_3 - f_5 g_3 p_1 p_3 q_2^2 + f_5 g_3 p_2^2 q_1 q_3 + 2 f_5 g_3 p_2 p_3 q_1 q_2 - f_6 g_1 \\
& p_2^2 q_2 q_3 + f_6 g_1 p_2 p_3 q_2^2 + 2 f_6 g_2 p_1 p_2 q_2 q_3 + f_6 g_2 p_1 p_3 q_2^2 - f_6 g_2 p_2^2 q_1 q_3 \\
& - 2 f_6 g_2 p_2 p_3 q_1 q_2 + 2 g_1 g_5 p_2^2 p_3 q_3 - 2 g_1 g_5 p_2 p_3^2 q_2 + g_1 g_6 p_2^3 q_3 - g_1 g_6 p_2^2 p_3 q_2 \\
& - 2 g_2 g_4 p_2^2 p_3 q_3 + 2 g_2 g_4 p_2 p_3^2 q_2 - g_2 g_6 p_1 p_2^2 q_3 - 2 g_2 g_6 p_1 p_2 p_3 q_2 + 3 g_2 g_6 \\
& p_2^2 p_3 q_1 - g_3 g_4 p_2^3 q_3 + g_3 g_4 p_2^2 p_3 q_2 + g_3 g_5 p_1 p_2^2 q_3 + 2 g_3 g_5 p_1 p_2 p_3 q_2 - 3 g_3 g_5 \\
& p_2^2 p_3 q_1 + 2 a_{1,2} f_3 p_2 q_2 q_3 + a_{1,2} f_3 p_3 q_2^2 + 3 a_{1,2} f_6 q_2^2 q_3 - a_{1,2} g_3 p_2^2 q_3 \\
& - 2 a_{1,2} g_3 p_2 p_3 q_2 - 2 a_{1,2} g_6 p_2 q_2 q_3 - a_{1,2} g_6 p_3 q_2^2 - 2 a_{1,3} f_2 p_2 q_2 q_3
\end{aligned}$$

$$\begin{aligned}
& -a_{1,3}f_2p_3q_2^2 - 3a_{1,3}f_5q_2^2q_3 + a_{1,3}g_2p_2^2q_3 + 2a_{1,3}g_2p_2p_3q_2 + 2a_{1,3}g_5p_2q_2q_3 \\
& + a_{1,3}g_5p_3q_2^2 + 2a_{2,3}f_1p_2q_2q_3 + a_{2,3}f_1p_3q_2^2 + 3a_{2,3}f_4q_2^2q_3 - a_{2,3}g_1p_2^2q_3 \\
& - 2a_{2,3}g_1p_2p_3q_2 - 2a_{2,3}g_4p_2q_2q_3 - a_{2,3}g_4p_3q_2^2 - b_{1,2}f_3p_2^2q_3 \\
& - 2b_{1,2}f_3p_2p_3q_2 - 2b_{1,2}f_6p_2q_2q_3 - b_{1,2}f_6p_3q_2^2 + 3b_{1,2}g_3p_2^2p_3 + b_{1,2}g_6p_2^2q_3 \\
& + 2b_{1,2}g_6p_2p_3q_2 + b_{1,3}f_2p_2^2q_3 + 2b_{1,3}f_2p_2p_3q_2 + 2b_{1,3}f_5p_2q_2q_3 + b_{1,3}f_5p_3 \\
& q_2^2 - 3b_{1,3}g_2p_2^2p_3 - b_{1,3}g_5p_2^2q_3 - 2b_{1,3}g_5p_2p_3q_2 - b_{2,3}f_1p_2^2q_3 \\
& - 2b_{2,3}f_1p_2p_3q_2 - 2b_{2,3}f_4p_2q_2q_3 - b_{2,3}f_4p_3q_2^2 + 3b_{2,3}g_1p_2^2p_3 + b_{2,3}g_4p_2^2q_3 \\
& + 2b_{2,3}g_4p_2p_3q_2
\end{aligned}$$

$$\triangleright I4 := \text{factor}\left(\frac{1}{6} \text{numer}(\text{diff}(Q3, y, y, y))\right)$$

$$I4 := -f_1f_5p_2q_2^2q_3 + f_1f_5p_3q_2^3 + f_1g_5p_2^2q_2q_3 - f_1g_5p_2p_3q_2^2 + f_2f_4p_2q_2^2q_3 - f_2f_4p_3q_2^3 \quad (33)$$

$$\begin{aligned}
& + f_2f_6p_1q_2^3 - f_2f_6p_2q_1q_2^2 - f_2g_4p_2^2q_2q_3 + f_2g_4p_2p_3q_2^2 - f_2g_6p_1p_2q_2^2 + f_2g_6 \\
& p_2^2q_1q_2 - f_3f_5p_1q_2^3 + f_3f_5p_2q_1q_2^2 + f_3g_5p_1p_2q_2^2 - f_3g_5p_2^2q_1q_2 - f_4g_2p_2^2q_2q_3 \\
& + f_4g_2p_2p_3q_2^2 + f_5g_1p_2^2q_2q_3 - f_5g_1p_2p_3q_2^2 + f_5g_3p_1p_2q_2^2 - f_5g_3p_2^2q_1q_2 \\
& - f_6g_2p_1p_2q_2^2 + f_6g_2p_2^2q_1q_2 - g_1g_5p_2^3q_3 + g_1g_5p_2^2p_3q_2 + g_2g_4p_2^3q_3 - g_2g_4 \\
& p_2^2p_3q_2 + g_2g_6p_1p_2^2q_2 - g_2g_6p_2^3q_1 - g_3g_5p_1p_2^2q_2 + g_3g_5p_2^3q_1 - a_{1,2}f_3p_2q_2^2 \\
& - a_{1,2}f_6q_2^3 + a_{1,2}g_3p_2^2q_2 + a_{1,2}g_6p_2q_2^2 + a_{1,3}f_2p_2q_2^2 + a_{1,3}f_5q_2^3 - a_{1,3}g_2p_2^2q_2 \\
& - a_{1,3}g_5p_2q_2^2 - a_{2,3}f_1p_2q_2^2 - a_{2,3}f_4q_2^3 + a_{2,3}g_1p_2^2q_2 + a_{2,3}g_4p_2q_2^2 + b_{1,2}f_3 \\
& p_2^2q_2 + b_{1,2}f_6p_2q_2^2 - b_{1,2}g_3p_2^3 - b_{1,2}g_6p_2^2q_2 - b_{1,3}f_2p_2^2q_2 - b_{1,3}f_5p_2q_2^2 \\
& + b_{1,3}g_2p_2^3 + b_{1,3}g_5p_2^2q_2 + b_{2,3}f_1p_2^2q_2 + b_{2,3}f_4p_2q_2^2 - b_{2,3}g_1p_2^3 - b_{2,3}g_4p_2^2q_2
\end{aligned}$$

$$\triangleright \# \text{solve}(\{op(SEQ), I1, I2, I3, I4\}, \{seq(seq(f_{i,j}, j = i..6), i = 1..6), seq(seq(g_{i,j}, j = i..6), i = 1..6)\})$$

Let us compute the MA conditions together with 4 new constraints at a nondegenerate 1-jet (these will be then linear conditions on 2-jets of f,g resp. on 2-jets of a,b (plus 1-jets of p,q) - the parameters; note that in I1,I2,I3,I4 we get a,b,p,q instead of 2-jets of f,g).

$$\triangleright pt := \{f[1] = 0, f[2] = 1, f[3] = 0, f[4] = 1, f[5] = 0, f[6] = 0, g[1] = 0, g[2] = 0, g[3] = 1, g[4] = 0, g[5] = 0, g[6] = 0\} :$$

$$\triangleright \text{subs}(pt, \{op(MAE)\})$$

$$\begin{aligned}
& \{f_{1,1} = 0, f_{1,2} = 0, f_{1,3} = -p_1, f_{1,4} = 0, f_{1,5} = a_{1,2}, f_{1,6} = a_{1,3}, f_{2,2} = 0, f_{2,3} = -p_2, f_{2,4} = \\
& -a_{1,2} + p_1, f_{2,5} = p_2, f_{2,6} = a_{2,3} + p_3, f_{3,3} = -2p_3, f_{3,4} = -a_{1,3}, f_{3,5} = -a_{2,3}, f_{3,6} = 0, \\
& f_{4,4} = 2p_1, f_{4,5} = p_2, f_{4,6} = p_3, f_{5,5} = 0, f_{5,6} = 0, f_{6,6} = 0, g_{1,1} = 0, g_{1,2} = 0, g_{1,3} = -q_1,
\end{aligned} \quad (34)$$

$$\begin{aligned} g_{1,4} &= 0, g_{1,5} = b_{1,2}, g_{1,6} = b_{1,3}, g_{2,2} = 0, g_{2,3} = -q_2, g_{2,4} = -b_{1,2} + q_1, g_{2,5} = q_2, g_{2,6} \\ &= b_{2,3} + q_3, g_{3,3} = -2q_3, g_{3,4} = -b_{1,3}, g_{3,5} = -b_{2,3}, g_{3,6} = 0, g_{4,4} = 2q_1, g_{4,5} = q_2, \\ g_{4,6} &= q_3, g_{5,5} = 0, g_{5,6} = 0, g_{6,6} = 0 \end{aligned}$$

$$\begin{aligned} &> \text{spt} := \text{solve}(\text{subs}(pt, \{I1, I2, I3, I4, p_2 q_3 \neq p_3 q_2\})); \\ &\quad \# \text{seq}(\text{nops}(\text{spt}[i]), i = 1 \dots \text{nops}(\{\text{spt}\})) \\ \text{spt} &:= \{a_{1,2} = b_{1,3} - q_2, a_{1,3} = -b_{2,3} + p_2 - q_3, a_{2,3} = -p_3, b_{1,2} = 0, b_{1,3} = b_{1,3}, b_{2,3} \\ &= b_{2,3}, p_2 = p_2, p_3 = p_3, q_2 = q_2, q_3 = q_3\} \end{aligned} \quad (35)$$

$$\begin{aligned} &> \text{simplify}(\text{subs}(\text{spt}, \text{subs}(pt, \{I1, I2, I3, I4\}))) \\ &\quad \{0\} \end{aligned} \quad (36)$$

$$\begin{aligned} &> SL := \text{solve}(\text{subs}(pt, \{I1, I2, I3, I4, p_2 q_3 \neq p_3 q_2\}), \{a_{1,2}, a_{1,3}, a_{2,3}, b_{1,2}\}) \\ SL &:= \{a_{1,2} = b_{1,3} - q_2, a_{1,3} = -b_{2,3} + p_2 - q_3, a_{2,3} = -p_3, b_{1,2} = 0\} \end{aligned} \quad (37)$$

$$\begin{aligned} &> \# \text{solve}(\{I1, I2, I3, I4, p_2 q_3 \neq p_3 q_2\}, \{a_{1,2}, a_{1,3}, a_{2,3}, b_{1,2}, b_{1,3}, b_{2,3}, p_1, p_2, p_3, q_1, q_2, q_3\}) \\ &> \text{factor}(\text{diff}(I1, a_{1,2})), \text{factor}(\text{diff}(I2, a_{1,2})), \text{factor}(\text{diff}(I3, a_{1,2})), \text{factor}(\text{diff}(I4, a_{1,2})) \\ q_3 & (f_3 p_3 q_3 + f_6 q_3^2 - g_3 p_3^2 - g_6 p_3 q_3), -f_3 p_2 q_3^2 - 2f_3 p_3 q_2 q_3 - 3f_6 q_2 q_3^2 + 2g_3 p_2 p_3 q_3 \\ &+ g_3 p_3^2 q_2 + g_6 p_2 q_3^2 + 2g_6 p_3 q_2 q_3, 2f_3 p_2 q_2 q_3 + f_3 p_3 q_2^2 + 3f_6 q_2^2 q_3 - g_3 p_2^2 q_3 \\ &- 2g_3 p_2 p_3 q_2 - 2g_6 p_2 q_2 q_3 - g_6 p_3 q_2^2, -q_2 (f_3 p_2 q_2 + f_6 q_2^2 - g_3 p_2^2 - g_6 p_2 q_2) \end{aligned} \quad (38)$$

$$\begin{aligned} &> \text{with}(\text{PolynomialIdeals}) : \\ &> ID := \langle \text{op}(\text{subs}(pt, \{I1, I2, I3, I4\})) \rangle : \\ &> \text{nops}(\text{IdeallInfo:-Variables}(ID)), \text{nops}(\text{MaximalIndependentSet}(ID)), \text{nops}(\text{IdeallInfo:-} \\ &\quad \text{Variables}(ID)) - \text{HilbertDimension}(ID) \\ &\quad 10, 8, 2 \end{aligned} \quad (39)$$

$$> \# PS3 := \text{PrimeDecomposition}(ID)$$

trial for linearizable (but nonlinear) eqn

$$\begin{aligned} &> Ff := u2 v3 - u3 v2 : Gg := u1 v2 - u2 v1 : \\ &> tmp := \{ \} : \text{for } i \text{ to } 6 \text{ do } tmp := tmp \text{ union } \{f_i = \text{diff}(Ff, \text{var}[i]), g_i = \text{diff}(Gg, \text{var}[i])\} : \text{for } j \\ &\quad \text{from } i \text{ to } 6 \text{ do } tmp := tmp \text{ union } \{f_{i,j} = \text{diff}(Ff, \text{var}[i], \text{var}[j]), g_{i,j} = \text{diff}(Gg, \text{var}[i], \\ &\quad \text{var}[j])\} : \text{od} : \text{od} : \\ &> tmp2 := \text{solve}(\text{simplify}(\text{subs}(tmp, MAE)), \{a_{1,2}, a_{1,3}, a_{2,3}, b_{1,2}, b_{1,3}, b_{2,3}, p_1, p_2, p_3, q_1, q_2, \\ &\quad q_3\}) \\ tmp2 &:= \{a_{1,2} = 0, a_{1,3} = 0, a_{2,3} = 1, b_{1,2} = 1, b_{1,3} = 0, b_{2,3} = 0, p_1 = 0, p_2 = 0, p_3 = 0, q_1 \\ &= 0, q_2 = 0, q_3 = 0\} \end{aligned} \quad (40)$$

$$\begin{aligned} &> \text{subs}(tmp2, \text{subs}(tmp, \{I1, I2, I3, I4\})) \\ &\quad \{0\} \end{aligned} \quad (41)$$

>

Check if the four equations above coincide with the four equations from prolongation-projection

>  $FOUREQNS := \{f_{1,5} = g_{1,6} - g_{4,5}, f_{3,5} = f_{4,6} + g_{3,6} - g_{5,6}, f_{4,5} = f_{1,6} - g_{3,5} + g_{4,6}, g_{1,5} = 0\} :$

$solve(subs(pt, subs(MAE, FOUREQNS)), \{a_{1,2}, a_{1,3}, a_{2,3}, b_{1,2}\}); SL$

$\{a_{1,2} = b_{1,3} - q_2, a_{1,3} = -b_{2,3} + p_2 - q_3, a_{2,3} = -p_3, b_{1,2} = 0\}$

$\{a_{1,2} = b_{1,3} - q_2, a_{1,3} = -b_{2,3} + p_2 - q_3, a_{2,3} = -p_3, b_{1,2} = 0\} \tag{42}$

YES!

$YES! \tag{43}$
