# Supplementary material for: Integrable systems in 4D associated with sixfolds in Gr(4,6)
Source: arXiv:1705.06999 ancillary file (2017-05-18)
Supplement: Supplementary file 6 [file DFKN-2017-SL6-action.pdf]

This notebook accompanies the paper B.Doubrov, E.Ferapontov, B.Kruglikov, V.Novikov "Integrable systems in 4D associated with sixfolds in  $\text{Gr}(4,6)$ ".

We compute the action of  $\text{SL}_6$  on the system equations on linear degeneracy and show it acts transitively: from one equation we derive all 20 equations of the system.

(\* List of generators of  $\text{SL}_6$ \*)

(\* X11 \*)

X11 := Block[{}],  $\xi_1 = x_1$ ;

$\xi_2 = 0$ ;

$\xi_3 = 0$ ;

$\xi_4 = x_4$ ;

$\xi_5 = 0$ ;

$\xi_6 = 0$ ;

$\eta_1 = 0$ ;

$\eta_2 = 0$ ;

(\* X12 \*)

X12 := Block[{}],  $\xi_1 = 0$ ;

$\xi_2 = x_1$ ;

$\xi_3 = 0$ ;

$\xi_4 = 0$ ;

$\xi_5 = x_4$ ;

$\xi_6 = 0$ ;

$\eta_1 = 0$ ;

$\eta_2 = 0$ ;

(\* X13 \*)

X13 := Block[{}],  $\xi_1 = 0$ ;

$\xi_2 = 0$ ;

$\xi_3 = x_1$ ;

$\xi_4 = 0$ ;

$\xi_5 = 0$ ;

$\xi_6 = x_4$ ;

$\eta_1 = 0$ ;

$\eta_2 = 0$ ;

(\* X14 \*)

X14 := Block[{}],  $\xi_1 = 0$ ;

$\xi_2 = 0$ ;

$\xi_3 = 0$ ;

$\xi_4 = 0$ ;

$\xi_5 = 0$ ;

$\xi_6 = 0$ ;

$\eta_1 = x_1$ ;

$\eta_2 = x_4$ ;

```
(* X21 *)
X21 := Block[{},  $\xi_1 = x_2$ ;
   $\xi_2 = 0$ ;
   $\xi_3 = 0$ ;
   $\xi_4 = x_5$ ;
   $\xi_5 = 0$ ;
   $\xi_6 = 0$ ;
   $\eta_1 = 0$ ;
   $\eta_2 = 0$ ;]
```

```
(* X22 *)
X22 := Block[{},  $\xi_1 = 0$ ;
   $\xi_2 = x_2$ ;
   $\xi_3 = 0$ ;
   $\xi_4 = 0$ ;
   $\xi_5 = x_5$ ;
   $\xi_6 = 0$ ;
   $\eta_1 = 0$ ;
   $\eta_2 = 0$ ;]
```

```
(* X23 *)
X23 := Block[{},  $\xi_1 = 0$ ;
   $\xi_2 = 0$ ;
   $\xi_3 = x_2$ ;
   $\xi_4 = 0$ ;
   $\xi_5 = 0$ ;
   $\xi_6 = x_5$ ;
   $\eta_1 = 0$ ;
   $\eta_2 = 0$ ;]
```

```
(* X24 *)
X24 := Block[{},  $\xi_1 = 0$ ;
   $\xi_2 = 0$ ;
   $\xi_3 = 0$ ;
   $\xi_4 = 0$ ;
   $\xi_5 = 0$ ;
   $\xi_6 = 0$ ;
   $\eta_1 = x_2$ ;
   $\eta_2 = x_5$ ;]
```

```
(* X31 *)
X31 := Block[{},  $\xi_1 = x_3$ ;
   $\xi_2 = 0$ ;
   $\xi_3 = 0$ ;
   $\xi_4 = x_6$ ;
   $\xi_5 = 0$ ;
   $\xi_6 = 0$ ;
   $\eta_1 = 0$ ;
   $\eta_2 = 0$ ;]
```

```
(* X32 *)
X32 := Block[{},  $\xi_1 = 0$ ;
   $\xi_2 = x_3$ ;
   $\xi_3 = 0$ ;
   $\xi_4 = 0$ ;
   $\xi_5 = x_6$ ;
   $\xi_6 = 0$ ;
   $\eta_1 = 0$ ;
   $\eta_2 = 0$ ;]
```

```
(* X33 *)
X33 := Block[{},  $\xi_1 = 0$ ;
   $\xi_2 = 0$ ;
   $\xi_3 = x_3$ ;
   $\xi_4 = 0$ ;
   $\xi_5 = 0$ ;
   $\xi_6 = x_6$ ;
   $\eta_1 = 0$ ;
   $\eta_2 = 0$ ;]
```

```
(* X34 *)
X34 := Block[{},  $\xi_1 = 0$ ;
   $\xi_2 = 0$ ;
   $\xi_3 = 0$ ;
   $\xi_4 = 0$ ;
   $\xi_5 = 0$ ;
   $\xi_6 = 0$ ;
   $\eta_1 = x_3$ ;
   $\eta_2 = x_6$ ;]
```

```
(* X41 *)
X41 := Block[{},  $\xi_1 = f$ ;
   $\xi_2 = 0$ ;
   $\xi_3 = 0$ ;
   $\xi_4 = g$ ;
   $\xi_5 = 0$ ;
   $\xi_6 = 0$ ;
   $\eta_1 = 0$ ;
   $\eta_2 = 0$ ;
```

```
(* X42 *)
X42 := Block[{},  $\xi_1 = 0$ ;
   $\xi_2 = f$ ;
   $\xi_3 = 0$ ;
   $\xi_4 = 0$ ;
   $\xi_5 = g$ ;
   $\xi_6 = 0$ ;
   $\eta_1 = 0$ ;
   $\eta_2 = 0$ ;
```

```
(* X43 *)
X43 := Block[{},  $\xi_1 = 0$ ;
   $\xi_2 = 0$ ;
   $\xi_3 = f$ ;
   $\xi_4 = 0$ ;
   $\xi_5 = 0$ ;
   $\xi_6 = g$ ;
   $\eta_1 = 0$ ;
   $\eta_2 = 0$ ;
```

```
(* X44 *)
X44 := Block[{},  $\xi_1 = 0$ ;
   $\xi_2 = 0$ ;
   $\xi_3 = 0$ ;
   $\xi_4 = 0$ ;
   $\xi_5 = 0$ ;
   $\xi_6 = 0$ ;
   $\eta_1 = f$ ;
   $\eta_2 = g$ ;
```

```
(* L11 *)
L11 := Block[{},  $\xi_1 = x_1$ ;
 $\xi_2 = x_2$ ;
 $\xi_3 = x_3$ ;
 $\xi_4 = 0$ ;
 $\xi_5 = 0$ ;
 $\xi_6 = 0$ ;
 $\eta_1 = f$ ;
 $\eta_2 = 0$ ;
```

```
(* L12 *)
L12 := Block[{},  $\xi_1 = 0$ ;
 $\xi_2 = 0$ ;
 $\xi_3 = 0$ ;
 $\xi_4 = x_1$ ;
 $\xi_5 = x_2$ ;
 $\xi_6 = x_3$ ;
 $\eta_1 = 0$ ;
 $\eta_2 = f$ ;
```

```
(* L21 *)
L21 := Block[{},  $\xi_1 = x_4$ ;
 $\xi_2 = x_5$ ;
 $\xi_3 = x_6$ ;
 $\xi_4 = 0$ ;
 $\xi_5 = 0$ ;
 $\xi_6 = 0$ ;
 $\eta_1 = g$ ;
 $\eta_2 = 0$ ;
```

```
(* L22 *)
L22 := Block[{},  $\xi_1 = 0$ ;
 $\xi_2 = 0$ ;
 $\xi_3 = 0$ ;
 $\xi_4 = x_4$ ;
 $\xi_5 = x_5$ ;
 $\xi_6 = x_6$ ;
 $\eta_1 = 0$ ;
 $\eta_2 = g$ ;
```

(\* P1 \*)

```
P1 := Block[{ },  $\xi_1 = x_1 x_1$ ;
 $\xi_2 = x_1 x_2$ ;
 $\xi_3 = x_1 x_3$ ;
 $\xi_4 = x_4 x_1$ ;
 $\xi_5 = x_4 x_2$ ;
 $\xi_6 = x_4 x_3$ ;
 $\eta_1 = x_1 f$ ;
 $\eta_2 = x_4 f$ ;
```

(\* P2 \*)

```
P2 := Block[{ },  $\xi_1 = x_2 x_1$ ;
 $\xi_2 = x_2 x_2$ ;
 $\xi_3 = x_2 x_3$ ;
 $\xi_4 = x_5 x_1$ ;
 $\xi_5 = x_5 x_2$ ;
 $\xi_6 = x_5 x_3$ ;
 $\eta_1 = x_2 f$ ;
 $\eta_2 = x_5 f$ ;
```

(\* P3 \*)

```
P3 := Block[{ },  $\xi_1 = x_3 x_1$ ;
 $\xi_2 = x_3 x_2$ ;
 $\xi_3 = x_3 x_3$ ;
 $\xi_4 = x_6 x_1$ ;
 $\xi_5 = x_6 x_2$ ;
 $\xi_6 = x_6 x_3$ ;
 $\eta_1 = x_3 f$ ;
 $\eta_2 = x_6 f$ ;
```

(\* P4 \*)

```
P4 := Block[{ },  $\xi_1 = f x_1$ ;
 $\xi_2 = f x_2$ ;
 $\xi_3 = f x_3$ ;
 $\xi_4 = g x_1$ ;
 $\xi_5 = g x_2$ ;
 $\xi_6 = g x_3$ ;
 $\eta_1 = f f$ ;
 $\eta_2 = g f$ ;
```

(\* Q1 \*)

```
Q1 := Block[{},  $\xi_1 = x_1 x_4$ ;
 $\xi_2 = x_1 x_5$ ;
 $\xi_3 = x_1 x_6$ ;
 $\xi_4 = x_4 x_4$ ;
 $\xi_5 = x_4 x_5$ ;
 $\xi_6 = x_4 x_6$ ;
 $\eta_1 = x_1 g$ ;
 $\eta_2 = x_4 g$ ;
```

(\* Q2 \*)

```
Q2 := Block[{},  $\xi_1 = x_2 x_4$ ;
 $\xi_2 = x_2 x_5$ ;
 $\xi_3 = x_2 x_6$ ;
 $\xi_4 = x_5 x_4$ ;
 $\xi_5 = x_5 x_5$ ;
 $\xi_6 = x_5 x_6$ ;
 $\eta_1 = x_2 g$ ;
 $\eta_2 = x_5 g$ ;
```

(\* Q3 \*)

```
Q3 := Block[{},  $\xi_1 = x_3 x_4$ ;
 $\xi_2 = x_3 x_5$ ;
 $\xi_3 = x_3 x_6$ ;
 $\xi_4 = x_6 x_4$ ;
 $\xi_5 = x_6 x_5$ ;
 $\xi_6 = x_6 x_6$ ;
 $\eta_1 = x_3 g$ ;
 $\eta_2 = x_6 g$ ;
```

(\* Q4 \*)

```
Q4 := Block[{},  $\xi_1 = f x_4$ ;
 $\xi_2 = f x_5$ ;
 $\xi_3 = f x_6$ ;
 $\xi_4 = g x_4$ ;
 $\xi_5 = g x_5$ ;
 $\xi_6 = g x_6$ ;
 $\eta_1 = f g$ ;
 $\eta_2 = g g$ ;
```

```

D1[exp_] := D[exp, x1] + D[exp, f] f1 + D[exp, g] g1 + D[exp, f1] f11 + D[exp, f2] f12 +
  D[exp, f3] f13 + D[exp, f4] f14 + D[exp, f5] f15 + D[exp, f6] f16 + D[exp, g1] g11 +
  D[exp, g2] g12 + D[exp, g3] g13 + D[exp, g4] g14 + D[exp, g5] g15 + D[exp, g6] g16;
D2[exp_] := D[exp, x2] + D[exp, f] f2 + D[exp, g] g2 + D[exp, f1] f12 + D[exp, f2] f22 +
  D[exp, f3] f23 + D[exp, f4] f24 + D[exp, f5] f25 + D[exp, f6] f26 + D[exp, g1] g12 +
  D[exp, g2] g22 + D[exp, g3] g23 + D[exp, g4] g24 + D[exp, g5] g25 + D[exp, g6] g26;
D3[exp_] := D[exp, x3] + D[exp, f] f3 + D[exp, g] g3 + D[exp, f1] f13 + D[exp, f2] f23 +
  D[exp, f3] f33 + D[exp, f4] f34 + D[exp, f5] f35 + D[exp, f6] f36 + D[exp, g1] g13 +
  D[exp, g2] g23 + D[exp, g3] g33 + D[exp, g4] g34 + D[exp, g5] g35 + D[exp, g6] g36;
D4[exp_] := D[exp, x4] + D[exp, f] f4 + D[exp, g] g4 + D[exp, f1] f14 + D[exp, f2] f24 +
  D[exp, f3] f34 + D[exp, f4] f44 + D[exp, f5] f45 + D[exp, f6] f46 + D[exp, g1] g14 +
  D[exp, g2] g24 + D[exp, g3] g34 + D[exp, g4] g44 + D[exp, g5] g45 + D[exp, g6] g46;
D5[exp_] := D[exp, x5] + D[exp, f] f5 + D[exp, g] g5 + D[exp, f1] f15 + D[exp, f2] f25 +
  D[exp, f3] f35 + D[exp, f4] f45 + D[exp, f5] f55 + D[exp, f6] f56 + D[exp, g1] g15 +
  D[exp, g2] g25 + D[exp, g3] g35 + D[exp, g4] g45 + D[exp, g5] g55 + D[exp, g6] g56;
D6[exp_] := D[exp, x6] + D[exp, f] f6 + D[exp, g] g6 + D[exp, f1] f16 + D[exp, f2] f26 +
  D[exp, f3] f36 + D[exp, f4] f46 + D[exp, f5] f56 + D[exp, f6] f66 + D[exp, g1] g16 +
  D[exp, g2] g26 + D[exp, g3] g36 + D[exp, g4] g46 + D[exp, g5] g56 + D[exp, g6] g66;

```

```
ExtDef[var_] := Block[{ }, var;
```

```

ξ11 = D1[η1] - f1 D1[ξ1] - f2 D1[ξ2] - f3 D1[ξ3] - f4 D1[ξ4] - f5 D1[ξ5] - f6 D1[ξ6];
ξ12 = D2[η1] - f1 D2[ξ1] - f2 D2[ξ2] - f3 D2[ξ3] - f4 D2[ξ4] - f5 D2[ξ5] - f6 D2[ξ6];
ξ13 = D3[η1] - f1 D3[ξ1] - f2 D3[ξ2] - f3 D3[ξ3] - f4 D3[ξ4] - f5 D3[ξ5] - f6 D3[ξ6];
ξ14 = D4[η1] - f1 D4[ξ1] - f2 D4[ξ2] - f3 D4[ξ3] - f4 D4[ξ4] - f5 D4[ξ5] - f6 D4[ξ6];
ξ15 = D5[η1] - f1 D5[ξ1] - f2 D5[ξ2] - f3 D5[ξ3] - f4 D5[ξ4] - f5 D5[ξ5] - f6 D5[ξ6];
ξ16 = D6[η1] - f1 D6[ξ1] - f2 D6[ξ2] - f3 D6[ξ3] - f4 D6[ξ4] - f5 D6[ξ5] - f6 D6[ξ6];

```

```

ξ21 = D1[η2] - g1 D1[ξ1] - g2 D1[ξ2] - g3 D1[ξ3] - g4 D1[ξ4] - g5 D1[ξ5] - g6 D1[ξ6];
ξ22 = D2[η2] - g1 D2[ξ1] - g2 D2[ξ2] - g3 D2[ξ3] - g4 D2[ξ4] - g5 D2[ξ5] - g6 D2[ξ6];
ξ23 = D3[η2] - g1 D3[ξ1] - g2 D3[ξ2] - g3 D3[ξ3] - g4 D3[ξ4] - g5 D3[ξ5] - g6 D3[ξ6];
ξ24 = D4[η2] - g1 D4[ξ1] - g2 D4[ξ2] - g3 D4[ξ3] - g4 D4[ξ4] - g5 D4[ξ5] - g6 D4[ξ6];
ξ25 = D5[η2] - g1 D5[ξ1] - g2 D5[ξ2] - g3 D5[ξ3] - g4 D5[ξ4] - g5 D5[ξ5] - g6 D5[ξ6];
ξ26 = D6[η2] - g1 D6[ξ1] - g2 D6[ξ2] - g3 D6[ξ3] - g4 D6[ξ4] - g5 D6[ξ5] - g6 D6[ξ6];

```

```

ξ111 = D1[ξ11] - f11 D1[ξ1] - f12 D1[ξ2] - f13 D1[ξ3] - f14 D1[ξ4] - f15 D1[ξ5] - f16 D1[ξ6];
ξ112 = D1[ξ12] - f12 D1[ξ1] - f22 D1[ξ2] - f23 D1[ξ3] - f24 D1[ξ4] - f25 D1[ξ5] - f26 D1[ξ6];
ξ113 = D1[ξ13] - f13 D1[ξ1] - f23 D1[ξ2] - f33 D1[ξ3] - f34 D1[ξ4] - f35 D1[ξ5] - f36 D1[ξ6];
ξ114 = D1[ξ14] - f14 D1[ξ1] - f24 D1[ξ2] - f34 D1[ξ3] - f44 D1[ξ4] - f45 D1[ξ5] - f46 D1[ξ6];
ξ115 = D1[ξ15] - f15 D1[ξ1] - f25 D1[ξ2] - f35 D1[ξ3] - f45 D1[ξ4] - f55 D1[ξ5] - f56 D1[ξ6];
ξ116 = D1[ξ16] - f16 D1[ξ1] - f26 D1[ξ2] - f36 D1[ξ3] - f46 D1[ξ4] - f56 D1[ξ5] - f66 D1[ξ6];

```

```

ξ122 = D2[ξ12] - f12 D2[ξ1] - f22 D2[ξ2] - f23 D2[ξ3] - f24 D2[ξ4] - f25 D2[ξ5] - f26 D2[ξ6];
ξ123 = D2[ξ13] - f13 D2[ξ1] - f23 D2[ξ2] - f33 D2[ξ3] - f34 D2[ξ4] - f35 D2[ξ5] - f36 D2[ξ6];
ξ124 = D2[ξ14] - f14 D2[ξ1] - f24 D2[ξ2] - f34 D2[ξ3] - f44 D2[ξ4] - f45 D2[ξ5] - f46 D2[ξ6];

```



$$\begin{aligned}\xi_{125} &= D2[\xi_{15}] - f_{15} D2[\xi_1] - f_{25} D2[\xi_2] - f_{35} D2[\xi_3] - f_{45} D2[\xi_4] - f_{55} D2[\xi_5] - f_{56} D2[\xi_6]; \\ \xi_{126} &= D2[\xi_{16}] - f_{16} D2[\xi_1] - f_{26} D2[\xi_2] - f_{36} D2[\xi_3] - f_{46} D2[\xi_4] - f_{56} D2[\xi_5] - f_{66} D2[\xi_6];\end{aligned}$$

$$\begin{aligned}\xi_{133} &= D3[\xi_{13}] - f_{13} D3[\xi_1] - f_{23} D3[\xi_2] - f_{33} D3[\xi_3] - f_{34} D3[\xi_4] - f_{35} D3[\xi_5] - f_{36} D3[\xi_6]; \\ \xi_{134} &= D3[\xi_{14}] - f_{14} D3[\xi_1] - f_{24} D3[\xi_2] - f_{34} D3[\xi_3] - f_{44} D3[\xi_4] - f_{45} D3[\xi_5] - f_{46} D3[\xi_6]; \\ \xi_{135} &= D3[\xi_{15}] - f_{15} D3[\xi_1] - f_{25} D3[\xi_2] - f_{35} D3[\xi_3] - f_{45} D3[\xi_4] - f_{55} D3[\xi_5] - f_{56} D3[\xi_6]; \\ \xi_{136} &= D3[\xi_{16}] - f_{16} D3[\xi_1] - f_{26} D3[\xi_2] - f_{36} D3[\xi_3] - f_{46} D3[\xi_4] - f_{56} D3[\xi_5] - f_{66} D3[\xi_6];\end{aligned}$$

$$\begin{aligned}\xi_{144} &= D4[\xi_{14}] - f_{14} D4[\xi_1] - f_{24} D4[\xi_2] - f_{34} D4[\xi_3] - f_{44} D4[\xi_4] - f_{45} D4[\xi_5] - f_{46} D4[\xi_6]; \\ \xi_{145} &= D4[\xi_{15}] - f_{15} D4[\xi_1] - f_{25} D4[\xi_2] - f_{35} D4[\xi_3] - f_{45} D4[\xi_4] - f_{55} D4[\xi_5] - f_{56} D4[\xi_6]; \\ \xi_{146} &= D4[\xi_{16}] - f_{16} D4[\xi_1] - f_{26} D4[\xi_2] - f_{36} D4[\xi_3] - f_{46} D4[\xi_4] - f_{56} D4[\xi_5] - f_{66} D4[\xi_6];\end{aligned}$$

$$\begin{aligned}\xi_{155} &= D5[\xi_{15}] - f_{15} D5[\xi_1] - f_{25} D5[\xi_2] - f_{35} D5[\xi_3] - f_{45} D5[\xi_4] - f_{55} D5[\xi_5] - f_{56} D5[\xi_6]; \\ \xi_{156} &= D5[\xi_{16}] - f_{16} D5[\xi_1] - f_{26} D5[\xi_2] - f_{36} D5[\xi_3] - f_{46} D5[\xi_4] - f_{56} D5[\xi_5] - f_{66} D5[\xi_6];\end{aligned}$$

$$\xi_{166} = D6[\xi_{16}] - f_{16} D6[\xi_1] - f_{26} D6[\xi_2] - f_{36} D6[\xi_3] - f_{46} D6[\xi_4] - f_{56} D6[\xi_5] - f_{66} D6[\xi_6];$$

$$\begin{aligned}\xi_{211} &= D1[\xi_{21}] - g_{11} D1[\xi_1] - g_{12} D1[\xi_2] - g_{13} D1[\xi_3] - g_{14} D1[\xi_4] - g_{15} D1[\xi_5] - g_{16} D1[\xi_6]; \\ \xi_{212} &= D1[\xi_{22}] - g_{12} D1[\xi_1] - g_{22} D1[\xi_2] - g_{23} D1[\xi_3] - g_{24} D1[\xi_4] - g_{25} D1[\xi_5] - g_{26} D1[\xi_6]; \\ \xi_{213} &= D1[\xi_{23}] - g_{13} D1[\xi_1] - g_{23} D1[\xi_2] - g_{33} D1[\xi_3] - g_{34} D1[\xi_4] - g_{35} D1[\xi_5] - g_{36} D1[\xi_6]; \\ \xi_{214} &= D1[\xi_{24}] - g_{14} D1[\xi_1] - g_{24} D1[\xi_2] - g_{34} D1[\xi_3] - g_{44} D1[\xi_4] - g_{45} D1[\xi_5] - g_{46} D1[\xi_6]; \\ \xi_{215} &= D1[\xi_{25}] - g_{15} D1[\xi_1] - g_{25} D1[\xi_2] - g_{35} D1[\xi_3] - g_{45} D1[\xi_4] - g_{55} D1[\xi_5] - g_{56} D1[\xi_6]; \\ \xi_{216} &= D1[\xi_{26}] - g_{16} D1[\xi_1] - g_{26} D1[\xi_2] - g_{36} D1[\xi_3] - g_{46} D1[\xi_4] - g_{56} D1[\xi_5] - g_{66} D1[\xi_6];\end{aligned}$$

$$\begin{aligned}\xi_{222} &= D2[\xi_{22}] - g_{12} D2[\xi_1] - g_{22} D2[\xi_2] - g_{23} D2[\xi_3] - g_{24} D2[\xi_4] - g_{25} D2[\xi_5] - g_{26} D2[\xi_6]; \\ \xi_{223} &= D2[\xi_{23}] - g_{13} D2[\xi_1] - g_{23} D2[\xi_2] - g_{33} D2[\xi_3] - g_{34} D2[\xi_4] - g_{35} D2[\xi_5] - g_{36} D2[\xi_6]; \\ \xi_{224} &= D2[\xi_{24}] - g_{14} D2[\xi_1] - g_{24} D2[\xi_2] - g_{34} D2[\xi_3] - g_{44} D2[\xi_4] - g_{45} D2[\xi_5] - g_{46} D2[\xi_6]; \\ \xi_{225} &= D2[\xi_{25}] - g_{15} D2[\xi_1] - g_{25} D2[\xi_2] - g_{35} D2[\xi_3] - g_{45} D2[\xi_4] - g_{55} D2[\xi_5] - g_{56} D2[\xi_6]; \\ \xi_{226} &= D2[\xi_{26}] - g_{16} D2[\xi_1] - g_{26} D2[\xi_2] - g_{36} D2[\xi_3] - g_{46} D2[\xi_4] - g_{56} D2[\xi_5] - g_{66} D2[\xi_6];\end{aligned}$$

$$\begin{aligned}\xi_{233} &= D3[\xi_{23}] - g_{13} D3[\xi_1] - g_{23} D3[\xi_2] - g_{33} D3[\xi_3] - g_{34} D3[\xi_4] - g_{35} D3[\xi_5] - g_{36} D3[\xi_6]; \\ \xi_{234} &= D3[\xi_{24}] - g_{14} D3[\xi_1] - g_{24} D3[\xi_2] - g_{34} D3[\xi_3] - g_{44} D3[\xi_4] - g_{45} D3[\xi_5] - g_{46} D3[\xi_6]; \\ \xi_{235} &= D3[\xi_{25}] - g_{15} D3[\xi_1] - g_{25} D3[\xi_2] - g_{35} D3[\xi_3] - g_{45} D3[\xi_4] - g_{55} D3[\xi_5] - g_{56} D3[\xi_6]; \\ \xi_{236} &= D3[\xi_{26}] - g_{16} D3[\xi_1] - g_{26} D3[\xi_2] - g_{36} D3[\xi_3] - g_{46} D3[\xi_4] - g_{56} D3[\xi_5] - g_{66} D3[\xi_6];\end{aligned}$$

$$\begin{aligned}\xi_{244} &= D4[\xi_{24}] - g_{14} D4[\xi_1] - g_{24} D4[\xi_2] - g_{34} D4[\xi_3] - g_{44} D4[\xi_4] - g_{45} D4[\xi_5] - g_{46} D4[\xi_6]; \\ \xi_{245} &= D4[\xi_{25}] - g_{15} D4[\xi_1] - g_{25} D4[\xi_2] - g_{35} D4[\xi_3] - g_{45} D4[\xi_4] - g_{55} D4[\xi_5] - g_{56} D4[\xi_6]; \\ \xi_{246} &= D4[\xi_{26}] - g_{16} D4[\xi_1] - g_{26} D4[\xi_2] - g_{36} D4[\xi_3] - g_{46} D4[\xi_4] - g_{56} D4[\xi_5] - g_{66} D4[\xi_6];\end{aligned}$$

$$\begin{aligned}\xi_{255} &= D5[\xi_{25}] - g_{15} D5[\xi_1] - g_{25} D5[\xi_2] - g_{35} D5[\xi_3] - g_{45} D5[\xi_4] - g_{55} D5[\xi_5] - g_{56} D5[\xi_6]; \\ \xi_{256} &= D5[\xi_{26}] - g_{16} D5[\xi_1] - g_{26} D5[\xi_2] - g_{36} D5[\xi_3] - g_{46} D5[\xi_4] - g_{56} D5[\xi_5] - g_{66} D5[\xi_6];\end{aligned}$$

$$\xi_{266} = D6[\xi_{26}] - g_{16} D6[\xi_1] - g_{26} D6[\xi_2] - g_{36} D6[\xi_3] - g_{46} D6[\xi_4] - g_{56} D6[\xi_5] - g_{66} D6[\xi_6];$$

$$R[\text{exp\_}] := \xi_1 D[\text{exp}, x_1] + \xi_2 D[\text{exp}, x_2] + \xi_3 D[\text{exp}, x_3] + \xi_4 D[\text{exp}, x_4] +$$

```


$$\begin{aligned}
& \xi_5 D[\text{exp}, x_5] + \xi_6 D[\text{exp}, x_6] + \eta_1 D[\text{exp}, f] + \eta_2 D[\text{exp}, g] + \xi_{11} D[\text{exp}, f_1] + \\
& \xi_{12} D[\text{exp}, f_2] + \xi_{13} D[\text{exp}, f_3] + \xi_{14} D[\text{exp}, f_4] + \xi_{15} D[\text{exp}, f_5] + \\
& \xi_{16} D[\text{exp}, f_6] + \xi_{21} D[\text{exp}, g_1] + \xi_{22} D[\text{exp}, g_2] + \xi_{23} D[\text{exp}, g_3] + \xi_{24} D[\text{exp}, g_4] + \\
& \xi_{25} D[\text{exp}, g_5] + \xi_{26} D[\text{exp}, g_6] + \xi_{111} D[\text{exp}, f_{11}] + \xi_{112} D[\text{exp}, f_{12}] + \\
& \xi_{113} D[\text{exp}, f_{13}] + \xi_{114} D[\text{exp}, f_{14}] + \xi_{115} D[\text{exp}, f_{15}] + \xi_{116} D[\text{exp}, f_{16}] + \\
& \xi_{122} D[\text{exp}, f_{22}] + \xi_{123} D[\text{exp}, f_{23}] + \xi_{124} D[\text{exp}, f_{24}] + \xi_{125} D[\text{exp}, f_{25}] + \\
& \xi_{126} D[\text{exp}, f_{26}] + \xi_{133} D[\text{exp}, f_{33}] + \xi_{134} D[\text{exp}, f_{34}] + \xi_{135} D[\text{exp}, f_{35}] + \\
& \xi_{136} D[\text{exp}, f_{36}] + \xi_{144} D[\text{exp}, f_{44}] + \xi_{145} D[\text{exp}, f_{45}] + \xi_{146} D[\text{exp}, f_{46}] + \\
& \xi_{155} D[\text{exp}, f_{55}] + \xi_{156} D[\text{exp}, f_{56}] + \xi_{166} D[\text{exp}, f_{66}] + \xi_{211} D[\text{exp}, g_{11}] + \\
& \xi_{212} D[\text{exp}, g_{12}] + \xi_{213} D[\text{exp}, g_{13}] + \xi_{214} D[\text{exp}, g_{14}] + \xi_{215} D[\text{exp}, g_{15}] + \\
& \xi_{216} D[\text{exp}, g_{16}] + \xi_{222} D[\text{exp}, g_{22}] + \xi_{223} D[\text{exp}, g_{23}] + \xi_{224} D[\text{exp}, g_{24}] + \\
& \xi_{225} D[\text{exp}, g_{25}] + \xi_{226} D[\text{exp}, g_{26}] + \xi_{233} D[\text{exp}, g_{33}] + \xi_{234} D[\text{exp}, g_{34}] + \\
& \xi_{235} D[\text{exp}, g_{35}] + \xi_{236} D[\text{exp}, g_{36}] + \xi_{244} D[\text{exp}, g_{44}] + \xi_{245} D[\text{exp}, g_{45}] + \\
& \xi_{246} D[\text{exp}, g_{46}] + \xi_{255} D[\text{exp}, g_{55}] + \xi_{256} D[\text{exp}, g_{56}] + \xi_{266} D[\text{exp}, g_{66}] ;]
\end{aligned}$$


S = {Fa → f1, Fb → f2, Fc → f3, Fp → f4, Fq → f5, Fr → f6, Ga → g1, Gb → g2, Gc → g3, Gp → g4,
Gq → g5, Gr → g6, Faa → f11, Fab → f12, Fac → f13, Fap → f14, Faq → f15, Far → f16,
Fbb → f22, Fbc → f23, Fbp → f24, Fbq → f25, Fbr → f26, Fcc → f33, Fcp → f34, Fcq → f35,
Fcr → f36, Fpp → f44, Fpq → f45, Fpr → f46, Fqq → f55, Fqr → f56, Frr → f66,
Gaa → g11, Gab → g12, Gac → g13, Gap → g14, Gaq → g15, Gar → g16, Gbb → g22,
Gbc → g23, Gbp → g24, Gbq → g25, Gbr → g26, Gcc → g33, Gcp → g34, Gcq → g35,
Gcr → g36, Gpp → g44, Gpq → g45, Gpr → g46, Gqq → g55, Gqr → g56, Grr → g66};

factorlist = {};
SetAttributes[killfactor, Listable];
killfactor[a_b_] := killfactor[a] killfactor[b];
killfactor[a_^_] := a
killfactor[a_] := 1 /; MemberQ[factorlist, a];
killfactor[a_] := a;
killfactor[a_] := 1 /; IntegerQ[a];
killfactor[a_] :=
  1 /; (FreeQ[a, f11] && FreeQ[a, f12] && FreeQ[a, f13] && FreeQ[a, f14] &&
    FreeQ[a, f15] && FreeQ[a, f16] && FreeQ[a, f22] && FreeQ[a, f23] && FreeQ[a, f24] &&
    FreeQ[a, f25] && FreeQ[a, f26] && FreeQ[a, f33] && FreeQ[a, f34] && FreeQ[a, f35] &&
    FreeQ[a, f36] && FreeQ[a, f44] && FreeQ[a, f45] && FreeQ[a, f46] && FreeQ[a, f55] &&
    FreeQ[a, f56] && FreeQ[a, f66] && FreeQ[a, Gaa] && FreeQ[a, Gab] && FreeQ[a, Gac] &&
    FreeQ[a, Gap] && FreeQ[a, Gaq] && FreeQ[a, Gar] && FreeQ[a, g11] && FreeQ[a, g12] &&
    FreeQ[a, g13] && FreeQ[a, g14] && FreeQ[a, g15] && FreeQ[a, g16] && FreeQ[a, g22] &&
    FreeQ[a, g23] && FreeQ[a, g24] && FreeQ[a, g25] && FreeQ[a, g26] && FreeQ[a, g33] &&
    FreeQ[a, g34] && FreeQ[a, g35] && FreeQ[a, g36] && FreeQ[a, g44] && FreeQ[a, g45] &&
    FreeQ[a, g46] && FreeQ[a, g55] && FreeQ[a, g56] && FreeQ[a, g66]);
killfactor[
  0] :=
  0;

```

(\* a nondegenerate point in the first jets;

this can be substituted wlog due to the transitivity arguments of the paper\*)

pt = {f1 → -5, f2 → 1, f3 → 2, f4 → 1, f5 → -1,

f6 → 3, g1 → -4, g2 → 7, g3 → 1, g4 → 1, g5 → -5, g6 → 4};

(\*20 Linear degeneracy equations at the point\*)

$$\begin{aligned} \text{Sol} = \left\{ \begin{aligned} f_{33} &\rightarrow -\frac{484 f_{11}}{9} - \frac{572 f_{12}}{9} + \frac{44 f_{13}}{3} - \frac{169 f_{22}}{9} + \frac{26 f_{23}}{3}, \\ f_{36} &\rightarrow \frac{352 f_{11}}{9} + \frac{560 f_{12}}{9} - \frac{16 f_{13}}{3} - \frac{484 f_{14}}{9} - \frac{286 f_{15}}{9} + \frac{22 f_{16}}{3} + \\ &\quad \frac{208 f_{22}}{9} - \frac{16 f_{23}}{3} - \frac{286 f_{24}}{9} - \frac{169 f_{25}}{9} + \frac{13 f_{26}}{3} + \frac{22 f_{34}}{3} + \frac{13 f_{35}}{3}, \\ f_{55} &\rightarrow -f_{44} - 2 f_{45}, f_{56} \rightarrow -\frac{16 f_{14}}{3} - \frac{16 f_{15}}{3} - \frac{16 f_{24}}{3} - \frac{16 f_{25}}{3} + 3 f_{44} + 3 f_{45} - f_{46}, \\ f_{66} &\rightarrow -\frac{256 f_{11}}{9} - \frac{512 f_{12}}{9} + \frac{992 f_{14}}{9} + \frac{704 f_{15}}{9} - \frac{32 f_{16}}{3} - \frac{256 f_{22}}{9} + \\ &\quad \frac{704 f_{24}}{9} + \frac{416 f_{25}}{9} - \frac{32 f_{26}}{3} - \frac{32 f_{34}}{3} - \frac{32 f_{35}}{3} - 9 f_{44} + 6 f_{46}, \\ g_{14} &\rightarrow 4 f_{11} + 6 f_{14} + 2 f_{44} - \frac{3 g_{11}}{4}, g_{22} \rightarrow \frac{147 f_{11}}{8} + 21 f_{12} + 6 f_{22} - \frac{49 g_{11}}{16} - \frac{7 g_{12}}{2}, \\ g_{23} &\rightarrow -\frac{721 f_{11}}{24} - \frac{215 f_{12}}{6} + \frac{21 f_{13}}{2} - \frac{32 f_{22}}{3} + 6 f_{23} - \frac{7 g_{11}}{16} - \frac{g_{12}}{4} - \frac{7 g_{13}}{4}, \\ g_{24} &\rightarrow \frac{27 f_{11}}{8} + 8 f_{12} + 6 f_{15} + 6 f_{24} - \frac{3 f_{44}}{2} + 4 f_{45} - \frac{9 g_{11}}{16} - \frac{3 g_{12}}{2} - g_{15}, \\ g_{25} &\rightarrow -\frac{63 f_{11}}{8} - 9 f_{12} - \frac{f_{22}}{2} + 6 f_{25} - \frac{7 f_{44}}{2} - 7 f_{45} + \frac{21 g_{11}}{16} + \frac{3 g_{12}}{2}, \\ g_{33} &\rightarrow -\frac{4165 f_{11}}{72} - \frac{616 f_{12}}{9} + \frac{49 f_{13}}{3} - \frac{182 f_{22}}{9} + \frac{28 f_{23}}{3} - \frac{g_{11}}{16} - \frac{g_{13}}{2}, \\ g_{34} &\rightarrow -\frac{75 f_{11}}{8} + 8 f_{13} - 16 f_{14} + 6 f_{16} + 6 f_{34} - \frac{13 f_{44}}{2} + 4 f_{46} - \frac{7 g_{11}}{16} - \frac{3 g_{13}}{2} - g_{16}, \\ g_{35} &\rightarrow \frac{59 f_{11}}{2} + 35 f_{12} - 9 f_{13} - \frac{112 f_{14}}{3} - \frac{112 f_{15}}{3} + 16 f_{22} - f_{23} - \frac{112 f_{24}}{3} - \\ &\quad \frac{64 f_{25}}{3} + 6 f_{26} + 6 f_{35} + 10 f_{44} - f_{45} - 7 f_{46} - \frac{g_{11}}{4} - \frac{g_{12}}{2} + \frac{3 g_{13}}{2} - g_{26}, \\ g_{36} &\rightarrow \frac{857 f_{11}}{24} + \frac{170 f_{12}}{3} - \frac{13 f_{13}}{3} - \frac{488 f_{14}}{9} - \frac{308 f_{15}}{9} + \frac{20 f_{16}}{3} + \frac{131 f_{22}}{6} - \frac{13 f_{23}}{3} - \\ &\quad \frac{308 f_{24}}{9} - \frac{182 f_{25}}{9} + \frac{14 f_{26}}{3} + \frac{20 f_{34}}{3} + \frac{14 f_{35}}{3} + \frac{3 f_{44}}{2} - f_{46} - \frac{g_{11}}{16} - \frac{g_{13}}{2}, \\ g_{44} &\rightarrow -\frac{3 f_{11}}{2} - 2 f_{14} + \frac{g_{11}}{4}, g_{45} \rightarrow -\frac{9 f_{11}}{16} - \frac{3 f_{12}}{2} - f_{15} - f_{24} + \frac{3 g_{11}}{32} + \frac{g_{12}}{4}, \\ g_{46} &\rightarrow -\frac{7 f_{11}}{16} - \frac{3 f_{13}}{2} - f_{16} - f_{34} + \frac{13 g_{11}}{32} + \frac{g_{13}}{4}, g_{55} \rightarrow \frac{21 f_{11}}{8} + 3 f_{12} - 2 f_{25} - \frac{7 g_{11}}{16} - \frac{g_{12}}{2}, \\ g_{56} &\rightarrow -\frac{101 f_{11}}{12} - \frac{59 f_{12}}{6} + \frac{3 f_{13}}{2} - \frac{8 f_{22}}{3} - f_{26} - f_{35} + \frac{5 g_{11}}{8} + \frac{3 g_{12}}{4} - \frac{g_{13}}{4}, \\ g_{66} &\rightarrow -\frac{881 f_{11}}{72} - \frac{416 f_{12}}{9} - 9 f_{13} + \frac{968 f_{14}}{9} + \frac{572 f_{15}}{9} - \frac{44 f_{16}}{3} - \\ &\quad \frac{208 f_{22}}{9} + \frac{572 f_{24}}{9} + \frac{338 f_{25}}{9} - \frac{26 f_{26}}{3} - \frac{44 f_{34}}{3} - \frac{26 f_{35}}{3} + \frac{3 g_{11}}{16} + \frac{3 g_{13}}{2} \end{aligned} \right\}; \end{aligned}$$

(\*The condition\*)

```
sys = { (-2 Fq Fqr Fr^2 Gb + Fqq Fr^3 Gb + Fq^2 Fr Frr Gb + 2 Fq^2 Fqr Fr Gc - Fq Fqq Fr^2 Gc - Fq^3 Frr Gc +
        Fc Fq Fr^2 Gqq - Fb Fr^3 Gqq + Fr^3 Gq Gqq - 2 Fc Fq^2 Fr Gqr + 2 Fb Fq Fr^2 Gqr - 2 Fq Fr^2 Gq Gqr -
        Fq Fr^2 Gqq Gr + 2 Fq^2 Fr Gqr Gr + Fc Fq^3 Grr - Fb Fq^2 Fr Grr + Fq^2 Fr Gq Grr - Fq^3 Gr Grr) };
```

```
sys0 = sys /. S
```

```
{ -2 f5 f56 f6^2 g2 + f55 f6^3 g2 + f5^2 f6 f66 g2 + 2 f5^2 f56 f6 g3 - f5 f55 f6^2 g3 - f5^3 f66 g3 +
  f3 f5 f6^2 g55 - f2 f6^3 g55 + f6^3 g5 g55 - 2 f3 f5^2 f6 g56 + 2 f2 f5 f6^2 g56 - 2 f5 f6^2 g5 g56 -
  f5 f6^2 g55 g6 + 2 f5^2 f6 g56 g6 + f3 f5^3 g66 - f2 f5^2 f6 g66 + f5^2 f6 g5 g66 - f5^3 g6 g66 }
```

```
Length[sys0]
```

```
1
```

```
Factor[sys0 /. pt /. Sol]
```

```
{0}
```

(\*It - action by all generators of the SL6\*)

```
It[exp_] := Block[{
  list = {"X11", "X12", "X13", "X14", "X21", "X22", "X23",
    "X24", "X31", "X32", "X33", "X34", "X41", "X42", "X43", "X44", "L11",
    "L12", "L21", "L22", "P1", "P2", "P3", "P4", "Q1", "Q2", "Q3", "Q4"},
  i, sys1 = {}, sysf = {}}, Do[ExtDef[ToExpression[list[[i]]]];
  sys1 = killfactor[Factor[Complement[Flatten[CoefficientList[Complement[
    killfactor[Factor[R[exp]]], {0}], {x1, x2, x3, x4, x5, x6, f, g}], {0}]]];
  AppendTo[sysf, sys1];
  sysf = Union[Flatten[sysf]] (*;
  Print["Generator ", list[[i]], " has been applied. The length of the system is ",
    Length[sysf]] *), {i, 1, Length[list]};
  sysf];
```

```
Length[sys0]
```

```
1
```

```
sys1 = It[sys0];
```

```
sys1 = Sort[sys1, LeafCount[#1] < LeafCount[#2] &];
```

```
Length[sys1]
```

```
7
```

```
Length[Solve[(sys1 /. pt) == 0][[1]]]
```

```
3
```

```

(*Selecting linearly independent equations*)
sys1m = {sys1[[1]]};
len = 1;
Do[systemp = sys1m;
  AppendTo[systemp, sys1[[i]]];
  If[Length[Solve[(systemp /. pt) == 0][[1]]] > len, sys1m = systemp;
    len = len + 1, None], {i, 2, Length[sys1]}]

Length[Solve[(sys1m /. pt) == 0][[1]]]
Length[sys1m]
3
3

(*The system vanishes modulo linear degeneracy conditions*)
sys1m /. pt /. Sol // Factor
{0, 0, 0}

(*Next iteration*)
sys2 = It[sys1m];

sys2 = Sort[sys2, LeafCount[#1] < LeafCount[#2] &];
Length[sys2]
19

Length[Solve[(sys2 /. pt) == 0][[1]]]
6

(*Selecting linearly independent equations*)
sys2m = {sys2[[1]]};
len = 1;
Do[systemp = sys2m;
  AppendTo[systemp, sys2[[i]]];
  If[Length[Solve[(systemp /. pt) == 0][[1]]] > len, sys2m = systemp;
    len = len + 1, None], {i, 2, Length[sys2]}]

Length[Solve[(sys2m /. pt) == 0][[1]]]
Length[sys2m]
6
6

(*The system vanishes modulo linear degeneracy conditions*)
sys2m /. pt /. Sol // Factor
{0, 0, 0, 0, 0, 0}

```

```

(*Next iteration*)
sys3 = It[sys2m];

Length[sys3]
39

Length[Solve[(sys3 /. pt) == 0][[1]]]
10

sys3 = Sort[sys3, LeafCount[#1] < LeafCount[#2] &];
Length[sys3]
39

(*Selecting linearly independent equations*)
sys3m = {sys3[[1]]};
len = 1;
Do[systemp = sys3m;
  AppendTo[systemp, sys3[[i]]];
  If[Length[Solve[(systemp /. pt) == 0][[1]]] > len, sys3m = systemp;
    len = len + 1, None], {i, 2, Length[sys3]}]

Length[Solve[(sys3m /. pt) == 0][[1]]]
Length[sys3m]
10

10

(*The system vanishes modulo linear degeneracy conditions*)
sys3m /. pt /. Sol // Factor
{0, 0, 0, 0, 0, 0, 0, 0, 0, 0}

(*Next iteration*)
sys4 = It[sys3m];

Length[Solve[(sys4 /. pt) == 0][[1]]]
14

sys4 = Sort[sys4, LeafCount[#1] < LeafCount[#2] &];
Length[sys4]
61

```

```

(*Selecting linearly independent equations*)
sys4m = {sys4[[1]]};
len = 1;
Do[systemp = sys4m;
  AppendTo[systemp, sys4[[i]]];
  If[Length[Solve[(systemp /. pt) == 0][[1]]] > len, sys4m = systemp;
    len = len + 1, None], {i, 2, Length[sys4]}]

Length[Solve[(sys4m /. pt) == 0][[1]]]
Length[sys4m]
14
14

(*The system vanishes modulo linear degeneracy conditions*)
sys4m /. pt /. Sol // Factor
{0, 0, 0, 0, 0, 0, 0, 0, 0, 0, 0, 0, 0, 0}

(*Next iteration*)
sys5 = It[sys4m];

sys5 = Sort[sys5, LeafCount[#1] < LeafCount[#2] &];
Length[sys5]
82

Length[Solve[(sys5 /. pt) == 0][[1]]]
17

(*Selecting linearly independent equations*)
sys5m = {sys5[[1]]};
len = 1;
Do[systemp = sys5m;
  AppendTo[systemp, sys5[[i]]];
  If[Length[Solve[(systemp /. pt) == 0][[1]]] > len, sys5m = systemp;
    len = len + 1, None], {i, 2, Length[sys5]}]

Length[Solve[(sys5m /. pt) == 0][[1]]]
Length[sys5m]
17
17

(*The system vanishes modulo linear degeneracy conditions*)
sys5m /. pt /. Sol // Factor
{0, 0, 0, 0, 0, 0, 0, 0, 0, 0, 0, 0, 0, 0, 0, 0}

```

```

(*Next iteration*)
sys6 = It[sys5m];

sys6 = Sort[sys6, LeafCount[#1] < LeafCount[#2] &];
Length[sys6]
101

Length[Solve[(sys6 /. pt) == 0][[1]]]
19

(*Selecting linearly independent equations*)
sys6m = {sys6[[1]]};
len = 1;
Do[systemp = sys6m;
  AppendTo[systemp, sys6[[i]]];
  If[Length[Solve[(systemp /. pt) == 0][[1]]] > len, sys6m = systemp;
    len = len + 1, None], {i, 2, Length[sys6]}]

Length[Solve[(sys6m /. pt) == 0][[1]]]
Length[sys6m]
19
19

(*The system vanishes modulo linear degeneracy conditions*)
sys6m /. pt /. Sol // Factor
{0, 0, 0, 0, 0, 0, 0, 0, 0, 0, 0, 0, 0, 0, 0, 0, 0, 0, 0, 0}

(*Next iteration*)
sys7 = It[sys6m];

sys7 = Sort[sys7, LeafCount[#1] < LeafCount[#2] &];
Length[sys7]
Length[Solve[(sys7 /. pt) == 0][[1]]]
109
20

(*Selecting linearly independent equations*)
sys7m = {sys7[[1]]};
len = 1;
Do[systemp = sys7m;
  AppendTo[systemp, sys7[[i]]];
  If[Length[Solve[(systemp /. pt) == 0][[1]]] > len, sys7m = systemp;
    len = len + 1, None], {i, 2, Length[sys7]}]

```



```

Length[Solve[(sys7m /. pt) == 0][[1]]]
Length[sys7m]
20
20

(*The system vanishes modulo linear degeneracy conditions*)
sys7m /. pt /. Sol // Factor
{0, 0, 0, 0, 0, 0, 0, 0, 0, 0, 0, 0, 0, 0, 0, 0, 0, 0, 0, 0}

(*The dimension of sys7m is 20 and it
vanishes modulo the linear degeneracy conditions,
therefore sys7m is equivalent to the linear degeneracy conditions*)

(*Next iteration*)
sys8 = It[sys7m];

sys8 = Sort[sys8, LeafCount[#1] < LeafCount[#2] &];
Length[sys8]
Length[Solve[(sys8 /. pt) == 0][[1]]]
115
20

(*Selecting linearly independent equations*)
sys8m = {sys8[[1]]};
len = 1;
Do[systemp = sys8m;
  AppendTo[systemp, sys8[[i]]];
  If[Length[Solve[(systemp /. pt) == 0][[1]]] > len, sys8m = systemp;
    len = len + 1, None], {i, 2, Length[sys8]}]

Length[Solve[(sys8m /. pt) == 0][[1]]]
Length[sys8m]
20
20

sys8m /. pt /. Sol // Factor
{0, 0, 0, 0, 0, 0, 0, 0, 0, 0, 0, 0, 0, 0, 0, 0, 0, 0, 0, 0}

```

The system vanishes modulo the linear degeneracy conditions. The dimension of sys8m is 20, which is the same as the dimension of sys7m - stabilization under the action. Therefore the original condition sys0 is equivalent to 20 conditions of linear degeneracy modulo the action of SL6.
