# Supplementary material for: Integrable systems in 4D associated with sixfolds in Gr(4,6)
Source: arXiv:1705.06999 ancillary file (2017-05-18)
Supplement: Supplementary file 7 [file DFKN-2017-Stabilizers.pdf]

This worksheet accompanies the paper B.Doubrov, E.Ferapontov, B.Kruglikov, V.Novikov "Integrable systems in 4D associated with sixfolds in Gr(4,6)".

The file ran on **Maple** version 17, the package **DifferentialGeometry** was used.

## I. Computation of the stabilizer for the integrable systems in 4D associated with quadratic maps $P^6 \rightarrow \text{Gr}(4,6)$

```

> restart :
> with(DifferentialGeometry) : with(GroupActions) : with(JetCalculus) : with(Tools) :
  with(LieAlgebras) : with(LinearAlgebra) : with(Physics) :
  Preferences("ShowFramePrompt",false) :
> DGsetup([x1, x2, x3, x4], [u, v], J0, 1) :
> V := evalDG((a11·x1 + a12·x2 + a13·x3 + a14·x4 + a15·u[ ] + a16·v[ ])·D_x1 + (a21·x1
  + a22·x2 + a23·x3 + a24·x4 + a25·u[ ] + a26·v[ ])·D_x2 + (a31·x1 + a32·x2 + a33
  ·x3 + a34·x4 + a35·u[ ] + a36·v[ ])·D_x3 + (a41·x1 + a42·x2 + a43·x3 + a44·x4
  + a45·u[ ] + a46·v[ ])·D_x4 + (a51·x1 + a52·x2 + a53·x3 + a54·x4 + a55·u[ ] + a56
  ·v[ ])·D_u[ ] + (a61·x1 + a62·x2 + a63·x3 + a64·x4 + a65·u[ ] - (a11 + a22 + a33
  + a44 + a55)·v[ ])·D_v[ ]) :
> V1 := Prolong(V, 1) :
> uv := [[u1, u2, u3, u4], [v1, v2, v3, v4]] : Cf := (i, j) → LieDerivative(V1, uv[i, j]) :
> for i to 2 do for j to 4 do (S||i)||j := subs({u1 = z11, u2 = z12, u3 = z13, u4 = w1[ ], v1 = z21,
  v2 = z22, v3 = z23, v4 = w2[ ]}, Cf(i, j)) : od:od:
> DGsetup([z11, z12, z13, z21, z22, z23], [w1, w2], K, 1) :
> W := evalDG(S11·D_z11 + S12·D_z12 + S13·D_z13 + S14·D_w1[ ] + S21·D_z21 + S22
  ·D_z22 + S23·D_z23 + S24·D_w2[ ]) : W1 := Prolong(W, 1) :
>
> Mg := subs(m(6, 6) = -(m(1, 1) + m(2, 2) + m(3, 3) + m(4, 4) + m(5, 5)), Matrix(6,
  m)) : M := [ ] : for i to 6 do for j to 6 do M := [op(M), coeff(Mg, m(i, j))] : od:od: M
  := M[1..35] :
> L := LieAlgebraData(M, Ex) : DGsetup(L) :
> CF := {u[1], u[2], u[3], u[4], v[1], v[2], v[3], v[4]} :
> var := [x1, x2, x3, x4, u[ ], v[ ]] : dvar := evalDG([dx1, dx2, dx3, dx4, du[ ], dv[ ]]) :
> EC := v → subs({E11 = e1, E12 = e2, E13 = e3, E14 = e4, E15 = e5, E16 = e6, E21 = e7, E22
  = e8, E23 = e9, E24 = e10, E25 = e11, E26 = e12, E31 = e13, E32 = e14, E33 = e15, E34
  = e16, E35 = e17, E36 = e18, E41 = e19, E42 = e20, E43 = e21, E44 = e22, E45 = e23, E46
  = e24, E51 = e25, E52 = e26, E53 = e27, E54 = e28, E55 = e29, E56 = e30, E61 = e31, E62
  = e32, E63 = e33, E64 = e34, E65 = e35, E66 = 0}, add(add((E||i)||j)·diff(Hook(v,
  dvar[i]), var[j]), i = 1..6), j = 1..6)) :
> EC(evalDG(u[ ]·D_u[ ] - v[ ]·D_v[ ]))

```

e29

(1)

Type [1,1,1,1]

```

> EQ := [u1 v2 - α u2 v1, u1 v3 - u4 v1] : S := solve(EQ, {v[2], v[3]}) :
> OT := {coeffs(numer(simplify(subs(S, LieDerivative(V1, EQ[1])))), CF),

```

```

coeffs(numer(simplify(subs(S, LieDerivative(VI, EQ[2])))), CF) } :
> R := solve(OT, {seq(seq((a||i)||j, i=1..6), j=1..6)}[1..35]):
> VF := subs(R, V)
VF := (a11 x1 + a14 x3 + a14 x4) D_x1 + (a23 α x4 + a22 x2 + a23 x3) D_x2
      + a44 x3 D_x3 + a44 x4 D_x4 + (a53 x3 + a55 u[]) D_u[] - ((a11 v[] + a22 v[]
      + 2 a44 v[] + a55 v[] - a64 x4) D_v[])
(2)
> coe := [a11, a14, a22, a23, a44, a53, a55, a64] :for i to nops(coe) do SuV||i := [seq(coe[j]
      = KroneckerDelta[i, j], j=1..nops(coe))] :od:
> SVF := DGsimplify(evalDG([seq(subs(SuV||i, VF), i=1..nops(coe))]))
SVF := [x1 D_x1 - (v[] D_v[]), (x3 + x4) D_x1, x2 D_x2 - (v[] D_v[]), (α x4
      + x3) D_x2, x3 D_x3 + x4 D_x4 - (2 v[] D_v[]), x3 D_u[], u[] D_u[] - (v[] D_v[]),
      x4 D_v[]]
(3)
> nops(coe); LieAlgebraData(SVF, alg)
8
[[e1, e2] = -e2, [e1, e8] = e8, [e2, e5] = -e2, [e3, e4] = -e4, [e3, e8] = e8, [e4, e5] = -e4,
[e5, e6] = e6, [e5, e8] = 3 e8, [e6, e7] = e6, [e7, e8] = e8]
(4)
> [[e1, e2] = -e2, [e1, e8] = e8, [e2, e5] = -e2, [e3, e4] = -e4, [e3, e8] = e8, [e4, e5] = -e4,
[e5, e6] = e6, [e5, e8] = 3 e8, [e6, e7] = e6, [e7, e8] = e8]
> Out := {} :for i to nops(SVF) do Out := {op(Out), EC(SVF[i])} :od: Out
{e10 α + e9, e15 + e22, e3 + e4, e1, e27, e29, e34, e8}
(5)
> DGsetup(L) : Centralizer(convert(Out, 'list'))
[]
(6)
> SubalgebraNormalizer(convert(Out, 'list')); nops(%)
[e34, e29, e27, e15 + e22, 1/α e9 + e10, e8, e3 + e4, e1]
8
(7)
> Ser := Series(convert(Out, 'list'), "Derived"); map(v→nops(v), Ser)
Ser := [[e9 + α e10, e3 + e4, e15 + e22, e1, e8, e27, e29, e34], [e9 + α e10, e3 + e4, -e27,
- (3 e34)], []]
[8, 4, 0]
(8)
> StrEq := subs({seq(e||i=v||i, i=1..8)}, [[e1, e2] = -e2, [e1, e8] = e8, [e2, e5] = -e2, [e3,
e4] = -e4, [e3, e8] = e8, [e4, e5] = -e4, [e5, e6] = e6, [e5, e8] = 3 e8, [e6, e7] = e6, [e7, e8]
= e8]), [seq(v||i, i=1..8)] : LAstr := LieAlgebraData(StrEq, La1) : DGsetup(LAstr)
Lie algebra: La1
(9)
> LieAlgebraData([1/6 (e5 + e1 + e3 + e7) - e1, 1/6 (e5 + e1 + e3 + e7) - e3, 1/6 (e5 + e1
+ e3 + e7) - e7, 1/6 (e5 + e1 + e3 + e7), e2, e4, e6, e8])
[[e1, e5] = e5, [e2, e6] = e6, [e3, e7] = e7, [e4, e8] = e8]
(10)

```

dim(Stab)=8, non-Abelian, self-normalizing, derived series (8,4,0)

>

Type [2,1,1]

> with(DifferentialGeometry) :

> EQ :=  $[u_1 v_2 - u_2 v_1 + v_1 v_2, u_1 v_4 - u_4 v_1 + v_1 v_3] : S := \text{solve}(EQ, \{v[2], v[3]\}) :$

> OT := {coeffs(numer(simplify(subs(S, LieDerivative(V1, EQ[1])))), CF),  
coeffs(numer(simplify(subs(S, LieDerivative(V1, EQ[2])))), CF)} :

> R := solve(OT, {seq(seq((a||i)||j, i=1..6), j=1..6)}[1..35]):

> VF := subs(R, V)

VF :=  $(a11 x1 + a14 x4) D_{x1} + (a22 x2 + a23 x3 + a23 x4) D_{x2} + a33 x3 D_{x3}$  (11)

$$+ a33 x4 D_{x4} - \left( \left( -a53 x3 - a54 x4 - \left( -a33 - \frac{a22}{2} - \frac{a11}{2} \right) u_{[]} \right. \right. \\ \left. \left. - a56 v_{[]} \right) D_{u_{[]}} \right) - \left( \left( a11 v_{[]} + a22 v_{[]} + 2 a33 v_{[]} + \left( -a33 - \frac{a22}{2} - \frac{a11}{2} \right) v_{[]} \right. \right. \\ \left. \left. - a54 x3 \right) D_{v_{[]}} \right)$$

> coe := [a11, a14, a22, a23, a33, a53, a54, a56] :for i to nops(coe) do SuV||i := [seq(coe[j]  
= KroneckerDelta[i,j], j=1..nops(coe))] :od:

> SVF := DGsimplify(evalDG([seq(subs(SuV||i, VF), i=1..nops(coe))]))

SVF :=  $\left[ x1 D_{x1} - \left( \frac{u_{[]}}{2} D_{u_{[]}} \right) - \left( \frac{v_{[]}}{2} D_{v_{[]}} \right), x4 D_{x1}, x2 D_{x2} - \left( \frac{u_{[]}}{2} D_{u_{[]}} \right) \right]$  (12)

$$- \left( \frac{v_{[]}}{2} D_{v_{[]}} \right), (x3 + x4) D_{x2}, x3 D_{x3} + x4 D_{x4} - (u_{[]} D_{u_{[]}}) - (v_{[]} D_{v_{[]}}),$$

$$x3 D_{u_{[]}}, x4 D_{u_{[]}} + x3 D_{v_{[]}}, v_{[]} D_{u_{[]}} \Big]$$

> nops(coe); LieAlgebraData(SVF, alg)

8

$[e1, e2] = -e2, [e1, e6] = \frac{1}{2} e6, [e1, e7] = \frac{1}{2} e7, [e2, e5] = -e2, [e3, e4] = -e4, [e3, e6]$  (13)

$$= \frac{1}{2} e6, [e3, e7] = \frac{1}{2} e7, [e4, e5] = -e4, [e5, e6] = 2 e6, [e5, e7] = 2 e7, [e7, e8] = e6$$

> Out := {} :for i to nops(SVF) do Out := {op(Out), EC(SVF[i])} :od: Out

$$\left\{ e1 - \frac{1}{2} e29, e33 + e28, e8 - \frac{1}{2} e29, e9 + e10, e15 + e22 - e29, e27, e30, e4 \right\} \quad (14)$$

> DGsetup(L) : Centralizer(convert(Out,'list'))

[ ]

(15)

> SubalgebraNormalizer(convert(Out,'list')); nops(%)

$$[-(2 e1) + e29, e27, -(2 e1) + e15 + e22, e9 + e10, -e1 + e8, e4, e28 + e33, e30]$$

8

(16)

> Ser := Series(convert(Out,'list'), "Derived"); map(v→nops(v), Ser)

$$Ser := \left[ \left[ e1 - \left( \frac{1}{2} e29 \right), e8 - \left( \frac{1}{2} e29 \right), e9 + e10, e28 + e33, e15 + e22 - e29, e4, e27, \right. \right. \\ \left. \left. e30 \right], \left[ - \left( \frac{1}{2} e28 \right) - \left( \frac{1}{2} e33 \right), e4, - \left( \frac{1}{2} e27 \right), e9 + e10 \right], [ ] \right] \\ [8, 4, 0] \quad (17)$$

$$> StrEq := subs \left( \{ seq(e || i = v || i, i = 1 .. 8) \}, \left[ [e1, e2] = -e2, [e1, e6] = \frac{1}{2} e6, [e1, e7] = \frac{1}{2} e7, \right. \right. \\ [e2, e5] = -e2, [e3, e4] = -e4, [e3, e6] = \frac{1}{2} e6, [e3, e7] = \frac{1}{2} e7, [e4, e5] = -e4, [e5, e6] \\ = 2 e6, [e5, e7] = 2 e7, [e7, e8] = e6 \left. \right], [seq(v || i, i = 1 .. 8)] : LAstr2 \\ := LieAlgebraData(StrEq, La2) : DGsetup(LAstr2) \\ Lie algebra: La2 \quad (18)$$

$$> LieAlgebraData \left( \left[ \left[ \frac{1}{6} (e5 + e1 + e3) - e1, \frac{1}{6} (e5 + e1 + e3) - e3, \frac{1}{3} (e5 + e1 + e3), e8, e2, \right. \right. \right. \\ \left. \left. \left. e4, e6, -e7 \right] \right] \right) \\ [[e1, e5] = e5, [e2, e6] = e6, [e3, e7] = e7, [e3, e8] = e8, [e4, e8] = e7] \quad (19)$$

dim(Stab)=8, non-Abelian, self-normalizing, derived series (8,4,0)

$$> \\ Type [2,2] \\ > with(DifferentialGeometry) : \\ > EQ := [u1 v2 - u2 v1 + v1^2, u1 v4 - u4 v1 + v1 v3] : S := solve(EQ, {v[2], v[3]}) : \\ > OT := {coeffs(numer(simplify(subs(S, LieDerivative(V1, EQ[1])))), CF), \\ coeffs(numer(simplify(subs(S, LieDerivative(V1, EQ[2])))), CF)} : \\ > R := solve(OT, {seq(seq((a || i) || j, i = 1 .. 6), j = 1 .. 6)} [1 .. 35]) : \\ > VF := subs(R, V) \\ VF := (a11 x1 + a12 x2 + a13 x3 + a14 x4) D_x1 + (a13 x4 + a22 x2) D_x2 + a33 x3 D_x3 \quad (20)$$

$$+ (a33 + a22 - a11) x4 D_x4 - \left( \left( -a53 x3 - a54 x4 - \left( -a33 - \frac{a22}{2} - \frac{a11}{2} \right) u_{[]} \right. \right. \\ \left. \left. - a56 v_{[]} \right) D_{u_{[]}} \right) + \left( -a11 v_{[]} - a22 v_{[]} - a33 v_{[]} - (a33 + a22 - a11) v_{[]} - \left( \right. \right. \\ \left. \left. - a33 - \frac{a22}{2} - \frac{a11}{2} \right) v_{[]} + a54 x3 \right) D_{v_{[]}}$$

$$> coe := [a11, a12, a13, a14, a22, a33, a53, a54, a56] : for i to nops(coe) do SuV || i \\ := [seq(coe[j] = KroneckerDelta[i, j], j = 1 .. nops(coe))] : od : \\ > SVF := DGsimplify(evalDG([seq(subs(SuV || i, VF), i = 1 .. nops(coe))])) \\ SVF := [x1 D_x1 - (x4 D_x4) - \left( \frac{u_{[]}}{2} D_{u_{[]}} \right) + \frac{v_{[]}}{2} D_{v_{[]}}, x2 D_x1, x3 D_x1 + x4 D_x2, \quad (21)$$

$$x4 D_{x1}, x2 D_{x2} + x4 D_{x4} - \left( \frac{u_{[]}}{2} D_{u_{[]}} \right) - \left( \frac{3 v_{[]}}{2} D_{v_{[]}} \right), x3 D_{x3} + x4 D_{x4} \\ - (u_{[]} D_{u_{[]}}) - (v_{[]} D_{v_{[]}}), x3 D_{u_{[]}}, x4 D_{u_{[]}} + x3 D_{v_{[]}}, v_{[]} D_{u_{[]}} \Big]$$

> nops(coe); LieAlgebraData(SVF, alg)

9

$$\left[ [e1, e2] = -e2, [e1, e3] = -e3, [e1, e4] = -2 e4, [e1, e7] = \frac{1}{2} e7, [e1, e8] = -\frac{1}{2} e8, [e1, e9] = e9, [e2, e3] = -e4, [e2, e5] = -e2, [e3, e6] = -e3, [e4, e5] = -e4, [e4, e6] = -e4, [e5, e7] = \frac{1}{2} e7, [e5, e8] = \frac{3}{2} e8, [e5, e9] = -e9, [e6, e7] = 2 e7, [e6, e8] = 2 e8, [e8, e9] = e7 \right] \quad (22)$$

> Out := { } :for i to nops(SVF) do Out := {op(Out), EC(SVF[i])} :od: Out

$$\left\{ e3 + e10, e33 + e28, e1 - e22 - \frac{1}{2} e29, e15 + e22 - e29, e8 + e22 - \frac{1}{2} e29, e2, e27, e30, e4 \right\} \quad (23)$$

> DGsetup(L) : Centralizer(convert(Out,'list'))

[ ]

(24)

> SubalgebraNormalizer(convert(Out,'list')); nops(%)

$$\left[ e28 + e33, e30, -e1 - e8 + e29, e27, -\left( \frac{1}{2} e1 \right) + \frac{1}{2} e8 + e22, -\left( \frac{1}{2} e1 \right) - \left( \frac{3}{2} e8 \right) + e15, e3 + e10, e4, e2 \right]$$

9

(25)

> Ser := Series(convert(Out,'list'), "Derived"); map(v→nops(v), Ser)

$$Ser := \left[ \left[ e3 + e10, e28 + e33, e1 - e22 - \left( \frac{1}{2} e29 \right), e8 + e22 - \left( \frac{1}{2} e29 \right), e15 + e22 - e29, e2, e4, e27, e30 \right], \left[ -e3 - e10, -e4, -\left( \frac{1}{2} e28 \right) - \left( \frac{1}{2} e33 \right), -e27, e2, -e30 \right], \left[ e4, -\left( \frac{1}{2} e27 \right) \right], [ ] \right]$$

[9, 6, 2, 0]

(26)

> LieAlgebraData([seq(e||i, i=1..8)])

$$\left[ [e1, e2] = -e2, [e1, e6] = \frac{1}{2} e6, [e1, e7] = \frac{1}{2} e7, [e2, e5] = -e2, [e3, e4] = -e4, [e3, e6] = \frac{1}{2} e6, [e3, e7] = \frac{1}{2} e7, [e4, e5] = -e4, [e5, e6] = 2 e6, [e5, e7] = 2 e7, [e7, e8] = e6 \right] \quad (27)$$

$$\begin{aligned}
> \text{StrEq} := \text{subs} \left( \left\{ \text{seq}(e \parallel i = v \parallel i, i = 1 \dots 9) \right\}, \left[ [e1, e2] = -e2, [e1, e3] = -e3, [e1, e4] = -2 e4, \right. \right. \\
[e1, e7] = \frac{1}{2} e7, [e1, e8] = -\frac{1}{2} e8, [e1, e9] = e9, [e2, e3] = -e4, [e2, e5] = -e2, [e3, e6] \\
= -e3, [e4, e5] = -e4, [e4, e6] = -e4, [e5, e7] = \frac{1}{2} e7, [e5, e8] = \frac{3}{2} e8, [e5, e9] = -e9, \\
\left. [e6, e7] = 2 e7, [e6, e8] = 2 e8, [e8, e9] = e7 \right] \right), [\text{seq}(v \parallel i, i = 1 \dots 9)] : \text{LAstr3} \\
:= \text{LieAlgebraData}(\text{StrEq}, \text{La3}) : \text{DGsetup}(\text{LAstr3}) \\
\text{Lie algebra: La3} \tag{28}
\end{aligned}$$

$$\begin{aligned}
> \text{LieAlgebraData} \left( \left[ \left[ -e1 - e6 + \frac{1}{2} (e6 + e5 + e1), -e5 - e1 + \frac{1}{3} (e6 + e5 + e1), \frac{1}{3} (e6 \right. \right. \right. \\
\left. \left. \left. + e5 + e1), e2, e3, e8, e9, -e4, e7 \right] \right] \right) \\
[[e1, e4] = e4, [e1, e7] = -e7, [e1, e8] = e8, [e1, e9] = -e9, [e2, e5] = e5, [e2, e8] = e8, [e3, \\
e6] = e6, [e3, e9] = e9, [e4, e5] = e8, [e6, e7] = e9] \tag{29}
\end{aligned}$$

dim(Stab)=9, non-Abelian, self-normalizing, derived series (9,6,2,0)

$$\begin{aligned}
> \\
\text{Type [3,1]} \\
> \text{with}(\text{DifferentialGeometry}) : \\
> \text{EQ} := [\mathbf{u_2} + \mathbf{v_1} \mathbf{v_2}, \mathbf{u_4} - \mathbf{v_3} + \mathbf{v_1} \mathbf{v_4}] : S := \text{solve}(\text{EQ}, \{v[2], v[3]\}) : \\
> \text{OT} := \{\text{coeffs}(\text{numer}(\text{simplify}(\text{subs}(S, \text{LieDerivative}(V1, \text{EQ}[1])))), CF), \\
\text{coeffs}(\text{numer}(\text{simplify}(\text{subs}(S, \text{LieDerivative}(V1, \text{EQ}[2])))), CF)\} : \\
> R := \text{solve}(\text{OT}, \{\text{seq}(\text{seq}((a \parallel i) \parallel j, i = 1 \dots 6), j = 1 \dots 6)\} [1 \dots 35]) : \\
> VF := \text{subs}(R, V)
\end{aligned}$$

$$\begin{aligned}
VF := (a11 x1 + a13 x3) D\_x1 + (a22 x2 + a24 x4) D\_x2 + \left( -a55 - \frac{a22}{2} \right. \\
\left. - \frac{a11}{2} \right) x3 D\_x3 + \left( -\frac{a55}{2} - \frac{a22}{2} - a11 \right) x4 D\_x4 + (a51 x1 + a53 x3 + a54 x4 \\
+ a55 u_{[]} + a56 v_{[]}) D\_u_{[]} + \left( -a11 v_{[]} - a22 v_{[]} - \left( -a55 - \frac{a22}{2} - \frac{a11}{2} \right) v_{[]} - \left( \right. \right. \\
\left. \left. - \frac{a55}{2} - \frac{a22}{2} - a11 \right) v_{[]} - a55 v_{[]} - a56 x1 + a54 x3 - a13 x4 \right) D\_v_{[]} \tag{30}
\end{aligned}$$

$$\begin{aligned}
> \text{coe} := [a11, a13, a22, a24, a51, a53, a54, a55, a56] : \text{for } i \text{ to } \text{nops}(\text{coe}) \text{ do } \text{SuV} \parallel i \\
:= [\text{seq}(\text{coe}[j] = \text{KroneckerDelta}[i, j], j = 1 \dots \text{nops}(\text{coe}))] : \text{od} : \\
> \text{SVF} := \text{DGsimplify}(\text{evalDG}([\text{seq}(\text{subs}(\text{SuV} \parallel i, VF), i = 1 \dots \text{nops}(\text{coe}))])) \\
\text{SVF} := \left[ x1 D\_x1 - \left( \frac{x3}{2} D\_x3 \right) - (x4 D\_x4) + \frac{v_{[]}}{2} D\_v_{[]}, x3 D\_x1 - (x4 D\_v_{[]}), x2 D\_x2 \right. \\
\left. - \left( \frac{x3}{2} D\_x3 \right) - \left( \frac{x4}{2} D\_x4 \right), x4 D\_x2, x1 D\_u_{[]}, x3 D\_u_{[]}, x4 D\_u_{[]} + x3 D\_v_{[]} \right] \tag{31}
\end{aligned}$$

$$-(x3 D_{x3}) - \left( \frac{x4}{2} D_{x4} \right) + u_{[]} D_{u[]} + \frac{v_{[]}}{2} D_{v[]} , v_{[]} D_{u[]} - (x1 D_{v[]}) \Bigg]$$

> nops(coe); LieAlgebraData(SVF, alg)

9

$$\begin{aligned} & \left[ [e1, e2] = -\frac{3}{2} e2, [e1, e4] = -e4, [e1, e5] = e5, [e1, e6] = -\frac{1}{2} e6, [e1, e7] = -e7, [e1, e9] \right. \\ & = \frac{1}{2} e9, [e2, e3] = \frac{1}{2} e2, [e2, e5] = e6, [e2, e8] = e2, [e2, e9] = -e7, [e3, e4] = -\frac{3}{2} e4, \\ & [e3, e6] = -\frac{1}{2} e6, [e3, e7] = -\frac{1}{2} e7, [e4, e8] = \frac{1}{2} e4, [e5, e8] = e5, [e6, e8] = 2 e6, [e7, \\ & \left. e8] = \frac{3}{2} e7, [e7, e9] = e6, [e8, e9] = -\frac{1}{2} e9 \right] \end{aligned} \quad (32)$$

> Out := { } :for i to nops(SVF) do Out := {op(Out), EC(SVF[i])} :od: Out

$$\left\{ e3 - e34, -e31 + e30, e33 + e28, e1 - \frac{1}{2} e15 - e22, -e15 - \frac{1}{2} e22 + e29, e8 - \frac{1}{2} e15 \right. \\ \left. - \frac{1}{2} e22, e10, e25, e27 \right\} \quad (33)$$

> DGsetup(L) : Centralizer(convert(Out,'list'))

[ ]

(34)

> SubalgebraNormalizer(convert(Out,'list')); nops(%)

$$[e1 - (3 e8) + e29, e27, e25, -(2 e1) + 2 e8 + e22, 2 e1 - (4 e8) + e15, e10, -e3 + e34, \\ e28 + e33, -e30 + e31]$$

9

(35)

> Ser := Series(convert(Out,'list'), "Derived"); map(v→nops(v), Ser)

$$\begin{aligned} Ser := & \left[ \left[ e3 - e34, e30 - e31, e28 + e33, e1 - \left( \frac{1}{2} e15 \right) - e22, e8 - \left( \frac{1}{2} e15 \right) \right. \right. \\ & - \left( \frac{1}{2} e22 \right), -e15 - \left( \frac{1}{2} e22 \right) + e29, e10, e25, e27 \Bigg], \left[ e28 + e33, -\left( \frac{3}{2} e3 \right) \right. \\ & + \frac{3}{2} e34, -e27, \frac{1}{2} e30 - \left( \frac{1}{2} e31 \right), e10, -e25 \Bigg], \left[ -\left( \frac{1}{2} e27 \right), -\left( \frac{3}{4} e28 \right) \right. \\ & \left. \left. - \left( \frac{3}{4} e33 \right) \right], [ ] \right] \end{aligned}$$

[9, 6, 2, 0]

(36)

$$\begin{aligned} & \text{StrEq} := \text{subs} \left( \{ \text{seq}(e || i = v || i, i = 1..9) \}, \left[ [e1, e2] = -\frac{3}{2} e2, [e1, e4] = -e4, [e1, e5] = e5, \right. \right. \\ & [e1, e6] = -\frac{1}{2} e6, [e1, e7] = -e7, [e1, e9] = \frac{1}{2} e9, [e2, e3] = \frac{1}{2} e2, [e2, e5] = e6, [e2, e8] \\ & \left. = e2, [e2, e9] = -e7, [e3, e4] = -\frac{3}{2} e4, [e3, e6] = -\frac{1}{2} e6, [e3, e7] = -\frac{1}{2} e7, [e4, e8] \right. \end{aligned}$$

$$= \frac{1}{2} e_4, [e_5, e_8] = e_5, [e_6, e_8] = 2 e_6, [e_7, e_8] = \frac{3}{2} e_7, [e_7, e_9] = e_6, [e_8, e_9] = -\frac{1}{2} e_9 \Bigg] \\ , [seq(v||i, i = 1..9)] : LAstr4 := LieAlgebraData(StrEq, La4) : DGsetup(LAstr4) \\ \text{Lie algebra: La4} \quad (37)$$

$$\begin{aligned} &> LieAlgebraData\left(\left[-e_8 - \frac{1}{2} (4 e_3 - 2 e_8) - \frac{1}{2} \left(e_1 - \frac{3}{2} e_8 - \frac{5}{4} (4 e_3 - 2 e_8)\right), 4 e_3 \right. \right. \\ &\quad \left. \left. - 2 e_8 + \frac{5}{6} \left(e_1 - \frac{3}{2} e_8 - \frac{5}{4} (4 e_3 - 2 e_8)\right), \frac{1}{6} \left(e_1 - \frac{3}{2} e_8 - \frac{5}{4} (4 e_3 - 2 e_8)\right), \right. \right. \\ &\quad \left. \left. e_2, e_9, e_5, e_4, -e_7, e_6\right]\right) \\ &[[e_1, e_4] = e_4, [e_1, e_8] = e_8, [e_1, e_9] = e_9, [e_2, e_5] = e_5, [e_2, e_6] = 2 e_6, [e_2, e_8] = e_8, [e_2, \\ &\quad e_9] = 2 e_9, [e_3, e_7] = e_7, [e_4, e_5] = e_8, [e_4, e_6] = e_9, [e_5, e_8] = e_9] \end{aligned} \quad (38)$$

> dim(Stab)=9, non-Abelian, self-normalizing, derived series (9,6,2,0)

> Type [4]

> with(DifferentialGeometry) :

> EQ :=  $[u_1 - v_2 + v_1^2, u_4 - v_3 + v_1 v_4] : S := solve(EQ, \{v[2], v[3]\}) :$

> OT := {coeffs(numer(simplify(subs(S, LieDerivative(V1, EQ[1])))), CF),  
coeffs(numer(simplify(subs(S, LieDerivative(V1, EQ[2])))), CF)} :

> R := solve(OT, {seq(seq((a||i)||j, i = 1..6), j = 1..6)}[1..35]):

> VF := subs(R, V)

$$VF := (a11 x1 + (-2 a61 - a56) x2 + a13 x3 + a14 x4) D\_x1 + (a14 x3 + a22 x2) D\_x2 \quad (39)$$

$$+ \left(\frac{3 a22}{2} - \frac{7 a11}{2}\right) x3 D\_x3 - \left(\left(-(-a61 - a56) x3 - \left(\frac{a22}{2} - \frac{5 a11}{2}\right) x4\right) D\_x4\right) + (a51 x1 + a52 x2 + a53 x3 + a54 x4 + (-2 a22 + 3 a11) u_{[]} \\ + a56 v_{[]}) D\_u_{[]} + \left(-a11 v_{[]} - a22 v_{[]} - \left(\frac{3 a22}{2} - \frac{7 a11}{2}\right) v_{[]} - \left(\frac{a22}{2} - \frac{5 a11}{2}\right) v_{[]} - (-2 a22 + 3 a11) v_{[]} + a61 x1 + a51 x2 + a54 x3 - a13 x4\right) D\_v_{[]}$$

> coe := [a11, a13, a14, a22, a51, a52, a53, a54, a56, a61] :for i to nops(coe) do SuV||i  
:= [seq(coe[j] = KroneckerDelta[i, j], j = 1..nops(coe))] :od:

> SVF := DGsimplify(evalDG([seq(subs(SuV||i, VF), i = 1..nops(coe))]))

$$SVF := \left[x1 D\_x1 - \left(\frac{7 x3}{2} D\_x3\right) - \left(\frac{5 x4}{2} D\_x4\right) + 3 u_{[]} D\_u_{[]} + 2 v_{[]} D\_v_{[]}, x3 D\_x1 \right. \quad (40)$$

$$\left. - (x4 D\_v_{[]}), x4 D\_x1 + x3 D\_x2, x2 D\_x2 + \frac{3 x3}{2} D\_x3 + \frac{x4}{2} D\_x4 - (2 u_{[]} D\_u_{[]}) \right.$$

$$\left. - (v_{[]} D\_v_{[]}), x1 D\_u_{[]} + x2 D\_v_{[]}, x2 D\_u_{[]}, x3 D\_u_{[]}, x4 D\_u_{[]} + x3 D\_v_{[]}, \right.$$



$$-(x2 D_{x1}) - (x3 D_{x4}) + v_{[]} D_{u_{[]}}, -(2 x2 D_{x1}) - (x3 D_{x4}) + x1 D_{v_{[]}]}]$$

> nops(coe); LieAlgebraData(SVF, alg)

10

$$\begin{aligned} [e1, e2] = -\frac{9}{2} e2, [e1, e3] = -\frac{7}{2} e3, [e1, e5] = -2 e5, [e1, e6] = -3 e6, [e1, e7] = \\ -\frac{13}{2} e7, [e1, e8] = -\frac{11}{2} e8, [e1, e9] = -e9, [e1, e10] = -e10, [e2, e4] = -\frac{3}{2} e2, [e2, \\ e5] = e7, [e2, e9] = -e8, [e3, e4] = -\frac{1}{2} e3, [e3, e5] = e8, [e3, e6] = e7, [e3, e10] = -e2, \\ [e4, e5] = 2 e5, [e4, e6] = 3 e6, [e4, e7] = \frac{7}{2} e7, [e4, e8] = \frac{5}{2} e8, [e4, e9] = e9, [e4, e10] \\ = e10, [e5, e9] = 2 e6, [e5, e10] = 2 e6, [e8, e9] = 2 e7, [e8, e10] = e7, [e9, e10] = -e5 \end{aligned} \quad (41)$$

> Out := { } :for i to nops(SVF) do Out := {op(Out), EC(SVF[i])} :od: Out

$$\begin{aligned} \left\{ e25 + e32, e3 - e34, e33 + e28, e9 + e4, -e2 - e21 + e30, e31 - 2 e2 - e21, e1 - \frac{7}{2} e15 \right. \\ \left. - \frac{5}{2} e22 + 3 e29, e8 + \frac{3}{2} e15 + \frac{1}{2} e22 - 2 e29, e26, e27 \right\} \end{aligned} \quad (42)$$

> DGsetup(L) : Centralizer(convert(Out,'list'))

[ ]

(43)

> SubalgebraNormalizer(convert(Out,'list')); nops(%)

$$\begin{aligned} [-e3 + e34, e28 + e33, e25 + e32, -(2 e2) - e21 + e31, -e2 - e21 + e30, -\left(\frac{1}{7} e1\right) \\ - \left(\frac{5}{7} e8\right) - \left(\frac{4}{7} e15\right) + e29, e27, e26, -\left(\frac{4}{7} e1\right) - \left(\frac{6}{7} e8\right) + \frac{5}{7} e15 + e22, e4 \\ + e9] \end{aligned}$$

10

(44)

> Ser := Series(convert(Out,'list'), "Derived"); map(v→nops(v), Ser)

$$\begin{aligned} Ser := \left[ \left[ e3 - e34, e4 + e9, e25 + e32, e28 + e33, -e2 - e21 + e30, -(2 e2) - e21 + e31, e1 \right. \right. \\ \left. - \left(\frac{7}{2} e15\right) - \left(\frac{5}{2} e22\right) + 3 e29, e8 + \frac{3}{2} e15 + \frac{1}{2} e22 - (2 e29), e26, e27 \right], \left[ -e27, \right. \\ \left. e28 + e33, -\left(\frac{9}{2} e3\right) + \frac{9}{2} e34, -\left(\frac{7}{2} e4\right) - \left(\frac{7}{2} e9\right), -(2 e26), -(2 e25) - (2 e32), \right. \\ \left. e2 + e21 - e30, 2 e2 + e21 - e31 \right], \left[ 2 e27, \frac{9}{2} e28 + \frac{9}{2} e33, \frac{7}{2} e3 - \left(\frac{7}{2} e34\right), \right. \\ \left. -(4 e26), e25 + e32 \right], \left[ -\left(\frac{7}{2} e27\right) \right], [ ] \end{aligned}$$

[10, 8, 5, 1, 0]

(45)

dim(Stab)=10, non-Abelian, self-normalizing, derived series (10,8,5,1,0)

>

Type [1,1,1]

> with(DifferentialGeometry) :

> EQ :=  $[u_3 v_1 - \alpha \cdot (v_2 - v_3) \cdot u_1, u_4 v_1 - \alpha \cdot (v_3 - v_4) \cdot u_1] : S := solve(EQ, \{v[2], v[3]\}) :$

> OT := {coeffs(numer(simplify(subs(S, LieDerivative(VI, EQ[1])))), CF),  
coeffs(numer(simplify(subs(S, LieDerivative(VI, EQ[2])))), CF)} :

> R := solve(OT, {seq(seq((a||i)||j, i=1..6), j=1..6)}[1..35]):

> VF := subs(R, V)

$$VF := \left( a11 x1 + \frac{(\alpha + 1)^2 a14 x2}{\alpha^2} + \frac{(\alpha + 1) a14 x3}{\alpha} + a14 x4 \right) D_{x1} + a44 x2 D_{x2} \quad (46)$$

$$+ a44 x3 D_{x3} + a44 x4 D_{x4} + (a52 x2 + a55 u_{[]}) D_{u_{[]}} - ((a11 v_{[]} + 3 a44 v_{[]}$$

$$+ a55 v_{[]} - a64 x2 - a64 x3 - a64 x4) D_{v_{[]}}$$

> coe := [a11, a14, a44, a52, a55, a64] :for i to nops(coe) do SuV||i := [seq(coe[j]  
= KroneckerDelta[i, j], j=1..nops(coe))] :od:

> SVF := DGsimplify(evalDG([seq(subs(SuV||i, VF), i=1..nops(coe))]))

$$SVF := \left[ x1 D_{x1} - (v_{[]} D_{v_{[]}}), \frac{\alpha^2 x2 + x3 \alpha^2 + x4 \alpha^2 + 2 \alpha x2 + x3 \alpha + x2}{\alpha^2} D_{x1}, \quad (47)$$

$$x2 D_{x2} + x3 D_{x3} + x4 D_{x4} - (3 v_{[]} D_{v_{[]}}), x2 D_{u_{[]}}, u_{[]} D_{u_{[]}} - (v_{[]} D_{v_{[]}}), (x2$$

$$+ x3 + x4) D_{v_{[]}} \right]$$

> nops(coe); LieAlgebraData(SVF, alg)

6

$$[[e1, e2] = -e2, [e1, e6] = e6, [e2, e3] = -e2, [e3, e4] = e4, [e3, e6] = 4 e6, [e4, e5] = e4, \quad (48)$$

$$[e5, e6] = e6]$$

> Out := {} :for i to nops(SVF) do Out := {op(Out), EC(SVF[i])} :od: Out

$$\left\{ \frac{e2 (\alpha^2 + 2 \alpha + 1)}{\alpha^2} + \frac{e3 (\alpha^2 + \alpha)}{\alpha^2} + e4, e32 + e33 + e34, e8 + e15 + e22, e1, e26, \quad (49)$$

$$e29 \right\}$$

> DGsetup(L) : Centralizer(convert(Out, 'list')); nops(%)

$$\left[ - \left( \frac{\alpha + 1}{2 \alpha + 1} e1 \right) + e8 - \left( \frac{7 \alpha^2 + 7 \alpha + 2}{\alpha (2 \alpha + 1)} e14 \right) - e15 - \left( \frac{\alpha}{2 \alpha + 1} e16 \right) \right.$$

$$\left. + \frac{2 (\alpha + 1)}{\alpha} e20 + \frac{\alpha + 1}{2 \alpha + 1} e21 + e29, - \left( \frac{1}{2 \alpha + 1} e1 \right) - \left( \frac{2 \alpha^2 + 2 \alpha + 1}{\alpha (2 \alpha + 1)} e14 \right) \right]$$

$$\left[ -e15 - \left( \frac{2\alpha}{2\alpha+1} e16 \right) + \frac{\alpha+1}{\alpha} e20 + \frac{2(\alpha+1)}{2\alpha+1} e21 + e22 \right]$$

(50)

> SubalgebraNormalizer(convert(Out,'list')); nops(%)

$$\left[ e32 + e33 + e34, e29, e26, e8 + e15 + e22, - \left( \frac{2\alpha+1}{\alpha+1} e8 \right) + e14 - \left( \frac{2\alpha+1}{\alpha+1} e15 \right) - \left( \frac{\alpha}{\alpha+1} e16 \right) + e21, \frac{\alpha}{\alpha+1} e8 - \left( \frac{2\alpha+1}{\alpha+1} e14 \right) + e20, \frac{(\alpha+1)^2}{\alpha^2} e2 + \frac{\alpha+1}{\alpha} e3 + e4, e1 \right]$$

(51)

> Ser := Series(convert(Out,'list'), "Derived"); map(v→nops(v), Ser)

$$Ser := \left[ \left[ \frac{\alpha^2 + 2\alpha + 1}{\alpha^2} e2 + \frac{\alpha+1}{\alpha} e3 + e4, e8 + e15 + e22, e32 + e33 + e34, e1, e26, e29 \right], \left[ \frac{\alpha^2 + 2\alpha + 1}{\alpha^2} e2 + \frac{\alpha+1}{\alpha} e3 + e4, -(4e32) - (4e33) - (4e34), -e26 \right], [ ] \right]$$

(52)

dim(Stab)=6, non-Abelian (dim(Centr)=2); not self-normalizing (dim(Norm)=8), derived series (6,3,0)

>

Type [2,1]

> with(DifferentialGeometry) :

> EQ := [u<sub>3</sub> v<sub>1</sub> - u<sub>1</sub> v<sub>3</sub> - (v<sub>2</sub> - α·v<sub>3</sub>) v<sub>1</sub>, u<sub>4</sub> v<sub>1</sub> - u<sub>1</sub> v<sub>4</sub> - (v<sub>3</sub> - α·v<sub>4</sub>) v<sub>1</sub>] : S := solve(EQ, {v[2], v[3]}) :

> OT := {coeffs(numer(simplify(subs(S, LieDerivative(V1, EQ[1])))), CF), coeffs(numer(simplify(subs(S, LieDerivative(V1, EQ[2])))), CF)} :

> R := solve(OT, {seq(seq((a||i)||j, i=1..6), j=1..6)}[1..35]) :

> VF := subs(R, V)

$$VF := ((a44 - 4a33 - 2a55) x1 + a14 \alpha^2 x2 + a14 \alpha x3 + a14 x4) D_x1 + (-a44 + 2a33) x2 D_x2 - ((-(-2a33 \alpha + 2a44 \alpha) x2 - a33 x3) D_x3) - ((-(-a33 \alpha + a44 \alpha) x3 - a44 x4) D_x4) + (a52 x2 + a55 u_{[]} + a56 v_{[]} + a62 x3) D_u_{[]} + (- (a44 - 4a33 - 2a55) v_{[]} - (-a44 + 2a33) v_{[]} - a33 v_{[]} - a44 v_{[]} - a55 v_{[]} + a62 x2) D_v_{[]}$$

(53)

> coe := [a14, a33, a44, a52, a55, a56, a62] : for i to nops(coe) do SuV||i := [seq(coe[j] = KroneckerDelta[i, j], j=1..nops(coe))] : od:

> SVF := DGsimplify(evalDG([seq(subs(SuV||i, VF), i=1..nops(coe))]))

(54)

$$SVF := \left[ \left( \alpha^2 x_2 + \alpha x_3 + x_4 \right) D_{x1}, -(4 x1 D_{x1}) + 2 x2 D_{x2} - \left( (2 \alpha x_2 - x_3) D_{x3} \right) \right. \\ \left. - (\alpha x_3 D_{x4}) + v_{[]} D_{v[]}, x1 D_{x1} - (x2 D_{x2}) + 2 \alpha x2 D_{x3} + (\alpha x_3 + x_4) D_{x4} \right. \\ \left. - (v_{[]} D_{v[]}), x2 D_{u[]}, -(2 x1 D_{x1}) + u_{[]} D_{u[]} + v_{[]} D_{v[]}, v_{[]} D_{u[]}, x3 D_{u[]} \right. \\ \left. + x2 D_{v[]} \right] \quad (54)$$

> nops(coe); LieAlgebraData(SVF, alg)

7

$$[[e1, e2] = -4 e1, [e1, e5] = -2 e1, [e2, e4] = 2 e4, [e2, e6] = e6, [e2, e7] = -2 \alpha e4 + e7, \\ [e3, e4] = -e4, [e3, e6] = -e6, [e3, e7] = 2 \alpha e4, [e4, e5] = e4, [e5, e7] = -e7, [e6, e7] = \\ -e4] \quad (55)$$

$$\text{Out} := \{ \} : \text{for } i \text{ to } \text{nops}(SVF) \text{ do } \text{Out} := \{ \text{op}(\text{Out}), \text{EC}(SVF[i]) \} : \text{od} : \text{Out} \\ \{ -2 e1 + e29, e32 + e27, e2 \alpha^2 + e3 \alpha + e4, -2 e14 \alpha - e21 \alpha - 4 e1 + 2 e8 + e15, 2 e14 \alpha \\ + e21 \alpha + e1 - e8 + e22, e26, e30 \} \quad (56)$$

$$\text{DGsetup}(L) : \text{Centralizer}(\text{convert}(\text{Out}, 'list')) \\ [-(2 e1) + e8 + e15 - (3 \alpha^2 e20) - (3 \alpha e21) - (2 e22) + e29] \quad (57)$$

$$\text{SubalgebraNormalizer}(\text{convert}(\text{Out}, 'list')); \text{nops}(\%) \\ \left[ e27 + e32, e30, -(2 e1) + e29, e26, -(3 e1) + e8 + e15 + e22, \frac{4}{\alpha} e1 - \left( \frac{2}{\alpha} e8 \right) + 2 e14 \right. \\ \left. - \left( \frac{1}{\alpha} e15 \right) + e21, - \left( \frac{2}{\alpha^2} e1 \right) + \frac{1}{\alpha^2} e8 - \left( \frac{2}{\alpha} e14 \right) + e20, \alpha^2 e2 + \alpha e3 + e4 \right] \\ 8 \quad (58)$$

$$\text{Ser} := \text{Series}(\text{convert}(\text{Out}, 'list'), "Derived"); \text{map}(v \rightarrow \text{nops}(v), \text{Ser}) \\ \text{Ser} := [[-(2 e1) + e29, e27 + e32, \alpha^2 e2 + \alpha e3 + e4, -(4 e1) + 2 e8 - (2 \alpha e14) + e15 \\ - (\alpha e21), e1 - e8 + 2 \alpha e14 + \alpha e21 + e22, e26, e30], [e27 + e32, -(2 \alpha^2 e2) \\ - (2 \alpha e3) - (2 e4), e26, -e30], [e26], [ ]] \\ [7, 4, 1, 0] \quad (59)$$

dim(Stab)=7, non-Abelian (dim(Cetr)=1), not self-normalizing (dim(Norm)=8), derived series (7,4,1,0)

>

Type [3]

> with(DifferentialGeometry) :

> EQ := [u<sub>3</sub> - v<sub>2</sub> + v<sub>1</sub> v<sub>3</sub>, u<sub>4</sub> - v<sub>3</sub> + v<sub>1</sub> v<sub>4</sub>] : S := solve(EQ, {v[2], v[3]}) :

> OT := {coeffs(numer(simplify(subs(S, LieDerivative(V1, EQ[1])))), CF), \\ coeffs(numer(simplify(subs(S, LieDerivative(V1, EQ[2])))), CF)} :

> R := solve(OT, {seq(seq((a || i) || j, i = 1 .. 6), j = 1 .. 6)})[1 .. 35] :

> VF := subs(R, V)

(60)

$$VF := (a11 x1 - a63 x2) D\_x1 + a22 x2 D\_x2 - \left( \left( -2 a43 x2 - \left( \frac{a22}{2} - \frac{a11}{2} \right) x3 \right) D\_x3 \right) - ((a11 x4 - a43 x3) D\_x4) - ((a22 u_{[]} - a51 x1 - a52 x2 - a53 x3 - a56 v_{[]} - a63 x4) D\_u_{[]}) + \left( - \left( \frac{a22}{2} - \frac{a11}{2} \right) v_{[]} + (-a56 - a43) x1 + a53 x2 + a63 x3 \right) D\_v_{[]} \quad (60)$$

> *coe* := [*a11*, *a22*, *a43*, *a51*, *a52*, *a53*, *a56*, *a63*] :for *i* to *nops*(*coe*) do *SuV* || *i* := [*seq*(*coe*[*j*] = *KroneckerDelta*[*i*, *j*], *j* = 1 ..*nops*(*coe*))] :od:

> *SVF* := *DG*simplify(*evalDG*( [*seq*(*subs*(*SuV* || *i*, *VF*), *i* = 1 ..*nops*(*coe*))] ))

$$SVF := \left[ x1 D\_x1 - \left( \frac{x3}{2} D\_x3 \right) - (x4 D\_x4) + \frac{v_{[]}}{2} D\_v_{[]}, x2 D\_x2 + \frac{x3}{2} D\_x3 - (u_{[]} D\_u_{[]}) - \left( \frac{v_{[]}}{2} D\_v_{[]} \right), 2 x2 D\_x3 + x3 D\_x4 - (x1 D\_v_{[]}), x1 D\_u_{[]}, x2 D\_u_{[]}, x3 D\_u_{[]} + x2 D\_v_{[]}, v_{[]} D\_u_{[]} - (x1 D\_v_{[]}), -(x2 D\_x1) + x4 D\_u_{[]} + x3 D\_v_{[]} \right] \quad (61)$$

> *nops*(*coe*); *LieAlgebraData*(*SVF*, *alg*)

$$\begin{aligned} & \left[ [e1, e3] = \frac{1}{2} e3, [e1, e4] = e4, [e1, e6] = -\frac{1}{2} e6, [e1, e7] = \frac{1}{2} e7, [e1, e8] = -e8, [e2, e3] \right. \\ & = \frac{1}{2} e3, [e2, e4] = e4, [e2, e5] = 2 e5, [e2, e6] = \frac{3}{2} e6, [e2, e7] = \frac{1}{2} e7, [e2, e8] = e8, \\ & \left. [e3, e6] = 2 e5, [e3, e7] = -e4, [e3, e8] = e6, [e4, e8] = e5, [e6, e7] = e5, [e7, e8] = -e6 \right] \quad (62) \end{aligned}$$

> *Out* := {} :for *i* to *nops*(*SVF*) do *Out* := {*op*(*Out*), *EC*(*SVF*[*i*])} :od: *Out*

$$\left\{ -e31 + e30, e32 + e27, e1 - \frac{1}{2} e15 - e22, -e2 + e33 + e28, -e31 + 2 e14 + e21, e8 + \frac{1}{2} e15 - e29, e25, e26 \right\} \quad (63)$$

> *DG*setup(*L*) : *Centralizer*(*convert*(*Out*, 'list'))

$$\left[ -e2 + e28 + e33, e27 + e32, -(2 e14) - e21 + e31, -(2 e14) - e21 + e30, -e8 - \left( \frac{1}{2} e15 \right) + e29, e26, e25, -e1 + \frac{1}{2} e15 + e22 \right] \quad (64)$$

> *SubalgebraNormalizer*(*convert*(*Out*, 'list')); *nops*(%)

$$\left[ -e2 + e28 + e33, e27 + e32, -(2 e14) - e21 + e31, -(2 e14) - e21 + e30, -e8 - \left( \frac{1}{2} e15 \right) + e29, e26, e25, -e1 + \frac{1}{2} e15 + e22 \right] \quad (65)$$

> *Ser* := *Series*(*convert*(*Out*, 'list'), "Derived"); *map*(*v* → *nops*(*v*), *Ser*)

$$\begin{aligned}
Ser := & \left[ \left[ e30 - e31, e27 + e32, e1 - \left( \frac{1}{2} e15 \right) - e22, -e2 + e28 + e33, e8 + \frac{1}{2} e15 - e29, \right. \right. \\
& \left. \left. 2 e14 + e21 - e31, e25, e26 \right], \left[ e26, \frac{1}{2} e30 - \left( \frac{1}{2} e31 \right), e27 + e32, -e25, -e2 + e28 \right. \right. \\
& \left. \left. + e33, -e14 - \left( \frac{1}{2} e21 \right) + \frac{1}{2} e31 \right], \left[ \frac{1}{2} e26, \frac{1}{2} e27 + \frac{1}{2} e32, \frac{1}{4} e25 \right], [ ] \right] \\
& [8, 6, 3, 0]
\end{aligned} \tag{66}$$

dim(Stab)=8, non-Abelian, self-normalizing, derived series (8,6,3,0)

$$\begin{aligned}
& > \\
& \text{Type [1,1]} \\
& > \text{with(DifferentialGeometry) :} \\
& > EQ := [u_2 v_3 - u_3 v_2 - u_2 v_2 + u_3 v_1, u_2 v_4 - u_4 v_2 - u_2 v_3 + u_4 v_1] : S := \text{solve}(EQ, \\
& \quad \{v[2], v[3]\}) : \\
& > OT := \{coeffs(numer(simplify(subs(S, LieDerivative(V1, EQ[1])))), CF), \\
& \quad coeffs(numer(simplify(subs(S, LieDerivative(V1, EQ[2])))), CF)\} : \\
& > R := \text{solve}(OT, \{seq(seq((a||i)||j, i=1..6), j=1..6)\}[1..35]) : \\
& > VF := \text{subs}(R, V)
\end{aligned}$$

$$\begin{aligned}
VF := & \left( -\frac{a32}{2} + a22 \right) x1 D\_x1 + \left( \frac{3 a32 x1}{2} + a22 x2 \right) D\_x2 + \left( a32 x2 + \left( \frac{a32}{2} \right. \right. \\
& \left. \left. + a22 \right) x3 \right) D\_x3 + \left( \frac{a32 x3}{2} + (a32 + a22) x4 \right) D\_x4 + (a51 x1 + a55 u_{[]}) D\_u_{[]} \\
& - \left( \left( \left( -\frac{a32}{2} + a22 \right) v_{[]} + a22 v_{[]} + \left( \frac{a32}{2} + a22 \right) v_{[]} + (a32 + a22) v_{[]} + a55 v_{[]} \right. \right. \\
& \left. \left. - a63 x1 - a63 x2 - a63 x3 - a63 x4 \right) D\_v_{[]} \right)
\end{aligned} \tag{67}$$

$$\begin{aligned}
& > coe := [a22, a32, a51, a55, a63] : \text{for } i \text{ to } nops(coe) \text{ do } SuV||i := [seq(coe[j] \\
& \quad = \text{KroneckerDelta}[i, j], j=1..nops(coe))] : \text{od} : \\
& > SVF := DGsimplify(evalDG([seq(subs(SuV||i, VF), i=1..nops(coe))])) \\
SVF := & \left[ x1 D\_x1 + x2 D\_x2 + x3 D\_x3 + x4 D\_x4 - (4 v_{[]} D\_v_{[]}), -\left( \frac{x1}{2} D\_x1 \right) \right. \\
& \left. + \frac{3 x1}{2} D\_x2 + \left( x2 + \frac{x3}{2} \right) D\_x3 + \left( \frac{x3}{2} + x4 \right) D\_x4 - (v_{[]} D\_v_{[]}), x1 D\_u_{[]}, \right. \\
& \left. u_{[]} D\_u_{[]} - (v_{[]} D\_v_{[]}), (x1 + x2 + x3 + x4) D\_v_{[]} \right]
\end{aligned} \tag{68}$$

$$> nops(coe); \text{LieAlgebraData}(SVF, alg)$$

5

$$\left[ [e1, e3] = e3, [e1, e5] = 5 e5, [e2, e3] = -\frac{1}{2} e3, [e2, e5] = 2 e5, [e3, e4] = e3, [e4, e5] = e5 \right] \tag{69}$$

$$\begin{aligned}
& > Out := \{ \} : \text{for } i \text{ to } nops(SVF) \text{ do } Out := \{op(Out), EC(SVF[i])\} : \text{od} : Out \\
& \left\{ e1 + e8 + e15 + e22, e31 + e32 + e33 + e34, -\frac{1}{2} e1 + \frac{3}{2} e7 + e14 + \frac{1}{2} e15 + \frac{1}{2} e21 \right\}
\end{aligned} \tag{70}$$

$$+ e22, e25, e29 \}$$

$$\begin{aligned} &> DGsetup(L) : Centralizer(convert(Out,'list')); nops(\%) \\ &[3 e7 + e8 - (9 e13) - (4 e14) - e15 + 6 e19 + 3 e20 + e21, e1 - (9 e7) - (2 e8) \\ &\quad + 15 e13 + 4 e14 - (7 e19) - (2 e20) + e29, -(9 e7) - (3 e8) + 21 e13 + 8 e14 \\ &\quad + e15 - (11 e19) - (4 e20) + e22] \\ &\quad \quad \quad 3 \end{aligned} \quad (71)$$

$$\begin{aligned} &> SubalgebraNormalizer(convert(Out,'list')); nops(\%) \\ &[e31 + e32 + e33 + e34, e29, e25, e1 + e8 + e15 + e22, -(3 e1) + 3 e7 - (2 e8) + 2 e14 \\ &\quad - e15 + e21, 3 e1 - (6 e7) + e8 + 3 e13 - (2 e14) + e20, -e1 + 3 e7 - (3 e13) \\ &\quad + e19] \\ &\quad \quad \quad 7 \end{aligned} \quad (72)$$

$$\begin{aligned} &> Ser := Series(convert(Out,'list'), "Derived"); map(v → nops(v), Ser) \\ Ser := &\left[ \left[ e1 + e8 + e15 + e22, e31 + e32 + e33 + e34, -\left(\frac{1}{2} e1\right) + \frac{3}{2} e7 + e14 + \frac{1}{2} e15 \right. \right. \\ &\quad \left. \left. + \frac{1}{2} e21 + e22, e25, e29 \right], [-(5 e31) - (5 e32) - (5 e33) - (5 e34), -e25], [ ] \right] \\ &\quad \quad \quad [5, 2, 0] \end{aligned} \quad (73)$$

dim(Stab)=5, non-Abelian (dim(Centr)=3), not self-normalizing (dim(Norm)=7), derived series (5,2,0)

>

Type [2]

> with(DifferentialGeometry) :

$$\begin{aligned} &> EQ := [u_2 v_3 - u_3 v_2 - v_1 v_3 + v_2^2, u_2 v_4 - u_4 v_2 - v_1 v_4 + v_2 v_3] : S := solve(EQ, \{v[1], \\ &\quad v[4]\}) : \end{aligned}$$

$$\begin{aligned} &> OT := \{coeffs(numer(simplify(subs(S, LieDerivative(V1, EQ[1])))), CF), \\ &\quad coeffs(numer(simplify(subs(S, LieDerivative(V1, EQ[2])))), CF)\} : \end{aligned}$$

$$> R := solve(OT, \{seq(seq((a || i) || j, i = 1 .. 6), j = 1 .. 6)\} [1 .. 35]) :$$

$$> VF := subs(R, V)$$

$$\begin{aligned} VF := &a11 x1 D_x1 + \left( a21 x1 + \left( \frac{a44}{3} + \frac{2 a11}{3} \right) x2 \right) D_x2 + \left( \frac{2 a21 x2}{3} + \left( \frac{2 a44}{3} \right. \right. \\ &\quad \left. \left. + \frac{a11}{3} \right) x3 \right) D_x3 + \left( \frac{a21 x3}{3} + a44 x4 \right) D_x4 - \left( \left( -a51 x1 - a52 x2 - \left( -\frac{5 a44}{6} \right. \right. \right. \\ &\quad \left. \left. - \frac{7 a11}{6} \right) u_{[]} - a56 v_{[]} \right) D_u_{[]} - \left( \left( a11 v_{[]} + \left( \frac{a44}{3} + \frac{2 a11}{3} \right) v_{[]} + \left( \frac{2 a44}{3} \right. \right. \right. \\ &\quad \left. \left. + \frac{a11}{3} \right) v_{[]} + a44 v_{[]} + \left( -\frac{5 a44}{6} - \frac{7 a11}{6} \right) v_{[]} - a52 x1 \right) D_v_{[]} \end{aligned} \quad (74)$$

$$\begin{aligned} &> coe := [a11, a21, a44, a51, a52, a56] : \text{for } i \text{ to } nops(coe) \text{ do } SuV || i := [seq(coe[j] \\ &\quad = KroneckerDelta[i, j], j = 1 .. nops(coe))] : \text{od} : \end{aligned}$$

$$> SVF := DGsimplify(evalDG([seq(subs(SuV || i, VF), i = 1 .. nops(coe))]))$$

(75)

$$SVF := \left[ x1 D_{x1} + \frac{2 x2}{3} D_{x2} + \frac{x3}{3} D_{x3} - \left( \frac{7 u_{[]}}{6} D_{u_{[]}} \right) - \left( \frac{5 v_{[]}}{6} D_{v_{[]}} \right), x1 D_{x2} \right. \\ \left. + \frac{2 x2}{3} D_{x3} + \frac{x3}{3} D_{x4}, \frac{x2}{3} D_{x2} + \frac{2 x3}{3} D_{x3} + x4 D_{x4} - \left( \frac{5 u_{[]}}{6} D_{u_{[]}} \right) \right. \\ \left. - \left( \frac{7 v_{[]}}{6} D_{v_{[]}} \right), x1 D_{u_{[]}}, x2 D_{u_{[]}} + x1 D_{v_{[]}}, v_{[]} D_{u_{[]}} \right] \quad (75)$$

> nops(coe); LieAlgebraData(SVF, alg)

$$\begin{aligned} & \left[ [e1, e2] = \frac{1}{3} e2, [e1, e4] = \frac{13}{6} e4, [e1, e5] = \frac{11}{6} e5, [e1, e6] = \frac{1}{3} e6, [e2, e3] = \frac{1}{3} e2, \right. \\ & \left. [e2, e5] = e4, [e3, e4] = \frac{5}{6} e4, [e3, e5] = \frac{7}{6} e5, [e3, e6] = -\frac{1}{3} e6, [e5, e6] = e4 \right] \end{aligned} \quad (76)$$

> Out := { } :for i to nops(SVF) do Out := {op(Out), EC(SVF[i])} :od: Out

$$\left\{ e31 + e26, e7 + \frac{2}{3} e14 + \frac{1}{3} e21, e1 + \frac{2}{3} e8 + \frac{1}{3} e15 - \frac{7}{6} e29, \frac{1}{3} e8 + \frac{2}{3} e15 + e22 \right. \\ \left. - \frac{5}{6} e29, e25, e30 \right\} \quad (77)$$

> DGsetup(L) : Centralizer(convert(Out,'list'))

$$[ ] \quad (78)$$

> SubalgebraNormalizer(convert(Out,'list')); nops(%)

$$\left[ e26 + e31, e30, -\left( \frac{6}{7} e1 \right) - \left( \frac{4}{7} e8 \right) - \left( \frac{2}{7} e15 \right) + e29, e25, -\left( \frac{5}{7} e1 \right) - \left( \frac{1}{7} e8 \right) \right. \\ \left. + \frac{3}{7} e15 + e22, 3 e7 + 2 e14 + e21 \right] \quad (79)$$

> Ser := Series(convert(Out,'list'), "Derived"); map(v→nops(v), Ser)

$$Ser := \left[ \left[ e26 + e31, e7 + \frac{2}{3} e14 + \frac{1}{3} e21, e1 + \frac{2}{3} e8 + \frac{1}{3} e15 - \left( \frac{7}{6} e29 \right), \frac{1}{3} e8 \right. \right. \\ \left. \left. + \frac{2}{3} e15 + e22 - \left( \frac{5}{6} e29 \right), e25, e30 \right], \left[ e25, \frac{11}{6} e26 + \frac{11}{6} e31, \frac{1}{3} e7 + \frac{2}{9} e14 \right. \right. \\ \left. \left. + \frac{1}{9} e21, -\left( \frac{1}{3} e30 \right) \right], \left[ \frac{11}{18} e25 \right], [ ] \right] \\ [6, 4, 1, 0] \quad (80)$$

dim(Stab)=6, non-Abelian, self-normalizing, derived series (6,4,1,0)

>

Type [1]

> with(DifferentialGeometry) :

> EQ :=  $\left[ (u_2 - u_1 v_1) (v_3 - v_1 v_2) - (u_3 - u_1 v_2) (v_2 - v_1^2), (u_2 - u_1 v_1) (v_4 - v_1 v_3) \right.$   
 $\left. - (u_4 - u_1 v_3) (v_2 - v_1^2) \right] : S := \text{solve}(EQ, \{u[1], v[4]\}) :$



```

> OT := {coeffs(numer(simplify(subs(S, LieDerivative(V1, EQ[1])))), CF),
coeffs(numer(simplify(subs(S, LieDerivative(V1, EQ[2])))), CF)} :
> R := solve(OT, {seq(seq((a||i)||j, i=1..6), j=1..6)}[1..35]):
> VF := subs(R, V)

```

$$VF := \left( a_{11} x_1 - \frac{4 a_{21} v_{[]}}{3} \right) D_{x1} + (a_{21} x_1 + a_{22} x_2) D_{x2} - \left( \left( -\frac{2 a_{21} x_2}{3} - (2 a_{22} - a_{11}) x_3 \right) D_{x3} \right) - \left( \left( -\frac{a_{21} x_3}{3} - (3 a_{22} - 2 a_{11}) x_4 \right) D_{x4} \right) - \left( (5 a_{22} u_{[]} - a_{56} v_{[]}) D_{u_{[]}} \right) + \left( -a_{11} v_{[]} + 4 a_{22} v_{[]} - (2 a_{22} - a_{11}) v_{[]} - (3 a_{22} - 2 a_{11}) v_{[]} \right) D_{v_{[]}} \quad (81)$$

```

> coe := [a11, a21, a22, a56] :for i to nops(coe) do SuV||i := [seq(coe[j]=KroneckerDelta[i,
j], j=1..nops(coe))] :od:
> SVF := DGsimplify(evalDG([seq(subs(SuV||i, VF), i=1..nops(coe))]))

```

$$SVF := \left[ x_1 D_{x1} - (x_3 D_{x3}) - (2 x_4 D_{x4}) + 2 v_{[]} D_{v_{[]}}, -\left( \frac{4 v_{[]}}{3} D_{x1} \right) + x_1 D_{x2} + \frac{2 x_2}{3} D_{x3} + \frac{x_3}{3} D_{x4}, x_2 D_{x2} + 2 x_3 D_{x3} + 3 x_4 D_{x4} - (5 u_{[]} D_{u_{[]}}) - (v_{[]} D_{v_{[]}}), v_{[]} D_{u_{[]}} \right] \quad (82)$$

```

> nops(coe); LieAlgebraData(SVF, alg)

```

4

$$[[e1, e2] = e2, [e1, e4] = 2 e4, [e2, e3] = e2, [e3, e4] = 4 e4] \quad (83)$$

```

> Out := {} :for i to nops(SVF) do Out := {op(Out), EC(SVF[i])} :od: Out
{e1 - e15 - 2 e22, e7 + 2/3 e14 + 1/3 e21 - 4/3 e6, e8 + 2 e15 + 3 e22 - 5 e29, e30}

```

```

> DGsetup(L) : Centralizer(convert(Out,'list'))
[ ]

```

$$SubalgebraNormalizer(convert(Out,'list')); nops(%)$$

$$\left[ e_{30}, -\left( \frac{3}{10} e_1 \right) - \left( \frac{1}{5} e_8 \right) - \left( \frac{1}{10} e_{15} \right) + e_{29}, -\left( \frac{1}{2} e_1 \right) + \frac{1}{2} e_{15} + e_{22}, -(4 e_6) + 3 e_7 + 2 e_{14} + e_{21} \right]$$

4

(86)

```

> Ser := Series(convert(Out,'list'), "Derived"); map(v->nops(v), Ser)
Ser := [[e1 - e15 - (2 e22), - (4/3 e6) + e7 + 2/3 e14 + 1/3 e21, e8 + 2 e15 + 3 e22 - (5 e29), e30], [4/3 e6 - e7 - (2/3 e14) - (1/3 e21), -(2 e30)], [ ]]
[4, 2, 0]

```

(87)

dim(Stab)=4, non-Abelian, self-normalizing, derived series (4,2,0)

>

Type []

> with(DifferentialGeometry) :

> EQ :=  $\left[ (u_2 - u_1 v_1) (v_3 - u_2 - v_1 v_2) - (u_3 - u_1 v_2) (v_2 - u_1 - v_1^2), (u_2 - u_1 v_1) (v_4 - u_3 - v_1 v_3) - (u_4 - u_1 v_3) (v_2 - u_1 - v_1^2) \right] : S := \text{solve}(EQ, \{u[3], v[4]\}) :$

> OT := {coeffs(numer(simplify(subs(S, LieDerivative(V1, EQ[1])))), CF),  
coeffs(numer(simplify(subs(S, LieDerivative(V1, EQ[2])))), CF)} :

> R := solve(OT, {seq(seq((a || i) || j, i = 1 .. 6), j = 1 .. 6)}[1 .. 35]) :

> VF := subs(R, V)

$$VF := \left( a_{11} x_1 + \frac{3 a_{23} x_2}{4} - \frac{4 a_{21} v_{[]}}{3} \right) D_{x1} - ((a_{11} x_2 - a_{21} x_1 - a_{23} x_3) D_{x2} - \left( \left( -\frac{2 a_{21} x_2}{3} + 3 a_{11} x_3 - \frac{5 a_{23} x_4}{4} \right) D_{x3} \right) - \left( \left( -\frac{a_{21} x_3}{3} + 5 a_{11} x_4 \right) D_{x4} \right) + \left( 5 a_{11} u_{[]} + \frac{a_{23} v_{[]}}{4} \right) D_{u_{[]}} + \left( 3 a_{11} v_{[]} - \frac{a_{23} x_1}{2} + \frac{5 a_{21} u_{[]}}{3} \right) D_{v_{[]}} \quad (88)$$

> coe := [a11, a21, a23] :for i to nops(coe) do SuV || i := [seq(coe[j] = KroneckerDelta[i, j], j = 1 .. nops(coe))] :od:

> SVF := DGSimplify(evalDG([seq(subs(SuV || i, VF), i = 1 .. nops(coe))]))

$$SVF := \left[ x_1 D_{x1} - (x_2 D_{x2}) - (3 x_3 D_{x3}) - (5 x_4 D_{x4}) + 5 u_{[]} D_{u_{[]}} + 3 v_{[]} D_{v_{[]}}, - \left( \frac{4 v_{[]}}{3} D_{x1} \right) + x_1 D_{x2} + \frac{2 x_2}{3} D_{x3} + \frac{x_3}{3} D_{x4} + \frac{5 u_{[]}}{3} D_{v_{[]}}, \frac{3 x_2}{4} D_{x1} + x_3 D_{x2} + \frac{5 x_4}{4} D_{x3} + \frac{v_{[]}}{4} D_{u_{[]}} - \left( \frac{x_1}{2} D_{v_{[]}} \right) \right] \quad (89)$$

> nops(coe); LieAlgebraData(SVF, alg)

3

$$\left[ [e1, e2] = 2 e2, [e1, e3] = -2 e3, [e2, e3] = \frac{1}{12} e1 \right] \quad (90)$$

> Out := {} :for i to nops(SVF) do Out := {op(Out), EC(SVF[i])} :od: Out

$$\left\{ e1 - e8 - 3 e15 - 5 e22 + 5 e29, -\frac{1}{2} e31 + \frac{3}{4} e2 + e9 + \frac{5}{4} e16 + \frac{1}{4} e30, e7 + \frac{2}{3} e14 + \frac{1}{3} e21 + \frac{5}{3} e35 - \frac{4}{3} e6 \right\} \quad (91)$$

> DGsetup(L) : Centralizer(convert(Out, 'list'))

[]

(92)

> SubalgebraNormalizer(convert(Out, 'list')); nops(%)

$$\left[ -\left( \frac{3}{2} e2 \right) - (2 e9) - \left( \frac{5}{2} e16 \right) - \left( \frac{1}{2} e30 \right) + e31, \frac{1}{5} e1 - \left( \frac{1}{5} e8 \right) - \left( \frac{3}{5} e15 \right) - e22 \right]$$

$$+ e_{29}, -\left(\frac{4}{5} e_6\right) + \frac{3}{5} e_7 + \frac{2}{5} e_{14} + \frac{1}{5} e_{21} + e_{35} \Bigg] \quad (93)$$

> Ser := Series(convert(Out,'list'), "Derived"); map(v→nops(v), Ser)

$$\begin{aligned} Ser := & \left[ \left[ e_1 - e_8 - (3 e_{15}) - (5 e_{22}) + 5 e_{29}, -\left(\frac{4}{3} e_6\right) + e_7 + \frac{2}{3} e_{14} + \frac{1}{3} e_{21} \right. \right. \\ & + \frac{5}{3} e_{35}, \frac{3}{4} e_2 + e_9 + \frac{5}{4} e_{16} + \frac{1}{4} e_{30} - \left(\frac{1}{2} e_{31}\right) \Bigg], \left[ \frac{8}{3} e_6 - (2 e_7) - \left(\frac{4}{3} e_{14}\right) \right. \\ & - \left(\frac{2}{3} e_{21}\right) - \left(\frac{10}{3} e_{35}\right), \frac{3}{2} e_2 + 2 e_9 + \frac{5}{2} e_{16} + \frac{1}{2} e_{30} - e_{31}, -\left(\frac{1}{12} e_1\right) \\ & \left. \left. + \frac{1}{12} e_8 + \frac{1}{4} e_{15} + \frac{5}{12} e_{22} - \left(\frac{5}{12} e_{29}\right) \right] \right] \\ & [3, 3] \end{aligned} \quad (94)$$

dim(Stab)=3, non-Abelian, self-normalizing: sl(2)

>

>

>

>

> ChangeFrame(J0) :

> EQ := {v<sub>3</sub> - f(u<sub>1</sub>, u<sub>2</sub>, u<sub>3</sub>, u<sub>4</sub>, v<sub>1</sub>, v<sub>2</sub>), v<sub>4</sub> - g(u<sub>1</sub>, u<sub>2</sub>, u<sub>3</sub>, u<sub>4</sub>, v<sub>1</sub>, v<sub>2</sub>)} : sEQ := solve(EQ, {v<sub>3</sub>, v<sub>4</sub>}) :

> X1 := Prolong(evalDG(x1·D\_x1 - v[ ]·D\_v[ ]), 1) : X2 := Prolong(evalDG(x2·D\_x2 - v[ ]·D\_v[ ]), 1) : X3 := Prolong(evalDG(x3·D\_x3 - v[ ]·D\_v[ ]), 1) :  
X4 := Prolong(evalDG(x4·D\_x4 - v[ ]·D\_v[ ]), 1) : X5 := Prolong(evalDG(u[ ]·D\_u[ ] - v[ ]·D\_v[ ]), 1) :

> pdsolve({seq(seq(subs(sEQ, LieDerivative(X||i, EQ[j])), i = 1..5), j = 1..2)})

$$\left\{ \begin{aligned} f(u_1, u_2, u_3, u_4, v_1, v_2) &= \frac{-F1\left(\frac{v_2 u_1}{u_2 v_1}\right) v_1 u_3}{u_1}, g(u_1, u_2, u_3, u_4, v_1, v_2) \\ &= \frac{-F2\left(\frac{v_2 u_1}{u_2 v_1}\right) v_1 u_4}{u_1} \end{aligned} \right\} \quad (95)$$

>

II. Computation of the stabilizer for the integrable systems in 4D associated with quadratic maps P<sup>6</sup>->Gr(4,6); this computations accompany the tables of 4D systems.

> restart :

> with(DifferentialGeometry) : with(GroupActions) : with(JetCalculus) : with(Tools) :  
with(LieAlgebras) : with(LinearAlgebra) : Preferences("ShowFramePrompt",false) :

> DGsetup([x1, x2, x3, x4], [u, v], J0, 1) :

```

> V := evalDG((a11·x1 + a12·x2 + a13·x3 + a14·x4 + a15·u[ ] + a16·v[ ])·D_x1 + (a21·x1
+ a22·x2 + a23·x3 + a24·x4 + a25·u[ ] + a26·v[ ])·D_x2 + (a31·x1 + a32·x2 + a33
·x3 + a34·x4 + a35·u[ ] + a36·v[ ])·D_x3 + (a41·x1 + a42·x2 + a43·x3 + a44·x4
+ a45·u[ ] + a46·v[ ])·D_x4 + (a51·x1 + a52·x2 + a53·x3 + a54·x4 + a55·u[ ] + a56
·v[ ])·D_u[ ] + (a61·x1 + a62·x2 + a63·x3 + a64·x4 + a65·u[ ] - (a11 + a22 + a33
+ a44 + a55)·v[ ])·D_v[ ]) :
> V1 := Prolong(V, 1) :
> uv := [[u1, u2, u3, u4], [v1, v2, v3, v4]] : Cf := (i, j) → LieDerivative(V1, uv[i, j]) :
> for i to 2 do for j to 4 do (S||i)||j := subs({u1 = z11, u2 = z12, u3 = z13, u4 = w1[ ], v1 = z21,
v2 = z22, v3 = z23, v4 = w2[ ]}, Cf(i, j)) : od:od:
> DGsetup([z11, z12, z13, z21, z22, z23], [w1, w2], K, 1) :
> W := evalDG(S11·D_z11 + S12·D_z12 + S13·D_z13 + S14·D_w1[ ] + S21·D_z21 + S22
·D_z22 + S23·D_z23 + S24·D_w2[ ]) : W1 := Prolong(W, 1) :
>
> Mg := subs(m(6, 6) = -(m(1, 1) + m(2, 2) + m(3, 3) + m(4, 4) + m(5, 5)), Matrix(6,
m)) : M := [ ] : for i to 6 do for j to 6 do M := [op(M), coeff(Mg, m(i, j))] : od:od: M
:= M[1..35] :
> L := LieAlgebraData(M, Ex) : DGsetup(L) :
> CF := {u[1], u[2], u[3], u[4], v[1], v[2], v[3], v[4]} :
> var := [x1, x2, x3, x4, u[ ], v[ ]] : dvar := evalDG([dx1, dx2, dx3, dx4, du[ ], dv[ ]]) :
> EC := v → subs({E11 = e1, E12 = e2, E13 = e3, E14 = e4, E15 = e5, E16 = e6, E21 = e7, E22
= e8, E23 = e9, E24 = e10, E25 = e11, E26 = e12, E31 = e13, E32 = e14, E33 = e15, E34
= e16, E35 = e17, E36 = e18, E41 = e19, E42 = e20, E43 = e21, E44 = e22, E45 = e23, E46
= e24, E51 = e25, E52 = e26, E53 = e27, E54 = e28, E55 = e29, E56 = e30, E61 = e31, E62
= e32, E63 = e33, E64 = e34, E65 = e35, E66 = 0}, add(add((E||i||j)·diff(Hook(v,
dvar[i]), var[j]), i = 1..6), j = 1..6)) :
> EC(evalDG(u[ ]·D_u[ ] - v[ ]·D_v[ ]))

```

e29

(96)

```

> with(Physics) :
Type [linear]
> EQ := [u2 - v1, u3 + v4] : S := solve(EQ, {v[1], v[4]}) :
> OT := {coeffs(numer(simplify(subs(S, DifferentialGeometry:-LieDerivative(V1, EQ[1])))),
CF), coeffs(numer(simplify(subs(S, DifferentialGeometry:-LieDerivative(V1, EQ[2])))),
CF)} :
> R := solve(OT, {seq(seq((a||i)||j, i = 1..6), j = 1..6)}[1..35]) :
> VF := subs(R, V)
VF := -((-a22 - 2 a44 - 2 a55) x1 + a65 x2 + a23 x4) D_x1 + (a22 x2 + a23 x3
- a56 x1) D_x2 + (-a41 x2 + (2 a22 + 3 a44 + 2 a55) x3 + a56 x4) D_x3 + (a41 x1
+ a44 x4 + a65 x3) D_x4 + (a51 x1 + a54 x4 + a55 u[ ] + a56 v[ ] + a61 x2
- a64 x3) D_u[ ] - (((-a22 - 2 a44 - 2 a55) v[ ] + a22 v[ ] + (2 a22 + 3 a44
+ 2 a55) v[ ] + a44 v[ ] + a55 v[ ] - a61 x1 - a62 x2 - a63 x3 - a64 x4 - a65 u[ ])

```

(97)

$D_v[ ]]$

>  $coe := [a22, a23, a41, a44, a51, a54, a55, a56, a61, a62, a63, a64, a65] : \text{for } i \text{ to } nops(coe)$   
**do**  $SuV || i := [seq(coe[j] = KroneckerDelta[i, j], j = 1 .. nops(coe))] : \text{od}$   
>  $SVF := DGsimplify(evalDG([seq(subs(SuV || i, VF), i = 1 .. nops(coe))]))$   
 $SVF := [- (x1 D_{x1}) + x2 D_{x2} + 2 x3 D_{x3} - (2 v[ ] D_v[ ]), - (x4 D_{x1}) + x3 D_{x2},$  (98)  
 $- (x2 D_{x3}) + x1 D_{x4}, - (2 x1 D_{x1}) + 3 x3 D_{x3} + x4 D_{x4} - (2 v[ ] D_v[ ]),$   
 $x1 D_u[ ], x4 D_u[ ], - (2 x1 D_{x1}) + 2 x3 D_{x3} + u[ ] D_u[ ] - (v[ ] D_v[ ]),$   
 $- (x1 D_{x2}) + x4 D_{x3} + v[ ] D_u[ ], x2 D_u[ ] + x1 D_v[ ], x2 D_v[ ], x3 D_v[ ],$   
 $- (x3 D_u[ ]) + x4 D_v[ ], - (x2 D_{x1}) + x3 D_{x4} + u[ ] D_v[ ]]$

>  $nops(coe); LieAlgebraData(SVF, alg)$

13

$[ [e1, e2] = e2, [e1, e3] = -e3, [e1, e5] = -e5, [e1, e8] = -2 e8, [e1, e9] = e9, [e1, e10]$  (99)  
 $= 3 e10, [e1, e11] = 4 e11, [e1, e12] = 2 e12, [e1, e13] = 2 e13, [e2, e3] = e1 - e4, [e2,$   
 $e4] = -3 e2, [e2, e5] = -e6, [e2, e7] = -2 e2, [e2, e9] = -e12, [e2, e10] = e11, [e3, e4]$   
 $= 3 e3, [e3, e6] = e5, [e3, e7] = 2 e3, [e3, e11] = -e10, [e3, e12] = e9, [e4, e5] = -2 e5,$   
 $[e4, e6] = e6, [e4, e8] = -2 e8, [e4, e10] = 2 e10, [e4, e11] = 5 e11, [e4, e12] = 3 e12,$   
 $[e4, e13] = 2 e13, [e5, e7] = 3 e5, [e5, e13] = e9, [e6, e7] = e6, [e6, e13] = e12, [e7, e8]$   
 $= -2 e8, [e7, e9] = -e9, [e7, e10] = e10, [e7, e11] = 3 e11, [e7, e12] = e12, [e7, e13]$   
 $= 2 e13, [e8, e9] = -2 e5, [e8, e10] = -e9, [e8, e11] = e12, [e8, e12] = -2 e6, [e8, e13]$   
 $= -e7 + e4 - e1, [e9, e13] = 2 e10, [e12, e13] = -2 e11]$

>  $Out := \{ \} : \text{for } i \text{ to } nops(SVF) \text{ do } Out := \{op(Out), EC(SVF[i])\} : \text{od}$   $Out$   
 $\{e19 - e14, -e27 + e34, e31 + e26, e9 - e4, -2 e1 + 2 e15 + e29, -2 e1 + 3 e15 + e22, -e1$  (100)  
 $+ e8 + 2 e15, -e2 + e21 + e35, -e7 + e16 + e30, e25, e28, e32, e33\}$

>  $DGsetup(L) : Centralizer(convert(Out, 'list'))$

[ ]

(101)

>  $SubalgebraNormalizer(convert(Out, 'list')); nops(\%)$

$\left[ e26 + e31, -e7 + e16 + e30, -e1 - e8 + e29, e28, e25, -\frac{e1}{2} - \frac{3 e8}{2} + e22, -e14 + e19,$   
 $-\frac{e1}{2} + \frac{e8}{2} + e15, -e4 + e9, -e2 + e21 + e35, -e27 + e34, e33, e32 \right]$

13

(102)

>  $Ser := Series(convert(Out, 'list'), "Derived"); map(v \rightarrow nops(v), Ser)$

$Ser := [[-e4 + e9, -e14 + e19, -e27 + e34, e26 + e31, -(2 e1) + 2 e15 + e29, -(2 e1)$   
 $+ 3 e15 + e22, -e1 + e8 + 2 e15, -e2 + e21 + e35, -e7 + e16 + e30, e25, e28, e32,$   
 $e33], [-e1 - e8 + e15 + e22, -e27 + e34, -(2 e4) + 2 e9, e28, -e33, -e26 - e31, 2 e14$   
 $- (2 e19), -e25, e32, 2 e2 - (2 e21) - (2 e35), -(2 e7) + 2 e16 + 2 e30, e1 - e8$   
 $- e15 + e22 - e29], [e27 - e34, 4 e4 - (4 e9), -e28, e33, -e26 - e31, 4 e14$   
 $- (4 e19), -e25, e32, 4 e1 + 4 e8 - (4 e15) - (4 e22), -(4 e1) + 4 e8 + 4 e15$   
 $- (4 e22) + 4 e29, -(4 e2) + 4 e21 + 4 e35, -(4 e7) + 4 e16 + 4 e30]]$

$$[13, 12, 12] \quad (103)$$

$$\begin{aligned} &> Le1 := LieAlgebraData([op(Out)]) \\ Le1 := & [[e1, e2] = e6 - e7, [e1, e4] = e3, [e1, e5] = 2 e1, [e1, e6] = 3 e1, [e1, e7] = e1, [e1, e10] = e11, [e1, e12] = -e13, [e2, e3] = -e4, [e2, e5] = -2 e2, [e2, e6] = -3 e2, [e2, e7] = -e2, [e2, e11] = -e10, [e2, e13] = e12, [e3, e5] = e3, [e3, e6] = 3 e3, [e3, e7] = 2 e3, [e3, e8] = 2 e13, [e3, e9] = -2 e11, [e4, e5] = -e4, [e4, e7] = e4, [e4, e8] = -2 e12, [e4, e9] = -2 e10, [e5, e8] = -2 e8, [e5, e9] = 2 e9, [e5, e10] = 3 e10, [e5, e11] = e11, [e5, e12] = -e12, [e5, e13] = -3 e13, [e6, e8] = -2 e8, [e6, e9] = 2 e9, [e6, e10] = 2 e10, [e6, e11] = -e11, [e6, e12] = -2 e12, [e6, e13] = -5 e13, [e7, e8] = -2 e8, [e7, e9] = 2 e9, [e7, e10] = e10, [e7, e12] = -3 e12, [e7, e13] = -4 e13, [e8, e9] = -e7 + e6 - e5, [e8, e10] = e4, [e8, e11] = e3, [e9, e12] = e4, [e9, e13] = -e3] \end{aligned} \quad (104)$$

$$> DGsetup(Le1) :$$

$$> LeviDecomposition( ) \quad \left[ \left[ e3, e4, e5 - \frac{e6}{2} - \frac{e7}{2}, e10, e11, e12, e13 \right], [e1, e2, e5, e6 - e7, e8, e9] \right] \quad (105)$$

$$\begin{aligned} &> LieAlgebraData\left(\left[\frac{2}{3} e5 - \frac{1}{3} e6 - \frac{1}{3} e7, e3, e4, e10, e11, e12, e13\right]\right) \\ & [[e1, e2] = e2, [e1, e3] = e3, [e1, e4] = e4, [e1, e5] = e5, [e1, e6] = e6, [e1, e7] = e7] \end{aligned} \quad (106)$$

$$\begin{aligned} &> LieAlgebraData([e1, e2, e6 - e7, e8, e9, e5 - e6 + e7]) \\ & [[e1, e2] = e3, [e1, e3] = 2 e1, [e2, e3] = -2 e2, [e4, e5] = -e6, [e4, e6] = 2 e4, [e5, e6] = -2 e5] \end{aligned} \quad (107)$$

$$\begin{aligned} &> LieAlgebraData\left(\left[e1, e2, e6 - e7, e8, e9, e5 - e6 + e7, \frac{2}{3} e5 - \frac{1}{3} e6 - \frac{1}{3} e7, e3, e4, e10, e11, e12, e13\right]\right) \\ & [[e1, e2] = e3, [e1, e3] = 2 e1, [e1, e9] = e8, [e1, e10] = e11, [e1, e12] = -e13, [e2, e3] = -2 e2, [e2, e8] = -e9, [e2, e11] = -e10, [e2, e13] = e12, [e3, e8] = -e8, [e3, e9] = e9, [e3, e10] = e10, [e3, e11] = -e11, [e3, e12] = e12, [e3, e13] = -e13, [e4, e5] = -e6, [e4, e6] = 2 e4, [e4, e8] = -2 e13, [e4, e9] = 2 e12, [e4, e10] = e9, [e4, e11] = e8, [e5, e6] = -2 e5, [e5, e8] = 2 e11, [e5, e9] = 2 e10, [e5, e12] = e9, [e5, e13] = -e8, [e6, e10] = 2 e10, [e6, e11] = 2 e11, [e6, e12] = -2 e12, [e6, e13] = -2 e13, [e7, e8] = e8, [e7, e9] = e9, [e7, e10] = e10, [e7, e11] = e11, [e7, e12] = e12, [e7, e13] = e13] \end{aligned} \quad (108)$$

dim(Stab)=13, semi-direct product (sl2+gl2) x R6, where R6=R2⊗R3 is Abelian and gl2=sl⊕R with R being the grading element; grading: (0,1)

>

$$> DGsetup(L) :$$

Type [2nd Plebansky]

$$> EQ := [u_2 - v_1, u_3 + v_4 + u_1 v_2 - v_1 u_2] : S := solve(EQ, \{v[1], v[4]\}) :$$

$$> OT := \{coeffs(numer(simplify(subs(S, DifferentialGeometry:-LieDerivative(VI, EQ[1])))), CF), coeffs(numer(simplify(subs(S, DifferentialGeometry:-LieDerivative(VI, EQ[2])))), CF)\}$$

$CF)\} :$

$\triangleright R := \text{solve}(OT, \{\text{seq}(\text{seq}((a \parallel i) \parallel j, i = 1 \dots 6), j = 1 \dots 6)\} [1 \dots 35]) :$   
 $\triangleright VF := \text{subs}(R, V)$  (109)

$VF := (a11 x1 + a13 x3 + a14 x4 - a65 x2) D\_x1 - ((a56 x1 + a11 x2 - (-2 a52$   
 $- a14) x3 - a24 x4) D\_x2) - ((- (a44 - 2 a11) x3 - a56 x4) D\_x3) + (a44 x4$   
 $+ a65 x3) D\_x4 + (a24 x1 - a44 u[ ] + a52 x2 + a53 x3 + a54 x4 + a56 v[ ]) D\_u[ ]$   
 $+ (- (a44 - 2 a11) v[ ] + a52 x1 + a13 x2 + a63 x3 - a53 x4 + a65 u[ ]) D\_v[ ]$

$\triangleright \text{coe} := [a11, a13, a14, a24, a44, a52, a53, a54, a56, a63, a65] : \text{for } i \text{ to } \text{nops}(\text{coe}) \text{ do } \text{SuV} \parallel i$   
 $:= [\text{seq}(\text{coe}[j] = \text{KroneckerDelta}[i, j], j = 1 \dots \text{nops}(\text{coe}))] : \text{od} :$

$\triangleright SVF := \text{DGsimplify}(\text{evalDG}([\text{seq}(\text{subs}(\text{SuV} \parallel i, VF), i = 1 \dots \text{nops}(\text{coe}))]))$   
 $SVF := [x1 D\_x1 - (x2 D\_x2) - (2 x3 D\_x3) + 2 v[ ] D\_v[ ], x3 D\_x1 + x2 D\_v[ ],$  (110)  
 $x4 D\_x1 - (x3 D\_x2), x4 D\_x2 + x1 D\_u[ ], x3 D\_x3 + x4 D\_x4 - (u[ ] D\_u[ ])$   
 $- (v[ ] D\_v[ ]), - (2 x3 D\_x2) + x2 D\_u[ ] + x1 D\_v[ ], x3 D\_u[ ] - (x4 D\_v[ ]),$   
 $x4 D\_u[ ], - (x1 D\_x2) + x4 D\_x3 + v[ ] D\_u[ ], x3 D\_v[ ], - (x2 D\_x1) + x3 D\_x4$   
 $+ u[ ] D\_v[ ]]$

$\triangleright \text{nops}(\text{coe}); \text{LieAlgebraData}(SVF, \text{alg})$

11

$[ [e1, e2] = -3 e2, [e1, e3] = -e3, [e1, e4] = e4, [e1, e6] = -e6, [e1, e7] = -2 e7, [e1, e9]$  (111)  
 $= 2 e9, [e1, e10] = -4 e10, [e1, e11] = -2 e11, [e2, e3] = e10, [e2, e4] = e7, [e2, e5] =$   
 $-e2, [e2, e6] = 3 e10, [e2, e9] = e6 - e3, [e3, e4] = e8, [e3, e5] = -e3, [e3, e6] = -e7,$   
 $[e4, e5] = -e4, [e4, e6] = e8, [e4, e11] = e6 - e3, [e5, e6] = e6, [e5, e7] = 2 e7, [e5, e8]$   
 $= 2 e8, [e5, e10] = 2 e10, [e6, e9] = 2 e4, [e6, e11] = 2 e2, [e7, e9] = -2 e8, [e7, e11]$   
 $= 2 e10, [e8, e11] = -e7, [e9, e10] = -e7, [e9, e11] = e1 + e5]$

$\triangleright \text{Out} := \{ \} : \text{for } i \text{ to } \text{nops}(SVF) \text{ do } \text{Out} := \{ \text{op}(\text{Out}), \text{EC}(SVF[i]) \} : \text{od} : \text{Out}$   
 $\{e25 + e10, e27 - e34, e32 + e3, -e9 + e4, e1 - e8 - 2 e15, e15 + e22 - e29, -e2 + e21$  (112)  
 $+ e35, e31 + e26 - 2 e9, -e7 + e16 + e30, e28, e33\}$

$\triangleright \text{DGsetup}(L) : \text{Centralizer}(\text{convert}(\text{Out}, 'list'))$  (113)  
 $[ ]$

$\triangleright \text{SubalgebraNormalizer}(\text{convert}(\text{Out}, 'list')); \text{nops}(\%)$   
 $\left[ e28, e10 + e25, -\frac{e1}{2} + \frac{e8}{2} + e15, -e4 + e9, -e2 + e21 + e35, -e27 + e34, e33, e3 \right.$   
 $\left. + e32, - (2 e4) + e26 + e31, -e7 + e16 + e30, -\frac{e1}{2} + \frac{e8}{2} - e22 + e29 \right]$

11

(114)

$\triangleright \text{Ser} := \text{Series}(\text{convert}(\text{Out}, 'list'), "Derived"); \text{map}(v \rightarrow \text{nops}(v), \text{Ser})$   
 $\text{Ser} := [[e4 - e9, e10 + e25, e27 - e34, e3 + e32, e1 - e8 - (2 e15), -e2 + e21 + e35, -e7$   
 $+ e16 + e30, e15 + e22 - e29, - (2 e9) + e26 + e31, e28, e33], [-e28, e33, -e4 + e9,$   
 $e27 - e34, e10 + e25, e4 + e9 - e26 - e31, - (3 e3) - (3 e32), - (2 e2) + 2 e21$   
 $+ 2 e35, 2 e7 - (2 e16) - (2 e30), e1 - e8 - e15 + e22 - e29], [- (2 e27) + 2 e34,$

$$\begin{aligned}
& - (2 e28), - (2 e33), 2 e4 + 2 e9 - (2 e26) - (2 e31), 2 e10 + 2 e25, 4 e3 + 4 e32, \\
& - (4 e1) + 4 e8 + 4 e15 - (4 e22) + 4 e29, 4 e2 - (4 e21) - (4 e35), 4 e7 - (4 e16) \\
& - (4 e30)], [- (16 e33), 16 e28, 8 e27 - (8 e34), - (16 e3) - (16 e32), - (16 e10) \\
& - (16 e25), - (8 e4) - (8 e9) + 8 e26 + 8 e31, - (32 e2) + 32 e21 + 32 e35, 32 e7 \\
& - (32 e16) - (32 e30), 16 e1 - (16 e8) - (16 e15) + 16 e22 - (16 e29)] \\
& [11, 10, 9, 9]
\end{aligned} \tag{115}$$

$$\begin{aligned}
& > Le1 := LieAlgebraData([op(Out)]) \\
Le1 := & [[e1, e2] = -e10, [e1, e4] = e11, [e1, e5] = -e1, [e1, e8] = e1, [e1, e9] = e3, [e2, e4] \\
& = e3, [e2, e5] = e2, [e2, e6] = e1 - e9, [e2, e8] = e2, [e2, e9] = -e10, [e3, e5] = -2 e3, \\
& [e3, e6] = -2 e11, [e3, e7] = 2 e10, [e3, e8] = 2 e3, [e4, e5] = -3 e4, [e4, e7] = e1 - e9, \\
& [e4, e8] = e4, [e4, e9] = -3 e11, [e5, e6] = 2 e6, [e5, e7] = -2 e7, [e5, e9] = e9, [e5, e11] \\
& = 4 e11, [e6, e7] = e5 + e8, [e6, e9] = 2 e4, [e6, e10] = -e3, [e7, e9] = 2 e2, [e7, e11] \\
& = e3, [e8, e9] = -e9, [e8, e10] = -2 e10, [e8, e11] = -2 e11]
\end{aligned} \tag{116}$$

$$\begin{aligned}
& > DGsetup(Le1) : \\
& > LeviDecomposition( ) \\
& [[e1, e2, e3, e4, e8, e9, e10, e11], [e5 + e8, e6, e7]]
\end{aligned} \tag{117}$$

$$\begin{aligned}
& > LieAlgebraData\left(\left[-e8, e1, e2, \frac{1}{2} e9 - \frac{1}{2} e1, \frac{1}{2} e4, -e10, \frac{1}{2} e3, \frac{1}{2} e11\right]\right) \\
& [[e1, e2] = e2, [e1, e3] = e3, [e1, e4] = e4, [e1, e5] = e5, [e1, e6] = 2 e6, [e1, e7] = 2 e7, [e1, \\
& e8] = 2 e8, [e2, e3] = e6, [e2, e4] = e7, [e2, e5] = e8, [e3, e4] = e6, [e3, e5] = e7, [e4, e5] \\
& = e8]
\end{aligned} \tag{118}$$

$$\begin{aligned}
& > LieAlgebraData([e7, -e6, e5 + e8]) \\
& [[e1, e2] = e3, [e1, e3] = 2 e1, [e2, e3] = -2 e2]
\end{aligned} \tag{119}$$

$$\begin{aligned}
& > LieAlgebraData\left(\left[e7, -e6, e5 + e8, -e8, e1, e2, \frac{1}{2} e9 - \frac{1}{2} e1, \frac{1}{2} e4, -e10, \frac{1}{2} e3, \frac{1}{2} e11\right]\right) \\
& [[e1, e2] = e3, [e1, e3] = 2 e1, [e1, e7] = e6, [e1, e8] = e7, [e1, e10] = e9, [e1, e11] = e10, \\
& [e2, e3] = -2 e2, [e2, e6] = -2 e7, [e2, e7] = -2 e8, [e2, e9] = -2 e10, [e2, e10] = \\
& -2 e11, [e3, e6] = -2 e6, [e3, e8] = 2 e8, [e3, e9] = -2 e9, [e3, e11] = 2 e11, [e4, e5] \\
& = e5, [e4, e6] = e6, [e4, e7] = e7, [e4, e8] = e8, [e4, e9] = 2 e9, [e4, e10] = 2 e10, [e4, \\
& e11] = 2 e11, [e5, e6] = e9, [e5, e7] = e10, [e5, e8] = e11, [e6, e7] = e9, [e6, e8] = e10, \\
& [e7, e8] = e11]
\end{aligned} \tag{120}$$

dim(Stab)=11, semi-direct product (gl2) x R7, where R7=R1⊕R3a⊕R3b, [R1,R3a]=Rb iso, [R3a,R3a]=R3b is the sl2 bracket, and gl2=sl⊕R with R being the grading element, grading (0,1,2); the derived series (11,10,9)

$$\begin{aligned}
& > \\
& > DGsetup(L) : \\
& \text{Type [1nd Plebansky]} \\
& > EQ := [u_2 - v_1, u_3 v_4 - v_3 u_4 - 1] : S := solve(EQ, \{v[1], v[4]\}) : \\
& > OT := \{coeffs(numer(simplify(subs(S, DifferentialGeometry:-LieDerivative(V1, EQ[1])))), \\
& CF), coeffs(numer(simplify(subs(S, DifferentialGeometry:-LieDerivative(V1, EQ[2])))),
\end{aligned}$$



$CF)\}$ :

$\triangleright R := \text{solve}(OT, \{\text{seq}(\text{seq}((a \parallel i) \parallel j, i = 1 \dots 6), j = 1 \dots 6)\} [1 \dots 35])$ :

$\triangleright VF := \text{subs}(R, V)$

$$VF := (a11 x1 + a12 x2) D\_x1 - ((-a21 x1 - (-2 a44 - 2 a33 - a11) x2) D\_x2) \quad (121)$$

$$+ (a33 x3 + a34 x4) D\_x3 + (a43 x3 + a44 x4) D\_x4 - \left( \left( -a51 x1 - a52 x2 - \left( -\frac{a44}{2} - \frac{a33}{2} - a11 \right) u[ ] + a21 v[ ] \right) D\_u[ ] \right) + \left( -a11 v[ ] - (-2 a44 - 2 a33 - a11) v[ ] - a33 v[ ] - a44 v[ ] - \left( -\frac{a44}{2} - \frac{a33}{2} - a11 \right) v[ ] + a52 x1 + a62 x2 - a12 u[ ] \right) D\_v[ ]$$

$\triangleright \text{coe} := [a11, a12, a21, a33, a34, a43, a44, a51, a52, a62]$  **for**  $i$  **to**  $\text{nops}(\text{coe})$  **do**  $\text{SuV} \parallel i$   
 $\quad := [\text{seq}(\text{coe}[j] = \text{KroneckerDelta}[i, j], j = 1 \dots \text{nops}(\text{coe}))]$  **od**:

$\triangleright SVF := \text{DGsimplify}(\text{evalDG}([\text{seq}(\text{subs}(\text{SuV} \parallel i, VF), i = 1 \dots \text{nops}(\text{coe}))]))$

$$SVF := \left[ x1 D\_x1 - (x2 D\_x2) - (u[ ] D\_u[ ]) + v[ ] D\_v[ ], x2 D\_x1 - (u[ ] D\_v[ ]), \quad (122)$$

$$x1 D\_x2 - (v[ ] D\_u[ ]), -(2 x2 D\_x2) + x3 D\_x3 - \frac{u[ ] D\_u[ ]}{2} + \frac{3 v[ ] D\_v[ ]}{2},$$

$$x4 D\_x3, x3 D\_x4, -(2 x2 D\_x2) + x4 D\_x4 - \frac{u[ ] D\_u[ ]}{2} + \frac{3 v[ ] D\_v[ ]}{2}, x1 D\_u[ ],$$

$$x2 D\_u[ ] + x1 D\_v[ ], x2 D\_v[ ] \right]$$

$\triangleright \text{nops}(\text{coe}); \text{LieAlgebraData}(SVF, \text{alg})$

10

$$\left[ [e1, e2] = -2 e2, [e1, e3] = 2 e3, [e1, e8] = 2 e8, [e1, e10] = -2 e10, [e2, e3] = -e1, [e2, e4] \quad (123)$$

$$= 2 e2, [e2, e7] = 2 e2, [e2, e8] = e9, [e2, e9] = 2 e10, [e3, e4] = -2 e3, [e3, e7] = -2 e3,$$

$$[e3, e9] = 2 e8, [e3, e10] = e9, [e4, e5] = -e5, [e4, e6] = e6, [e4, e8] = \frac{1}{2} e8, [e4, e9] =$$

$$-\frac{3}{2} e9, [e4, e10] = -\frac{7}{2} e10, [e5, e6] = e7 - e4, [e5, e7] = -e5, [e6, e7] = e6, [e7, e8]$$

$$= \frac{1}{2} e8, [e7, e9] = -\frac{3}{2} e9, [e7, e10] = -\frac{7}{2} e10 \right]$$

$\triangleright \text{Out} := \{ \} \text{for } i \text{ to } \text{nops}(SVF) \text{ do } \text{Out} := \{ \text{op}(\text{Out}), \text{EC}(SVF[i]) \} \text{od: Out}$

$$\left\{ e2 - e35, e31 + e26, e7 - e30, e1 - e8 - e29, -2 e8 + e15 - \frac{1}{2} e29, -2 e8 + e22 \quad (124)$$

$$- \frac{1}{2} e29, e16, e21, e25, e32 \right\}$$

$$\begin{aligned} &> DGsetup(L) : Centralizer(convert(Out,'list')) \\ &\quad [e1 + e8 - (2\ e15) - (2\ e22) + e29] \end{aligned} \quad (125)$$

$$\begin{aligned} &> Nout := SubalgebraNormalizer(convert(Out,'list')); nops(%) \\ Nout := &\left[ -e2 + e35, e32, e26 + e31, -e7 + e30, -e1 + e29, e25, -\frac{e1}{2} + e22, e21, e16, -\frac{e1}{2} \right. \\ &\quad \left. + e15, e8 \right] \end{aligned} \quad (126)$$

$$\begin{aligned} &> Ser := Series(convert(Out,'list'), "Derived"); map(v→nops(v), Ser) \\ Ser := &\left[ \left[ e2 - e35, e7 - e30, e26 + e31, e1 - e8 - e29, -(2\ e8) + e15 - \frac{e29}{2}, -(2\ e8) \right. \right. \\ &\quad \left. + e22 - \frac{e29}{2}, e16, e21, e25, e32 \right], [e1 - e8 - e29, -(2\ e32), -(2\ e2) + 2\ e35, -e26 \\ &\quad - e31, -(2\ e25), 2\ e7 - (2\ e30), e16, -e21, e15 - e22], [-(4\ e32), -(4\ e2) + 4\ e35, \\ &\quad 4\ e25, -(4\ e7) + 4\ e30, -(4\ e26) - (4\ e31), -(4\ e1) + 4\ e8 + 4\ e29, -e15 + e22, \\ &\quad -(2\ e16), -(2\ e21)] \end{aligned} \quad (127)$$

$$\begin{aligned} &> Le1 := LieAlgebraData([op(Out)]) \\ Le1 := &\left[ [e1, e2] = e4, [e1, e3] = -2\ e10, [e1, e4] = -2\ e1, [e1, e5] = -2\ e1, [e1, e6] = -2\ e1, \right. \\ &\quad [e1, e9] = -e3, [e2, e3] = -2\ e9, [e2, e4] = 2\ e2, [e2, e5] = 2\ e2, [e2, e6] = 2\ e2, [e2, e10] \\ &\quad = -e3, [e3, e5] = -\frac{3}{2}\ e3, [e3, e6] = -\frac{3}{2}\ e3, [e4, e9] = -2\ e9, [e4, e10] = 2\ e10, [e5, e7] \\ &\quad = e7, [e5, e8] = -e8, [e5, e9] = -\frac{1}{2}\ e9, [e5, e10] = \frac{7}{2}\ e10, [e6, e7] = -e7, [e6, e8] \\ &\quad \left. = e8, [e6, e9] = -\frac{1}{2}\ e9, [e6, e10] = \frac{7}{2}\ e10, [e7, e8] = e5 - e6 \right] \end{aligned} \quad (128)$$

$$\begin{aligned} &> DGsetup(Le1) : \\ &> LeviDecomposition( ) \\ &\quad \left[ \left[ e3, e4 - \frac{e5}{2} - \frac{e6}{2}, e9, e10 \right], [e1, e2, e4, e5 - e6, e7, e8] \right] \end{aligned} \quad (129)$$

$$\begin{aligned} &> LieAlgebraData\left(\left[ -\frac{2}{3}\ e4 + \frac{1}{3}\ e5 + \frac{1}{3}\ e6, e9, e3, e10 \right]\right) \\ &\quad [ [e1, e2] = e2, [e1, e3] = e3, [e1, e4] = e4 ] \end{aligned} \quad (130)$$

$$\begin{aligned} &> LieAlgebraData([e2, -e1, e4, e8, -e7, e5 - e6]) \\ &\quad [ [e1, e2] = e3, [e1, e3] = 2\ e1, [e2, e3] = -2\ e2, [e4, e5] = e6, [e4, e6] = 2\ e4, [e5, e6] = \\ &\quad -2\ e5 ] \end{aligned} \quad (131)$$

$$\begin{aligned} &> LieAlgebraData\left(\left[ e2, -e1, e4, e8, -e7, e5 - e6, -\frac{2}{3}\ e4 + \frac{1}{3}\ e5 + \frac{1}{3}\ e6, e9, e3, e10 \right]\right) \end{aligned} \quad (132)$$

$$[[e1, e2] = e3, [e1, e3] = 2 e1, [e1, e9] = -2 e8, [e1, e10] = -e9, [e2, e3] = -2 e2, [e2, e8] = e9, [e2, e9] = 2 e10, [e3, e8] = -2 e8, [e3, e10] = 2 e10, [e4, e5] = e6, [e4, e6] = 2 e4, [e5, e6] = -2 e5, [e7, e8] = e8, [e7, e9] = e9, [e7, e10] = e10] \quad (132)$$

> Le2 := LieAlgebraData([op(Nout)])

$$Le2 := \left[ [e1, e3] = 2 e2, [e1, e4] = -e11 - e5, [e1, e5] = e1, [e1, e6] = e3, [e1, e7] = \frac{1}{2} e1, [e1, e10] = \frac{1}{2} e1, [e1, e11] = e1, [e2, e4] = -e3, [e2, e7] = \frac{1}{2} e2, [e2, e10] = \frac{1}{2} e2, [e2, e11] = 2 e2, [e3, e4] = -2 e6, [e3, e5] = -e3, [e3, e11] = e3, [e4, e5] = -e4, [e4, e7] = -\frac{1}{2} e4, [e4, e10] = -\frac{1}{2} e4, [e4, e11] = -e4, [e5, e6] = 2 e6, [e6, e7] = -\frac{1}{2} e6, [e6, e10] = -\frac{1}{2} e6, [e7, e8] = e8, [e7, e9] = -e9, [e8, e9] = -e10 + e7, [e8, e10] = e8, [e9, e10] = -e9 \right] \quad (133)$$

> DGsetup(Le2) :

$$LeviDecomposition([e2, e3, e5 - e11, e6, e7 + e10 - e11], [e1, e4, e5 + e11, e7 - e10, e8, e9]) \quad (134)$$

$$LieAlgebraData([e7 + e10 - e11, e6, e2, e3, e5 - e11 - 2 \cdot (e7 + e10 - e11)], [[e1, e2] = e2, [e1, e3] = e3, [e1, e4] = e4]) \quad (135)$$

$$Centralizer([e1, e4, e5 + e1, e7 - e10, e8, e9]) [-e5 + e11, -e5 + e7 + e10] \quad (136)$$

dim(Stab)=10, semi-direct product (sl2+gl2) x R3, R3 is the standard irep of gl2=sl2+R with the grading element R for grading (0,1) and the first sl2 acting trivially;  
derived series (10,9) and the normalizer is (gl2+gl2) x R3

>

> DGsetup(L) :

Type [Husain]

$$EQ := [u_2 - v_1, u_1 + v_2 + u_3 v_4 - v_3 u_4] : S := solve(EQ, \{v[1], v[4]\}) :$$

$$OT := \{coeffs(numer(simplify(subs(S, DifferentialGeometry:-LieDerivative(V1, EQ[1])))), CF), coeffs(numer(simplify(subs(S, DifferentialGeometry:-LieDerivative(V1, EQ[2])))), CF)\} :$$

$$R := solve(OT, \{seq(seq((a||i)||j, i=1..6), j=1..6)\}[1..35]) :$$

$$VF := subs(R, V)$$

$$VF := (a15 u[ ] + a16 v[ ] - a21 x2 + a22 x1) D_x1 - ((a15 v[ ] - a16 u[ ] - a21 x1 - a22 x2) D_x2) + (a33 x3 + a34 x4) D_x3 - ((a33 x4 - a43 x3) D_x4) - ((a21 v[ ] + a22 u[ ] - a51 x1 - a52 x2) D_u[ ]) + (a21 u[ ] - a22 v[ ] - a51 x2 + a52 x1) D_v[ ] \quad (137)$$

$$coe := [a15, a16, a21, a22, a33, a34, a43, a51, a52] : \text{for } i \text{ to } nops(coe) \text{ do } SuV || i := [seq(coe[j] = KroneckerDelta[i, j], j = 1..nops(coe))] : \text{od} :$$

$$\begin{aligned}
&> SVF := DGsimplify(evalDG([seq(subs(SuV||i, VF), i = 1..nops(coe))])) \\
SVF &:= [u[ ] D_x1 - (v[ ] D_x2), v[ ] D_x1 + u[ ] D_x2, -(x2 D_x1) + x1 D_x2 \\
&\quad - (v[ ] D_u[ ]) + u[ ] D_v[ ], x1 D_x1 + x2 D_x2 - (u[ ] D_u[ ]) - (v[ ] D_v[ ]), \\
&\quad x3 D_x3 - (x4 D_x4), x4 D_x3, x3 D_x4, x1 D_u[ ] - (x2 D_v[ ]), x2 D_u[ ] \\
&\quad + x1 D_v[ ]]
\end{aligned} \tag{138}$$

$$\begin{aligned}
&> nops(coe); LieAlgebraData(SVF, alg) \\
&\quad 9 \\
&[[e1, e3] = 2 e2, [e1, e4] = 2 e1, [e1, e8] = -e4, [e1, e9] = e3, [e2, e3] = -2 e1, [e2, e4] \\
&\quad = 2 e2, [e2, e8] = -e3, [e2, e9] = -e4, [e3, e8] = -2 e9, [e3, e9] = 2 e8, [e4, e8] = 2 e8, \\
&\quad [e4, e9] = 2 e9, [e5, e6] = -2 e6, [e5, e7] = 2 e7, [e6, e7] = -e5]
\end{aligned} \tag{139}$$

$$\begin{aligned}
&> Out := \{ \} : \text{for } i \text{ to } nops(SVF) \text{ do } Out := \{op(Out), EC(SVF[i])\} : \text{od: } Out \\
&\{e11 + e6, e15 - e22, e25 - e32, e31 + e26, e5 - e12, e1 + e8 - e29, e7 - e2 + e35 - e30, \\
&\quad e16, e21\}
\end{aligned} \tag{140}$$

$$\begin{aligned}
&> DGsetup(L) : Centralizer(convert(Out, 'list')) \\
&\quad [e2 - e7 - e30 + e35, e1 + e8 - (2 e15) - (2 e22) + e29]
\end{aligned} \tag{141}$$

$$\begin{aligned}
&> Nout := SubalgebraNormalizer(convert(Out, 'list')); nops(%) \\
Nout &:= \left[ -e30 + e35, -e25 + e32, e26 + e31, -e1 - e8 + e29, -\frac{e1}{2} - \frac{e8}{2} + e22, e21, \right. \\
&\quad \left. e16, -\frac{e1}{2} - \frac{e8}{2} + e15, -e5 + e12, e6 + e11, -e2 + e7 \right] \\
&\quad 11
\end{aligned} \tag{142}$$

$$\begin{aligned}
&> Ser := Series(convert(Out, 'list'), "Derived"); map(v → nops(v), Ser) \\
Ser &:= [[e5 - e12, e6 + e11, e15 - e22, e25 - e32, e26 + e31, e1 + e8 - e29, -e2 + e7 \\
&\quad - e30 + e35, e16, e21], [e1 + e8 - e29, e2 - e7 + e30 - e35, -(2 e5) + 2 e12, -(2 e6) \\
&\quad - (2 e11), 2 e16, -(2 e21), 2 e25 - (2 e32), -(2 e26) - (2 e31), e15 - e22]] \\
&\quad [9, 9]
\end{aligned} \tag{143}$$

$$\begin{aligned}
&> Le1 := LieAlgebraData(convert(Out, 'list')) \\
Le1 &:= [[e1, e4] = e6, [e1, e5] = -e7, [e1, e6] = -2 e1, [e1, e7] = -2 e2, [e2, e4] = e7, [e2, \\
&\quad e5] = e6, [e2, e6] = -2 e2, [e2, e7] = 2 e1, [e3, e8] = 2 e8, [e3, e9] = -2 e9, [e4, e6] \\
&\quad = 2 e4, [e4, e7] = -2 e5, [e5, e6] = 2 e5, [e5, e7] = 2 e4, [e8, e9] = e3]
\end{aligned} \tag{144}$$

$$\begin{aligned}
&> DGsetup(Le1) \\
&\quad Lie algebra: L2
\end{aligned} \tag{145}$$

$$\begin{aligned}
&> LeviDecomposition( ) \\
&\quad [[ ], [e1, e2, e3, e4, e5, e6, e7, e8, e9]]
\end{aligned} \tag{146}$$

$$\begin{aligned}
&> Query("Semisimple") \\
&\quad true
\end{aligned} \tag{147}$$

$$\begin{aligned}
&> LieAlgebraData([e4, -e1, e6, e9, -e8, e3]) \\
&[[e1, e2] = e3, [e1, e3] = 2 e1, [e2, e3] = -2 e2, [e4, e5] = e6, [e4, e6] = 2 e4, [e5, e6] = \\
&\quad -2 e5]
\end{aligned} \tag{148}$$

$$> \text{Centralizer}([e4, -e1, e6, e9, -e8, e3]) \quad [ ] \quad (149)$$

$$> \text{Centralizer}([e3, e8, e9]) \quad [e7, e6, e5, e4, e2, e1] \quad (150)$$

$$> \text{Centralizer}([e1, e4, e6]) \quad [e9, e8, e3] \quad (151)$$

$$> \text{LieAlgebraData}([e4, -e1, e6, e5, e2, -e7]) \\ [[e1, e2] = e3, [e1, e3] = 2 e1, [e1, e5] = e6, [e1, e6] = 2 e4, [e2, e3] = -2 e2, [e2, e4] = -e6, [e2, e6] = -2 e5, [e3, e4] = -2 e4, [e3, e5] = 2 e5, [e4, e5] = -e3, [e4, e6] = -2 e1, [e5, e6] = 2 e2] \quad (152)$$

$$> \text{LieAlgebraData}([e4, -e1, e6, I e5, I e2, -I e7]) \\ [[e1, e2] = e3, [e1, e3] = 2 e1, [e1, e5] = e6, [e1, e6] = 2 e4, [e2, e3] = -2 e2, [e2, e4] = -e6, [e2, e6] = -2 e5, [e3, e4] = -2 e4, [e3, e5] = 2 e5, [e4, e5] = e3, [e4, e6] = 2 e1, [e5, e6] = -2 e2] \quad (153)$$

$$> \text{Centralizer}([e4 + I e5, -e1 + I e2, e6 - I e7]) \quad [e9, e8, -(I e6) + e7, I e4 + e5, e3, -(I e1) + e2] \quad (154)$$

$$> \text{Centralizer}([e4 - I e5, -e1 - I e2, e6 + I e7]) \quad [e9, e8, I e6 + e7, -(I e4) + e5, e3, I e1 + e2] \quad (155)$$

$$> \text{LieAlgebraData}\left(\left[\frac{1}{2} e4 - \frac{I}{2} e5, -\frac{1}{2} e1 - \frac{I}{2} e2, \frac{1}{2} e6 + \frac{I}{2} e7, \frac{1}{2} e4 + \frac{I}{2} e5, -\frac{1}{2} e1 + \frac{I}{2} e2, \frac{1}{2} e6 - \frac{I}{2} e7\right]\right) \\ [[e1, e2] = e3, [e1, e3] = 2 e1, [e2, e3] = -2 e2, [e4, e5] = e6, [e4, e6] = 2 e4, [e5, e6] = -2 e5] \quad (156)$$

$$> \text{Le2} := \text{LieAlgebraData}([op(Nout)]) \\ \text{Le2} := \left[ [e1, e2] = -e3, [e1, e3] = e2, [e1, e9] = -e10, [e1, e10] = e9, [e2, e4] = -2 e2, [e2, e5] = -\frac{1}{2} e2, [e2, e8] = -\frac{1}{2} e2, [e2, e9] = e4, [e2, e10] = e1 + e11, [e2, e11] = e3, [e3, e4] = -2 e3, [e3, e5] = -\frac{1}{2} e3, [e3, e8] = -\frac{1}{2} e3, [e3, e9] = -e11 - e1, [e3, e10] = e4, [e3, e11] = -e2, [e4, e9] = -2 e9, [e4, e10] = -2 e10, [e5, e6] = e6, [e5, e7] = -e7, [e5, e9] = -\frac{1}{2} e9, [e5, e10] = -\frac{1}{2} e10, [e6, e7] = e5 - e8, [e6, e8] = e6, [e7, e8] = -e7, [e8, e9] = -\frac{1}{2} e9, [e8, e10] = -\frac{1}{2} e10, [e9, e11] = e10, [e10, e11] = -e9 \right] \quad (157)$$

$$> \text{DGsetup}(\text{Le2}) \quad \text{Lie algebra: L3} \quad (158)$$

$$> \text{LeviDecomposition}() \quad (159)$$

$$\begin{bmatrix} [e1 - e11, e4 - (2 e5) - (2 e8)], [e1 + e11, e2, e3, e4, e5 - e8, e6, e7, e9, e10] \end{bmatrix} \quad (159)$$

$$\begin{bmatrix} > LieAlgebraData([e1 - e11, e4 - 2 e5 - 2 e8]) \end{bmatrix} \quad (160)$$

$$\begin{bmatrix} > Centralizer([e1 + e11, e2, e3, e4, e5 - e8, e6, e7, e9, e10]) \end{bmatrix} \quad (161)$$

$$\begin{bmatrix} [-e1 + e11, -\frac{e4}{2} + e5 + e8] \end{bmatrix}$$

$$\begin{bmatrix} \dim(\text{Stab})=9, \text{ semi-simple: } \mathfrak{sl}_2 \oplus \mathfrak{sl}(2, \mathbb{C}); \text{ normalizer is } \mathfrak{s}[\mathfrak{gl}_2 \oplus \mathfrak{gl}(2, \mathbb{C})] = \mathfrak{sl}_2 \oplus \mathfrak{gl}(2, \mathbb{C}) \end{bmatrix}$$

$$\begin{bmatrix} > \end{bmatrix}$$
