# Supplementary material for: Integrable systems in 4D associated with sixfolds in Gr(4,6)
Source: arXiv:1705.06999 ancillary file (2017-05-18)
Supplement: Supplementary file 8 [file DFKN-2017-Weyl_tensor_selfduality.pdf]

This notebook accompanies the paper B.Doubrov, E.Ferapontov, B.Kruglikov, V.Novikov "Integrable systems in 4D associated with sixfolds in Gr(4,6)".

We compute the Weyl tensor of the conformal structure corresponding to the 2x2 system:  $u=f[ux,uy,uz,vx,vy,vz]$ ,  $v=g[ux,uy,uz,vx,vy,vz]$  and check that its self-duality (with a proper change of orientation or equivalently the density =square root of the determinant) is equivalent to the integrability constraints. In fact, we check that half-vanishing of the Weyl tensor, i.e.  $W[-]=0$  or  $W[+]=0$ , corresponds to one of the branches of the space of integrable 2x2 systems: Monge-Ampere or general linear degenerate.

```
u = U[x, y, z, t];
```

```
v = V[x, y, z, t];
```

```
ux = D[u, x];
```

```
uy = D[u, y];
```

```
uz = D[u, z];
```

```
vx = D[v, x];
```

```
vy = D[v, y];
```

```
vz = D[v, z];
```

```
S1 = {f1 → D[f[ux, uy, uz, vx, vy, vz], ux],
      f2 → D[f[ux, uy, uz, vx, vy, vz], uy], f3 → D[f[ux, uy, uz, vx, vy, vz], uz],
      f4 → D[f[ux, uy, uz, vx, vy, vz], vx], f5 → D[f[ux, uy, uz, vx, vy, vz], vy],
      f6 → D[f[ux, uy, uz, vx, vy, vz], vz], g1 → D[gg[ux, uy, uz, vx, vy, vz], ux],
      g2 → D[gg[ux, uy, uz, vx, vy, vz], uy], g3 → D[gg[ux, uy, uz, vx, vy, vz], uz],
      g4 → D[gg[ux, uy, uz, vx, vy, vz], vx], g5 → D[gg[ux, uy, uz, vx, vy, vz], vy],
      g6 → D[gg[ux, uy, uz, vx, vy, vz], vz]} // Factor;
```

```
(*G - metric with upper indecies*)
```

```
G = {{-f4 g1 + f1 g4, 1/2 (-f5 g1 - f4 g2 + f2 g4 + f1 g5),
      1/2 (-f6 g1 - f4 g3 + f3 g4 + f1 g6), 1/2 (-f1 - g4)}, {1/2 (-f5 g1 - f4 g2 + f2 g4 + f1 g5),
      -f5 g2 + f2 g5, 1/2 (-f6 g2 - f5 g3 + f3 g5 + f2 g6), 1/2 (-f2 - g5)},
      {1/2 (-f6 g1 - f4 g3 + f3 g4 + f1 g6), 1/2 (-f6 g2 - f5 g3 + f3 g5 + f2 g6), -f6 g3 + f3 g6,
      1/2 (-f3 - g6)}, {1/2 (-f1 - g4), 1/2 (-f2 - g5), 1/2 (-f3 - g6), 1}} /. S1;
```

```
together[a_, b_] :=
```

```
Block[{res = 0, lcm = 1}, lcm = PolynomialLCM[Denominator[a], Denominator[b]];
res = (Factor[lcm/Denominator[a]] Numerator[a] +
```

```
Factor[lcm/Denominator[b]] Numerator[b])/lcm;
```

```
(* g - metric*)
```

```
g = Inverse[G] // Factor;
```

```
var = {x, y, z, t};
```

```

der[exp_, n_] := (D[Numerator[exp], var[[n]]] Denominator[exp] -
  D[Denominator[exp], var[[n]]] Numerator[exp]) /. Sub / Denominator[exp]^2;

varlist = {U(2,0,0,0)[x, y, z, t], U(1,1,0,0)[x, y, z, t], U(1,0,1,0)[x, y, z, t],
  U(0,2,0,0)[x, y, z, t], U(0,1,1,0)[x, y, z, t], U(0,0,2,0)[x, y, z, t],
  V(2,0,0,0)[x, y, z, t], V(1,1,0,0)[x, y, z, t], V(1,0,1,0)[x, y, z, t],
  V(0,2,0,0)[x, y, z, t], V(0,1,1,0)[x, y, z, t], V(0,0,2,0)[x, y, z, t]};

Sub = {U(0,0,0,1)[x, y, z, t] →
  f[U(1,0,0,0)[x, y, z, t], U(0,1,0,0)[x, y, z, t], U(0,0,1,0)[x, y, z, t],
  V(1,0,0,0)[x, y, z, t], V(0,1,0,0)[x, y, z, t], V(0,0,1,0)[x, y, z, t]],
  V(0,0,0,1)[x, y, z, t] → gg[U(1,0,0,0)[x, y, z, t], U(0,1,0,0)[x, y, z, t], U(0,0,1,0)[
  x, y, z, t], V(1,0,0,0)[x, y, z, t], V(0,1,0,0)[x, y, z, t], V(0,0,1,0)[x, y, z, t]]};

diffsl[list_] := Block[{list1 = {}, listn = {}, el, jj},
  Do[AppendTo[list1, list[[i]][[1]]], {i, 1, Length[list]}];
  Do[If[FreeQ[list1, der[list[[i]][[1]], 1]], jj = Factor[der[list[[i]][[2]], 1] /. Sub];
    el = der[list[[i]][[1]], 1] → jj;
    AppendTo[listn, el];
    AppendTo[list1, der[list[[i]][[1]], 1], None];
  If[FreeQ[list1, der[list[[i]][[1]], 2]], jj = Factor[der[list[[i]][[2]], 2] /. Sub];
    el = der[list[[i]][[1]], 2] → jj;
    AppendTo[listn, el];
    AppendTo[list1, der[list[[i]][[1]], 2], None];
  If[FreeQ[list1, der[list[[i]][[1]], 3]], jj = Factor[der[list[[i]][[2]], 3] /. Sub];
    el = der[list[[i]][[1]], 3] → jj;
    AppendTo[listn, el];
    AppendTo[list1, der[list[[i]][[1]], 3], None], {i, 1, Length[list]}];
  Flatten[{list, listn}]]

Sub = diffsl[Sub];
Sub = diffsl[Sub];
Sub = diffsl[Sub];
Sub = diffsl[Sub];

(*Sub - the list for factorisation due to the system and its prolongation*)

SS = {f(1,0,0,0,0)[U(1,0,0,0)[x, y, z, t], U(0,1,0,0)[x, y, z, t], U(0,0,1,0)[x, y, z, t],
  V(1,0,0,0)[x, y, z, t], V(0,1,0,0)[x, y, z, t], V(0,0,1,0)[x, y, z, t]] → f1,
  f(0,1,0,0,0)[U(1,0,0,0)[x, y, z, t], U(0,1,0,0)[x, y, z, t], U(0,0,1,0)[x, y, z, t],
  V(1,0,0,0)[x, y, z, t], V(0,1,0,0)[x, y, z, t], V(0,0,1,0)[x, y, z, t]] → f2,
  f(0,0,1,0,0)[U(1,0,0,0)[x, y, z, t], U(0,1,0,0)[x, y, z, t], U(0,0,1,0)[x, y, z, t],
  V(1,0,0,0)[x, y, z, t], V(0,1,0,0)[x, y, z, t], V(0,0,1,0)[x, y, z, t]] → f3,
  f(0,0,0,1,0)[U(1,0,0,0)[x, y, z, t], U(0,1,0,0)[x, y, z, t], U(0,0,1,0)[x, y, z, t],
  V(1,0,0,0)[x, y, z, t], V(0,1,0,0)[x, y, z, t], V(0,0,1,0)[x, y, z, t]] → f4,
  f(0,0,0,0,1)[U(1,0,0,0)[x, y, z, t], U(0,1,0,0)[x, y, z, t], U(0,0,1,0)[x, y, z, t],
  V(1,0,0,0)[x, y, z, t], V(0,1,0,0)[x, y, z, t], V(0,0,1,0)[x, y, z, t]]

```

[illegible]

[illegible]

```

V(1,0,0,0) [x, y, z, t], V(0,1,0,0) [x, y, z, t], V(0,0,1,0) [x, y, z, t] → gg36,
gg(0,0,0,2,0,0) [U(1,0,0,0) [x, y, z, t], U(0,1,0,0) [x, y, z, t], U(0,0,1,0) [x, y, z, t],
V(1,0,0,0) [x, y, z, t], V(0,1,0,0) [x, y, z, t], V(0,0,1,0) [x, y, z, t]] → gg44,
gg(0,0,0,1,1,0) [U(1,0,0,0) [x, y, z, t], U(0,1,0,0) [x, y, z, t], U(0,0,1,0) [x, y, z, t],
V(1,0,0,0) [x, y, z, t], V(0,1,0,0) [x, y, z, t], V(0,0,1,0) [x, y, z, t]] → gg45,
gg(0,0,0,1,0,1) [U(1,0,0,0) [x, y, z, t], U(0,1,0,0) [x, y, z, t], U(0,0,1,0) [x, y, z, t],
V(1,0,0,0) [x, y, z, t], V(0,1,0,0) [x, y, z, t], V(0,0,1,0) [x, y, z, t]] → gg46,
gg(0,0,0,0,2,0) [U(1,0,0,0) [x, y, z, t], U(0,1,0,0) [x, y, z, t], U(0,0,1,0) [x, y, z, t],
V(1,0,0,0) [x, y, z, t], V(0,1,0,0) [x, y, z, t], V(0,0,1,0) [x, y, z, t]] → gg55,
gg(0,0,0,0,1,1) [U(1,0,0,0) [x, y, z, t], U(0,1,0,0) [x, y, z, t], U(0,0,1,0) [x, y, z, t],
V(1,0,0,0) [x, y, z, t], V(0,1,0,0) [x, y, z, t], V(0,0,1,0) [x, y, z, t]] → gg56,
gg(0,0,0,0,0,2) [U(1,0,0,0) [x, y, z, t], U(0,1,0,0) [x, y, z, t], U(0,0,1,0) [x, y, z, t],
V(1,0,0,0) [x, y, z, t], V(0,1,0,0) [x, y, z, t], V(0,0,1,0) [x, y, z, t]] → gg66};
SS1 = {U(2,0,0,0) [x, y, z, t] → 0, U(1,1,0,0) [x, y, z, t] → 0, U(1,0,1,0) [x, y, z, t] → 0,
U(0,2,0,0) [x, y, z, t] → 0, U(0,1,1,0) [x, y, z, t] → 0, U(0,0,2,0) [x, y, z, t] → 0,
V(2,0,0,0) [x, y, z, t] → 0, V(1,1,0,0) [x, y, z, t] → 0, V(1,0,1,0) [x, y, z, t] → 0,
V(0,2,0,0) [x, y, z, t] → 0, V(0,1,1,0) [x, y, z, t] → 0, V(0,0,2,0) [x, y, z, t] → 0};

(*pt - chosen nondegenerate point of the first jets - due to transitivity of SL6
action this choice and further substitution can be made wlog, see the paper*)

pt = {f1 → 0, f2 → 1, f3 → 0, f4 → 1, f5 → 0,
f6 → 0, gg1 → 0, gg2 → 0, gg3 → 1, gg4 → 0, gg5 → 0, gg6 → 0};

(*compute the Levi-Civita connection*)
Rm[k_, i_, j_] := Block[{res = 0}, Do[
res = together[res, 1/2 G[[k]][[l]] der[g[[l]][[j]], i]];
res = together[res, 1/2 G[[k]][[l]] der[g[[i]][[l]], j]];
res = together[res, -1/2 G[[k]][[l]] der[g[[i]][[j]], l]], {l, 1, 4}];
Factor[res /. SS /. pt];

(*glist - list of connection elements*)
glist = {};
Do[Do[Do[AppendTo[glist, R[k, i, j] → Rm[k, i, j]], {j, 1, 4}], {i, 1, 4}], {k, 1, 4}]

(*compute the Riemann curvature*)
Rm[i_, q_, k_, l_] := Block[{res = 0}, res = together[res, der[(R[i, q, k] /. glist), l]];
res = together[res, -der[(R[i, q, l] /. glist), k]];
(*Do[res=res+(R[i,p,l] /. glist) (R[p,q,k] /. glist) - (R[i,p,k] /. glist)
(R[p,q,l] /. glist), {p, 1, 4}];*) res = Factor[(res /. SS) /. SS1 /. pt];
res];

(*Rlist - list of symbols of Riemann tensor elements*)

```

```

Rlist = {};
Do[Do[Do[Do[js = Rm[i, j, k, l];
  el = R[i, j, k, l] → js;
  AppendTo[Rlist, el];
  el = R[i, j, l, k] → -js;
  AppendTo[Rlist, el], {l, k + 1, 4}];
  el = R[i, j, k, k] → 0;
  AppendTo[Rlist, el], {k, 1, 4}], {j, 1, 4}], {i, 1, 4}];

(*gcompute the Ricci curvature*)

RRm[q_, l_] := Block[{el = 0;
  Do[el = together[el, (R[i, q, i, l] /. Rlist)], {i, 1, 4}];
  Factor[el]]

RRlist = {};
Do[Do[AppendTo[RRlist, RR[q, l] → RRm[q, l]], {l, 1, 4}], {q, 1, 4}]

(*S - scalar curvature*)

(*S*)
S = 0;
Do[Do[S = together[S, (G[[l]][[q]] /. SS /. pt) (RR[q, l] /. RRlist)], {q, 1, 4}],
  {l, 1, 4}];
S = Factor[S];

(*R1 - lowering the first index in R*)

R1[i_, j_, k_, l_] := Block[{res = 0;
  Do[res = together[res, (g[[i]][[s]] /. SS /. pt) (R[s, j, k, l] /. Rlist)], {s, 1, 4}];
  Factor[res]];

(*gcompute the Weyl curvature*)

w[i_, j_] := Factor[together[1/2 (RR[i, j] /. RRlist), -S/12 (g[[i]][[j]] /. SS /. pt)]];

Wm[i_, j_, k_, l_] := Block[{res = 0; res = together[res, (R1[i, j, k, l])];
  res = together[res, -w[i, k] (g[[j]][[l]] /. SS /. pt)];
  res = together[res, -w[j, l] (g[[i]][[k]] /. SS /. pt)];
  res = together[res, +w[j, k] (g[[i]][[l]] /. SS /. pt)];
  res = together[res, +w[i, l] (g[[j]][[k]] /. SS /. pt)];
  Factor[res]];

Wlist = {};
Do[Do[Do[el = W[i, j, k, k] → 0;
  AppendTo[Wlist, el];
  el = W[k, k, i, j] → 0;
  AppendTo[Wlist, el], {k, 1, 4}], {j, 1, 4}], {i, 1, 4}]

```

```

Do[Do[Do[Do[js = W[i, j, k, l];
  el = W[i, j, k, l] → js;
  AppendTo[Wlist, el];
  el = W[i, j, l, k] → -js;
  AppendTo[Wlist, el];
  el = W[j, i, k, l] → -js;
  AppendTo[Wlist, el];
  el = W[j, i, l, k] → js;
  AppendTo[Wlist, el];
  el = W[k, l, i, j] → js;
  AppendTo[Wlist, el];
  el = W[k, l, j, i] → -js;
  AppendTo[Wlist, el];
  el = W[l, k, i, j] → -js;
  AppendTo[Wlist, el];
  el = W[l, k, j, i] → js;
  AppendTo[Wlist, el], {l, j + (k + 1 - j) Sign[k - i], 4}], {k, i, 4}], {j, i + 1, 4}],
{i, 1, 4}];
Wlist = Union[Wlist];

Wlist1 = {};
Do[Do[Do[Do[js = Wm[i, j, k, l];
  el = W[i, j, k, l] → js;
  AppendTo[Wlist1, el], {l, j + (k + 1 - j) Sign[k - i], 4}], {k, i, 4}], {j, i + 1, 4}],
{i, 1, 4}];

Wlist2 = Wlist1;

(*Wlist1, (or Wlist2) - list of components of the Weyl tensor*)

```

```

elist = {};
Do[Do[Do[Do[AppendTo[elist, e[i1, i2, i3, i4] → 0], {i4, 1, 4}], {i3, 1, 4}], {i2, 1, 4}],
  {i1, 1, 4}];
elist1 = {};
AppendTo[elist1, {e[1, 2, 3, 4] → 1,
  e[1, 2, 4, 3] → -1,
  e[1, 3, 2, 4] → -1,
  e[1, 3, 4, 2] → 1,
  e[1, 4, 2, 3] → 1,
  e[1, 4, 3, 2] → -1,
  e[2, 1, 3, 4] → -1,
  e[2, 1, 4, 3] → 1,
  e[2, 3, 1, 4] → 1,
  e[2, 3, 4, 1] → -1,
  e[2, 4, 1, 3] → -1,
  e[2, 4, 3, 1] → 1,
  e[3, 1, 2, 4] → 1,
  e[3, 1, 4, 2] → -1,
  e[3, 2, 1, 4] → -1,
  e[3, 2, 4, 1] → 1,
  e[3, 4, 1, 2] → 1,
  e[3, 4, 2, 1] → -1,
  e[4, 1, 2, 3] → -1,
  e[4, 1, 3, 2] → 1,
  e[4, 2, 1, 3] → 1,
  e[4, 2, 3, 1] → -1,
  e[4, 3, 1, 2] → -1,
  e[4, 3, 2, 1] → 1}];
elist1 = Flatten[elist1];

(* elist - absolutely antisymmetric tensor *)

(* WW - Weyl tensor with the upper first two indecies
  Gsqrt - root of the determinant of the metric
  Vol - volume form *)

WW[i_, j_, k_, l_] := Block[{res, a, b}, res = 0;
  Do[Do[res = together[res, (G[[i]][[a]] /. SS /. pt) (G[[j]][[b]] /. SS /. pt)
    (W[a, b, k, l] /. Wlist /. Wlist2)], {b, 1, 4}], {a, 1, 4}];
  Factor[res]];
Gsqrt =  $\frac{1}{4} (-gg^{(0,0,0,0,1,0)} [U^{(1,0,0,0)} [x, y, z, t], U^{(0,1,0,0)} [x, y, z, t], U^{(0,0,1,0)} [x, y, z, t],$ 
   $V^{(1,0,0,0)} [x, y, z, t], V^{(0,1,0,0)} [x, y, z, t], V^{(0,0,1,0)} [x, y, z, t]]$ 
   $f^{(0,0,0,1,0,0)} [U^{(1,0,0,0)} [x, y, z, t], U^{(0,1,0,0)} [x, y, z, t], U^{(0,0,1,0)} [x, y, z, t],$ 
   $V^{(1,0,0,0)} [x, y, z, t], V^{(0,1,0,0)} [x, y, z, t], V^{(0,0,1,0)} [x, y, z, t]]$ 
   $gg^{(0,0,1,0,0,0)} [U^{(1,0,0,0)} [x, y, z, t], U^{(0,1,0,0)} [x, y, z, t], U^{(0,0,1,0)} [x, y, z, t],$ 

```



[illegible]

```

gg(0,0,0,0,0,1) [U(1,0,0,0) [x, y, z, t], U(0,1,0,0) [x, y, z, t], U(0,0,1,0) [x, y, z, t],
  V(1,0,0,0) [x, y, z, t], V(0,1,0,0) [x, y, z, t], V(0,0,1,0) [x, y, z, t]]
f(0,0,0,0,1,0) [U(1,0,0,0) [x, y, z, t], U(0,1,0,0) [x, y, z, t], U(0,0,1,0) [x, y, z, t],
  V(1,0,0,0) [x, y, z, t], V(0,1,0,0) [x, y, z, t], V(0,0,1,0) [x, y, z, t]]
gg(1,0,0,0,0,0) [U(1,0,0,0) [x, y, z, t], U(0,1,0,0) [x, y, z, t], U(0,0,1,0) [x, y, z, t],
  V(1,0,0,0) [x, y, z, t], V(0,1,0,0) [x, y, z, t], V(0,0,1,0) [x, y, z, t]] +
f(0,0,0,0,0,1) [U(1,0,0,0) [x, y, z, t], U(0,1,0,0) [x, y, z, t], U(0,0,1,0) [x, y, z, t],
  V(1,0,0,0) [x, y, z, t], V(0,1,0,0) [x, y, z, t], V(0,0,1,0) [x, y, z, t]]
gg(0,0,0,0,1,0) [U(1,0,0,0) [x, y, z, t], U(0,1,0,0) [x, y, z, t], U(0,0,1,0) [x, y, z, t],
  V(1,0,0,0) [x, y, z, t], V(0,1,0,0) [x, y, z, t], V(0,0,1,0) [x, y, z, t]]
gg(1,0,0,0,0,0) [U(1,0,0,0) [x, y, z, t], U(0,1,0,0) [x, y, z, t], U(0,0,1,0) [x, y, z, t],
  V(1,0,0,0) [x, y, z, t], V(0,1,0,0) [x, y, z, t], V(0,0,1,0) [x, y, z, t]] +
f(0,0,0,0,1,0) [U(1,0,0,0) [x, y, z, t], U(0,1,0,0) [x, y, z, t], U(0,0,1,0) [x, y, z, t],
  V(1,0,0,0) [x, y, z, t], V(0,1,0,0) [x, y, z, t], V(0,0,1,0) [x, y, z, t]]
f(0,0,1,0,0,0) [U(1,0,0,0) [x, y, z, t], U(0,1,0,0) [x, y, z, t], U(0,0,1,0) [x, y, z, t],
  V(1,0,0,0) [x, y, z, t], V(0,1,0,0) [x, y, z, t], V(0,0,1,0) [x, y, z, t]]
gg(1,0,0,0,0,0) [U(1,0,0,0) [x, y, z, t], U(0,1,0,0) [x, y, z, t], U(0,0,1,0) [x, y, z, t],
  V(1,0,0,0) [x, y, z, t], V(0,1,0,0) [x, y, z, t], V(0,0,1,0) [x, y, z, t]] -
f(0,0,0,0,0,1) [U(1,0,0,0) [x, y, z, t], U(0,1,0,0) [x, y, z, t], U(0,0,1,0) [x, y, z, t],
  V(1,0,0,0) [x, y, z, t], V(0,1,0,0) [x, y, z, t], V(0,0,1,0) [x, y, z, t]]
f(0,1,0,0,0,0) [U(1,0,0,0) [x, y, z, t], U(0,1,0,0) [x, y, z, t], U(0,0,1,0) [x, y, z, t],
  V(1,0,0,0) [x, y, z, t], V(0,1,0,0) [x, y, z, t], V(0,0,1,0) [x, y, z, t]]
gg(1,0,0,0,0,0) [U(1,0,0,0) [x, y, z, t], U(0,1,0,0) [x, y, z, t], U(0,0,1,0) [x, y, z, t],
  V(1,0,0,0) [x, y, z, t], V(0,1,0,0) [x, y, z, t], V(0,0,1,0) [x, y, z, t]]
V(1,0,0,0) [x, y, z, t], V(0,1,0,0) [x, y, z, t], V(0,0,1,0) [x, y, z, t]] /. SS /. pt;
Vol[i_, j_, k_, l_] := (ϵ[i, j, k, l] /. ϵlist1 /. ϵlist) / Gsqrt;

(*WS=W^* -- Hodge star applied to W*)
WS[i_, j_, k_, l_] := Block[{res = 0, a, b},
  Do[Do[res = together[res, 1 / 2 Vol[i, j, a, b] WW[a, b, k, l]], {b, 1, 4}], {a, 1, 4}];
  res];

(*Wplus - 1/2(W + Self-Dual part of W);
Wminus - 1/2(W - Self-Dual part of W)*)
Wplus[i_, j_, k_, l_] :=
  1 / 2 (together[W[i, j, k, l] /. Wlist /. Wlist1], WS[i, j, k, l]);
Wminus[i_, j_, k_, l_] :=
  1 / 2 (together[W[i, j, k, l] /. Wlist /. Wlist1], -WS[i, j, k, l]);

Wpluslist = {};
Do[Do[Do[Do[AppendTo[Wpluslist, Factor[Wplus[i, j, k, l]]], {l, 1, 4}], {k, 1, 4}],
  {j, 1, 4}], {i, 1, 4}]

```

```

Wminuslist = {};
Do[Do[Do[Do[AppendTo[Wminuslist, Factor[Wminus[i, j, k, l]]], {l, 1, 4}], {k, 1, 4}],
    {j, 1, 4}], {i, 1, 4}]

(* splitting Wplus and Wminus by third derivatives*)
vars = {U(3,0,0,0)[x, y, z, t], U(2,1,0,0)[x, y, z, t], U(2,0,1,0)[x, y, z, t],
    U(1,2,0,0)[x, y, z, t], U(1,1,1,0)[x, y, z, t], U(1,0,2,0)[x, y, z, t], U(0,3,0,0)[x, y, z, t],
    U(0,2,1,0)[x, y, z, t], U(0,1,2,0)[x, y, z, t], U(0,0,3,0)[x, y, z, t], V(3,0,0,0)[x, y, z, t],
    V(2,1,0,0)[x, y, z, t], V(2,0,1,0)[x, y, z, t], V(1,2,0,0)[x, y, z, t],
    V(1,1,1,0)[x, y, z, t], V(1,0,2,0)[x, y, z, t], V(0,3,0,0)[x, y, z, t],
    V(0,2,1,0)[x, y, z, t], V(0,1,2,0)[x, y, z, t], V(0,0,3,0)[x, y, z, t]};

sysplus = {};
Do[Do[var = vars[[j]];
    varc = Complement[vars, {var}];
    el = Numerator[Wpluslist[[i]]] /. var → 1;
    Do[el = el /. varc[[k]] → 0, {k, 1, Length[varc]}];
    el = Factor[el];
    AppendTo[sysplus, el];
    , {j, 1, Length[vars]}], {i, 1, Length[Wpluslist]}]

sysminus = {};
Do[Do[var = vars[[j]];
    varc = Complement[vars, {var}];
    el = Numerator[Wminuslist[[i]]] /. var → 1;
    Do[el = el /. varc[[k]] → 0, {k, 1, Length[varc]}];
    el = Factor[el];
    AppendTo[sysminus, el];
    , {j, 1, Length[vars]}], {i, 1, Length[Wminuslist]}]

Length[ToRules[Reduce[sysminus == 0]]]

```

24

(\*L - Monge - Ampere conditions; taken from the Maple files\*)

```

L = {f11 → -2 * gg1 * p1, f12 → -gg1 * p2 - gg2 * p1, f13 → -gg1 * p3 - gg3 * p1,
      f14 → f1 * p1 - gg4 * p1, f15 → f1 * p2 - gg5 * p1 + a12, f16 → f1 * p3 - gg6 * p1 + a13,
      f22 → -2 * gg2 * p2, f23 → -gg2 * p3 - gg3 * p2, f24 → f2 * p1 - gg4 * p2 - a12,
      f25 → f2 * p2 - gg5 * p2, f26 → f2 * p3 - gg6 * p2 + a23, f33 → -2 * gg3 * p3,
      f34 → f3 * p1 - gg4 * p3 - a13, f35 → f3 * p2 - gg5 * p3 - a23, f36 → f3 * p3 - gg6 * p3,
      f44 → 2 * f4 * p1, f45 → f4 * p2 + f5 * p1, f46 → f4 * p3 + f6 * p1, f55 → 2 * f5 * p2,
      f56 → f5 * p3 + f6 * p2, f66 → 2 * f6 * p3, gg11 → -2 * gg1 * q1, gg12 → -gg1 * q2 - gg2 * q1,
      gg13 → -gg1 * q3 - gg3 * q1, gg14 → f1 * q1 - gg4 * q1, gg15 → f1 * q2 - gg5 * q1 + b12,
      gg16 → f1 * q3 - gg6 * q1 + b13, gg22 → -2 * gg2 * q2, gg23 → -gg2 * q3 - gg3 * q2,
      gg24 → f2 * q1 - gg4 * q2 - b12, gg25 → f2 * q2 - gg5 * q2, gg26 → f2 * q3 - gg6 * q2 + b23,
      gg33 → -2 * gg3 * q3, gg34 → f3 * q1 - gg4 * q3 - b13, gg35 → f3 * q2 - gg5 * q3 - b23,
      gg36 → f3 * q3 - gg6 * q3, gg44 → 2 * f4 * q1, gg45 → f4 * q2 + f5 * q1,
      gg46 → f4 * q3 + f6 * q1, gg55 → 2 * f5 * q2, gg56 → f5 * q3 + f6 * q2, gg66 → 2 * f6 * q3};
L0 =
  L /.
  pt;

```

(\*The conditions  $W^+=0$  is equivalent to Monge-Ampere conditions\*)

```
Length[ToRules[Reduce[sysplus == 0]]]
```

```
30
```

```
Complement[(sysplus /. L0 // Factor), {0}]
```

```
{}
```

These 30 conditions are precisely the Monge-Ampere constraints (signs are interchanged wrt the paper and our Maple conventions).

(\*Ld0, Ld1 - conditions of linear degeneracy at the point pt\*)

```

Ld0 = {f11 → -2 * gg14, f12 → -f14 - gg13 - gg15 - gg24, f13 → -f15 - f24 - gg45 - gg23,
      f22 → 0, f23 → -f45 - gg26 - gg35 + gg46, f25 → f45 + gg26 + gg35 - gg46,
      f26 → -f35 - gg56 + f46 + gg36, f33 → -2 * f46 - 2 * gg36, f36 → -f56,
      f44 → -2 * gg16 - 2 * gg34 + 2 * f15 + 2 * f24 + 2 * gg45 + 2 * gg23, f55 → 2 * gg56, f66 → 0,
      gg11 → 0, gg12 → gg14, gg22 → 2 * f14 + 2 * gg13 + 2 * gg15 + 2 * gg24, gg25 → gg45,
      gg33 → -2 * f16 - 2 * f34 - 2 * gg46, gg44 → -2 * f14 - 2 * gg13, gg55 → 0, gg66 → 2 * f56};
Ld1 = {f15 → gg16 - gg45, f35 → f46 + gg36 - gg56, f45 → f16 - gg35 + gg46, gg15 → 0};

```

(\* $W^-=0$  is equivalent to linear degeneracy conditions\*)

```
Length[ToRules[Reduce[sysminus == 0]]]
```

```
24
```

```
Complement[(sysminus /. Ld0 /. Ld1 // Factor), {0}]
```

```
{}
```

These 24 conditions are precisely the general equations of linear degeneracy (signs are interchanged wrt the paper and our Maple conventions).

(\*W=0 <=>  $W^-=W^+=0$  is equivalent to linearizability conditions\*)

syszero = {sysplus, sysminus} // Flatten;

Length[ToRules[Reduce[syszero == 0]]]

34

Complement[(syszero /. Ld0 /. Ld1 /. L0 // Factor), {0}]

{}

These 34 conditions are precisely the linearizability equations for 2x2 systems (compare the Maple files).
